# Supplementary material for: On Sequences in Cyclic Groups with Distinct Partial Sums
Source: arXiv:2203.16658 ancillary file (2022-04-01)
Supplement: Supplementary file 1 [file Tables.pdf]

# On Sequences in Cyclic Groups with Distinct Partial Sums - Additional Material

S. Costa, S. Della Fiore, M. A. Ollis and S. Z. Rovner-Frydman

$$S \subseteq \mathbb{Z}_p \times \mathbb{Z}_2 \setminus \{(0, 0)\}, |S| = 10$$

| $\lambda$ | $\mathbf{a}$                   | deg | monomial/s                                                       | coefficient/s                           |
|-----------|--------------------------------|-----|------------------------------------------------------------------|-----------------------------------------|
| (10, 0)   | (0, 0, 0, 0, 0, 0, 0, 0, 0, 0) | 89  | $x_1^8 x_2^9 x_3^9 x_4^9 x_5^9 x_6^9 x_7^9 x_8^9 x_9^9 x_{10}^9$ | $2^5 \cdot 7 \cdot 11^2 \cdot 21966239$ |
|           |                                |     | $x_1^9 x_2^8 x_3^9 x_4^9 x_5^9 x_6^9 x_7^9 x_8^9 x_9^9 x_{10}^9$ | $2 \cdot 13 \cdot 211 \cdot 256046627$  |
| (9, 1)    | (0, 0, 0, 0, 0, 1, 0, 0, 0, 0) | 52  | $x_2^2 x_3^4 x_4^7 x_5^8 x_7^8 x_8^8 x_9^8 x_{10}^8$             | $-1 \cdot 2^2$                          |
| (8, 2)    | (0, 1, 0, 0, 0, 0, 1, 0, 0, 0) | 45  | $x_1 x_3 x_4^7 x_5^7 x_6^7 x_7 x_8^7 x_9^7 x_{10}^7$             | $-1 \cdot 2 \cdot 3 \cdot 7$            |
| (7, 3)    | (0, 0, 0, 0, 1, 0, 0, 0, 1, 1) | 42  | $x_2^6 x_3^6 x_4^2 x_5^6 x_6^6 x_7^6 x_8^2 x_9^2 x_{10}^2$       | $-1 \cdot 2 \cdot 3 \cdot 7$            |
| (6, 4)    | (0, 0, 0, 1, 0, 0, 0, 1, 1, 1) | 39  | $x_1^5 x_2^5 x_3^5 x_4^3 x_5^5 x_6^5 x_7^3 x_8^3 x_9^3 x_{10}^2$ | $2 \cdot 5$                             |
| (5, 5)    | (0, 0, 0, 1, 0, 0, 1, 1, 1, 1) | 40  | $x_1^4 x_2^4 x_3^4 x_4^4 x_5^4 x_6^4 x_7^4 x_8^4 x_9^4 x_{10}^4$ | $2^2 \cdot 157$                         |
|           |                                |     | (0, 1, 0, 1, 0, 1, 0, 1, 0, 1)                                   | 40                                      |
| (4, 6)    | (0, 1, 0, 1, 1, 1, 1, 0, 1, 0) | 41  | $x_2^2 x_3^5 x_4^3 x_5^5 x_6^5 x_7^5 x_8^3 x_9^5 x_{10}^3$       | $2^4 \cdot 3 \cdot 5 \cdot 13$          |
|           |                                |     | $x_1^3 x_2^4 x_3^3 x_4^2 x_5^5 x_6^5 x_7^3 x_8^5 x_9^3 x_{10}^3$ | $2 \cdot 3 \cdot 463$                   |
| (3, 7)    | (0, 0, 1, 0, 1, 1, 1, 1, 1, 1) | 46  | $x_2^2 x_3^6 x_4^2 x_5^6 x_6^6 x_7^6 x_8^6 x_9^6 x_{10}^6$       | $-1 \cdot 2^3 \cdot 3^2$                |
| (2, 8)    | (0, 1, 0, 1, 1, 1, 1, 1, 1, 1) | 51  | $x_1 x_2 x_3 x_4^6 x_5^7 x_6^7 x_7^7 x_8^7 x_9^7 x_{10}^7$       | $-1 \cdot 2 \cdot 1277$                 |
|           |                                |     | $x_1 x_3 x_4^7 x_5^7 x_6^7 x_7^7 x_8^7 x_9^7 x_{10}^7$           | $-1 \cdot 2 \cdot 17^2$                 |
| (1, 9)    | (1, 0, 1, 1, 1, 1, 1, 1, 1, 1) | 60  | $x_2^2 x_3^2 x_4^8 x_5^8 x_6^8 x_7^8 x_8^8 x_9^8 x_{10}^8$       | $2 \cdot 17^2$                          |
|           |                                |     | $x_1^2 x_2^3 x_3^7 x_4^8 x_5^8 x_6^8 x_7^8 x_8^8 x_9^8 x_{10}^8$ | $2^2 \cdot 647$                         |
| (0, 10)   | (1, 1, 1, 1, 1, 1, 1, 1, 1, 1) | 69  | $x_1^2 x_2^2 x_3^4 x_4^7 x_5^9 x_6^9 x_7^9 x_8^9 x_9^9 x_{10}^9$ | $2 \cdot 3 \cdot 733$                   |
|           |                                |     | $x_1^2 x_2^2 x_3^4 x_4^9 x_5^9 x_6^9 x_7^9 x_8^9 x_9^9 x_{10}^9$ | $2^5 \cdot 3^2 \cdot 5$                 |

$$S \subseteq \mathbb{Z}_p \times \mathbb{Z}_3 \setminus \{(0, 0)\}, |S| = 10$$

| $\lambda$  | $\mathbf{a}$                   | deg | monomial/s                                                       | coefficient/s                           |
|------------|--------------------------------|-----|------------------------------------------------------------------|-----------------------------------------|
| (10, 0, 0) | (0, 0, 0, 0, 0, 0, 0, 0, 0, 0) | 89  | $x_1^8 x_2^9 x_3^9 x_4^9 x_5^9 x_6^9 x_7^9 x_8^9 x_9^9 x_{10}^9$ | $2^5 \cdot 7 \cdot 11^2 \cdot 21966239$ |
|            |                                |     | $x_1^9 x_2^8 x_3^9 x_4^9 x_5^9 x_6^9 x_7^9 x_8^9 x_9^9 x_{10}^9$ | $2 \cdot 13 \cdot 211 \cdot 256046627$  |
| (9, 1, 0)  | (0, 0, 0, 0, 0, 1, 0, 0, 0, 0) | 52  | $x_2^2 x_3^4 x_4^7 x_5^8 x_7^8 x_8^8 x_9^8 x_{10}^8$             | $-1 \cdot 2^2$                          |
| (8, 2, 0)  | (0, 0, 0, 1, 0, 0, 0, 1, 0, 0) | 36  | $x_2^2 x_3^4 x_5^3 x_6^6 x_7^7 x_8^6 x_9^7 x_{10}^7$             | $-1 \cdot 2$                            |
| (8, 1, 1)  | (0, 0, 0, 0, 1, 0, 0, 0, 0, 2) | 44  | $x_1 x_2^3 x_3^6 x_4^7 x_5^6 x_6^7 x_7^7 x_8^7 x_9^7$            | $-1 \cdot 2^2$                          |

$$S \subseteq \mathbb{Z}_p \times \mathbb{Z}_3 \setminus \{(0, 0)\}, |S| = 10$$

| $\lambda$ | $\mathbf{a}$                   | deg | monomial/s                                              | coefficient/s  |
|-----------|--------------------------------|-----|---------------------------------------------------------|----------------|
| (7, 3, 0) | (0, 0, 1, 0, 0, 0, 1, 0, 0, 1) | 31  | $x_1x_2^3x_4^2x_5^5x_6^6x_7x_8^5x_9^6x_{10}^2$          | $-1 \cdot 2$   |
| (7, 2, 1) | (0, 0, 0, 1, 0, 0, 1, 0, 0, 2) | 30  | $x_2^2x_3^4x_4x_5^5x_6^6x_7x_8^5x_9^6$                  | 2              |
| (6, 4, 0) | (0, 0, 1, 0, 0, 1, 0, 0, 1, 1) | 30  | $x_2^2x_3^2x_4^4x_5^5x_6^2x_7x_8^5x_9^3x_{10}^3$        | 2              |
| (6, 3, 1) | (0, 0, 0, 1, 0, 0, 1, 0, 2, 1) | 27  | $x_2^2x_3^5x_4x_5^5x_6^2x_7x_8^5x_{10}^2$               | -1             |
| (6, 2, 2) | (0, 0, 1, 0, 0, 1, 0, 0, 2, 2) | 25  | $x_1x_2^3x_4^4x_5^5x_6^4x_7x_8^5x_9x_{10}$              | $-1 \cdot 2$   |
| (5, 5, 0) | (0, 0, 1, 0, 0, 1, 0, 1, 1, 1) | 30  | $x_2^2x_3x_4^3x_5^4x_6^4x_7^4x_8^4x_9^4x_{10}^4$        | $-1 \cdot 3^2$ |
| (5, 4, 1) | (0, 0, 1, 0, 0, 1, 0, 2, 1, 1) | 25  | $x_1x_2^3x_3x_4^3x_5^4x_6^3x_7^4x_9^3x_{10}^3$          | 1              |
| (5, 3, 2) | (0, 0, 0, 1, 0, 1, 0, 2, 1, 2) | 24  | $x_1^4x_2^4x_3^3x_4^2x_5^4x_6^2x_7^2x_8x_9^2$           | 2              |
| (4, 6, 0) | (0, 1, 0, 0, 1, 0, 1, 1, 1, 1) | 31  | $x_1^3x_2^5x_3^3x_4^5x_5^3x_6^4x_7^4x_8x_9$             | -1             |
| (4, 5, 1) | (0, 0, 1, 0, 1, 0, 1, 1, 1, 2) | 27  | $x_2^2x_3^3x_4^3x_5^4x_6^3x_7^4x_8^4x_9^4$              | $2^2 \cdot 3$  |
| (4, 4, 2) | (0, 0, 0, 1, 0, 1, 2, 1, 2, 1) | 24  | $x_1^2x_2^2x_3^3x_4^3x_5^3x_6^3x_7x_8^3x_9x_{10}^3$     | -2             |
| (4, 3, 3) | (0, 0, 1, 0, 1, 0, 2, 1, 2, 2) | 22  | $x_1x_2^3x_3^2x_4^2x_5^3x_6^3x_7^2x_8^2x_9^2x_{10}^2$   | $2^2 \cdot 3$  |
| (3, 7, 0) | (0, 1, 0, 1, 0, 1, 1, 1, 1, 1) | 36  | $x_2x_3^2x_4x_5^6x_6^6x_7x_8^6x_9^6x_{10}^6$            | -1             |
| (3, 6, 1) | (0, 0, 1, 0, 1, 1, 1, 1, 2, 1) | 30  | $x_1^2x_2x_3^5x_4^2x_5^5x_6^5x_7^5x_8^4x_{10}$          | 1              |
| (3, 5, 2) | (0, 0, 1, 0, 1, 2, 1, 2, 1, 1) | 25  | $x_1^2x_2^2x_3x_4^2x_5^4x_6x_7^4x_8x_9^4x_{10}^4$       | 2              |
| (3, 4, 3) | (0, 0, 1, 0, 1, 1, 2, 2, 1, 2) | 24  | $x_1^2x_2^2x_3^3x_4^2x_5^3x_6^3x_7^2x_8^3x_9^3x_{10}^2$ | $-1 \cdot 2^2$ |
| (2, 8, 0) | (0, 1, 0, 1, 1, 1, 1, 1, 1, 1) | 42  | $x_3x_4^2x_5^4x_6^7x_7^7x_8^7x_9^7x_{10}^7$             | -1             |
| (2, 7, 1) | (0, 1, 0, 1, 1, 1, 1, 2, 1, 1) | 34  | $x_1x_3x_4^2x_5^6x_6^6x_7x_8^6x_{10}^6$                 | -1             |
| (2, 6, 2) | (2, 0, 1, 1, 1, 1, 1, 2, 1, 0) | 30  | $x_3^3x_4^5x_5^5x_6^5x_7^5x_8x_9^5x_{10}$               | 2              |
| (2, 5, 3) | (2, 1, 1, 1, 0, 2, 2, 1, 0, 1) | 27  | $x_1^2x_2^4x_3^4x_4^2x_6^2x_7^4x_8^4x_9x_{10}^4$        | $-1 \cdot 3^3$ |
| (2, 4, 4) | (0, 1, 0, 1, 1, 2, 2, 1, 2, 2) | 25  | $x_1x_2^2x_3x_4^3x_5^3x_6^3x_7^3x_8^3x_9^3x_{10}^3$     | 3              |
| (1, 9, 0) | (1, 0, 1, 1, 1, 1, 1, 1, 1, 1) | 49  | $x_3x_4^4x_5^5x_6^7x_7^8x_8^8x_9^8x_{10}^8$             | $2 \cdot 3$    |
| (1, 8, 1) | (0, 1, 1, 1, 1, 1, 1, 1, 1, 2) | 42  | $x_2x_3^2x_4^4x_5^7x_6^7x_7^7x_8^7x_9^7$                | 1              |
| (1, 7, 2) | (0, 1, 1, 1, 1, 1, 1, 2, 2, 1) | 36  | $x_3^4x_4^6x_5^6x_6^6x_7^6x_8x_9x_{10}^6$               | $2^2 \cdot 3$  |
| (1, 6, 3) | (1, 1, 0, 1, 1, 1, 2, 1, 2, 2) | 31  | $x_2^5x_4^5x_5^5x_6^2x_7^5x_8^2x_9^2x_{10}^2$           | $-1 \cdot 2^2$ |

$$S \subseteq \mathbb{Z}_p \times \mathbb{Z}_3 \setminus \{(0, 0)\}, |S| = 10$$

| $\lambda$  | $\mathbf{a}$                   | deg | monomial/s                                                     | coefficient/s  |
|------------|--------------------------------|-----|----------------------------------------------------------------|----------------|
| (1, 5, 4)  | (0, 1, 1, 1, 1, 1, 2, 2, 2, 2) | 30  | $x_2^4 x_3^4 x_4^4 x_5^4 x_6^3 x_7^3 x_8^3 x_9 x_{10}$         | -1             |
| (0, 10, 0) | (1, 1, 1, 1, 1, 1, 1, 1, 1, 1) | 60  | $x_1^2 x_2^2 x_3^4 x_4^7 x_5^9 x_6^9 x_7^9 x_8^9 x_9^9 x_{10}$ | $-1 \cdot 3$   |
| (0, 9, 1)  | (1, 1, 1, 1, 1, 2, 1, 1, 1, 1) | 51  | $x_2^2 x_3^3 x_4^6 x_5^8 x_7^8 x_8^8 x_9^8 x_{10}$             | $2 \cdot 5$    |
| (0, 8, 2)  | (1, 1, 1, 1, 1, 1, 1, 1, 2, 2) | 43  | $x_2^2 x_3^4 x_4^7 x_5^7 x_6^7 x_7^7 x_8^7 x_9 x_{10}$         | -1             |
| (0, 7, 3)  | (2, 1, 1, 1, 1, 1, 1, 1, 2, 2) | 39  | $x_1 x_2^2 x_3^2 x_4^6 x_5^6 x_6^6 x_7^6 x_8^6 x_9^2 x_{10}^2$ | 1              |
| (0, 6, 4)  | (2, 1, 2, 1, 1, 1, 1, 1, 2, 2) | 38  | $x_1 x_2^3 x_3^3 x_4^5 x_5^5 x_6^5 x_7^5 x_8^3 x_9^3 x_{10}$   | $-1 \cdot 2^2$ |
| (0, 5, 5)  | (1, 1, 1, 1, 1, 2, 2, 2, 2, 2) | 34  | $x_2^2 x_3^4 x_4^4 x_5^4 x_6^4 x_7^4 x_8^4 x_9^4 x_{10}$       | -1             |

$$S \subseteq \mathbb{Z}_p \times \mathbb{Z}_4 \setminus \{(0, 0)\}, |S| = 10$$

| $\lambda$     | $\mathbf{a}$                   | deg | monomial/s                                                                                                                           | coefficient/s                                                                     |
|---------------|--------------------------------|-----|--------------------------------------------------------------------------------------------------------------------------------------|-----------------------------------------------------------------------------------|
| (10, 0, 0, 0) | (0, 0, 0, 0, 0, 0, 0, 0, 0, 0) | 89  | $x_1^8 x_2^9 x_3^9 x_4^9 x_5^9 x_6^9 x_7^9 x_8^9 x_9^9 x_{10}^9$<br>$x_1^9 x_2^8 x_3^9 x_4^9 x_5^9 x_6^9 x_7^9 x_8^9 x_9^9 x_{10}^9$ | $2^5 \cdot 7 \cdot 11^2 \cdot 21966239$<br>$2 \cdot 13 \cdot 211 \cdot 256046627$ |
| (9, 1, 0, 0)  | (0, 0, 0, 0, 0, 1, 0, 0, 0, 0) | 52  | $x_2^2 x_3^4 x_4^7 x_5^8 x_7^8 x_8^8 x_9^8 x_{10}$                                                                                   | $-1 \cdot 2^2$                                                                    |
| (9, 0, 1, 0)  | (0, 0, 0, 0, 0, 2, 0, 0, 0, 0) | 52  | $x_2^2 x_3^4 x_4^7 x_5^8 x_7^8 x_8^8 x_9^8 x_{10}$                                                                                   | $-1 \cdot 2^2$                                                                    |
| (8, 2, 0, 0)  | (0, 0, 0, 1, 0, 0, 0, 1, 0, 0) | 36  | $x_2^2 x_3^4 x_5^6 x_6^7 x_7^8 x_8^6 x_9^7 x_{10}$                                                                                   | $-1 \cdot 2$                                                                      |
| (8, 1, 0, 1)  | (0, 0, 0, 0, 1, 0, 0, 0, 0, 3) | 44  | $x_1 x_2^3 x_3^6 x_4^7 x_6^6 x_7^7 x_8^7 x_9^7$                                                                                      | $-1 \cdot 2^2$                                                                    |
| (8, 1, 1, 0)  | (0, 0, 0, 1, 0, 0, 0, 2, 0, 0) | 35  | $x_2^2 x_3^4 x_5^6 x_6^7 x_7^6 x_9^7 x_{10}$                                                                                         | $-1 \cdot 2$                                                                      |
| (8, 0, 2, 0)  | (0, 0, 0, 0, 2, 0, 0, 0, 0, 2) | 45  | $x_1 x_2^3 x_3^6 x_4^7 x_6^6 x_7^7 x_8^7 x_9^7 x_{10}$                                                                               | $-1 \cdot 2^2$                                                                    |
| (7, 3, 0, 0)  | (0, 0, 1, 0, 0, 1, 0, 0, 1, 0) | 27  | $x_2^2 x_4^2 x_5^4 x_6^4 x_7^6 x_8^6 x_9^6 x_{10}$                                                                                   | 1                                                                                 |
| (7, 2, 0, 1)  | (0, 0, 0, 1, 0, 0, 1, 0, 0, 3) | 30  | $x_2^2 x_3^4 x_4^5 x_5^6 x_6^7 x_7^5 x_8^6 x_9^6$                                                                                    | 2                                                                                 |
| (7, 2, 1, 0)  | (0, 0, 1, 0, 0, 0, 1, 0, 0, 2) | 29  | $x_1 x_2^3 x_4^2 x_5^5 x_6^6 x_7^5 x_8^6 x_9^6$                                                                                      | $-1 \cdot 2$                                                                      |
| (7, 1, 1, 1)  | (0, 0, 1, 0, 0, 2, 0, 0, 3, 0) | 24  | $x_2^2 x_4^2 x_5^4 x_7^4 x_8^6 x_{10}^6$                                                                                             | 1                                                                                 |
| (7, 1, 2, 0)  | (0, 0, 2, 0, 0, 1, 0, 0, 2, 0) | 25  | $x_2^2 x_4^2 x_5^4 x_7^4 x_8^6 x_9 x_{10}^6$                                                                                         | 1                                                                                 |
| (7, 0, 3, 0)  | (0, 0, 0, 0, 2, 0, 0, 0, 2, 2) | 42  | $x_2^6 x_3^6 x_4^6 x_5^2 x_6^6 x_7^6 x_8^6 x_9^2 x_{10}^2$                                                                           | $-1 \cdot 2 \cdot 3 \cdot 7$                                                      |
| (6, 4, 0, 0)  | (0, 1, 0, 0, 1, 0, 0, 1, 0, 1) | 24  | $x_1 x_3 x_4^3 x_5^3 x_6^5 x_7^5 x_8^5 x_9^3 x_{10}^3$                                                                               | -1                                                                                |
| (6, 3, 0, 1)  | (0, 0, 1, 0, 0, 1, 0, 1, 0, 3) | 22  | $x_2^2 x_4^2 x_5^4 x_6^2 x_7^5 x_8^2 x_9^5$                                                                                          | 1                                                                                 |
| (6, 2, 0, 2)  | (0, 0, 1, 0, 0, 1, 0, 0, 3, 3) | 25  | $x_1 x_2^3 x_4^4 x_5^5 x_6^4 x_7^5 x_8^5 x_9 x_{10}$                                                                                 | $-1 \cdot 2$                                                                      |
| (6, 3, 1, 0)  | (0, 0, 1, 0, 1, 0, 0, 1, 0, 2) | 22  | $x_2^2 x_3 x_4^3 x_5^3 x_6^5 x_7^5 x_8^2 x_9^5$                                                                                      | 1                                                                                 |

$$S \subseteq \mathbb{Z}_p \times \mathbb{Z}_4 \setminus \{(0, 0)\}, |S| = 10$$

| $\lambda$    | $\mathbf{a}$                                                     | deg      | monomial/s                                                                                                                           | coefficient/s                                       |
|--------------|------------------------------------------------------------------|----------|--------------------------------------------------------------------------------------------------------------------------------------|-----------------------------------------------------|
| (6, 2, 1, 1) | (0, 0, 1, 0, 0, 2, 0, 3, 0, 1)                                   | 20       | $x_2^2 x_4^2 x_5^5 x_7^5 x_9^5 x_{10}$                                                                                               | 1                                                   |
| (6, 2, 2, 0) | (0, 0, 1, 0, 2, 0, 0, 2, 1, 0)                                   | 21       | $x_2^2 x_4^3 x_6^4 x_7^5 x_8 x_9 x_{10}^5$                                                                                           | -1                                                  |
| (6, 1, 2, 1) | (0, 1, 0, 0, 2, 0, 0, 3, 0, 2)                                   | 19       | $x_1 x_3 x_4^3 x_6^3 x_7^5 x_9^5 x_{10}$                                                                                             | -1                                                  |
| (6, 1, 3, 0) | (0, 0, 2, 0, 0, 1, 0, 2, 0, 2)                                   | 22       | $x_2^2 x_4^2 x_5^5 x_7^5 x_8 x_9^5 x_{10}^2$                                                                                         | 1                                                   |
| (6, 0, 4, 0) | (0, 0, 0, 2, 0, 0, 0, 2, 2, 2)                                   | 39       | $x_1^2 x_2^5 x_3^5 x_4^3 x_5^5 x_6^5 x_7^5 x_8^3 x_9^3 x_{10}^3$<br>$x_1^3 x_2^4 x_3^5 x_4^3 x_5^5 x_6^5 x_7^5 x_8^3 x_9^3 x_{10}^3$ | $2^4 \cdot 3 \cdot 11$<br>$2^4 \cdot 3 \cdot 13$    |
| (5, 5, 0, 0) | (0, 1, 0, 1, 0, 0, 1, 0, 1, 1)                                   | 25       | $x_2 x_3^2 x_4 x_5^2 x_6^4 x_7^3 x_8^4 x_9^4 x_{10}^4$                                                                               | 1                                                   |
| (5, 4, 0, 1) | (0, 0, 1, 0, 0, 1, 0, 1, 3, 1)                                   | 21       | $x_2^2 x_4^2 x_5^4 x_6^3 x_7^4 x_8^3 x_{10}^3$                                                                                       | 1                                                   |
| (5, 3, 0, 2) | (0, 0, 1, 0, 1, 0, 1, 0, 3, 3)                                   | 19       | $x_2^2 x_3 x_4^3 x_5 x_6^4 x_7^2 x_8^4 x_9 x_{10}$                                                                                   | -1                                                  |
| (5, 4, 1, 0) | (0, 0, 1, 0, 1, 0, 1, 0, 2, 1)                                   | 21       | $x_2^2 x_4^2 x_5^3 x_6^4 x_7^3 x_8^4 x_{10}^3$                                                                                       | 1                                                   |
| (5, 3, 1, 1) | (0, 1, 0, 0, 1, 0, 1, 0, 3, 2)                                   | 17       | $x_1 x_3 x_4^3 x_5^2 x_6^4 x_7^2 x_8^4$                                                                                              | -1                                                  |
| (5, 2, 1, 2) | (0, 0, 1, 0, 0, 2, 3, 0, 1, 3)                                   | 17       | $x_2^2 x_3 x_4^3 x_5^4 x_7 x_8^4 x_9 x_{10}$                                                                                         | $-1 \cdot 2$                                        |
| (5, 3, 2, 0) | (0, 0, 1, 0, 2, 0, 2, 1, 0, 1)                                   | 19       | $x_2^2 x_4^4 x_5 x_6^4 x_7 x_8 x_9^4 x_{10}^2$                                                                                       | -1                                                  |
| (5, 2, 2, 1) | (0, 0, 1, 0, 2, 0, 3, 0, 1, 2)                                   | 17       | $x_2^2 x_3 x_4^4 x_6^4 x_8^4 x_9 x_{10}$                                                                                             | 1                                                   |
| (5, 2, 3, 0) | (0, 1, 0, 2, 0, 0, 2, 1, 0, 2)                                   | 18       | $x_1 x_3 x_5^3 x_6^4 x_7^2 x_8 x_9^4 x_{10}^2$                                                                                       | $-1 \cdot 2$                                        |
| (5, 1, 3, 1) | (0, 0, 1, 0, 2, 0, 2, 2, 3, 0)                                   | 18       | $x_2^2 x_4^2 x_5^2 x_6^4 x_7^2 x_8^2 x_{10}^4$                                                                                       | 1                                                   |
| (5, 1, 4, 0) | (0, 0, 2, 0, 0, 1, 0, 2, 2, 2)                                   | 21       | $x_2^2 x_4^2 x_5^4 x_7^4 x_8^3 x_9^3 x_{10}^3$                                                                                       | -1                                                  |
| (5, 0, 5, 0) | (0, 0, 0, 2, 0, 0, 2, 2, 2, 2)<br>(0, 0, 0, 2, 0, 2, 2, 0, 2, 2) | 40<br>40 | $x_1^4 x_2^4 x_3^4 x_4^4 x_5^4 x_6^4 x_7^4 x_8^4 x_9^4 x_{10}^4$<br>$x_1^4 x_2^4 x_3^4 x_4^4 x_5^4 x_6^4 x_7^4 x_8^4 x_9^4 x_{10}^4$ | $2^2 \cdot 157$<br>$-1 \cdot 3^2 \cdot 5 \cdot 197$ |
| (4, 6, 0, 0) | (0, 1, 0, 1, 0, 1, 0, 1, 1, 1)                                   | 27       | $x_3 x_4^2 x_5^3 x_6^3 x_7^3 x_8^5 x_9^5 x_{10}^5$                                                                                   | 2                                                   |
| (4, 5, 0, 1) | (0, 1, 0, 0, 1, 0, 1, 3, 1, 1)                                   | 21       | $x_1 x_3 x_4^3 x_5 x_6^3 x_7^4 x_9^4 x_{10}^4$                                                                                       | -1                                                  |
| (4, 4, 0, 2) | (0, 0, 1, 0, 0, 1, 1, 3, 1, 3)                                   | 19       | $x_2^3 x_4^2 x_5^3 x_6^3 x_7^3 x_8 x_9^3 x_{10}$                                                                                     | 1                                                   |
| (4, 3, 0, 3) | (0, 1, 0, 1, 0, 1, 0, 3, 3, 3)                                   | 17       | $x_1 x_3 x_4 x_5^3 x_6^2 x_7^3 x_8^2 x_9^2 x_{10}^2$                                                                                 | 1                                                   |
| (4, 5, 1, 0) | (0, 0, 1, 0, 1, 0, 1, 2, 1, 1)                                   | 22       | $x_2^2 x_4^2 x_5^3 x_6^3 x_7^4 x_9^4 x_{10}^4$                                                                                       | 2                                                   |
| (4, 4, 1, 1) | (0, 0, 1, 0, 1, 0, 1, 3, 1, 2)                                   | 18       | $x_2^2 x_3 x_4^3 x_5^3 x_6^3 x_7^3 x_9^3$                                                                                            | 1                                                   |
| (4, 3, 1, 2) | (0, 0, 1, 0, 0, 2, 3, 1, 3, 1)                                   | 16       | $x_2^3 x_3^2 x_4^2 x_5^3 x_7 x_8^2 x_9 x_{10}^2$                                                                                     | 1                                                   |

$$S \subseteq \mathbb{Z}_p \times \mathbb{Z}_4 \setminus \{(0, 0)\}, |S| = 10$$

| $\lambda$    | $\mathbf{a}$                   | deg | monomial/s                                                       | coefficient/s   |
|--------------|--------------------------------|-----|------------------------------------------------------------------|-----------------|
| (4, 4, 2, 0) | (0, 1, 0, 1, 0, 1, 0, 2, 1, 2) | 18  | $x_1 x_3 x_4^2 x_5^3 x_6^3 x_7^3 x_8^3 x_9^3 x_{10}$             | -1              |
| (4, 3, 2, 1) | (0, 0, 1, 0, 2, 0, 2, 1, 1, 3) | 16  | $x_2^3 x_3 x_4^3 x_5 x_6^3 x_7 x_8^2 x_9^2$                      | $-1 \cdot 2$    |
| (4, 2, 2, 2) | (0, 1, 0, 0, 2, 3, 0, 1, 3, 2) | 14  | $x_1 x_2 x_3^2 x_4^3 x_6 x_7^3 x_8 x_9 x_{10}$                   | 2               |
| (4, 3, 3, 0) | (0, 0, 1, 1, 0, 0, 1, 2, 2, 2) | 18  | $x_2^3 x_3 x_4 x_5^2 x_6^3 x_7^2 x_8^2 x_9^2 x_{10}^2$           | -1              |
| (4, 2, 3, 1) | (0, 0, 1, 0, 2, 2, 2, 3, 0, 1) | 16  | $x_2^2 x_3 x_4^3 x_5^2 x_6^2 x_7^2 x_8^3 x_{10}$                 | $-1 \cdot 3$    |
| (4, 2, 4, 0) | (0, 0, 1, 2, 0, 2, 2, 2, 1, 0) | 19  | $x_2^3 x_3^3 x_4^3 x_7^3 x_8^3 x_9 x_{10}^3$                     | 2               |
| (4, 1, 4, 1) | (0, 1, 0, 2, 0, 2, 2, 3, 0, 2) | 17  | $x_1 x_3 x_3^3 x_6^3 x_7^3 x_8^3 x_{10}^3$                       | $-1 \cdot 3$    |
| (4, 1, 5, 0) | (0, 0, 2, 0, 0, 1, 2, 2, 2, 2) | 22  | $x_2^3 x_3 x_4^2 x_5^3 x_7 x_8^4 x_9^4 x_{10}^4$                 | -1              |
| (4, 0, 6, 0) | (0, 0, 2, 0, 0, 2, 2, 2, 2, 2) | 41  | $x_1^3 x_2^3 x_3^4 x_4^3 x_5^3 x_6^5 x_7^5 x_8^5 x_9^5 x_{10}^5$ | $2^3 \cdot 5^2$ |
| (3, 7, 0, 0) | (0, 1, 0, 1, 0, 1, 1, 1, 1, 1) | 31  | $x_3 x_4 x_5^2 x_6^3 x_7^6 x_8^6 x_9^6 x_{10}^6$                 | $-1 \cdot 2$    |
| (3, 6, 0, 1) | (0, 1, 0, 1, 0, 1, 3, 1, 1, 1) | 25  | $x_2 x_3^2 x_4 x_5^2 x_6^4 x_8^5 x_9^5 x_{10}^5$                 | 1               |
| (3, 5, 0, 2) | (0, 0, 1, 0, 1, 1, 3, 1, 3, 1) | 21  | $x_2^2 x_4^2 x_5^3 x_6^4 x_7 x_8^4 x_9 x_{10}^4$                 | 2               |
| (3, 4, 0, 3) | (0, 0, 1, 0, 1, 1, 3, 1, 3, 3) | 19  | $x_2^2 x_3^2 x_4^2 x_5 x_6^3 x_7^2 x_8^3 x_9^2 x_{10}^2$         | -1              |
| (3, 6, 1, 0) | (0, 1, 0, 1, 0, 1, 2, 1, 1, 1) | 24  | $x_1 x_3 x_4 x_5^2 x_6^4 x_8^5 x_9^5 x_{10}^5$                   | -1              |
| (3, 5, 1, 1) | (0, 0, 1, 0, 1, 1, 2, 1, 1, 3) | 20  | $x_2^2 x_3 x_4^2 x_5^3 x_6^4 x_8^4 x_9^4$                        | 1               |
| (3, 4, 1, 2) | (0, 1, 0, 0, 1, 1, 3, 1, 3, 2) | 16  | $x_1^2 x_3 x_4^2 x_5^3 x_6^3 x_7 x_8^3 x_9$                      | -1              |
| (3, 3, 1, 3) | (0, 0, 1, 0, 1, 1, 3, 3, 2, 3) | 16  | $x_2^2 x_3^2 x_4^2 x_5^2 x_6^2 x_7^2 x_8^2 x_{10}^2$             | 3               |
| (3, 5, 2, 0) | (0, 0, 1, 1, 0, 1, 2, 1, 1, 2) | 21  | $x_2^2 x_3 x_4^2 x_5^2 x_6^4 x_7 x_8^4 x_9^4 x_{10}$             | $-1 \cdot 2^2$  |
| (3, 4, 2, 1) | (0, 0, 1, 0, 2, 3, 1, 2, 1, 1) | 17  | $x_2^2 x_3^2 x_4^2 x_5 x_6^3 x_7 x_8^3 x_9^3 x_{10}^3$           | $-1 \cdot 2$    |
| (3, 3, 2, 2) | (0, 0, 1, 1, 0, 3, 2, 3, 1, 2) | 15  | $x_1 x_2^2 x_3^2 x_4^2 x_5^2 x_6 x_7 x_8 x_9^2 x_{10}$           | 1               |
| (3, 4, 3, 0) | (0, 0, 1, 1, 0, 1, 2, 2, 2, 1) | 19  | $x_2^2 x_4^3 x_5^2 x_6^3 x_7^2 x_8^2 x_9^2 x_{10}^3$             | -1              |
| (3, 3, 3, 1) | (0, 1, 0, 1, 0, 1, 2, 2, 3, 2) | 15  | $x_1 x_3^2 x_4^2 x_5^2 x_6^2 x_7^2 x_8^2 x_{10}^2$               | $-1 \cdot 3$    |
| (3, 2, 3, 2) | (0, 0, 1, 0, 2, 3, 1, 2, 2, 3) | 15  | $x_1 x_2^2 x_3 x_4^2 x_5^2 x_6 x_7 x_8^2 x_9^2 x_{10}$           | 2               |
| (3, 3, 4, 0) | (0, 0, 1, 2, 2, 1, 0, 1, 2, 2) | 19  | $x_2^2 x_3 x_4^2 x_5^3 x_6 x_7^2 x_8^2 x_9^2 x_{10}^3$           | $-1 \cdot 2$    |
| (3, 2, 4, 1) | (0, 0, 1, 2, 2, 2, 3, 0, 1, 2) | 17  | $x_1 x_2^2 x_3 x_4^2 x_5^2 x_6^3 x_8^2 x_9 x_{10}^3$             | $2^2$           |
| (3, 2, 5, 0) | (0, 1, 2, 0, 2, 2, 2, 1, 0, 2) | 20  | $x_1 x_4 x_3^3 x_6^4 x_7^4 x_8 x_9^2 x_{10}^4$                   | -1              |

$$S \subseteq \mathbb{Z}_p \times \mathbb{Z}_4 \setminus \{(0, 0)\}, |S| = 10$$

| $\lambda$    | $\mathbf{a}$                   | deg | monomial/s                                                 | coefficient/s            |
|--------------|--------------------------------|-----|------------------------------------------------------------|--------------------------|
| (3, 1, 5, 1) | (0, 0, 1, 2, 2, 2, 2, 2, 3, 0) | 20  | $x_2^2 x_4 x_5^3 x_6^4 x_7^4 x_8^4 x_{10}^2$               | 1                        |
| (3, 1, 6, 0) | (0, 0, 2, 0, 1, 2, 2, 2, 2, 2) | 25  | $x_2^2 x_4^2 x_6^2 x_7^4 x_8^5 x_9^5 x_{10}$               | 1                        |
| (3, 0, 7, 0) | (0, 0, 2, 0, 2, 2, 2, 2, 2, 2) | 46  | $x_2^2 x_3^6 x_4^2 x_5^6 x_6^6 x_7^6 x_8^6 x_9^6 x_{10}^6$ | $-1 \cdot 2^3 \cdot 3^2$ |
| (2, 8, 0, 0) | (1, 0, 1, 0, 1, 1, 1, 1, 1, 1) | 36  | $x_3 x_4 x_5^2 x_6^5 x_7^6 x_8^7 x_9^7 x_{10}^7$           | -1                       |
| (2, 7, 0, 1) | (0, 1, 0, 1, 1, 1, 1, 1, 1, 3) | 30  | $x_3 x_4^2 x_5^3 x_6^6 x_7^6 x_8^6 x_9^6$                  | $-1 \cdot 2$             |
| (2, 6, 0, 2) | (0, 1, 0, 1, 1, 3, 1, 3, 1, 1) | 24  | $x_1 x_3 x_4^2 x_5^3 x_6 x_7^5 x_8 x_9^5 x_{10}^5$         | $-1 \cdot 2$             |
| (2, 5, 0, 3) | (0, 1, 0, 1, 1, 1, 3, 3, 1, 3) | 22  | $x_3 x_4^3 x_5^4 x_6^4 x_7^2 x_8^2 x_9^4 x_{10}^2$         | 1                        |
| (2, 4, 0, 4) | (0, 1, 0, 1, 1, 3, 1, 3, 3, 3) | 20  | $x_1 x_3 x_4 x_5^2 x_6^3 x_7^3 x_8^3 x_9^3 x_{10}^3$       | -1                       |
| (2, 7, 1, 0) | (0, 1, 1, 0, 1, 1, 1, 1, 1, 2) | 30  | $x_2 x_3 x_4 x_5^3 x_6^6 x_7^6 x_8^6 x_9^6$                | $-1 \cdot 2$             |
| (2, 6, 1, 1) | (0, 1, 0, 1, 1, 1, 1, 2, 3, 1) | 24  | $x_3 x_4^3 x_5^5 x_6^5 x_7^5 x_{10}^5$                     | 1                        |
| (2, 5, 1, 2) | (0, 1, 0, 1, 1, 1, 2, 1, 3, 3) | 20  | $x_2^2 x_3 x_4^3 x_5^4 x_6^4 x_8^4 x_9 x_{10}$             | -1                       |
| (2, 4, 1, 3) | (0, 1, 0, 1, 1, 2, 3, 3, 3, 1) | 18  | $x_2^2 x_3 x_4^3 x_5^3 x_7^2 x_8^2 x_9^2 x_{10}^3$         | 3                        |
| (2, 6, 2, 0) | (0, 1, 0, 1, 1, 1, 2, 1, 2, 1) | 25  | $x_3 x_4^2 x_5^5 x_6^5 x_7 x_8^5 x_9 x_{10}^5$             | $-1 \cdot 2^2$           |
| (2, 5, 2, 1) | (0, 1, 0, 1, 1, 2, 1, 1, 3, 2) | 19  | $x_1 x_3 x_4^3 x_5^4 x_6 x_7^4 x_8^4 x_{10}$               | 3                        |
| (2, 4, 2, 2) | (0, 1, 0, 1, 1, 2, 3, 2, 1, 3) | 17  | $x_2^3 x_3 x_4^3 x_5^3 x_6 x_7 x_8 x_9^3 x_{10}$           | $-1 \cdot 2^3$           |
| (2, 3, 2, 3) | (0, 1, 0, 1, 1, 3, 3, 2, 3, 2) | 15  | $x_1 x_2 x_3 x_4^2 x_5^2 x_7^2 x_8 x_9^2 x_{10}$           | 3                        |
|              | (3, 0, 1, 1, 1, 0, 3, 2, 3, 2) | 15  | $x_1 x_2 x_3^2 x_4^2 x_5^2 x_6^2 x_7^2 x_8 x_9^2 x_{10}$   | 5                        |
| (2, 5, 3, 0) | (0, 1, 0, 1, 1, 1, 2, 1, 2, 2) | 22  | $x_3 x_4^3 x_5^4 x_6^4 x_7^2 x_8^4 x_9^2 x_{10}^2$         | 1                        |
| (2, 4, 3, 1) | (0, 1, 0, 1, 1, 3, 2, 2, 1, 2) | 18  | $x_2^2 x_3 x_4^3 x_5^3 x_7^2 x_8^2 x_9^3 x_{10}^2$         | 1                        |
| (2, 3, 3, 2) | (0, 1, 0, 1, 2, 2, 1, 3, 3, 2) | 16  | $x_1 x_2^2 x_3 x_4^2 x_5^2 x_6^2 x_7^2 x_8 x_9 x_{10}^2$   | 2                        |
| (2, 4, 4, 0) | (0, 1, 1, 0, 1, 2, 2, 2, 1, 2) | 20  | $x_1 x_3 x_4 x_5^2 x_6^3 x_7^3 x_8^3 x_9^3 x_{10}^3$       | 1                        |
| (2, 3, 4, 1) | (0, 1, 0, 1, 1, 2, 2, 3, 2, 2) | 18  | $x_2 x_3 x_4^2 x_5^2 x_6^3 x_7^3 x_9^3 x_{10}^3$           | $-1 \cdot 2 \cdot 3$     |
| (2, 2, 4, 2) | (0, 1, 0, 2, 3, 1, 2, 2, 3, 2) | 16  | $x_1 x_3 x_4^2 x_5 x_6 x_7^3 x_8^3 x_9 x_{10}^3$           | 2                        |
| (2, 3, 5, 0) | (0, 1, 1, 0, 2, 2, 1, 2, 2, 2) | 22  | $x_2 x_3 x_4 x_5^2 x_6^3 x_7^2 x_8^4 x_9^4 x_{10}^4$       | 1                        |
| (2, 2, 5, 1) | (0, 1, 0, 2, 2, 2, 3, 2, 2, 1) | 20  | $x_1 x_2 x_3 x_4^4 x_5^4 x_6^4 x_8^4 x_9$                  | -1                       |
| (2, 2, 6, 0) | (0, 1, 2, 0, 2, 2, 2, 1, 2, 2) | 25  | $x_4 x_5^3 x_6^5 x_7^5 x_8 x_9^5 x_{10}^5$                 | $-1 \cdot 5$             |

$$S \subseteq \mathbb{Z}_p \times \mathbb{Z}_4 \setminus \{(0, 0)\}, |S| = 10$$

| $\lambda$    | $\mathbf{a}$                   | deg | monomial/s                                                                                                           | coefficient/s                                      |
|--------------|--------------------------------|-----|----------------------------------------------------------------------------------------------------------------------|----------------------------------------------------|
| (2, 1, 6, 1) | (0, 1, 2, 2, 2, 2, 2, 3, 0, 2) | 23  | $x_1 x_4^2 x_5^4 x_6^5 x_7^5 x_9 x_{10}^5$                                                                           | -1                                                 |
| (2, 1, 7, 0) | (0, 2, 0, 2, 1, 2, 2, 2, 2, 2) | 30  | $x_3 x_4^3 x_6^3 x_7^5 x_8^6 x_9^6 x_{10}^6$                                                                         | 1                                                  |
| (2, 0, 8, 0) | (0, 2, 0, 2, 2, 2, 2, 2, 2, 2) | 51  | $x_1 x_3 x_4^7 x_5^7 x_6^7 x_7^7 x_8^7 x_9^7 x_{10}^7$<br>$x_1 x_2 x_3 x_4^6 x_5^7 x_6^7 x_7^7 x_8^7 x_9^7 x_{10}^7$ | $-1 \cdot 2 \cdot 17^2$<br>$-1 \cdot 2 \cdot 1277$ |
| (1, 9, 0, 0) | (1, 1, 0, 1, 1, 1, 1, 1, 1, 1) | 45  | $x_1 x_2 x_4^2 x_5^4 x_6^6 x_7^7 x_8^8 x_9^8 x_{10}^8$                                                               | 1                                                  |
| (1, 8, 0, 1) | (0, 1, 1, 1, 1, 1, 1, 1, 3, 1) | 37  | $x_3 x_4^3 x_5^5 x_6^7 x_7^7 x_8^7 x_{10}^7$                                                                         | -1                                                 |
| (1, 7, 0, 2) | (0, 1, 1, 1, 1, 1, 1, 1, 3, 3) | 31  | $x_2 x_3 x_4^3 x_5^6 x_6^6 x_7^6 x_8^6 x_9 x_{10}$                                                                   | 2                                                  |
| (1, 6, 0, 3) | (0, 1, 1, 1, 1, 3, 3, 3, 1, 1) | 27  | $x_3 x_4^5 x_5^5 x_6^2 x_7^2 x_8^2 x_9^5 x_{10}^5$                                                                   | $-1 \cdot 2^2$                                     |
| (1, 5, 0, 4) | (0, 1, 1, 1, 1, 3, 3, 1, 3, 3) | 25  | $x_2 x_3^2 x_4^3 x_5^4 x_6^2 x_7^3 x_8^4 x_9^3 x_{10}^3$                                                             | 2                                                  |
| (1, 8, 1, 0) | (0, 1, 1, 1, 1, 1, 1, 1, 2, 1) | 37  | $x_3^2 x_4^2 x_5^5 x_6^7 x_7^7 x_8^7 x_{10}^7$                                                                       | -1                                                 |
| (1, 7, 1, 1) | (1, 0, 1, 1, 1, 1, 1, 1, 3, 2) | 29  | $x_3^2 x_4^3 x_5^6 x_6^6 x_7^6 x_8^6$                                                                                | 2                                                  |
| (1, 6, 1, 2) | (0, 1, 1, 1, 1, 1, 2, 3, 1, 3) | 25  | $x_3^3 x_4^5 x_5^5 x_6^5 x_8 x_9^5 x_{10}$                                                                           | $-1 \cdot 3$                                       |
| (1, 5, 1, 3) | (1, 0, 1, 1, 1, 2, 1, 3, 3, 3) | 21  | $x_3^3 x_4^4 x_5^4 x_7^4 x_8^2 x_9^2 x_{10}^2$                                                                       | 1                                                  |
| (1, 4, 1, 4) | (0, 1, 1, 1, 2, 3, 3, 3, 1, 3) | 21  | $x_3^3 x_4^3 x_6^3 x_7^3 x_8^3 x_9^3 x_{10}^3$                                                                       | $-1 \cdot 3$                                       |
| (1, 7, 2, 0) | (0, 1, 1, 1, 1, 2, 1, 2, 1, 1) | 31  | $x_3^2 x_4^3 x_5^6 x_6^6 x_7^6 x_8^6 x_9^6 x_{10}^6$                                                                 | $-1 \cdot 2^2$                                     |
| (1, 6, 2, 1) | (0, 1, 1, 1, 1, 1, 2, 3, 1, 2) | 25  | $x_2 x_3^2 x_4^5 x_5^5 x_6^5 x_7^5 x_9^5 x_{10}$                                                                     | $-1 \cdot 3$                                       |
| (1, 5, 2, 2) | (0, 1, 1, 1, 1, 2, 1, 3, 3, 2) | 21  | $x_2 x_3^4 x_4^4 x_5^4 x_6 x_7^4 x_8 x_9 x_{10}$                                                                     | 2                                                  |
| (1, 4, 2, 3) | (0, 1, 1, 1, 2, 3, 2, 1, 3, 3) | 19  | $x_2^2 x_3^3 x_4^3 x_5^2 x_6^2 x_7^3 x_8^2 x_9^2 x_{10}^2$                                                           | $2 \cdot 3$                                        |
| (1, 6, 3, 0) | (1, 0, 1, 1, 1, 2, 1, 2, 1, 2) | 26  | $x_3 x_4^4 x_5^5 x_6^2 x_7^5 x_8^2 x_9^5 x_{10}^2$                                                                   | $2 \cdot 3$                                        |
| (1, 5, 3, 1) | (0, 1, 1, 1, 1, 1, 2, 2, 2, 3) | 22  | $x_2 x_3^3 x_4^4 x_5^4 x_6^4 x_7^2 x_8^2 x_9^2$                                                                      | $-1 \cdot 2$                                       |
| (1, 4, 3, 2) | (1, 0, 1, 1, 2, 1, 2, 3, 3, 2) | 18  | $x_1^2 x_3^2 x_4^3 x_5^2 x_6^3 x_7^2 x_8 x_9 x_{10}^2$                                                               | $-1 \cdot 2$                                       |
| (1, 3, 3, 3) | (0, 1, 1, 1, 2, 2, 2, 3, 3, 3) | 18  | $x_2^2 x_3^2 x_4^2 x_5^2 x_6^2 x_7^2 x_8^2 x_9^2 x_{10}^2$                                                           | -1                                                 |
| (1, 5, 4, 0) | (0, 1, 1, 1, 1, 2, 1, 2, 2, 2) | 25  | $x_2 x_3 x_4^3 x_5^4 x_6^3 x_7^4 x_8^3 x_9^3 x_{10}^3$                                                               | 1                                                  |
| (1, 4, 4, 1) | (0, 1, 1, 1, 2, 1, 2, 2, 3, 2) | 21  | $x_2 x_3^2 x_4^3 x_5^3 x_6^3 x_7^3 x_8^3 x_{10}^3$                                                                   | 1                                                  |
| (1, 3, 4, 2) | (0, 1, 1, 1, 2, 2, 3, 2, 2, 3) | 19  | $x_2 x_3^2 x_4^2 x_5^3 x_6^3 x_7^3 x_8^3 x_9^3 x_{10}$                                                               | $2^3$                                              |
| (1, 4, 5, 0) | (0, 1, 1, 1, 2, 2, 2, 1, 2, 2) | 25  | $x_3^2 x_4^2 x_5^2 x_6^4 x_7^4 x_8^3 x_9^4 x_{10}^4$                                                                 | 3                                                  |

$$S \subseteq \mathbb{Z}_p \times \mathbb{Z}_4 \setminus \{(0, 0)\}, |S| = 10$$

| $\lambda$     | $\mathbf{a}$                   | deg | monomial/s                                                                                           | coefficient/s                                         |
|---------------|--------------------------------|-----|------------------------------------------------------------------------------------------------------|-------------------------------------------------------|
| (1, 3, 5, 1)  | (1, 0, 1, 1, 2, 2, 3, 2, 2, 2) | 21  | $x_3x_4^2x_5^2x_6^4x_8^4x_9^4x_{10}^4$                                                               | -1                                                    |
| (1, 2, 5, 2)  | (0, 1, 2, 1, 2, 3, 2, 2, 2, 3) | 21  | $x_3^2x_4x_5^4x_6x_7^4x_8^4x_9^4x_{10}$                                                              | 1                                                     |
| (1, 3, 6, 0)  | (0, 1, 1, 2, 2, 1, 2, 2, 2, 2) | 27  | $x_3x_4^2x_5^3x_6^2x_7^4x_8^5x_9^5x_{10}^5$                                                          | 1                                                     |
| (1, 2, 6, 1)  | (0, 1, 2, 2, 2, 3, 2, 2, 1, 2) | 25  | $x_2x_4^3x_5^5x_7^5x_8^5x_9x_{10}^5$                                                                 | -1 · 2                                                |
| (1, 2, 7, 0)  | (1, 2, 0, 2, 2, 2, 1, 2, 2, 2) | 30  | $x_4^2x_5^4x_6^5x_7x_8^6x_9^6x_{10}^6$                                                               | -1                                                    |
| (1, 1, 7, 1)  | (0, 1, 2, 2, 2, 2, 2, 3, 2, 2) | 30  | $x_4^2x_5^4x_6^6x_7^6x_9^6x_{10}^6$                                                                  | -1 · 5                                                |
| (1, 1, 8, 0)  | (0, 2, 2, 2, 1, 2, 2, 2, 2, 2) | 37  | $x_3^3x_4^3x_6^4x_7^6x_8^7x_9^7x_{10}^7$                                                             | 1                                                     |
| (1, 0, 9, 0)  | (0, 2, 2, 2, 2, 2, 2, 2, 2, 2) | 60  | $x_2x_3^3x_4^8x_5^8x_6^8x_7^8x_8^8x_9^8x_{10}^8$<br>$x_2x_3^3x_4^7x_5^8x_6^8x_7^8x_8^8x_9^8x_{10}^8$ | -1 · 2 · 17 <sup>2</sup><br>-1 · 2 <sup>3</sup> · 283 |
| (0, 10, 0, 0) | (1, 1, 1, 1, 1, 1, 1, 1, 1, 1) | 55  | $x_1^2x_2^4x_3x_4^5x_5^8x_7^8x_8^9x_9^9x_{10}^9$                                                     | -1 · 2                                                |
| (0, 9, 0, 1)  | (1, 1, 1, 1, 1, 1, 1, 3, 1, 1) | 45  | $x_2x_3^3x_4^5x_5^5x_6^7x_7^8x_8^8x_{10}^8$                                                          | 1                                                     |
| (0, 8, 0, 2)  | (1, 1, 1, 1, 1, 3, 1, 1, 1, 3) | 39  | $x_2^2x_3^2x_4^5x_5^7x_6x_7^7x_8^7x_9^7x_{10}$                                                       | 2                                                     |
| (0, 7, 0, 3)  | (1, 1, 1, 1, 1, 1, 1, 3, 3, 3) | 33  | $x_2x_3^3x_4^5x_5^6x_6^6x_7^6x_8^2x_9^2x_{10}^2$                                                     | -1 · 2                                                |
| (0, 6, 0, 4)  | (1, 1, 1, 1, 1, 3, 3, 3, 1, 3) | 31  | $x_2^2x_3^2x_4^5x_5^5x_6^3x_7^3x_8^3x_9^5x_{10}^3$                                                   | -1 · 5                                                |
| (0, 5, 0, 5)  | (1, 1, 1, 1, 3, 3, 1, 3, 3, 3) | 29  | $x_2x_3^3x_4^4x_5x_6^4x_7^4x_8^4x_9^4x_{10}^4$                                                       | -1                                                    |
| (0, 9, 1, 0)  | (1, 1, 1, 1, 1, 1, 1, 1, 1, 2) | 46  | $x_1x_2x_3^3x_4^4x_5^6x_6^7x_7^8x_8^8x_9^8$                                                          | 2                                                     |
| (0, 8, 1, 1)  | (1, 1, 1, 1, 1, 1, 1, 3, 1, 2) | 38  | $x_1x_2x_3^3x_4^5x_5^7x_6^7x_7^7x_9^7$                                                               | -1 · 3                                                |
| (0, 7, 1, 2)  | (1, 1, 1, 1, 1, 1, 3, 1, 2, 3) | 32  | $x_2^2x_3^4x_4^6x_5^6x_6^6x_7x_8^6x_{10}$                                                            | -1 · 3                                                |
| (0, 6, 1, 3)  | (1, 1, 1, 1, 1, 2, 3, 1, 3, 3) | 28  | $x_1x_2x_3^5x_4^5x_5^5x_7^2x_8^5x_9^2x_{10}^2$                                                       | -1                                                    |
| (0, 5, 1, 4)  | (1, 1, 1, 1, 2, 3, 1, 3, 3, 3) | 26  | $x_2^2x_3^4x_4^4x_6^3x_7^4x_8^3x_9^3x_{10}^3$                                                        | 1                                                     |
| (0, 8, 2, 0)  | (1, 1, 1, 1, 1, 1, 1, 2, 1, 2) | 38  | $x_2x_3^2x_4^5x_5^7x_6^7x_7^7x_8^7x_9^7x_{10}$                                                       | -1                                                    |
| (0, 7, 2, 1)  | (1, 1, 1, 1, 1, 1, 1, 2, 3, 2) | 32  | $x_1x_2^2x_3^3x_4^6x_5^6x_6^6x_7^6x_8x_{10}$                                                         | 2                                                     |
| (0, 6, 2, 2)  | (1, 1, 1, 1, 1, 1, 3, 2, 3, 2) | 26  | $x_2^3x_3^4x_4^5x_5^5x_6^5x_7x_8x_9x_{10}$                                                           | -1 · 2                                                |
| (0, 5, 2, 3)  | (1, 1, 1, 1, 1, 2, 3, 2, 3, 3) | 24  | $x_1x_2^3x_3^4x_4^4x_5^4x_6x_7^2x_8x_9^2x_{10}^2$                                                    | 2 · 3                                                 |
| (0, 4, 2, 4)  | (1, 1, 1, 2, 3, 2, 1, 3, 3, 3) | 22  | $x_2^2x_3^3x_4x_5^3x_6x_7^3x_8^3x_9^3x_{10}^3$                                                       | 2 <sup>2</sup> · 3                                    |
| (0, 7, 3, 0)  | (1, 1, 1, 1, 1, 1, 2, 2, 1, 2) | 34  | $x_1x_2x_3^3x_4^5x_5^6x_6^6x_7^2x_8^2x_9^6x_{10}^2$                                                  | -1 · 3                                                |

$$S \subseteq \mathbb{Z}_p \times \mathbb{Z}_4 \setminus \{(0, 0)\}, |S| = 10$$

| $\lambda$     | $\mathbf{a}$                   | deg | monomial/s                                                       | coefficient/s           |
|---------------|--------------------------------|-----|------------------------------------------------------------------|-------------------------|
| (0, 6, 3, 1)  | (1, 1, 1, 1, 1, 1, 2, 2, 3, 2) | 28  | $x_2^3 x_3^4 x_4^5 x_5^5 x_6^2 x_7^2 x_8^2 x_{10}^2$             | $-1 \cdot 2$            |
| (0, 5, 3, 2)  | (1, 1, 1, 1, 2, 1, 2, 2, 3, 3) | 24  | $x_1^2 x_2^2 x_3^4 x_4^4 x_5^2 x_6^4 x_7^2 x_8^2 x_9 x_{10}$     | $-1 \cdot 2$            |
| (0, 4, 3, 3)  | (1, 1, 1, 2, 1, 2, 2, 3, 3, 3) | 22  | $x_1 x_2^3 x_3^3 x_4^2 x_5^3 x_6^2 x_7^2 x_8^2 x_9^2 x_{10}^2$   | $-1 \cdot 2^2$          |
| (0, 6, 4, 0)  | (1, 1, 1, 1, 1, 2, 2, 1, 2, 2) | 31  | $x_2^3 x_3^2 x_4^4 x_5^5 x_6^3 x_7^5 x_8^3 x_9^3 x_{10}^3$       | $-1 \cdot 2$            |
| (0, 5, 4, 1)  | (1, 1, 1, 1, 1, 2, 2, 2, 3, 2) | 25  | $x_1 x_2 x_3^3 x_4^4 x_5^4 x_6^3 x_7^3 x_8^3 x_{10}^3$           | $-1$                    |
| (0, 4, 4, 2)  | (1, 1, 1, 2, 1, 2, 3, 2, 2, 3) | 23  | $x_2^3 x_3^3 x_4^3 x_5^3 x_6^3 x_7^3 x_8^3 x_9^3 x_{10}$         | $-1 \cdot 2^2$          |
| (0, 3, 4, 3)  | (1, 1, 1, 2, 2, 2, 3, 3, 3, 2) | 21  | $x_2 x_3^2 x_4^3 x_5^3 x_6^3 x_7^2 x_8^2 x_9^2 x_{10}^3$         | 3                       |
| (0, 5, 5, 0)  | (1, 1, 1, 1, 2, 2, 1, 2, 2, 2) | 30  | $x_2 x_3^3 x_4^4 x_5^2 x_6^4 x_7^4 x_8^4 x_9^4 x_{10}^4$         | 3                       |
| (0, 4, 5, 1)  | (1, 1, 1, 2, 1, 2, 2, 2, 3, 2) | 26  | $x_1 x_2 x_3^2 x_4^3 x_5^3 x_6^4 x_7^4 x_8^4 x_{10}^4$           | $-1$                    |
| (0, 3, 5, 2)  | (1, 1, 2, 1, 2, 2, 2, 3, 2, 3) | 24  | $x_2 x_3^3 x_4^2 x_5^4 x_6^4 x_7^4 x_8^4 x_9^4 x_{10}$           | 1                       |
| (0, 4, 6, 0)  | (1, 1, 1, 2, 2, 2, 1, 2, 2, 2) | 30  | $x_2 x_3^2 x_4 x_5^3 x_6^5 x_7^5 x_8^5 x_9^5 x_{10}^5$           | $-1 \cdot 3$            |
| (0, 3, 6, 1)  | (1, 1, 1, 2, 2, 2, 2, 3, 2, 2) | 28  | $x_2^2 x_3^2 x_4 x_5^3 x_6^5 x_7^5 x_9^5 x_{10}^5$               | 5                       |
| (0, 2, 6, 2)  | (1, 1, 2, 2, 3, 2, 2, 2, 3, 2) | 26  | $x_2 x_3^2 x_4^2 x_5 x_6^4 x_7^5 x_8^5 x_9 x_{10}^5$             | 1                       |
| (0, 3, 7, 0)  | (1, 1, 2, 2, 2, 2, 1, 2, 2, 2) | 34  | $x_1 x_2 x_3 x_4^2 x_5^4 x_6^5 x_7^2 x_8^6 x_9^6 x_{10}^6$       | 1                       |
| (0, 2, 7, 1)  | (1, 1, 2, 2, 2, 2, 3, 2, 2, 2) | 32  | $x_2 x_3 x_4^2 x_5^4 x_6^6 x_8^6 x_9^6 x_{10}^6$                 | $-1$                    |
| (0, 2, 8, 0)  | (1, 2, 2, 2, 2, 1, 2, 2, 2, 2) | 39  | $x_3^2 x_4^3 x_5^6 x_6 x_7^6 x_8^7 x_9^7 x_{10}^7$               | 1                       |
| (0, 1, 8, 1)  | (1, 2, 2, 2, 2, 2, 3, 2, 2, 2) | 37  | $x_3^2 x_4^3 x_5^5 x_6^6 x_8^7 x_9^7 x_{10}^7$                   | $-1$                    |
| (0, 1, 9, 0)  | (2, 2, 2, 2, 1, 2, 2, 2, 2, 2) | 46  | $x_2^2 x_3^3 x_4^5 x_6^5 x_7^8 x_8^8 x_9^8 x_{10}^8$             | 1                       |
| (0, 0, 10, 0) | (2, 2, 2, 2, 2, 2, 2, 2, 2, 2) | 69  | $x_1^2 x_2^2 x_3^4 x_4^9 x_5^7 x_6^9 x_7^9 x_8^9 x_9^9 x_{10}^9$ | $2^5 \cdot 3^2 \cdot 5$ |

$$S \subseteq \mathbb{Z}_p \times \mathbb{Z}_5 \setminus \{(0, 0)\}, |S| = 10$$

| $\lambda$        | $\mathbf{a}$                   | deg | monomial/s                                                                                                                           | coefficient/s                                                                     |
|------------------|--------------------------------|-----|--------------------------------------------------------------------------------------------------------------------------------------|-----------------------------------------------------------------------------------|
| (10, 0, 0, 0, 0) | (0, 0, 0, 0, 0, 0, 0, 0, 0, 0) | 89  | $x_1^8 x_2^9 x_3^9 x_4^9 x_5^9 x_6^9 x_7^9 x_8^9 x_9^9 x_{10}^9$<br>$x_1^9 x_2^8 x_3^9 x_4^9 x_5^9 x_6^9 x_7^9 x_8^9 x_9^9 x_{10}^9$ | $2^5 \cdot 7 \cdot 11^2 \cdot 21966239$<br>$2 \cdot 13 \cdot 211 \cdot 256046627$ |
| (9, 1, 0, 0, 0)  | (0, 0, 0, 0, 0, 1, 0, 0, 0, 0) | 52  | $x_2^2 x_3^4 x_4^7 x_5^8 x_7^8 x_8^8 x_9^8 x_{10}^8$                                                                                 | $-1 \cdot 2^2$                                                                    |
| (8, 2, 0, 0, 0)  | (0, 0, 0, 1, 0, 0, 0, 1, 0, 0) | 36  | $x_1 x_2^3 x_3^6 x_5^5 x_6^7 x_8 x_9^6 x_{10}^7$                                                                                     | $-1$                                                                              |
| (8, 1, 1, 0, 0)  | (0, 0, 0, 1, 0, 0, 0, 2, 0, 0) | 35  | $x_1 x_2^3 x_3^6 x_5^5 x_6^7 x_9^6 x_{10}^7$                                                                                         | $-1$                                                                              |
| (8, 1, 0, 0, 1)  | (0, 0, 0, 0, 1, 0, 0, 0, 0, 4) | 44  | $x_1 x_2^3 x_3^6 x_4^7 x_6^6 x_7^7 x_8^7 x_9^7$                                                                                      | $-1 \cdot 2^2$                                                                    |

$$S \subseteq \mathbb{Z}_p \times \mathbb{Z}_5 \setminus \{(0, 0)\}, |S| = 10$$

| $\lambda$       | $\mathbf{a}$                   | deg | monomial/s                                         | coefficient/s |
|-----------------|--------------------------------|-----|----------------------------------------------------|---------------|
| (7, 3, 0, 0, 0) | (0, 0, 1, 0, 0, 1, 0, 0, 1, 0) | 27  | $x_1 x_2^3 x_4^3 x_5^5 x_6 x_8^6 x_9^2 x_{10}^6$   | 1             |
| (7, 2, 1, 0, 0) | (0, 0, 1, 0, 0, 1, 0, 0, 2, 0) | 25  | $x_1 x_2^3 x_4^3 x_5^5 x_6 x_8^6 x_{10}^6$         | 1             |
| (7, 2, 0, 1, 0) | (0, 0, 1, 0, 0, 0, 1, 0, 0, 3) | 29  | $x_1 x_2^3 x_4^2 x_5^5 x_6^6 x_7 x_8^5 x_9^6$      | $-1 \cdot 2$  |
| (7, 2, 0, 0, 1) | (0, 0, 0, 1, 0, 0, 1, 0, 0, 4) | 30  | $x_2^2 x_3^4 x_4 x_5^5 x_6^6 x_7 x_8^5 x_9^6$      | 2             |
| (7, 1, 1, 1, 0) | (0, 0, 2, 0, 0, 1, 0, 0, 3, 0) | 24  | $x_1 x_2^3 x_4^3 x_5^5 x_8^6 x_{10}^6$             | 1             |
| (6, 4, 0, 0, 0) | (0, 0, 1, 0, 1, 0, 1, 0, 1, 0) | 22  | $x_2^2 x_3 x_4^2 x_5^2 x_6^3 x_8^4 x_9^3 x_{10}^5$ | 1             |
| (6, 3, 1, 0, 0) | (0, 1, 0, 0, 1, 0, 0, 1, 0, 2) | 21  | $x_1 x_3 x_4^3 x_5 x_6^3 x_7^5 x_8^2 x_9^5$        | $-1$          |
| (6, 3, 0, 1, 0) | (0, 0, 1, 0, 1, 0, 0, 1, 0, 3) | 22  | $x_2^2 x_3 x_4^3 x_5 x_6^3 x_7^5 x_8^2 x_9^5$      | 1             |
| (6, 3, 0, 0, 1) | (0, 0, 1, 0, 0, 1, 0, 1, 0, 4) | 22  | $x_2^2 x_4^2 x_5^4 x_6^2 x_7^5 x_8^2 x_9^5$        | 1             |
| (6, 2, 2, 0, 0) | (0, 0, 2, 0, 1, 0, 1, 0, 2, 0) | 18  | $x_2^2 x_4^2 x_6^3 x_7 x_8^4 x_9 x_{10}^5$         | 1             |
| (6, 2, 1, 1, 0) | (0, 0, 1, 0, 2, 0, 1, 0, 3, 0) | 17  | $x_2^2 x_4^2 x_6^3 x_7 x_8^4 x_{10}^5$             | 1             |
| (6, 2, 1, 0, 1) | (0, 0, 1, 0, 1, 0, 2, 0, 4, 0) | 17  | $x_2^2 x_4^2 x_5 x_6^3 x_8^4 x_{10}^5$             | 1             |
| (6, 2, 0, 1, 1) | (0, 0, 1, 0, 0, 3, 0, 4, 0, 1) | 20  | $x_2^2 x_4^2 x_5^5 x_7^5 x_9^5 x_{10}$             | 1             |
| (6, 2, 0, 0, 2) | (0, 0, 1, 0, 0, 1, 0, 0, 4, 4) | 25  | $x_1 x_2^3 x_4^4 x_5^5 x_6 x_7^4 x_8^5 x_9 x_{10}$ | $-1 \cdot 2$  |
| (6, 1, 1, 1, 1) | (0, 1, 0, 0, 2, 0, 0, 4, 0, 3) | 18  | $x_1 x_3 x_4^3 x_6^3 x_7^5 x_9^5$                  | $-1$          |
| (5, 5, 0, 0, 0) | (0, 1, 0, 1, 0, 1, 0, 1, 0, 1) | 21  | $x_1^2 x_3^2 x_4 x_5^3 x_6^2 x_8^3 x_9^4 x_{10}^4$ | 1             |
| (5, 4, 1, 0, 0) | (0, 0, 1, 1, 0, 1, 0, 1, 0, 2) | 18  | $x_2^2 x_3 x_4 x_5^2 x_6^2 x_7^3 x_8^3 x_9^4$      | $-1$          |
| (5, 4, 0, 1, 0) | (0, 0, 1, 0, 1, 1, 0, 1, 0, 3) | 18  | $x_2^2 x_4^2 x_5^2 x_6^2 x_7^3 x_8^3 x_9^4$        | $-1$          |
| (5, 4, 0, 0, 1) | (0, 0, 1, 0, 1, 0, 1, 1, 0, 4) | 18  | $x_2^2 x_4^2 x_5 x_6^3 x_7^3 x_8^3 x_9^4$          | $-1$          |
| (5, 3, 2, 0, 0) | (0, 0, 1, 2, 0, 1, 0, 2, 1, 0) | 16  | $x_2^2 x_3^2 x_6 x_7^4 x_8 x_9^2 x_{10}^4$         | 1             |
| (5, 3, 1, 1, 0) | (0, 0, 1, 0, 1, 2, 0, 3, 1, 0) | 15  | $x_2^2 x_4^2 x_5 x_7^4 x_9^2 x_{10}^4$             | 1             |
| (5, 3, 1, 0, 1) | (0, 0, 1, 0, 1, 0, 2, 4, 0, 1) | 15  | $x_2^2 x_4^2 x_5 x_6^4 x_9^4 x_{10}^2$             | $-1$          |
| (5, 3, 0, 2, 0) | (0, 0, 1, 0, 3, 3, 0, 1, 0, 1) | 16  | $x_2^2 x_4^2 x_5 x_6^3 x_7 x_8 x_9^4 x_{10}^2$     | $-1$          |
| (5, 3, 0, 1, 1) | (0, 1, 0, 0, 1, 0, 1, 0, 4, 3) | 17  | $x_1 x_3 x_4^3 x_5^2 x_6^4 x_7^2 x_8^4$            | $-1$          |
| (5, 3, 0, 0, 2) | (0, 0, 1, 0, 1, 0, 1, 0, 4, 4) | 19  | $x_2^2 x_3 x_4^3 x_5 x_6^4 x_7^2 x_8^4 x_9 x_{10}$ | $-1$          |

$$S \subseteq \mathbb{Z}_p \times \mathbb{Z}_5 \setminus \{(0, 0)\}, |S| = 10$$

| $\lambda$       | $\mathbf{a}$                   | deg | monomial/s                                           | coefficient/s |
|-----------------|--------------------------------|-----|------------------------------------------------------|---------------|
| (5, 2, 2, 1, 0) | (0, 0, 1, 0, 2, 0, 1, 3, 0, 2) | 14  | $x_2^2 x_4^2 x_6^4 x_7 x_9^4 x_{10}$                 | -1            |
| (5, 2, 2, 0, 1) | (0, 1, 0, 1, 0, 2, 0, 4, 0, 2) | 13  | $x_1 x_3 x_4 x_5^2 x_7^3 x_9^4 x_{10}$               | -1            |
| (5, 2, 1, 1, 1) | (0, 0, 1, 1, 0, 2, 0, 4, 0, 3) | 13  | $x_2^2 x_3 x_4 x_5^2 x_7^3 x_9^4$                    | -1            |
| (5, 2, 1, 0, 2) | (0, 0, 1, 0, 1, 2, 0, 4, 0, 4) | 14  | $x_2^2 x_4^3 x_5 x_7^3 x_9^4 x_{10}$                 | -1            |
| (4, 6, 0, 0, 0) | (0, 1, 1, 0, 1, 0, 1, 0, 1, 1) | 24  | $x_2^2 x_3^2 x_4 x_5^4 x_6^2 x_8^3 x_9^5 x_{10}^5$   | 1             |
| (4, 5, 1, 0, 0) | (0, 0, 1, 1, 1, 0, 1, 0, 2, 1) | 19  | $x_2^2 x_4^2 x_5^2 x_6^2 x_7^4 x_8^3 x_{10}^4$       | -1            |
| (4, 5, 0, 1, 0) | (0, 0, 1, 0, 1, 1, 1, 0, 3, 1) | 19  | $x_2^2 x_4^2 x_5 x_6^3 x_7^4 x_8^3 x_{10}^4$         | -1            |
| (4, 5, 0, 0, 1) | (0, 0, 1, 0, 1, 0, 1, 1, 4, 1) | 19  | $x_2^2 x_4^2 x_5 x_6^3 x_7^4 x_8^3 x_{10}^4$         | 1             |
| (4, 4, 2, 0, 0) | (0, 0, 1, 1, 0, 1, 1, 0, 2, 2) | 16  | $x_2^2 x_4 x_5^2 x_6^3 x_7^3 x_8^3 x_9 x_{10}$       | -1            |
| (4, 4, 1, 1, 0) | (0, 0, 1, 0, 2, 1, 3, 0, 1, 1) | 15  | $x_2^2 x_4^2 x_6^2 x_8^3 x_9^3 x_{10}^3$             | -1            |
| (4, 4, 1, 0, 1) | (0, 1, 0, 1, 0, 1, 1, 0, 4, 2) | 14  | $x_1 x_3 x_4 x_5^2 x_6^3 x_7^3 x_8^3$                | 1             |
| (4, 4, 0, 2, 0) | (0, 1, 0, 1, 1, 0, 1, 0, 3, 3) | 15  | $x_1 x_3 x_4 x_5^2 x_6^2 x_7^3 x_8^3 x_9 x_{10}$     | -1            |
| (4, 4, 0, 1, 1) | (0, 0, 1, 1, 0, 1, 1, 0, 4, 3) | 15  | $x_2^2 x_3 x_4 x_5^2 x_6^3 x_7^3 x_8^3$              | 1             |
| (4, 4, 0, 0, 2) | (0, 0, 1, 0, 1, 1, 1, 0, 4, 4) | 16  | $x_2^2 x_4^2 x_5^2 x_6^2 x_7^3 x_8^3 x_9 x_{10}$     | -1            |
| (4, 3, 3, 0, 0) | (0, 0, 1, 1, 0, 2, 2, 2, 0, 1) | 15  | $x_2^2 x_4 x_5^2 x_6 x_7^2 x_8^2 x_9^3 x_{10}^2$     | -1            |
| (4, 3, 2, 1, 0) | (0, 1, 0, 1, 2, 0, 3, 1, 0, 2) | 12  | $x_1 x_3 x_4 x_6^3 x_8^2 x_9^3 x_{10}$               | -1            |
| (4, 3, 2, 0, 1) | (0, 0, 1, 1, 0, 2, 4, 0, 1, 2) | 13  | $x_2^2 x_3 x_4 x_5^3 x_8^3 x_9^2 x_{10}$             | 1             |
| (4, 3, 1, 2, 0) | (0, 0, 1, 1, 2, 0, 3, 1, 0, 3) | 13  | $x_2^2 x_3 x_4 x_6^2 x_7 x_8^2 x_9^3 x_{10}$         | -1            |
| (4, 3, 1, 1, 1) | (0, 0, 1, 0, 1, 2, 4, 0, 1, 3) | 12  | $x_2^2 x_4^3 x_5^2 x_8^3 x_9^2$                      | 2             |
| (4, 3, 1, 0, 2) | (0, 0, 1, 0, 1, 0, 2, 4, 1, 4) | 13  | $x_2^2 x_3 x_4 x_5^2 x_6^3 x_9^2 x_{10}$             | 1             |
| (4, 3, 0, 2, 1) | (0, 0, 1, 0, 3, 0, 3, 1, 4, 1) | 13  | $x_2^2 x_3^2 x_4^2 x_6^3 x_7 x_8 x_{10}^2$           | 1             |
| (4, 3, 0, 1, 2) | (0, 0, 1, 0, 3, 4, 4, 0, 1, 1) | 13  | $x_2^2 x_4^3 x_7 x_8^3 x_9^2 x_{10}^2$               | -1            |
| (4, 3, 0, 0, 3) | (0, 1, 0, 1, 0, 1, 0, 4, 4, 4) | 17  | $x_1 x_3 x_4 x_5^3 x_6^2 x_7^3 x_8^2 x_9^2 x_{10}^2$ | 1             |
| (4, 2, 2, 2, 0) | (0, 0, 1, 2, 0, 1, 2, 3, 3, 0) | 12  | $x_2^2 x_3^3 x_6 x_7 x_8 x_9 x_{10}^3$               | 1             |
| (4, 2, 2, 1, 1) | (0, 0, 1, 0, 2, 1, 3, 0, 2, 4) | 11  | $x_2^2 x_4^3 x_5 x_6 x_8^3 x_9$                      | 2             |
| (4, 2, 1, 1, 2) | (0, 1, 0, 1, 2, 0, 4, 0, 4, 3) | 10  | $x_1 x_3^2 x_4 x_6^2 x_8^3 x_9$                      | 1             |

$$S \subseteq \mathbb{Z}_p \times \mathbb{Z}_5 \setminus \{(0, 0)\}, |S| = 10$$

| $\lambda$       | $\mathbf{a}$                      | deg | monomial/s                                           | coefficient/s |
|-----------------|-----------------------------------|-----|------------------------------------------------------|---------------|
| (3, 7, 0, 0, 0) | (0, 1, 1, 1, 0, 1, 0, 1, 1, 1)    | 28  | $x_1 x_3^2 x_4^2 x_5^2 x_6^3 x_8^6 x_9^6 x_{10}^6$   | -1            |
| (3, 6, 1, 0, 0) | (0, 0, 1, 1, 1, 1, 0, 2, 1, 1)    | 22  | $x_2^2 x_4 x_5^3 x_6^4 x_7^2 x_9^5 x_{10}^5$         | -1            |
| (3, 6, 0, 1, 0) | (0, 0, 1, 0, 1, 1, 1, 1, 3, 1, 1) | 22  | $x_2^2 x_4^2 x_5 x_6^2 x_7^5 x_9^5 x_{10}^5$         | -1            |
| (3, 6, 0, 0, 1) | (0, 1, 0, 1, 0, 1, 1, 1, 4, 1, 1) | 21  | $x_1 x_3 x_4 x_5^2 x_6^2 x_7^4 x_9^5 x_{10}^5$       | -1            |
| (3, 5, 2, 0, 0) | (0, 0, 1, 1, 0, 1, 1, 2, 2, 1)    | 18  | $x_2^2 x_4 x_5^2 x_6^4 x_7^3 x_8 x_9 x_{10}^4$       | 1             |
| (3, 5, 1, 1, 0) | (0, 1, 0, 1, 1, 1, 0, 3, 1, 2)    | 16  | $x_1 x_3 x_4 x_5^3 x_6^4 x_7^2 x_9^4$                | 1             |
| (3, 5, 1, 0, 1) | (0, 0, 1, 1, 0, 1, 1, 1, 4, 1, 2) | 17  | $x_2^2 x_3 x_4 x_5^2 x_6^4 x_7^3 x_9^4$              | -1            |
| (3, 5, 0, 2, 0) | (0, 0, 1, 1, 1, 1, 0, 3, 1, 3)    | 18  | $x_2^2 x_3 x_4 x_5^2 x_6^4 x_7^2 x_8 x_9^4 x_{10}$   | -1            |
| (3, 5, 0, 1, 1) | (0, 0, 1, 0, 1, 1, 1, 1, 4, 1, 3) | 17  | $x_2^2 x_4^2 x_5^2 x_6^4 x_7^3 x_9^4$                | -1            |
| (3, 5, 0, 0, 2) | (0, 0, 1, 1, 4, 1, 1, 1, 0, 4)    | 18  | $x_2^2 x_4 x_5 x_6^3 x_7^4 x_8^4 x_9^2 x_{10}$       | -1            |
| (3, 4, 3, 0, 0) | (0, 1, 1, 0, 1, 1, 0, 2, 2, 2)    | 15  | $x_1 x_3 x_4 x_5^2 x_6^3 x_7^2 x_8 x_9^2 x_{10}^2$   | -1            |
| (3, 4, 2, 1, 0) | (0, 0, 1, 1, 1, 0, 1, 3, 2, 2)    | 14  | $x_2^2 x_3 x_4^2 x_5^2 x_6^2 x_7^3 x_9 x_{10}$       | 1             |
| (3, 4, 2, 0, 1) | (0, 0, 1, 1, 1, 1, 0, 2, 2, 4)    | 14  | $x_2^2 x_4^2 x_5^3 x_6^3 x_7^2 x_8 x_9$              | 1             |
| (3, 4, 1, 2, 0) | (0, 0, 1, 0, 2, 1, 3, 1, 1, 3)    | 14  | $x_2^2 x_4^2 x_6^3 x_8^3 x_9^3 x_{10}$               | 1             |
| (3, 4, 1, 1, 1) | (0, 0, 1, 0, 1, 2, 4, 1, 3, 1)    | 13  | $x_2^2 x_4^2 x_5^3 x_8^3 x_{10}^3$                   | 1             |
| (3, 4, 1, 0, 2) | (0, 0, 1, 1, 0, 4, 2, 1, 4, 1)    | 14  | $x_2^2 x_4^3 x_5^2 x_6 x_8^2 x_9 x_{10}^3$           | 2             |
| (3, 4, 0, 3, 0) | (0, 0, 1, 0, 3, 3, 1, 1, 3, 1)    | 16  | $x_2^2 x_4^2 x_6 x_7^3 x_8^3 x_9^2 x_{10}^3$         | -1            |
| (3, 4, 0, 2, 1) | (0, 0, 1, 0, 3, 3, 1, 4, 1, 1)    | 14  | $x_2^2 x_4^2 x_5 x_6 x_7^2 x_9^3 x_{10}^3$           | -1            |
| (3, 4, 0, 1, 2) | (0, 1, 0, 1, 1, 1, 0, 4, 4, 3)    | 13  | $x_1 x_3 x_4^2 x_5^2 x_6^3 x_7^2 x_8 x_9$            | 1             |
| (3, 4, 0, 0, 3) | (0, 0, 1, 1, 1, 1, 0, 4, 4, 4)    | 16  | $x_2^2 x_3 x_4 x_5^2 x_6^3 x_7^2 x_8 x_9^2 x_{10}^2$ | -1            |
| (3, 3, 3, 1, 0) | (0, 0, 1, 1, 2, 2, 2, 0, 1, 3)    | 13  | $x_2^2 x_4^2 x_5 x_6^2 x_7^2 x_8^2 x_9^2$            | 1             |
| (3, 3, 3, 0, 1) | (0, 0, 1, 1, 0, 2, 2, 2, 1, 4)    | 13  | $x_2^2 x_4^2 x_5^2 x_6 x_7^2 x_8^2 x_9^2$            | 1             |
| (3, 3, 2, 2, 0) | (0, 0, 1, 1, 2, 0, 3, 1, 3, 2)    | 12  | $x_2^2 x_3 x_4 x_5 x_6^2 x_7 x_8^2 x_9 x_{10}$       | 2             |
| (3, 3, 2, 1, 1) | (0, 0, 1, 0, 2, 1, 3, 1, 4, 2)    | 11  | $x_2^2 x_3 x_4^2 x_5 x_6^2 x_8^2 x_{10}$             | -1            |
| (3, 3, 2, 0, 2) | (0, 1, 0, 1, 0, 2, 4, 1, 4, 2)    | 11  | $x_1 x_2 x_3 x_4^2 x_5^2 x_8^2 x_9 x_{10}$           | -1            |

$$S \subseteq \mathbb{Z}_p \times \mathbb{Z}_5 \setminus \{(0, 0)\}, |S| = 10$$

| $\lambda$       | $\mathbf{a}$                   | deg | monomial/s                                           | coefficient/s |
|-----------------|--------------------------------|-----|------------------------------------------------------|---------------|
| (3, 3, 1, 2, 1) | (0, 1, 0, 1, 2, 4, 0, 1, 3, 3) | 10  | $x_1 x_3 x_4^2 x_7^2 x_8^2 x_9 x_{10}$               | 1             |
| (3, 3, 1, 1, 2) | (0, 0, 1, 1, 0, 2, 4, 1, 4, 3) | 11  | $x_2^2 x_3^2 x_4^2 x_5^2 x_8^2 x_9$                  | -1            |
| (3, 3, 1, 0, 3) | (0, 0, 1, 0, 1, 2, 4, 1, 4, 4) | 13  | $x_2^2 x_4^2 x_5^2 x_7 x_8^2 x_9^2 x_{10}^2$         | -1            |
| (3, 3, 0, 2, 2) | (0, 0, 1, 0, 3, 3, 1, 1, 4, 4) | 12  | $x_2^2 x_3 x_4^2 x_5 x_6 x_7 x_8^2 x_9 x_{10}$       | 1             |
| (3, 2, 2, 2, 1) | (0, 0, 1, 2, 1, 3, 0, 2, 4, 3) | 10  | $x_2^2 x_3 x_4 x_5 x_6 x_7^2 x_8 x_{10}$             | 2             |
| (2, 8, 0, 0, 0) | (0, 1, 1, 1, 1, 0, 1, 1, 1, 1) | 34  | $x_2 x_3^2 x_4^4 x_5^6 x_6^6 x_8^6 x_9^7 x_{10}^7$   | -1            |
| (2, 7, 1, 0, 0) | (0, 1, 0, 1, 1, 1, 1, 2, 1, 1) | 27  | $x_3 x_4 x_5^2 x_6^5 x_7^6 x_8^6 x_9^6 x_{10}^6$     | -1 · 2        |
| (2, 7, 0, 1, 0) | (0, 1, 0, 1, 1, 1, 3, 1, 1, 1) | 26  | $x_1 x_3 x_4 x_5^2 x_6^4 x_8^5 x_9^6 x_{10}^6$       | -1            |
| (2, 7, 0, 0, 1) | (0, 1, 1, 0, 1, 1, 4, 1, 1, 1) | 27  | $x_2 x_3 x_4 x_5^2 x_6^4 x_8^6 x_9^6 x_{10}^6$       | -1            |
| (2, 6, 2, 0, 0) | (0, 1, 1, 0, 1, 1, 2, 2, 1, 1) | 21  | $x_1 x_3 x_4 x_5^2 x_6^4 x_7 x_8 x_9^5 x_{10}^5$     | -1            |
| (2, 6, 1, 1, 0) | (0, 1, 0, 1, 1, 1, 3, 1, 1, 2) | 21  | $x_2^2 x_3 x_4 x_5^2 x_6^5 x_8^5 x_9^5$              | -1            |
| (2, 6, 1, 0, 1) | (0, 1, 0, 1, 1, 1, 4, 1, 2, 1) | 21  | $x_2^2 x_3 x_4^2 x_5^2 x_6^4 x_8^5 x_{10}^5$         | -1            |
| (2, 6, 0, 2, 0) | (0, 1, 0, 1, 1, 1, 3, 1, 3)    | 22  | $x_3 x_4^2 x_5^2 x_6^5 x_7^5 x_8^5 x_9^5 x_{10}$     | 1             |
| (2, 6, 0, 1, 1) | (0, 1, 0, 1, 1, 1, 4, 3, 1)    | 21  | $x_3 x_4 x_5^4 x_6^5 x_7^5 x_{10}^5$                 | 1             |
| (2, 6, 0, 0, 2) | (0, 1, 0, 1, 1, 1, 4, 4, 1, 1) | 22  | $x_3 x_4 x_5^3 x_6^5 x_7 x_8 x_9^5 x_{10}^5$         | 2             |
| (2, 5, 3, 0, 0) | (0, 1, 1, 0, 1, 1, 2, 2, 1, 2) | 19  | $x_2 x_3 x_4 x_5^2 x_6^4 x_7^2 x_8^2 x_9^4 x_{10}^2$ | 2             |
| (2, 5, 2, 1, 0) | (0, 1, 0, 1, 1, 1, 2, 2, 1, 3) | 17  | $x_3 x_4^2 x_5^4 x_6^4 x_7 x_8 x_9^4$                | -1 · 2        |
| (2, 5, 2, 0, 1) | (0, 1, 0, 1, 1, 1, 2, 1, 2, 4) | 17  | $x_3 x_4^2 x_5^4 x_6^4 x_7 x_8^4 x_9$                | -1            |
| (2, 5, 1, 2, 0) | (0, 1, 0, 1, 1, 1, 2, 3, 3, 1) | 17  | $x_2 x_3 x_4 x_5^4 x_6^4 x_8 x_9 x_{10}^4$           | 2             |
| (2, 5, 1, 1, 1) | (0, 1, 0, 1, 1, 1, 3, 1, 4, 2) | 16  | $x_3 x_4^4 x_5^3 x_6^4 x_8^4$                        | -1            |
| (2, 5, 1, 0, 2) | (0, 1, 1, 0, 1, 1, 4, 1, 2, 4) | 16  | $x_1 x_3 x_4 x_5^4 x_6^3 x_7 x_8^4 x_{10}$           | -1            |
| (2, 5, 0, 3, 0) | (0, 1, 0, 1, 1, 1, 3, 1, 3, 3) | 19  | $x_3 x_4^2 x_5^2 x_6^4 x_7^2 x_8^4 x_9^2 x_{10}^2$   | 1             |
| (2, 5, 0, 2, 1) | (0, 1, 0, 1, 1, 1, 4, 1, 3, 3) | 16  | $x_1 x_3 x_4 x_5^4 x_6^3 x_8^4 x_9 x_{10}$           | -1            |
| (2, 5, 0, 1, 2) | (0, 1, 0, 1, 1, 1, 4, 1, 3, 4) | 17  | $x_2^2 x_3 x_4 x_5^4 x_6^3 x_7 x_8^4 x_{10}$         | 1             |
| (2, 5, 0, 0, 3) | (0, 1, 0, 1, 1, 1, 4, 1, 4, 4) | 19  | $x_3 x_4^2 x_5^2 x_6^4 x_7^2 x_8^4 x_9^2 x_{10}^2$   | 1             |
| (2, 4, 4, 0, 0) | (0, 1, 1, 1, 1, 0, 2, 2, 2, 2) | 18  | $x_3^2 x_4^2 x_5^3 x_6 x_7 x_8^3 x_9^3 x_{10}^3$     | -1            |

$$S \subseteq \mathbb{Z}_p \times \mathbb{Z}_5 \setminus \{(0, 0)\}, |S| = 10$$

| $\lambda$       | $\mathbf{a}$                   | deg | monomial/s                                  | coefficient/s |
|-----------------|--------------------------------|-----|---------------------------------------------|---------------|
| (2, 4, 3, 1, 0) | (0, 1, 0, 1, 1, 1, 3, 2, 2, 2) | 15  | $x_3x_4^2x_5^3x_6^3x_8^2x_9^2x_{10}^2$      | 1             |
| (2, 4, 3, 0, 1) | (0, 1, 0, 2, 1, 1, 2, 1, 4, 2) | 15  | $x_3x_4x_5^3x_6^3x_7^2x_8^3x_{10}^2$        | 2             |
| (2, 4, 2, 2, 0) | (0, 1, 0, 1, 1, 2, 3, 1, 3, 2) | 14  | $x_3x_4^3x_5^3x_6x_7x_8^3x_9x_{10}$         | 2             |
| (2, 4, 2, 1, 1) | (0, 1, 0, 1, 1, 1, 3, 2, 4, 2) | 12  | $x_1x_3x_4^2x_5^3x_6^3x_8x_{10}$            | -1            |
| (2, 4, 2, 0, 2) | (0, 1, 0, 1, 1, 1, 4, 4, 2, 2) | 14  | $x_2^2x_3x_4^2x_5^2x_6^3x_7x_8x_9x_{10}$    | -1            |
| (2, 4, 1, 3, 0) | (0, 1, 0, 2, 1, 3, 1, 1, 3, 3) | 14  | $x_1x_3x_5x_6x_7^3x_8^3x_9^2x_{10}^2$       | -1            |
| (2, 4, 1, 2, 1) | (0, 1, 0, 1, 1, 1, 3, 2, 4, 3) | 13  | $x_2^2x_3x_4^2x_5^3x_6^3x_7x_{10}$          | 1             |
| (2, 4, 1, 1, 2) | (0, 1, 0, 1, 2, 1, 3, 1, 4, 4) | 13  | $x_2x_3x_4^3x_6^3x_8^3x_9x_{10}$            | 2             |
| (2, 4, 1, 0, 3) | (0, 1, 0, 1, 1, 1, 4, 4, 2, 4) | 15  | $x_3x_4^2x_5^3x_6^3x_7^2x_8^2x_{10}^2$      | -1 · 2        |
| (2, 4, 0, 3, 1) | (0, 1, 0, 1, 1, 1, 4, 3, 3, 3) | 15  | $x_3x_4^2x_5^3x_6^3x_8^2x_9^2x_{10}^2$      | 1             |
| (2, 4, 0, 2, 2) | (0, 1, 0, 1, 1, 1, 3, 4, 3, 4) | 14  | $x_2x_3x_4^2x_5^3x_6^3x_7x_8x_9x_{10}$      | -1 · 2        |
| (2, 4, 0, 1, 3) | (0, 1, 0, 3, 4, 4, 1, 4, 1, 1) | 15  | $x_2x_3x_6^2x_7^3x_8^2x_9^3x_{10}^3$        | 1             |
| (2, 4, 0, 0, 4) | (0, 1, 1, 1, 1, 0, 4, 4, 4, 4) | 17  | $x_1x_3x_4^2x_5^3x_6x_7x_8^2x_9^3x_{10}^3$  | -1            |
| (2, 3, 3, 2, 0) | (0, 1, 0, 2, 1, 3, 2, 3, 1, 2) | 12  | $x_1x_2x_3x_4x_5x_7^2x_8x_9^2x_{10}^2$      | -1            |
| (2, 3, 3, 1, 1) | (0, 1, 0, 2, 1, 3, 1, 4, 2, 2) | 12  | $x_1x_2^2x_3x_5^2x_7^2x_9^2x_{10}^2$        | 1             |
| (2, 3, 3, 0, 2) | (0, 1, 0, 1, 2, 2, 2, 1, 4, 4) | 13  | $x_3x_4^2x_5^2x_6^2x_7^2x_8^2x_9x_{10}$     | 1             |
| (2, 3, 2, 2, 1) | (3, 3, 1, 4, 2, 1, 0, 1, 0, 2) | 11  | $x_1x_2x_3^2x_5x_6x_7x_8^2x_9x_{10}$        | 1             |
| (2, 3, 2, 1, 2) | (0, 1, 1, 2, 0, 4, 3, 1, 4, 2) | 11  | $x_2^2x_3^2x_4x_5x_6x_8^2x_9x_{10}$         | 2             |
| (2, 3, 2, 0, 3) | (0, 1, 2, 4, 4, 4, 2, 1, 1, 0) | 13  | $x_2x_3x_4x_5^2x_6^2x_7x_8^2x_9^2x_{10}$    | -1 · 2        |
| (2, 3, 1, 2, 2) | (0, 2, 1, 1, 0, 4, 3, 1, 4, 3) | 11  | $x_3^2x_4^2x_5x_6x_7x_8^2x_9x_{10}$         | 1             |
| (2, 3, 1, 1, 3) | (0, 1, 2, 1, 0, 4, 4, 4, 1, 3) | 11  | $x_1x_4^2x_5x_6x_7^2x_8^2x_9^2$             | 1             |
| (2, 2, 2, 2, 2) | (0, 2, 0, 1, 3, 3, 4, 1, 2, 4) | 9   | $x_1x_3x_4x_5x_6x_7x_8x_9x_{10}$            | -1            |
| (1, 9, 0, 0, 0) | (1, 1, 1, 0, 1, 1, 1, 1, 1, 1) | 42  | $x_1x_2^2x_3^3x_5^5x_6^7x_8^8x_9^8x_{10}^8$ | 1             |
| (1, 8, 1, 0, 0) | (1, 1, 1, 1, 2, 1, 1, 1, 0, 1) | 33  | $x_1x_2^2x_3^4x_4^5x_6^7x_8^7x_{10}^7$      | 1             |
| (1, 8, 0, 1, 0) | (1, 1, 1, 1, 3, 1, 1, 1, 0, 1) | 34  | $x_1^2x_2^2x_3^3x_4^6x_6^7x_8^7x_{10}^7$    | 1             |

$$S \subseteq \mathbb{Z}_p \times \mathbb{Z}_5 \setminus \{(0, 0)\}, |S| = 10$$

| $\lambda$       | $\mathbf{a}$                   | deg | monomial/s                                       | coefficient/s |
|-----------------|--------------------------------|-----|--------------------------------------------------|---------------|
| (1, 8, 0, 0, 1) | (1, 1, 1, 1, 4, 1, 1, 1, 0, 1) | 34  | $x_1 x_2^3 x_3^3 x_4^6 x_6^7 x_8^7 x_{10}^7$     | 1             |
| (1, 7, 2, 0, 0) | (1, 1, 2, 2, 1, 1, 0, 1, 1, 1) | 28  | $x_1 x_2^3 x_4 x_5^3 x_6^3 x_8^5 x_9^6 x_{10}^6$ | 1             |
| (1, 7, 1, 1, 0) | (1, 1, 1, 1, 1, 1, 2, 1, 3, 0) | 27  | $x_2^3 x_3^2 x_4^4 x_5^6 x_6^6 x_8^6$            | -1            |
| (1, 7, 1, 0, 1) | (4, 1, 1, 1, 1, 1, 2, 0, 1, 1) | 27  | $x_2 x_3 x_4^2 x_5^5 x_6^6 x_9^6 x_{10}^6$       | -1 · 2        |
| (1, 7, 0, 2, 0) | (1, 1, 1, 1, 1, 1, 3, 0, 3, 1) | 28  | $x_2^2 x_3^3 x_4^3 x_5^6 x_6^6 x_7 x_9 x_{10}^6$ | 2             |
| (1, 7, 0, 1, 1) | (1, 3, 1, 1, 1, 1, 4, 1, 0, 1) | 27  | $x_1 x_2^3 x_4^3 x_5^3 x_6^6 x_8^6 x_{10}^6$     | 1             |
| (1, 7, 0, 0, 2) | (1, 1, 0, 1, 1, 4, 1, 1, 1, 4) | 27  | $x_2 x_4^2 x_5^4 x_6^6 x_7^6 x_8^6 x_9^6 x_{10}$ | -1            |
| (1, 6, 3, 0, 0) | (2, 1, 1, 1, 1, 2, 1, 2, 0, 1) | 24  | $x_1 x_3 x_4^3 x_5^5 x_6^2 x_7^5 x_8^2 x_{10}^5$ | 2             |
| (1, 6, 2, 1, 0) | (1, 1, 1, 3, 1, 2, 0, 1, 1, 2) | 22  | $x_2 x_3^5 x_4^4 x_5^6 x_8^5 x_9^5 x_{10}$       | 1             |
| (1, 6, 2, 0, 1) | (1, 2, 2, 1, 1, 0, 1, 1, 4, 1) | 22  | $x_1 x_3 x_4^2 x_5^3 x_7^5 x_8^5 x_{10}^5$       | 1             |
| (1, 6, 1, 2, 0) | (1, 1, 2, 1, 0, 3, 3, 1, 1, 1) | 22  | $x_2^2 x_4^5 x_7 x_8^4 x_9^5 x_{10}^5$           | -1            |
| (1, 6, 1, 1, 1) | (1, 2, 4, 1, 3, 1, 1, 1, 0, 1) | 20  | $x_4^3 x_6^3 x_7^5 x_8^4 x_{10}^5$               | 1             |
| (1, 6, 1, 0, 2) | (2, 1, 1, 4, 4, 1, 1, 1, 1, 0) | 22  | $x_2^2 x_4 x_5 x_6^4 x_7^4 x_8^5 x_9^5$          | 1             |
| (1, 6, 0, 3, 0) | (1, 1, 0, 1, 1, 1, 3, 3, 3, 1) | 23  | $x_2 x_4^2 x_5^5 x_6^5 x_7 x_8^2 x_9^2 x_{10}^5$ | 1             |
| (1, 6, 0, 2, 1) | (3, 1, 3, 0, 1, 1, 1, 1, 1, 4) | 22  | $x_2^2 x_3 x_5^2 x_6^3 x_7^4 x_8^5 x_9^5$        | -1            |
| (1, 6, 0, 1, 2) | (1, 4, 1, 1, 0, 1, 1, 4, 1, 3) | 22  | $x_2 x_3^2 x_4^4 x_6^5 x_7^4 x_8 x_9^5$          | 1             |
| (1, 6, 0, 0, 3) | (4, 0, 1, 1, 1, 1, 4, 4, 1, 1) | 24  | $x_3 x_4 x_5^3 x_6^5 x_7^2 x_8^2 x_9^5 x_{10}^5$ | 2             |
| (1, 5, 4, 0, 0) | (1, 2, 1, 2, 1, 0, 2, 1, 2, 1) | 22  | $x_2 x_3 x_4^2 x_5^4 x_7^3 x_8^4 x_9^3 x_{10}^4$ | 2             |
| (1, 5, 3, 1, 0) | (1, 2, 0, 1, 2, 1, 3, 2, 1, 1) | 19  | $x_4^3 x_5^2 x_6^4 x_8^2 x_9^4 x_{10}^4$         | 1             |
| (1, 5, 3, 0, 1) | (1, 2, 1, 1, 1, 2, 4, 0, 2, 1) | 18  | $x_2^2 x_4^4 x_5^4 x_6^2 x_9^2 x_{10}^4$         | -1            |
| (1, 5, 2, 2, 0) | (1, 2, 1, 0, 2, 1, 1, 1, 3, 3) | 17  | $x_3^4 x_5 x_6^2 x_7^4 x_8^4 x_9 x_{10}$         | 1             |
| (1, 5, 2, 1, 1) | (0, 2, 4, 1, 1, 1, 1, 3, 1, 2) | 17  | $x_2 x_4 x_5^3 x_6^3 x_7^4 x_9^4 x_{10}$         | -1            |
| (1, 5, 2, 0, 2) | (4, 1, 1, 2, 1, 0, 2, 1, 1, 4) | 18  | $x_2 x_3^2 x_4 x_5^4 x_7 x_8^4 x_9^4 x_{10}$     | 3             |
| (1, 5, 1, 3, 0) | (3, 1, 3, 1, 3, 0, 1, 2, 1, 1) | 19  | $x_3 x_4^4 x_5^2 x_7^4 x_9^4 x_{10}^4$           | 1             |
| (1, 5, 1, 2, 1) | (0, 1, 2, 1, 3, 1, 1, 3, 4, 1) | 17  | $x_4^3 x_5 x_6^4 x_7^4 x_8 x_{10}^4$             | -1            |
| (1, 5, 1, 1, 2) | (1, 1, 3, 4, 0, 1, 1, 2, 4, 1) | 17  | $x_1 x_2^2 x_4 x_6^4 x_7^4 x_9 x_{10}^4$         | 3             |

$$S \subseteq \mathbb{Z}_p \times \mathbb{Z}_5 \setminus \{(0, 0)\}, |S| = 10$$

| $\lambda$       | $\mathbf{a}$                   | deg | monomial/s                                           | coefficient/s       |
|-----------------|--------------------------------|-----|------------------------------------------------------|---------------------|
| (1, 5, 1, 0, 3) | (1, 4, 1, 1, 1, 4, 2, 4, 0, 1) | 19  | $x_1 x_2^2 x_3^2 x_4^2 x_5^4 x_6^2 x_8^2 x_{10}^4$   | -1 · 2              |
| (1, 5, 0, 4, 0) | (3, 1, 1, 3, 1, 3, 1, 3, 0, 1) | 22  | $x_3^2 x_4^2 x_5^4 x_6^3 x_7^4 x_8^3 x_{10}^4$       | -1 · 3              |
| (1, 5, 0, 3, 1) | (4, 1, 3, 3, 3, 1, 1, 1, 0, 1) | 19  | $x_2^2 x_3 x_4 x_5^2 x_6^3 x_7^3 x_8^3 x_{10}^4$     | -1                  |
| (1, 5, 0, 2, 2) | (1, 1, 4, 1, 3, 3, 1, 4, 1, 0) | 18  | $x_2^2 x_3 x_4^4 x_5 x_6 x_7^4 x_8 x_9^4$            | -1 · 2              |
| (1, 5, 0, 1, 3) | (4, 3, 4, 0, 1, 1, 1, 4, 1, 1) | 18  | $x_3^2 x_5 x_6 x_7^4 x_8^2 x_9^4 x_{10}^4$           | -1                  |
| (1, 5, 0, 0, 4) | (1, 1, 1, 1, 0, 4, 4, 4, 4, 1) | 22  | $x_1 x_2 x_3^2 x_4^4 x_6 x_7^3 x_8^3 x_9^3 x_{10}^4$ | 1                   |
| (1, 4, 4, 1, 0) | (1, 1, 3, 2, 1, 1, 0, 2, 2, 2) | 17  | $x_2^3 x_4 x_5^2 x_6^3 x_8^2 x_9^3 x_{10}^3$         | -1                  |
| (1, 4, 4, 0, 1) | (2, 0, 2, 1, 1, 2, 1, 4, 2, 1) | 18  | $x_3 x_4^2 x_5^3 x_6^3 x_7^3 x_9^3 x_{10}^3$         | 1                   |
| (1, 4, 3, 2, 0) | (0, 1, 2, 3, 1, 1, 1, 3, 2, 2) | 16  | $x_2 x_3 x_4 x_5^2 x_6^3 x_7^3 x_8 x_9^2 x_{10}^2$   | -1 · 2              |
| (1, 4, 3, 1, 1) | (1, 2, 2, 0, 1, 1, 2, 4, 1, 3) | 15  | $x_2^2 x_3^2 x_5^3 x_6^3 x_7^2 x_9^3$                | -1                  |
| (1, 4, 3, 0, 2) | (1, 2, 1, 1, 2, 4, 1, 2, 4, 0) | 16  | $x_2^2 x_3^2 x_4^3 x_5^2 x_6 x_7^3 x_8^2 x_9$        | -1 · 2              |
| (1, 4, 2, 3, 0) | (1, 2, 3, 1, 1, 2, 3, 1, 0, 3) | 16  | $x_2^2 x_4^3 x_5^3 x_6 x_7^2 x_8^3 x_{10}^2$         | -1 · 2              |
| (1, 4, 2, 2, 1) | (1, 0, 3, 3, 2, 1, 2, 1, 4, 1) | 14  | $x_1^3 x_4 x_5 x_6^2 x_7 x_8^3 x_{10}^3$             | -1                  |
| (1, 4, 2, 1, 2) | (1, 1, 2, 0, 4, 3, 1, 1, 2, 4) | 14  | $x_1 x_2^3 x_3 x_5 x_7^3 x_8^3 x_9 x_{10}$           | -1 · 2 <sup>2</sup> |
| (1, 4, 2, 0, 3) | (1, 0, 1, 1, 1, 4, 4, 2, 4, 2) | 15  | $x_3 x_4^3 x_5^3 x_6^2 x_7^2 x_8 x_9^2 x_{10}$       | 1                   |
| (1, 4, 1, 3, 1) | (0, 1, 1, 3, 2, 1, 3, 3, 4, 1) | 15  | $x_3^3 x_4^2 x_6^3 x_7^2 x_8^2 x_{10}^3$             | 1                   |
| (1, 4, 1, 2, 2) | (1, 1, 1, 3, 4, 3, 4, 2, 0, 1) | 13  | $x_2^3 x_3^3 x_4 x_5 x_6 x_7 x_{10}^3$               | 3                   |
| (1, 4, 1, 1, 3) | (1, 3, 0, 1, 1, 2, 4, 1, 4, 4) | 15  | $x_1 x_4^3 x_5^3 x_7 x_8^3 x_9^2 x_{10}^2$           | 1                   |
| (1, 4, 1, 0, 4) | (1, 4, 4, 1, 4, 2, 1, 1, 0, 4) | 18  | $x_2 x_3^2 x_4^3 x_5^3 x_7^3 x_8^3 x_{10}^3$         | -1 · 2 <sup>2</sup> |
| (1, 4, 0, 3, 2) | (0, 1, 3, 4, 1, 3, 1, 3, 1, 4) | 16  | $x_2^2 x_3^3 x_6^2 x_7^3 x_8^2 x_9^3 x_{10}$         | 1                   |
| (1, 4, 0, 2, 3) | (1, 1, 0, 3, 4, 4, 1, 4, 3, 1) | 16  | $x_2^3 x_4 x_5^2 x_6 x_7^3 x_8^2 x_9 x_{10}^3$       | 1                   |
| (1, 3, 3, 3, 0) | (0, 2, 1, 3, 3, 2, 3, 2, 1, 1) | 15  | $x_3 x_4^2 x_5^2 x_6^2 x_7^2 x_8^2 x_9^2 x_{10}^2$   | 1                   |
| (1, 3, 3, 2, 1) | (0, 2, 4, 2, 1, 1, 3, 3, 1, 2) | 13  | $x_2 x_4^2 x_5^2 x_6^2 x_7 x_8 x_9^2 x_{10}^2$       | 1                   |
| (1, 3, 3, 1, 2) | (1, 0, 3, 2, 1, 1, 4, 2, 4, 2) | 12  | $x_4^2 x_5^2 x_6^2 x_7 x_8^2 x_9 x_{10}^2$           | -1                  |
| (1, 3, 2, 2, 2) | (0, 4, 1, 1, 2, 4, 2, 3, 1, 3) | 12  | $x_2 x_3^2 x_4^2 x_5 x_6 x_7 x_8 x_9^2 x_{10}$       | 2 <sup>2</sup>      |

$$S \subseteq \mathbb{Z}_p \times \mathbb{Z}_5 \setminus \{(0, 0)\}, |S| = 10$$

| $\lambda$        | $\mathbf{a}$                      | deg | monomial/s                                                 | coefficient/s  |
|------------------|-----------------------------------|-----|------------------------------------------------------------|----------------|
| (1, 3, 2, 1, 3)  | (0, 4, 4, 1, 2, 4, 2, 1, 3, 1)    | 13  | $x_2^2 x_3 x_4^2 x_5 x_6^2 x_7 x_8^2 x_{10}^2$             | $-1 \cdot 2^2$ |
| (0, 10, 0, 0, 0) | (1, 1, 1, 1, 1, 1, 1, 1, 1, 1)    | 51  | $x_1 x_2^2 x_3^3 x_4^4 x_5^7 x_6^8 x_8^8 x_9^9 x_{10}^9$   | -1             |
| (0, 9, 1, 0, 0)  | (1, 1, 1, 1, 2, 1, 1, 1, 1, 1)    | 43  | $x_1^2 x_2^2 x_3^3 x_4^6 x_7^7 x_8^8 x_9^8 x_{10}^8$       | -1             |
| (0, 9, 0, 1, 0)  | (3, 1, 1, 1, 1, 1, 1, 1, 1, 1)    | 43  | $x_2 x_3^3 x_4^5 x_5^7 x_8^8 x_9^8 x_{10}^8$               | 1              |
| (0, 9, 0, 0, 1)  | (1, 1, 1, 1, 4, 1, 1, 1, 1, 1)    | 43  | $x_1 x_2^2 x_3^4 x_4^6 x_7^7 x_8^8 x_9^8 x_{10}^8$         | -1             |
| (0, 8, 2, 0, 0)  | (1, 1, 1, 1, 1, 1, 2, 1, 2, 1)    | 36  | $x_2^2 x_3^2 x_4^3 x_5^7 x_6^7 x_8^7 x_9 x_{10}^7$         | 1              |
| (0, 8, 1, 1, 0)  | (2, 1, 1, 1, 1, 3, 1, 1, 1, 1)    | 35  | $x_2^2 x_3^2 x_4^4 x_5^7 x_8^6 x_9^7 x_{10}^7$             | -1             |
| (0, 8, 1, 0, 1)  | (1, 1, 1, 2, 1, 1, 1, 1, 1, 4, 1) | 35  | $x_1 x_2^2 x_3^4 x_5^7 x_6^7 x_8^7 x_{10}^7$               | -1             |
| (0, 8, 0, 2, 0)  | (1, 1, 1, 3, 1, 1, 1, 1, 1, 3)    | 36  | $x_1 x_2^2 x_3^5 x_4^5 x_6^7 x_8^7 x_9^7 x_{10}$           | -1             |
| (0, 8, 0, 1, 1)  | (1, 1, 1, 1, 4, 3, 1, 1, 1, 1)    | 34  | $x_1 x_2^2 x_3^3 x_4^7 x_8^7 x_9^7 x_{10}^7$               | 1              |
| (0, 8, 0, 0, 2)  | (1, 1, 1, 1, 4, 4, 1, 1, 1, 1)    | 36  | $x_1^2 x_2^2 x_3^3 x_4^7 x_5 x_6 x_8^6 x_9^7 x_{10}^7$     | 1              |
| (0, 7, 3, 0, 0)  | (2, 2, 1, 1, 1, 1, 1, 2, 1, 1)    | 31  | $x_2 x_3 x_4 x_5^3 x_6^5 x_7^6 x_8^2 x_9^6 x_{10}^6$       | $-1 \cdot 2$   |
| (0, 7, 2, 1, 0)  | (1, 2, 1, 3, 1, 2, 1, 1, 1, 1)    | 29  | $x_3^2 x_5^4 x_6 x_7^4 x_8^6 x_9^6 x_{10}^6$               | -1             |
| (0, 7, 2, 0, 1)  | (4, 2, 1, 1, 1, 1, 1, 1, 1, 2)    | 28  | $x_4^2 x_5^3 x_6^5 x_7^5 x_8^6 x_9^6 x_{10}$               | 1              |
| (0, 7, 1, 2, 0)  | (1, 3, 1, 2, 1, 3, 1, 1, 1, 1)    | 28  | $x_3^3 x_5^3 x_6 x_7^4 x_8^5 x_9^6 x_{10}^6$               | -1             |
| (0, 7, 1, 1, 1)  | (1, 1, 1, 1, 3, 1, 4, 2, 1, 1)    | 28  | $x_1 x_2 x_3^2 x_4^6 x_6^6 x_9^6 x_{10}^6$                 | 1              |
| (0, 7, 1, 0, 2)  | (1, 2, 1, 1, 4, 1, 1, 1, 1, 4)    | 29  | $x_3 x_4^4 x_5 x_6^5 x_7^5 x_8^6 x_9^6 x_{10}$             | -1             |
| (0, 7, 0, 3, 0)  | (3, 1, 3, 1, 1, 1, 1, 1, 3, 1)    | 31  | $x_3^2 x_4^2 x_5^3 x_6^4 x_7^6 x_8^6 x_9^2 x_{10}^6$       | 1              |
| (0, 7, 0, 2, 1)  | (1, 3, 1, 1, 1, 1, 1, 4, 3, 1)    | 29  | $x_3^2 x_4^3 x_5^5 x_6^6 x_7 x_9 x_{10}^6$                 | 1              |
| (0, 7, 0, 1, 2)  | (1, 3, 4, 1, 1, 1, 1, 1, 4, 1)    | 29  | $x_3 x_4^2 x_5^3 x_6^4 x_7^6 x_8^6 x_9 x_{10}^6$           | -1             |
| (0, 7, 0, 0, 3)  | (4, 1, 1, 1, 4, 1, 1, 4, 1, 1)    | 31  | $x_1 x_2 x_3 x_4^2 x_5^2 x_6^4 x_7^6 x_8^2 x_9^6 x_{10}^6$ | -1             |
| (0, 6, 4, 0, 0)  | (1, 1, 1, 2, 2, 1, 1, 2, 2, 1)    | 28  | $x_2 x_3^2 x_4 x_5^3 x_6^5 x_7^5 x_8^3 x_9^3 x_{10}^5$     | 2              |
| (0, 6, 3, 1, 0)  | (1, 1, 1, 1, 3, 1, 1, 2, 2, 2)    | 24  | $x_2 x_3^2 x_4^5 x_6^5 x_7^5 x_8^2 x_9^2 x_{10}^2$         | -1             |
| (0, 6, 3, 0, 1)  | (2, 1, 1, 1, 1, 1, 2, 4, 2, 1)    | 25  | $x_3 x_4^5 x_5^5 x_6^5 x_7^2 x_9^2 x_{10}^5$               | 2              |
| (0, 6, 2, 2, 0)  | (1, 1, 1, 2, 3, 1, 3, 2, 1, 1)    | 24  | $x_1 x_2 x_3^3 x_4 x_5 x_6^5 x_7 x_8 x_9^5 x_{10}^5$       | 2              |
| (0, 6, 2, 1, 1)  | (2, 1, 1, 1, 1, 3, 4, 2, 1, 1)    | 23  | $x_1 x_2 x_3 x_4^4 x_5^5 x_8 x_9^5 x_{10}^5$               | 1              |

$$S \subseteq \mathbb{Z}_p \times \mathbb{Z}_5 \setminus \{(0, 0)\}, |S| = 10$$

| $\lambda$       | $\mathbf{a}$                   | deg | monomial/s                                               | coefficient/s |
|-----------------|--------------------------------|-----|----------------------------------------------------------|---------------|
| (0, 6, 2, 0, 2) | (1, 2, 4, 1, 1, 1, 1, 1, 2, 4) | 24  | $x_1 x_2 x_4^3 x_5^3 x_6^4 x_7^5 x_8^5 x_9 x_{10}$       | 1             |
| (0, 6, 1, 3, 0) | (1, 1, 1, 1, 1, 3, 1, 2, 3, 3) | 25  | $x_2^2 x_3^3 x_4^4 x_5^5 x_6^2 x_7^5 x_9^2 x_{10}^2$     | -1            |
| (0, 6, 1, 2, 1) | (1, 1, 4, 2, 1, 3, 1, 1, 1, 3) | 23  | $x_2^3 x_3^3 x_6 x_7^5 x_8^5 x_9^5 x_{10}$               | 1             |
| (0, 6, 1, 1, 2) | (1, 1, 1, 1, 3, 1, 2, 1, 4, 4) | 23  | $x_1 x_2 x_3^4 x_4^5 x_6^5 x_8^5 x_9 x_{10}$             | 1             |
| (0, 6, 1, 0, 3) | (2, 1, 1, 4, 1, 1, 1, 1, 4, 4) | 24  | $x_3 x_4^2 x_5^3 x_6^4 x_7^5 x_8^5 x_9^2 x_{10}^2$       | -1            |
| (0, 6, 0, 4, 0) | (1, 3, 3, 3, 3, 1, 1, 1, 1, 1) | 28  | $x_1 x_3 x_4^3 x_5^3 x_6^2 x_7^4 x_8^4 x_9^5 x_{10}^5$   | -1            |
| (0, 6, 0, 3, 1) | (1, 1, 1, 4, 1, 3, 3, 1, 3, 1) | 25  | $x_2 x_3^4 x_4^4 x_5^2 x_6^2 x_7^5 x_8^2 x_9^5 x_{10}^5$ | 1             |
| (0, 6, 0, 2, 2) | (1, 3, 4, 4, 1, 1, 1, 1, 1, 3) | 23  | $x_1 x_4 x_5^2 x_6^3 x_7^5 x_8^5 x_9^5 x_{10}$           | 1             |
| (0, 6, 0, 1, 3) | (4, 1, 4, 1, 1, 1, 1, 4, 1, 3) | 25  | $x_2 x_3^2 x_4^3 x_5^3 x_6^4 x_7^4 x_8^2 x_9^5$          | -1            |
| (0, 6, 0, 0, 4) | (4, 1, 1, 1, 4, 1, 1, 1, 4, 4) | 28  | $x_2 x_3 x_4^3 x_5^3 x_6^5 x_7^4 x_8^5 x_9^3 x_{10}^3$   | 1             |
| (0, 5, 5, 0, 0) | (1, 2, 2, 2, 1, 1, 2, 1, 2, 1) | 26  | $x_3^3 x_4^2 x_5^2 x_6^3 x_7^4 x_8^4 x_9^4 x_{10}^4$     | -1            |
| (0, 5, 4, 1, 0) | (2, 2, 2, 1, 1, 3, 2, 1, 1, 1) | 23  | $x_2^2 x_3^3 x_4 x_5^3 x_7^3 x_8^4 x_9^4 x_{10}^4$       | -1            |
| (0, 5, 4, 0, 1) | (2, 1, 1, 2, 4, 1, 2, 1, 2, 1) | 23  | $x_1 x_3 x_4^3 x_6^4 x_7^3 x_8^4 x_9^3 x_{10}^4$         | 3             |
| (0, 5, 3, 2, 0) | (3, 3, 1, 2, 1, 2, 1, 1, 2, 1) | 21  | $x_2 x_3 x_5^3 x_6^2 x_7^4 x_8^4 x_9^2 x_{10}^4$         | 2             |
| (0, 5, 3, 1, 1) | (2, 1, 1, 2, 1, 4, 3, 1, 2, 1) | 20  | $x_2 x_3^3 x_4^2 x_5^4 x_8^4 x_9^2 x_{10}^4$             | -1            |
| (0, 5, 3, 0, 2) | (1, 1, 1, 4, 2, 1, 2, 4, 2, 1) | 21  | $x_2 x_3^4 x_4 x_5^2 x_6^4 x_7^2 x_8 x_9^2 x_{10}^4$     | $3^2$         |
| (0, 5, 2, 3, 0) | (1, 3, 1, 2, 1, 1, 3, 3, 1, 2) | 21  | $x_2 x_3^2 x_4 x_5^4 x_6^4 x_7^2 x_8^2 x_9^4 x_{10}$     | 1             |
| (0, 5, 2, 2, 1) | (1, 1, 1, 2, 3, 1, 2, 1, 4, 3) | 19  | $x_2^3 x_3^4 x_4 x_5 x_6^4 x_7 x_8^4 x_{10}$             | -1            |
| (0, 5, 2, 1, 2) | (2, 1, 1, 4, 3, 4, 1, 1, 2, 1) | 18  | $x_3^3 x_4 x_6 x_7^4 x_8^4 x_9 x_{10}^4$                 | -1            |
| (0, 5, 2, 0, 3) | (1, 1, 1, 4, 2, 4, 4, 2, 1, 1) | 21  | $x_1 x_2 x_3^3 x_4^2 x_5 x_6^2 x_7^2 x_8 x_9^4 x_{10}^4$ | -1            |
| (0, 5, 1, 4, 0) | (1, 3, 3, 2, 1, 3, 3, 1, 1, 1) | 23  | $x_2 x_3^3 x_5^3 x_6^2 x_7^3 x_8^3 x_9^4 x_{10}^4$       | 1             |
| (0, 5, 1, 3, 1) | (4, 1, 1, 3, 3, 1, 3, 1, 1, 2) | 19  | $x_2^2 x_3 x_4 x_5 x_6^4 x_7^2 x_8^4 x_9^4$              | 1             |
| (0, 5, 1, 2, 2) | (3, 1, 3, 1, 1, 1, 4, 2, 1, 4) | 19  | $x_3 x_4^4 x_5^4 x_6^4 x_7 x_9^4 x_{10}$                 | 1             |
| (0, 5, 1, 1, 3) | (4, 1, 2, 1, 1, 4, 3, 1, 4, 1) | 20  | $x_2^2 x_4^2 x_5^4 x_6^2 x_8^4 x_9^2 x_{10}^4$           | $-1 \cdot 2$  |
| (0, 5, 1, 0, 4) | (1, 4, 4, 1, 4, 2, 1, 1, 4, 1) | 23  | $x_2 x_3 x_4^4 x_5^3 x_7^4 x_8^3 x_9^3 x_{10}^4$         | 2             |

$$S \subseteq \mathbb{Z}_p \times \mathbb{Z}_5 \setminus \{(0, 0)\}, |S| = 10$$

| $\lambda$       | $\mathbf{a}$                   | deg | monomial/s                                                 | coefficient/s  |
|-----------------|--------------------------------|-----|------------------------------------------------------------|----------------|
| (0, 5, 0, 4, 1) | (4, 3, 3, 1, 1, 1, 3, 1, 3)    | 23  | $x_3^2 x_4 x_5^2 x_6^4 x_7^3 x_8^4 x_9^3 x_{10}^3$         | 2              |
| (0, 5, 0, 3, 2) | (1, 3, 1, 1, 3, 4, 4, 1, 1, 3) | 21  | $x_3^4 x_4^4 x_5^2 x_7 x_8^4 x_9^4 x_{10}^2$               | 2              |
| (0, 5, 0, 2, 3) | (4, 1, 1, 1, 4, 1, 1, 3, 3, 4) | 21  | $x_1^2 x_2 x_3^2 x_4^2 x_5^4 x_6^4 x_7^4 x_8 x_9 x_{10}^2$ | $-1 \cdot 2$   |
| (0, 5, 0, 1, 4) | (1, 4, 1, 3, 4, 4, 4, 1, 1, 1) | 23  | $x_2^2 x_3^4 x_5 x_6^2 x_7^3 x_8^3 x_9^4 x_{10}^4$         | 1              |
| (0, 5, 0, 0, 5) | (4, 4, 4, 4, 1, 4, 1, 1, 1, 1) | 26  | $x_2 x_3^2 x_4^3 x_5^2 x_6^4 x_7^3 x_8^3 x_9^4 x_{10}^4$   | 1              |
| (0, 4, 4, 2, 0) | (2, 1, 3, 3, 2, 2, 1, 1, 2, 1) | 20  | $x_2 x_4 x_5^3 x_6^3 x_7^3 x_8^3 x_9^3 x_{10}^3$           | 1              |
| (0, 4, 4, 1, 1) | (1, 1, 1, 3, 2, 2, 4, 1, 2, 2) | 19  | $x_2^2 x_3^3 x_5^2 x_6^3 x_8^3 x_9^3 x_{10}^3$             | 2              |
| (0, 4, 4, 0, 2) | (2, 4, 1, 2, 2, 2, 1, 4, 1, 1) | 19  | $x_3 x_4^2 x_5^3 x_6^3 x_7^3 x_8 x_9^3 x_{10}^3$           | $-1$           |
| (0, 4, 3, 3, 0) | (1, 3, 3, 1, 3, 2, 2, 2, 1, 1) | 19  | $x_2 x_3 x_4^3 x_5^2 x_6^2 x_7^2 x_8^2 x_9^3 x_{10}^3$     | 1              |
| (0, 4, 3, 2, 1) | (1, 2, 3, 1, 2, 4, 1, 3, 2, 1) | 16  | $x_2 x_3 x_4^3 x_5^2 x_7^3 x_8 x_9^2 x_{10}^3$             | $-1 \cdot 3$   |
| (0, 4, 3, 1, 2) | (2, 1, 1, 4, 4, 3, 1, 2, 1, 2) | 17  | $x_1^2 x_3^3 x_4 x_5 x_7^3 x_8^2 x_9^3 x_{10}^2$           | $2^2$          |
| (0, 4, 3, 0, 3) | (2, 1, 1, 2, 4, 1, 2, 1, 4, 4) | 19  | $x_1 x_2 x_3 x_4^2 x_5^2 x_6^3 x_7^2 x_8^3 x_9^2 x_{10}^2$ | 1              |
| (0, 4, 2, 3, 1) | (2, 2, 1, 1, 3, 1, 3, 4, 1, 3) | 17  | $x_2 x_3 x_4^3 x_5^2 x_6^3 x_7^2 x_9^3 x_{10}^2$           | 3              |
| (0, 4, 2, 2, 2) | (1, 1, 2, 4, 3, 4, 3, 1, 2, 1) | 16  | $x_1 x_2^3 x_3 x_4 x_5 x_6 x_7 x_8^3 x_9 x_{10}^3$         | $2^2$          |
| (0, 4, 2, 1, 3) | (1, 1, 1, 4, 4, 3, 1, 2, 2, 4) | 17  | $x_1 x_2^2 x_3^3 x_4^2 x_5^2 x_7^3 x_8 x_9 x_{10}^2$       | $-1 \cdot 2$   |
| (0, 4, 2, 0, 4) | (1, 1, 1, 4, 4, 2, 4, 2, 1, 4) | 20  | $x_2 x_3^2 x_4^3 x_5^3 x_6 x_7^3 x_8 x_9^3 x_{10}^3$       | 1              |
| (0, 4, 1, 3, 2) | (3, 2, 1, 1, 4, 3, 4, 1, 3, 1) | 17  | $x_1^2 x_4^3 x_5 x_6^2 x_7 x_8^3 x_9^2 x_{10}^3$           | $-1 \cdot 2^2$ |
| (0, 4, 1, 2, 3) | (1, 1, 3, 4, 4, 3, 1, 1, 4, 2) | 17  | $x_2^3 x_3 x_4^2 x_5^2 x_6 x_7^3 x_8^3 x_9^2$              | $2^2$          |
| (0, 4, 1, 1, 4) | (1, 1, 1, 2, 4, 4, 4, 4, 3, 1) | 18  | $x_1^2 x_2 x_3^3 x_5 x_6^2 x_7^3 x_8^3 x_{10}^3$           | $-1$           |
| (0, 4, 0, 3, 3) | (4, 4, 3, 3, 3, 4, 1, 1, 1, 1) | 18  | $x_2 x_3 x_4^2 x_5^2 x_6^2 x_7 x_8^3 x_9^3 x_{10}^3$       | $-1$           |
| (0, 3, 3, 3, 1) | (1, 3, 4, 2, 3, 1, 3, 2, 2, 1) | 16  | $x_1 x_2 x_4^2 x_5^2 x_6^2 x_7^2 x_8^2 x_9^2 x_{10}^2$     | 1              |
| (0, 3, 3, 2, 2) | (2, 1, 1, 3, 2, 2, 1, 4, 4, 3) | 15  | $x_1 x_2^2 x_3^2 x_4 x_5^2 x_6^2 x_7^2 x_8 x_9 x_{10}$     | $-1$           |
| (0, 3, 2, 2, 3) | (1, 1, 2, 4, 2, 3, 1, 3, 4, 4) | 14  | $x_2^2 x_3 x_4^2 x_5 x_6 x_7^2 x_8 x_9^2 x_{10}^2$         | 2              |

$$S \subseteq \mathbb{Z}_p \times \mathbb{Z}_2 \setminus \{(0, 0)\}, |S| = 11$$

| $\lambda$ | $\mathbf{a}$                      | deg | monomial/s                                                                                                                                                                                                         | coefficient/s                                                                                                  |
|-----------|-----------------------------------|-----|--------------------------------------------------------------------------------------------------------------------------------------------------------------------------------------------------------------------|----------------------------------------------------------------------------------------------------------------|
| (11, 0)   | (0, 0, 0, 0, 0, 0, 0, 0, 0, 0, 0) | 109 | $x_1^9 x_2^{10} x_3^{10} x_4^{10} x_5^{10} x_6^{10} x_7^{10} x_8^{10} x_9^{10} x_{10}^{10} x_{11}^{10}$<br>$x_1^{10} x_2^9 x_3^{10} x_4^{10} x_5^{10} x_6^{10} x_7^{10} x_8^{10} x_9^{10} x_{10}^{10} x_{11}^{10}$ | $-1 \cdot 2^3 \cdot 5 \cdot 11 \cdot 3019 \cdot 13647452681$<br>$-1 \cdot 2^3 \cdot 3^2 \cdot 644208651072689$ |
| (10, 1)   | (0, 0, 0, 0, 0, 1, 0, 0, 0, 0, 0) | 65  | $x_1 x_2^3 x_3^8 x_4^8 x_5^9 x_6^9 x_7^9 x_8^9 x_9^9 x_{10}^9 x_{11}^9$                                                                                                                                            | $-1 \cdot 2^2 \cdot 3^3 \cdot 7$                                                                               |
| (9, 2)    | (0, 0, 0, 0, 1, 0, 0, 0, 0, 0, 1) | 57  | $x_1^2 x_2^7 x_3^8 x_4^8 x_7^8 x_8^8 x_9^8 x_{10}^8 x_{11}^8$                                                                                                                                                      | $2^2 \cdot 3^3 \cdot 7$                                                                                        |
| (8, 3)    | (0, 0, 0, 0, 1, 0, 0, 0, 0, 1, 1) | 53  | $x_1^7 x_2^7 x_3^7 x_4^6 x_5^2 x_7^6 x_8^6 x_9^7 x_{10}^2 x_{11}^2$                                                                                                                                                | $-1 \cdot 2^6$                                                                                                 |
| (7, 4)    | (0, 0, 0, 1, 0, 0, 0, 0, 1, 1, 1) | 49  | $x_1^5 x_2^6 x_3^6 x_4^3 x_5^5 x_6^6 x_7^6 x_8^6 x_9^3 x_{10} x_{11}^2$                                                                                                                                            | $3^2 \cdot 5$                                                                                                  |
| (6, 5)    | (0, 0, 0, 1, 0, 0, 0, 1, 1, 1, 1) | 49  | $x_1^4 x_2^5 x_3^5 x_4^4 x_5^5 x_6^5 x_7^4 x_8^4 x_9^4 x_{10}^4 x_{11}^4$<br>$x_1^5 x_2^4 x_3^4 x_4^4 x_5^5 x_6^5 x_7^4 x_8^4 x_9^4 x_{10}^4 x_{11}^4$                                                             | $2 \cdot 3 \cdot 11$<br>$-1 \cdot 2^4 \cdot 3 \cdot 23$                                                        |
| (5, 6)    | (0, 0, 1, 0, 0, 0, 1, 1, 1, 1, 1) | 49  | $x_1^3 x_2^4 x_3^5 x_4^4 x_5^4 x_6^4 x_7^5 x_8^5 x_9^5 x_{10}^5 x_{11}^5$<br>$x_1^4 x_2^3 x_3^4 x_4^4 x_5^4 x_6^4 x_7^5 x_8^5 x_9^5 x_{10}^5 x_{11}^5$                                                             | $2^2 \cdot 13 \cdot 337$<br>$2^3 \cdot 3 \cdot 37$                                                             |
| (4, 7)    | (0, 0, 1, 0, 0, 1, 1, 1, 1, 1, 1) | 53  | $x_1^2 x_2^3 x_3^6 x_4^3 x_5^3 x_6^6 x_7^6 x_8^6 x_9^6 x_{10}^6 x_{11}^6$<br>$x_1^3 x_2^2 x_3^6 x_4^3 x_5^3 x_6^6 x_7^6 x_8^6 x_9^6 x_{10}^6 x_{11}^6$                                                             | $2^2 \cdot 23 \cdot 349$<br>$-1 \cdot 2^2 \cdot 7^2 \cdot 29$                                                  |
| (3, 8)    | (0, 1, 0, 0, 1, 1, 1, 1, 1, 1, 1) | 57  | $x_1^2 x_2^2 x_3^2 x_4^2 x_5^7 x_6^7 x_7^7 x_8^7 x_9^7 x_{10}^7 x_{11}^7$<br>$x_1^2 x_2^3 x_3^2 x_4^2 x_5^6 x_6^7 x_7^7 x_8^7 x_9^7 x_{10}^7 x_{11}^7$                                                             | $2^4 \cdot 5^2 \cdot 7 \cdot 11$<br>$2^5 \cdot 3 \cdot 467$                                                    |
| (2, 9)    | (0, 1, 0, 1, 1, 1, 1, 1, 1, 1, 1) | 65  | $x_2^8 x_3 x_4^8 x_5^8 x_7^8 x_8^8 x_9^8 x_{10}^8 x_{11}^8$<br>$x_1 x_2^7 x_3 x_4^8 x_5^8 x_7^8 x_8^8 x_9^8 x_{10}^8 x_{11}^8$                                                                                     | $2^2 \cdot 3 \cdot 1709$<br>$2 \cdot 7 \cdot 13 \cdot 353$                                                     |
| (1, 10)   | (1, 0, 1, 1, 1, 1, 1, 1, 1, 1, 1) | 73  | $x_1^8 x_3^8 x_4^8 x_5^9 x_7^8 x_8^5 x_9^9 x_{10}^9 x_{11}^9$<br>$x_1^8 x_3^8 x_4^8 x_5^8 x_7^8 x_8^5 x_9^9 x_{10}^9 x_{11}^9$                                                                                     | $-1 \cdot 3 \cdot 5 \cdot 11$<br>$5 \cdot 77863$                                                               |
| (0, 11)   | (1, 1, 1, 1, 1, 1, 1, 1, 1, 1, 1) | 85  | $x_1^3 x_2^4 x_3^8 x_4^{10} x_5^{10} x_6^{10} x_7^{10} x_8^{10} x_9^{10} x_{10}^{10} x_{11}^{10}$<br>$x_1^3 x_2^4 x_3^9 x_4^{10} x_5^{10} x_6^{10} x_7^{10} x_8^{10} x_9^{10} x_{10}^{10} x_{11}^{10}$             | $-1 \cdot 2^2 \cdot 74257$<br>$-1 \cdot 90997$                                                                 |

$$S \subseteq \mathbb{Z}_p \times \mathbb{Z}_3 \setminus \{(0, 0)\}, |S| = 11$$

| $\lambda$  | $\mathbf{a}$                      | deg | monomial/s                                                                                                                                                                                                         | coefficient/s                                                                                                  |
|------------|-----------------------------------|-----|--------------------------------------------------------------------------------------------------------------------------------------------------------------------------------------------------------------------|----------------------------------------------------------------------------------------------------------------|
| (11, 0, 0) | (0, 0, 0, 0, 0, 0, 0, 0, 0, 0, 0) | 109 | $x_1^9 x_2^{10} x_3^{10} x_4^{10} x_5^{10} x_6^{10} x_7^{10} x_8^{10} x_9^{10} x_{10}^{10} x_{11}^{10}$<br>$x_1^{10} x_2^9 x_3^{10} x_4^{10} x_5^{10} x_6^{10} x_7^{10} x_8^{10} x_9^{10} x_{10}^{10} x_{11}^{10}$ | $-1 \cdot 2^3 \cdot 5 \cdot 11 \cdot 3019 \cdot 13647452681$<br>$-1 \cdot 2^3 \cdot 3^2 \cdot 644208651072689$ |
| (10, 1, 0) | (0, 0, 0, 0, 0, 1, 0, 0, 0, 0, 0) | 65  | $x_1 x_2^3 x_3^7 x_4^9 x_5^9 x_7^9 x_8^9 x_{10}^9 x_{11}^9$<br>$x_1 x_2^4 x_3^6 x_4^9 x_5^9 x_7^9 x_8^9 x_{10}^9 x_{11}^9$                                                                                         | $2 \cdot 19^2$<br>$2^2 \cdot 5 \cdot 89$                                                                       |
| (9, 2, 0)  | (0, 0, 0, 1, 0, 0, 0, 1, 0, 0, 0) | 46  | $x_2^2 x_3^4 x_5^3 x_6^5 x_7^8 x_8^7 x_9^8 x_{10}^8 x_{11}^8$                                                                                                                                                      | 1                                                                                                              |
| (9, 1, 1)  | (0, 0, 0, 0, 1, 0, 0, 0, 0, 0, 2) | 56  | $x_1^8 x_2^8 x_3^8 x_4^8 x_6^7 x_7^7 x_9^2 x_{10}^2$                                                                                                                                                               | $2^2 \cdot 3 \cdot 5$                                                                                          |
| (8, 3, 0)  | (0, 0, 1, 0, 0, 0, 1, 0, 0, 0, 1) | 40  | $x_1^2 x_2^4 x_4^4 x_5^7 x_7^6 x_8^7 x_9^7 x_{10}^2 x_{11}^2$                                                                                                                                                      | 2                                                                                                              |
| (8, 2, 1)  | (0, 0, 0, 1, 0, 0, 1, 0, 0, 0, 2) | 39  | $x_1 x_2^3 x_3^6 x_4^7 x_5^7 x_7^6 x_8^7 x_9^7 x_{10}^7$                                                                                                                                                           | $-1 \cdot 2^2$                                                                                                 |
| (7, 4, 0)  | (0, 0, 1, 0, 0, 1, 0, 0, 0, 1, 1) | 38  | $x_1 x_2^3 x_3^2 x_4^6 x_5^6 x_6^2 x_8^6 x_9^6 x_{10}^3 x_{11}^3$                                                                                                                                                  | $-1 \cdot 2$                                                                                                   |

$$S \subseteq \mathbb{Z}_p \times \mathbb{Z}_3 \setminus \{(0, 0)\}, |S| = 11$$

| $\lambda$  | $\mathbf{a}$                      | deg | monomial/s                                                                                                                                                | coefficient/s                  |
|------------|-----------------------------------|-----|-----------------------------------------------------------------------------------------------------------------------------------------------------------|--------------------------------|
| (7, 3, 1)  | (0, 0, 0, 1, 0, 0, 1, 0, 0, 2, 1) | 35  | $x_2^5 x_3^5 x_4^6 x_5^6 x_6^2 x_7^6 x_8^6 x_9 x_{11}^2$                                                                                                  | $-1 \cdot 2$                   |
| (7, 2, 2)  | (0, 0, 1, 0, 0, 1, 0, 0, 0, 2, 2) | 33  | $x_1 x_2^3 x_3^3 x_4^6 x_5^6 x_6^5 x_7^6 x_8^6 x_9 x_{10} x_{11}$                                                                                         | 1                              |
| (6, 5, 0)  | (0, 0, 1, 0, 0, 1, 0, 0, 1, 1, 1) | 37  | $x_2^4 x_3^4 x_4^5 x_5^4 x_6^5 x_7^5 x_8^4 x_9^4 x_{10}^4 x_{11}^4$                                                                                       | $-1 \cdot 2^2$                 |
| (6, 4, 1)  | (0, 0, 1, 0, 0, 1, 0, 0, 2, 1, 1) | 32  | $x_1 x_2^3 x_3^4 x_4^5 x_5^3 x_6^5 x_7^5 x_8^3 x_{10}^3 x_{11}^3$                                                                                         | 2                              |
| (6, 3, 2)  | (0, 0, 0, 1, 0, 1, 0, 0, 2, 1, 2) | 31  | $x_1^5 x_2^5 x_3^4 x_4^2 x_5^5 x_6^2 x_7^4 x_8 x_9 x_{10}^2$                                                                                              | $-1 \cdot 2$                   |
| (5, 6, 0)  | (0, 1, 0, 0, 1, 0, 0, 1, 1, 1, 1) | 37  | $x_1 x_2 x_3^3 x_4^4 x_5^4 x_6^4 x_7^5 x_8^5 x_9^5 x_{10}^5 x_{11}^5$                                                                                     | $-1 \cdot 2 \cdot 3$           |
| (5, 5, 1)  | (0, 0, 1, 0, 1, 0, 0, 1, 1, 1, 2) | 33  | $x_2^2 x_3^3 x_4^4 x_5^4 x_6^4 x_7^4 x_8^4 x_9^4 x_{10}^4$                                                                                                | $2^2 \cdot 3$                  |
| (5, 4, 2)  | (0, 0, 0, 1, 0, 1, 0, 2, 1, 2, 1) | 30  | $x_2^4 x_3^4 x_4^3 x_5^4 x_6^3 x_7^4 x_8 x_9^3 x_{10} x_{11}^3$                                                                                           | $2 \cdot 5^2$                  |
| (5, 3, 3)  | (0, 0, 1, 0, 1, 0, 0, 2, 1, 2, 2) | 28  | $x_1 x_2^3 x_3^2 x_4^4 x_5^2 x_6^4 x_7^4 x_8^2 x_9^2 x_{10}^2 x_{11}^2$                                                                                   | $2^2 \cdot 3$                  |
| (4, 7, 0)  | (0, 1, 0, 1, 0, 0, 1, 1, 1, 1, 1) | 41  | $x_2^2 x_3^3 x_4^6 x_5^3 x_6^3 x_7^6 x_8^6 x_9^6 x_{10}^6 x_{11}^6$                                                                                       | 3                              |
| (4, 6, 1)  | (0, 0, 1, 0, 1, 0, 1, 1, 1, 2, 1) | 35  | $x_1 x_2^3 x_3^5 x_4^3 x_5^5 x_6^2 x_7^4 x_8^5 x_9^5 x_{11}^2$                                                                                            | $2^3$                          |
| (4, 5, 2)  | (0, 0, 1, 0, 1, 0, 2, 1, 2, 1, 1) | 30  | $x_1^3 x_2^3 x_3^4 x_4^3 x_5^4 x_6^2 x_7 x_8^4 x_{10}^4 x_{11}^2$                                                                                         | -1                             |
| (4, 4, 3)  | (0, 0, 1, 0, 1, 1, 2, 0, 2, 1, 2) | 29  | $x_1^3 x_2^2 x_3^3 x_4^3 x_5^3 x_6^3 x_7^2 x_8^3 x_9^2 x_{10}^3 x_{11}^2$                                                                                 | $2 \cdot 3^2$                  |
| (3, 8, 0)  | (0, 1, 0, 1, 0, 1, 1, 1, 1, 1, 1) | 46  | $x_2 x_3 x_4^7 x_5^2 x_6^7 x_7^7 x_8^7 x_9^7 x_{10}^7 x_{11}^7$                                                                                           | $2 \cdot 7$                    |
| (3, 7, 1)  | (0, 1, 0, 1, 0, 1, 1, 1, 2, 1, 1) | 38  | $x_1 x_3 x_4^4 x_5^2 x_6^6 x_7^6 x_8^6 x_{10}^6 x_{11}^6$                                                                                                 | $-1 \cdot 2 \cdot 5$           |
| (3, 6, 2)  | (0, 0, 1, 1, 0, 1, 1, 1, 2, 1, 2) | 34  | $x_1^2 x_2^2 x_3^5 x_4^5 x_5^2 x_6^5 x_7^5 x_8^5 x_9 x_{10}^2$                                                                                            | $2^4$                          |
| (3, 5, 3)  | (0, 0, 2, 1, 1, 0, 1, 2, 1, 2, 1) | 31  | $\frac{x_1^2 x_2^2 x_3^3 x_4^4 x_5^2 x_6^4 x_7^4 x_8^2 x_9^4 x_{10}^4 x_{11}^4}{x_1^2 x_2^2 x_3^2 x_4^4 x_5^3 x_6^2 x_7^4 x_8^2 x_9^4 x_{10}^4 x_{11}^4}$ | $2^2 \cdot 5^2$<br>$-7$        |
| (3, 4, 4)  | (0, 0, 1, 1, 0, 2, 1, 2, 1, 2, 2) | 29  | $x_1^2 x_2^2 x_3^3 x_4^3 x_5^2 x_6^3 x_7^3 x_8^3 x_9^3 x_{10}^3 x_{11}^3$                                                                                 | $-1 \cdot 2^4$                 |
| (2, 9, 0)  | (1, 0, 1, 0, 1, 1, 1, 1, 1, 1, 1) | 52  | $x_1 x_2^3 x_4 x_5^8 x_7^8 x_8^8 x_9^8 x_{10}^8 x_{11}^8$                                                                                                 | $3 \cdot 5$                    |
| (2, 8, 1)  | (0, 1, 1, 0, 1, 1, 1, 1, 1, 1, 2) | 45  | $x_2 x_3^3 x_4 x_5^5 x_6^7 x_7^7 x_8^7 x_9^7 x_{10}^7$                                                                                                    | $-1 \cdot 2^4$                 |
| (2, 7, 2)  | (0, 1, 0, 1, 1, 1, 1, 2, 1, 2, 1) | 40  | $x_1 x_3 x_4^6 x_5^6 x_6^6 x_7^6 x_8^6 x_9 x_{10}^6 x_{11}^6$                                                                                             | 3                              |
| (2, 6, 3)  | (0, 1, 0, 1, 2, 1, 2, 1, 2, 1, 1) | 35  | $x_1 x_2^5 x_3 x_4^5 x_5^2 x_6^5 x_7 x_8^5 x_9^2 x_{10}^5 x_{11}^3$                                                                                       | $2 \cdot 3 \cdot 5$            |
| (2, 5, 4)  | (0, 1, 1, 0, 1, 2, 2, 1, 2, 1, 2) | 34  | $x_1 x_2^4 x_3^4 x_4 x_5^4 x_6^3 x_7^3 x_8^4 x_9^3 x_{10}^4 x_{11}^3$                                                                                     | $2^3 \cdot 11 \cdot 53$        |
|            | (0, 1, 0, 1, 1, 2, 2, 1, 2, 1, 2) | 34  | $x_1 x_2^4 x_3 x_4^4 x_5^3 x_6^3 x_7^3 x_8^4 x_9^3 x_{10}^4 x_{11}^3$                                                                                     | $2^2 \cdot 3 \cdot 5 \cdot 17$ |
| (1, 10, 0) | (1, 1, 0, 1, 1, 1, 1, 1, 1, 1, 1) | 62  | $x_1^2 x_2^2 x_4^9 x_5^9 x_7^9 x_8^9 x_9^9 x_{10}^9 x_{11}^9$                                                                                             | $3 \cdot 5$                    |
| (1, 9, 1)  | (0, 1, 1, 1, 1, 1, 1, 1, 1, 2, 1) | 53  | $x_2^2 x_3^3 x_4^8 x_5^8 x_7^8 x_8^8 x_9^8 x_{11}^8$                                                                                                      | $3 \cdot 5$                    |

$$S \subseteq \mathbb{Z}_p \times \mathbb{Z}_3 \setminus \{(0, 0)\}, |S| = 11$$

| $\lambda$  | $\mathbf{a}$                      | deg | monomial/s                                                                                                                                           | coefficient/s                                                              |
|------------|-----------------------------------|-----|------------------------------------------------------------------------------------------------------------------------------------------------------|----------------------------------------------------------------------------|
| (1, 8, 2)  | (2, 1, 1, 1, 1, 1, 0, 1, 2, 1, 1) | 45  | $x_2^2 x_3 x_4^6 x_5^7 x_6^7 x_8^7 x_9 x_{10}^7 x_{11}^7$                                                                                            | $-1 \cdot 2^2$                                                             |
| (1, 7, 3)  | (0, 1, 1, 1, 1, 1, 1, 2, 2, 1, 2) | 41  | $x_2^3 x_3^3 x_4^5 x_6^6 x_7^6 x_8^2 x_9^2 x_{10}^6 x_{11}^2$                                                                                        | $2^4 \cdot 3$                                                              |
| (1, 6, 4)  | (0, 1, 1, 1, 1, 1, 2, 1, 2, 2, 2) | 38  | $x_2^3 x_3^4 x_4^4 x_5^5 x_6^3 x_7^3 x_8^5 x_9^3 x_{10}^3 x_{11}^3$                                                                                  | $-1 \cdot 3^3$                                                             |
| (1, 5, 5)  | (1, 1, 0, 1, 2, 2, 1, 2, 1, 2, 2) | 37  | $x_1^3 x_2^4 x_3^4 x_4^5 x_6^4 x_7^4 x_8^4 x_9^3 x_{10}^4 x_{11}^4$                                                                                  | $2 \cdot 3^2$                                                              |
| (0, 11, 0) | (1, 1, 1, 1, 1, 1, 1, 1, 1, 1, 1) | 73  | $x_1 x_2^3 x_3^4 x_4^5 x_5^{10} x_6^{10} x_8^{10} x_9^{10} x_{10}^{10} x_{11}^{10}$                                                                  | $3^2 \cdot 5$                                                              |
| (0, 10, 1) | (1, 1, 1, 1, 1, 1, 1, 1, 2, 1, 1) | 62  | $x_1 x_2^2 x_3^5 x_4^9 x_5^9 x_7^9 x_8^9 x_{10}^9 x_{11}^9$                                                                                          | 7                                                                          |
| (0, 9, 2)  | (1, 1, 2, 2, 1, 1, 1, 1, 1, 1, 1) | 56  | $x_1^2 x_2^3 x_3 x_4 x_5^8 x_6^8 x_8^8 x_9^8 x_{10}^8 x_{11}^8$<br>$x_1^2 x_2^3 x_3 x_4 x_5^8 x_6^8 x_8^8 x_9^8 x_{10}^8 x_{11}^8$                   | $-1 \cdot 2^2 \cdot 11$<br>$-1 \cdot 3 \cdot 31$                           |
| (0, 8, 3)  | (1, 1, 2, 2, 1, 1, 2, 1, 1, 1, 1) | 50  | $x_2^2 x_3^2 x_4^2 x_5^7 x_6^7 x_7^7 x_8^7 x_9^7 x_{10}^7 x_{11}^7$<br>$x_2^2 x_3^2 x_4^2 x_5^7 x_6^7 x_7^7 x_8^7 x_9^7 x_{10}^7 x_{11}^7$           | $-1 \cdot 61$<br>$-1 \cdot 113$                                            |
| (0, 7, 4)  | (1, 1, 1, 1, 1, 1, 2, 2, 1, 2, 2) | 44  | $x_1^3 x_2^3 x_3^5 x_4^6 x_5^6 x_6^3 x_7^3 x_8^6 x_9^3 x_{10}^3$                                                                                     | $-1 \cdot 2^4 \cdot 3$                                                     |
| (0, 6, 5)  | (1, 1, 2, 2, 1, 1, 2, 2, 1, 1, 2) | 46  | $x_1 x_2^5 x_3^4 x_4^4 x_5^5 x_6^4 x_7^4 x_8^5 x_9^5 x_{10}^4 x_{11}^4$<br>$x_1^2 x_2^4 x_3^4 x_4^5 x_5^5 x_6^4 x_7^4 x_8^5 x_9^5 x_{10}^4 x_{11}^4$ | $2 \cdot 3 \cdot 5 \cdot 7 \cdot 13 \cdot 29$<br>$2^2 \cdot 19 \cdot 1699$ |

$$S \subseteq \mathbb{Z}_p \times \mathbb{Z}_4 \setminus \{(0, 0)\}, |S| = 11$$

| $\lambda$     | $\mathbf{a}$                      | deg | monomial/s                                                                                                                                                                                                         | coefficient/s                                                                                                  |
|---------------|-----------------------------------|-----|--------------------------------------------------------------------------------------------------------------------------------------------------------------------------------------------------------------------|----------------------------------------------------------------------------------------------------------------|
| (11, 0, 0, 0) | (0, 0, 0, 0, 0, 0, 0, 0, 0, 0, 0) | 109 | $x_1^9 x_2^{10} x_3^{10} x_4^{10} x_5^{10} x_6^{10} x_7^{10} x_8^{10} x_9^{10} x_{10}^{10} x_{11}^{10}$<br>$x_1^{10} x_2^9 x_3^{10} x_4^{10} x_5^{10} x_6^{10} x_7^{10} x_8^{10} x_9^{10} x_{10}^{10} x_{11}^{10}$ | $-1 \cdot 2^3 \cdot 5 \cdot 11 \cdot 3019 \cdot 13647452681$<br>$-1 \cdot 2^3 \cdot 3^2 \cdot 644208651072689$ |
| (10, 1, 0, 0) | (0, 0, 0, 0, 0, 1, 0, 0, 0, 0, 0) | 65  | $x_1 x_2^3 x_3^7 x_4^9 x_5^9 x_6^9 x_8^9 x_9^9 x_{10}^9 x_{11}^9$<br>$x_1 x_2^4 x_3^6 x_4^9 x_5^9 x_6^9 x_8^9 x_9^9 x_{10}^9 x_{11}^9$                                                                             | $-1 \cdot 2^2 \cdot 3 \cdot 7 \cdot 11$<br>$-1 \cdot 2^2 \cdot 5^2 \cdot 23$                                   |
| (10, 0, 1, 0) | (0, 0, 0, 0, 0, 2, 0, 0, 0, 0, 0) | 65  | $x_1 x_2^3 x_3^7 x_4^9 x_5^9 x_6^9 x_8^9 x_9^9 x_{10}^9 x_{11}^9$<br>$x_1 x_2^4 x_3^6 x_4^9 x_5^9 x_6^9 x_8^9 x_9^9 x_{10}^9 x_{11}^9$                                                                             | $-1 \cdot 2^2 \cdot 3 \cdot 7 \cdot 11$<br>$-1 \cdot 2^2 \cdot 5^2 \cdot 23$                                   |
| (9, 2, 0, 0)  | (0, 0, 0, 1, 0, 0, 0, 1, 0, 0, 0) | 46  | $x_1 x_2^3 x_3^5 x_4^5 x_6^8 x_8 x_9^7 x_{10}^8 x_{11}^8$                                                                                                                                                          | $-1 \cdot 2$                                                                                                   |
| (9, 1, 0, 1)  | (0, 0, 0, 0, 1, 0, 0, 0, 0, 0, 3) | 56  | $x_1 x_2^3 x_3^5 x_4^8 x_6^7 x_7^8 x_8^8 x_9^8 x_{10}^8$                                                                                                                                                           | $-1 \cdot 2^2$                                                                                                 |
| (9, 1, 1, 0)  | (0, 0, 0, 1, 0, 0, 0, 2, 0, 0, 0) | 45  | $x_1 x_2^3 x_3^5 x_4^5 x_6^8 x_7^8 x_9^8 x_{10}^8 x_{11}^8$                                                                                                                                                        | $-1 \cdot 2$                                                                                                   |
| (9, 0, 2, 0)  | (0, 0, 0, 0, 2, 0, 0, 0, 0, 0, 2) | 57  | $x_1^2 x_2^7 x_3^7 x_4^8 x_7^8 x_8^8 x_9^8 x_{10}^8 x_{11}^8$                                                                                                                                                      | $2^2 \cdot 3^3 \cdot 7$                                                                                        |
| (8, 3, 0, 0)  | (0, 0, 1, 0, 0, 1, 0, 0, 1, 0, 0) | 35  | $x_1 x_2^3 x_3^3 x_4^5 x_6 x_7^8 x_8^2 x_{10}^6 x_{11}^7$                                                                                                                                                          | -1                                                                                                             |
| (8, 2, 0, 1)  | (0, 0, 0, 1, 0, 0, 1, 0, 0, 0, 3) | 39  | $x_2^2 x_3^4 x_4^4 x_5^4 x_6^7 x_7^8 x_8^6 x_9^7 x_{10}^7$                                                                                                                                                         | -1                                                                                                             |
| (8, 2, 1, 0)  | (0, 0, 1, 0, 0, 0, 1, 0, 0, 0, 2) | 38  | $x_1 x_2^3 x_3 x_4^2 x_5^4 x_6^7 x_8^6 x_9^7 x_{10}^7$                                                                                                                                                             | -1                                                                                                             |
| (8, 1, 1, 1)  | (0, 0, 1, 0, 0, 2, 0, 0, 3, 0, 0) | 32  | $x_1 x_2^3 x_3^3 x_4^5 x_7^8 x_{10}^6 x_{11}^7$                                                                                                                                                                    | -1                                                                                                             |

$$S \subseteq \mathbb{Z}_p \times \mathbb{Z}_4 \setminus \{(0, 0)\}, |S| = 11$$

| $\lambda$    | $\mathbf{a}$                      | deg | monomial/s                                                                                                                                             | coefficient/s                                           |
|--------------|-----------------------------------|-----|--------------------------------------------------------------------------------------------------------------------------------------------------------|---------------------------------------------------------|
| (8, 1, 2, 0) | (0, 0, 2, 0, 0, 1, 0, 0, 2, 0, 0) | 33  | $x_1 x_2^3 x_3^4 x_5^7 x_8^9 x_9 x_{10}^6 x_{11}^7$                                                                                                    | -1                                                      |
| (8, 0, 3, 0) | (0, 0, 0, 0, 2, 0, 0, 0, 0, 2, 2) | 53  | $x_1^7 x_2^7 x_3^7 x_4^6 x_5^2 x_7^7 x_8^6 x_9^7 x_{10}^2 x_{11}^2$                                                                                    | $-1 \cdot 2^6$                                          |
| (7, 4, 0, 0) | (0, 1, 0, 0, 1, 0, 0, 1, 0, 0, 1) | 31  | $x_1^2 x_3^2 x_4^4 x_5 x_6^6 x_8^2 x_9^5 x_{10}^6 x_{11}^3$                                                                                            | 1                                                       |
| (7, 3, 0, 1) | (0, 0, 1, 0, 0, 1, 0, 1, 0, 0, 3) | 29  | $x_2^2 x_4^2 x_5^4 x_6^2 x_7^6 x_8^2 x_9^5 x_{10}^6$                                                                                                   | -1                                                      |
| (7, 2, 0, 2) | (0, 0, 1, 0, 0, 1, 0, 0, 0, 3, 3) | 33  | $x_1 x_2^3 x_4^3 x_5^6 x_6 x_7^5 x_8^6 x_9^6 x_{10} x_{11}$                                                                                            | 1                                                       |
| (7, 3, 1, 0) | (0, 0, 1, 0, 1, 0, 0, 1, 0, 0, 2) | 29  | $x_2^2 x_3 x_4^3 x_5 x_6^3 x_7^6 x_8^2 x_9^5 x_{10}^6$                                                                                                 | -1                                                      |
| (7, 2, 1, 1) | (0, 0, 1, 0, 0, 2, 0, 3, 0, 0, 1) | 27  | $x_2^2 x_4^2 x_5^5 x_7^6 x_9^5 x_{10}^6 x_{11}$                                                                                                        | -1                                                      |
| (7, 2, 2, 0) | (0, 0, 1, 0, 2, 0, 0, 2, 1, 0, 0) | 28  | $x_2^2 x_4^2 x_5^5 x_6^6 x_7 x_8 x_9 x_{10}^5 x_{11}^6$                                                                                                | $-1 \cdot 2$                                            |
| (7, 1, 2, 1) | (0, 1, 0, 0, 2, 0, 0, 3, 0, 0, 2) | 26  | $x_1 x_3 x_4^3 x_6^3 x_7^6 x_9^5 x_{10}^6 x_{11}$                                                                                                      | 1                                                       |
| (7, 1, 3, 0) | (0, 0, 2, 0, 0, 1, 0, 2, 0, 0, 2) | 29  | $x_2^2 x_4^2 x_5^5 x_7^6 x_8 x_9^5 x_{10}^6 x_{11}^2$                                                                                                  | -1                                                      |
| (7, 0, 4, 0) | (0, 0, 0, 2, 0, 0, 0, 0, 2, 2, 2) | 49  | $x_1^2 x_2^5 x_3^6 x_4^3 x_5^6 x_6^6 x_7^6 x_8^6 x_9^3 x_{10}^3 x_{11}^3$                                                                              | $-1 \cdot 2^9 \cdot 3^2$                                |
| (6, 5, 0, 0) | (0, 1, 0, 1, 0, 0, 1, 0, 0, 1, 1) | 31  | $x_2 x_3^2 x_4 x_5^2 x_6^5 x_7^3 x_8^4 x_9^5 x_{10}^4 x_{11}^4$                                                                                        | -1                                                      |
| (6, 4, 0, 1) | (0, 0, 1, 0, 0, 1, 0, 1, 0, 3, 1) | 27  | $x_2^2 x_4^2 x_5^5 x_6^2 x_7^5 x_8^3 x_9^5 x_{11}^3$                                                                                                   | 1                                                       |
| (6, 3, 0, 2) | (0, 0, 1, 0, 1, 0, 1, 0, 0, 3, 3) | 25  | $x_2^2 x_3 x_4^3 x_5 x_6^5 x_7^2 x_8^4 x_9^5 x_{10} x_{11}$                                                                                            | 1                                                       |
| (6, 4, 1, 0) | (0, 0, 1, 0, 1, 0, 1, 0, 0, 2, 1) | 27  | $x_2^2 x_4^2 x_5^5 x_6^3 x_7^3 x_8^4 x_9^5 x_{11}^3$                                                                                                   | -1                                                      |
| (6, 3, 1, 1) | (0, 1, 0, 0, 1, 0, 1, 0, 0, 3, 2) | 23  | $x_1 x_3 x_4^3 x_5^2 x_6^5 x_7^2 x_8^4 x_9^5$                                                                                                          | 1                                                       |
| (6, 2, 1, 2) | (0, 0, 1, 0, 0, 2, 0, 3, 0, 1, 3) | 23  | $x_2^2 x_4^3 x_5^5 x_7^5 x_8 x_9^5 x_{10} x_{11}$                                                                                                      | 2                                                       |
| (6, 3, 2, 0) | (0, 0, 1, 0, 2, 0, 2, 1, 0, 0, 1) | 25  | $x_2^2 x_4^4 x_5 x_6^5 x_7 x_8 x_9^4 x_{10}^5 x_{11}^2$                                                                                                | -1                                                      |
| (6, 2, 2, 1) | (0, 0, 1, 0, 2, 0, 3, 0, 0, 1, 2) | 23  | $x_2^2 x_3 x_4^4 x_5^5 x_6^4 x_8^5 x_9 x_{10} x_{11}$                                                                                                  | -1                                                      |
| (6, 2, 3, 0) | (0, 1, 0, 2, 0, 0, 2, 1, 0, 0, 2) | 24  | $x_1 x_3 x_5^3 x_6^5 x_7^2 x_8 x_9^4 x_{10}^5 x_{11}^2$                                                                                                | $2^2$                                                   |
| (6, 1, 3, 1) | (0, 0, 1, 0, 2, 0, 2, 2, 3, 0, 0) | 24  | $x_2^2 x_4^2 x_5^2 x_6^5 x_7^2 x_8^2 x_{10}^4 x_{11}^5$                                                                                                | -1                                                      |
| (6, 1, 4, 0) | (0, 0, 2, 0, 0, 1, 0, 2, 0, 2, 2) | 27  | $x_2^2 x_4^2 x_5^5 x_7^4 x_8^3 x_9^5 x_{10}^3 x_{11}^3$                                                                                                | -1                                                      |
| (6, 0, 5, 0) | (0, 0, 0, 2, 0, 0, 0, 2, 2, 2, 2) | 49  | $x_1^4 x_2^5 x_3^5 x_4^4 x_5^5 x_6^5 x_7^5 x_8^4 x_9^4 x_{10}^4 x_{11}^4$<br>$x_1^5 x_2^4 x_3^5 x_4^4 x_5^5 x_6^5 x_7^5 x_8^4 x_9^4 x_{10}^4 x_{11}^4$ | $2 \cdot 3 \cdot 11$<br>$-1 \cdot 2^4 \cdot 3 \cdot 23$ |
| (5, 6, 0, 0) | (0, 1, 0, 1, 0, 1, 0, 0, 1, 1, 1) | 32  | $x_3 x_4^2 x_5^4 x_6^3 x_7^3 x_8^4 x_9^5 x_{10}^5 x_{11}^5$                                                                                            | $-1 \cdot 2$                                            |
| (5, 5, 0, 1) | (0, 1, 0, 0, 1, 0, 1, 0, 3, 1, 1) | 26  | $x_1 x_3 x_4^4 x_5 x_6^3 x_7^4 x_8^4 x_{10}^4 x_{11}^4$                                                                                                | -1                                                      |

$$S \subseteq \mathbb{Z}_p \times \mathbb{Z}_4 \setminus \{(0, 0)\}, |S| = 11$$

| $\lambda$    | $\mathbf{a}$                      | deg | monomial/s                                                                                                                                             | coefficient/s                                      |
|--------------|-----------------------------------|-----|--------------------------------------------------------------------------------------------------------------------------------------------------------|----------------------------------------------------|
| (5, 4, 0, 2) | (0, 0, 1, 0, 0, 1, 1, 0, 3, 1, 3) | 24  | $x_2^2 x_4^3 x_5^4 x_6^3 x_7^3 x_8^4 x_9 x_{10}^3 x_{11}$                                                                                              | 3                                                  |
| (5, 3, 0, 3) | (0, 1, 0, 1, 0, 1, 0, 0, 3, 3, 3) | 22  | $x_1 x_3 x_4 x_5^4 x_6^2 x_7^3 x_8^4 x_9^2 x_{10}^2 x_{11}^2$                                                                                          | -1                                                 |
| (5, 5, 1, 0) | (0, 0, 1, 0, 1, 0, 1, 0, 2, 1, 1) | 27  | $x_2^2 x_4^2 x_5^3 x_6^4 x_7^4 x_8^4 x_{10}^4 x_{11}^4$                                                                                                | $-1 \cdot 2^2$                                     |
| (5, 4, 1, 1) | (0, 0, 1, 0, 1, 0, 1, 0, 3, 1, 2) | 23  | $x_2^2 x_3 x_4^4 x_5^2 x_6^4 x_7^3 x_8^4 x_{10}^3$                                                                                                     | 1                                                  |
| (5, 3, 1, 2) | (0, 0, 1, 0, 0, 2, 3, 0, 1, 3, 1) | 21  | $x_2^2 x_3^2 x_4^3 x_5^4 x_7 x_8^4 x_9^2 x_{10} x_{11}^2$                                                                                              | 3                                                  |
| (5, 4, 2, 0) | (0, 1, 0, 1, 0, 1, 0, 0, 2, 1, 2) | 23  | $x_1 x_3 x_4^2 x_5^4 x_6^3 x_7^3 x_8^4 x_9 x_{10}^3 x_{11}$                                                                                            | 1                                                  |
| (5, 3, 2, 1) | (0, 0, 1, 0, 2, 0, 2, 1, 0, 1, 3) | 21  | $x_2^2 x_3 x_4^4 x_5 x_6^4 x_7 x_8^2 x_9^4 x_{10}^2$                                                                                                   | $-1 \cdot 3$                                       |
| (5, 2, 2, 2) | (0, 1, 0, 0, 2, 0, 3, 0, 1, 3, 2) | 19  | $x_1 x_3^2 x_4^4 x_6^4 x_7 x_8^4 x_9 x_{10} x_{11}$                                                                                                    | $-1 \cdot 2$                                       |
| (5, 3, 3, 0) | (0, 0, 1, 1, 0, 0, 1, 0, 2, 2, 2) | 23  | $x_2^2 x_3 x_4 x_5^3 x_6^4 x_7^2 x_8^4 x_9^2 x_{10}^2 x_{11}^2$                                                                                        | -1                                                 |
| (5, 2, 3, 1) | (0, 0, 1, 0, 2, 2, 2, 3, 0, 0, 1) | 21  | $x_2^2 x_3 x_4^4 x_5^2 x_6^2 x_7^2 x_9^3 x_{10}^4 x_{11}$                                                                                              | 3                                                  |
| (5, 2, 4, 0) | (0, 0, 1, 2, 0, 2, 2, 2, 1, 0, 0) | 24  | $x_2^4 x_5^3 x_6^3 x_7^2 x_8^3 x_9 x_{10}^3 x_{11}^4$                                                                                                  | $-1 \cdot 2$                                       |
| (5, 1, 4, 1) | (0, 1, 0, 2, 0, 2, 2, 3, 0, 0, 2) | 22  | $x_1 x_3 x_5^4 x_6^3 x_7^3 x_9^3 x_{10}^4 x_{11}^3$                                                                                                    | 3                                                  |
| (5, 1, 5, 0) | (0, 0, 2, 0, 0, 1, 2, 0, 2, 2, 2) | 27  | $x_2^2 x_3 x_4^3 x_5^4 x_7 x_8^4 x_9^4 x_{10}^4 x_{11}^4$                                                                                              | $-1 \cdot 3$                                       |
| (5, 0, 6, 0) | (0, 0, 2, 0, 0, 0, 2, 2, 2, 2, 2) | 49  | $x_1^3 x_2^4 x_3^5 x_4^4 x_5^4 x_6^5 x_7^5 x_8^5 x_9^5 x_{10}^5 x_{11}^5$<br>$x_1^4 x_2^3 x_3^5 x_4^4 x_5^4 x_6^4 x_7^5 x_8^5 x_9^5 x_{10}^5 x_{11}^5$ | $2^2 \cdot 13 \cdot 337$<br>$2^3 \cdot 3 \cdot 37$ |
| (4, 7, 0, 0) | (0, 1, 0, 1, 0, 1, 0, 1, 1, 1, 1) | 35  | $x_3 x_4 x_5^2 x_6^4 x_7^3 x_8^6 x_9^6 x_{10}^6 x_{11}^6$                                                                                              | 2                                                  |
| (4, 6, 0, 1) | (0, 1, 0, 1, 0, 1, 0, 3, 1, 1, 1) | 29  | $x_2 x_3^2 x_4 x_5^3 x_6^4 x_7^3 x_9^5 x_{10}^5 x_{11}^5$                                                                                              | -1                                                 |
| (4, 5, 0, 2) | (0, 0, 1, 0, 0, 1, 1, 3, 1, 3, 1) | 25  | $x_2^3 x_4^2 x_5^3 x_6^3 x_7^4 x_8 x_9^4 x_{10} x_{11}^4$                                                                                              | $-1 \cdot 2$                                       |
| (4, 4, 0, 3) | (0, 0, 1, 0, 1, 1, 0, 3, 1, 3, 3) | 23  | $x_2^2 x_3 x_4^3 x_5^2 x_6^3 x_7^3 x_8^2 x_9^3 x_{10}^2 x_{11}^2$                                                                                      | 3                                                  |
| (4, 6, 1, 0) | (0, 1, 0, 1, 0, 1, 0, 2, 1, 1, 1) | 28  | $x_1 x_3 x_4 x_5^3 x_6^4 x_7^3 x_9^5 x_{10}^5 x_{11}^5$                                                                                                | 2                                                  |
| (4, 5, 1, 1) | (0, 0, 1, 0, 1, 1, 0, 2, 1, 1, 3) | 24  | $x_2^2 x_4^3 x_5^4 x_6^4 x_7^3 x_9^4 x_{10}^4$                                                                                                         | $-1 \cdot 2^2$                                     |
| (4, 4, 1, 2) | (0, 1, 0, 0, 1, 1, 0, 3, 1, 3, 2) | 20  | $x_1 x_3^2 x_4^3 x_5^3 x_6^3 x_7^3 x_8 x_9^3 x_{10}$                                                                                                   | $-1 \cdot 3$                                       |
| (4, 3, 1, 3) | (0, 0, 1, 0, 0, 2, 3, 1, 3, 1, 3) | 20  | $x_2^3 x_3^2 x_4^2 x_5^3 x_7^2 x_8^2 x_9^2 x_{10}^2 x_{11}^2$                                                                                          | $-1 \cdot 2 \cdot 3$                               |
| (4, 5, 2, 0) | (0, 0, 1, 1, 0, 1, 0, 2, 1, 1, 2) | 25  | $x_2^2 x_3 x_4^2 x_5^3 x_6^4 x_7^3 x_8 x_9^4 x_{10}^4 x_{11}$                                                                                          | $2^2$                                              |
| (4, 4, 2, 1) | (0, 0, 1, 0, 2, 3, 0, 1, 2, 1, 1) | 21  | $x_1^3 x_2^2 x_3^3 x_4^3 x_5 x_7^3 x_8^3 x_{10}^3$                                                                                                     | 2                                                  |
| (4, 3, 2, 2) | (0, 0, 1, 0, 2, 3, 0, 1, 3, 1, 2) | 19  | $x_1 x_2^3 x_3^2 x_4^3 x_6 x_7^3 x_8^2 x_9 x_{10}^2 x_{11}$                                                                                            | $2^2 \cdot 3$                                      |

$$S \subseteq \mathbb{Z}_p \times \mathbb{Z}_4 \setminus \{(0, 0)\}, |S| = 11$$

| $\lambda$    | $\mathbf{a}$                      | deg | monomial/s                                                                                                                                             | coefficient/s                                                 |
|--------------|-----------------------------------|-----|--------------------------------------------------------------------------------------------------------------------------------------------------------|---------------------------------------------------------------|
| (4, 4, 3, 0) | (0, 0, 1, 1, 0, 1, 0, 2, 2, 2, 1) | 23  | $x_2^2 x_3 x_4^2 x_5^3 x_6^3 x_7^3 x_8^2 x_9^2 x_{10}^2 x_{11}^3$                                                                                      | 2                                                             |
| (4, 3, 3, 1) | (0, 1, 0, 1, 0, 1, 0, 2, 2, 3, 2) | 19  | $x_1^3 x_2^2 x_3^2 x_4^2 x_5^3 x_6^2 x_7 x_8^2 x_9 x_{11}$                                                                                             | 1                                                             |
| (4, 2, 3, 2) | (0, 0, 1, 0, 2, 2, 2, 3, 0, 1, 3) | 19  | $x_2^3 x_3 x_4^3 x_5^2 x_6^2 x_7 x_8 x_9^3 x_{10} x_{11}$                                                                                              | $-1 \cdot 2$                                                  |
| (4, 3, 4, 0) | (0, 0, 1, 2, 2, 1, 0, 0, 1, 2, 2) | 23  | $x_2^3 x_3 x_4^2 x_5^3 x_6 x_7^2 x_8^3 x_9^2 x_{10}^3 x_{11}^3$                                                                                        | 2                                                             |
| (4, 2, 4, 1) | (0, 0, 1, 2, 2, 2, 3, 0, 0, 1, 2) | 21  | $x_1 x_2^3 x_3 x_4^2 x_5^2 x_6^3 x_8^2 x_9^3 x_{10} x_{11}^3$                                                                                          | $-1 \cdot 2^3$                                                |
| (4, 2, 5, 0) | (0, 1, 2, 0, 2, 2, 2, 1, 0, 0, 2) | 24  | $x_1 x_4^2 x_5^3 x_6^4 x_7^4 x_8 x_9^2 x_{10}^3 x_{11}^4$                                                                                              | 1                                                             |
| (4, 1, 5, 1) | (0, 0, 1, 2, 2, 2, 2, 2, 3, 0, 0) | 24  | $x_2^3 x_4 x_5^3 x_6^4 x_7^4 x_8^4 x_{10}^2 x_{11}^3$                                                                                                  | -1                                                            |
| (4, 1, 6, 0) | (0, 0, 2, 0, 0, 1, 2, 2, 2, 2, 2) | 29  | $x_2^3 x_4^2 x_5^3 x_7^2 x_8^4 x_9^5 x_{10}^5 x_{11}^5$                                                                                                | -1                                                            |
| (4, 0, 7, 0) | (0, 0, 2, 0, 0, 2, 2, 2, 2, 2, 2) | 53  | $x_1^2 x_2^3 x_3^6 x_4^3 x_5^3 x_6^6 x_7^6 x_8^6 x_9^6 x_{10}^6 x_{11}^6$<br>$x_1^3 x_2^2 x_3^6 x_4^3 x_5^3 x_6^6 x_7^6 x_8^6 x_9^6 x_{10}^6 x_{11}^6$ | $2^2 \cdot 23 \cdot 349$<br>$-1 \cdot 2^2 \cdot 7^2 \cdot 29$ |
| (3, 8, 0, 0) | (1, 0, 1, 0, 1, 0, 1, 1, 1, 1, 1) | 39  | $x_1 x_2^3 x_4 x_5^5 x_6^2 x_7 x_8^7 x_9^7 x_{10}^7 x_{11}^7$                                                                                          | 2                                                             |
| (3, 7, 0, 1) | (0, 1, 0, 1, 1, 0, 1, 1, 1, 1, 3) | 33  | $x_3 x_4^2 x_5^4 x_6^2 x_7^6 x_8^6 x_9^6 x_{10}^6$                                                                                                     | 2                                                             |
| (3, 6, 0, 2) | (0, 1, 0, 0, 1, 1, 3, 1, 3, 1, 1) | 27  | $x_1^2 x_3 x_4^2 x_5^2 x_6^3 x_7 x_8^5 x_9 x_{10}^5 x_{11}^5$                                                                                          | 2                                                             |
| (3, 5, 0, 3) | (0, 1, 0, 0, 1, 1, 1, 3, 3, 1, 3) | 25  | $x_1 x_3 x_4^2 x_5^3 x_6^4 x_7^4 x_8^2 x_9^2 x_{10}^4 x_{11}^2$                                                                                        | -1                                                            |
| (3, 4, 0, 4) | (0, 1, 0, 1, 1, 0, 3, 1, 3, 3, 3) | 23  | $x_1 x_3 x_4 x_5^3 x_6^2 x_7^3 x_8^3 x_9^3 x_{10}^3 x_{11}^3$                                                                                          | 2                                                             |
| (3, 7, 1, 0) | (0, 1, 1, 0, 1, 0, 1, 1, 1, 1, 2) | 33  | $x_2 x_3 x_4 x_5^4 x_6^2 x_7^6 x_8^6 x_9^6 x_{10}^6$                                                                                                   | 2                                                             |
| (3, 6, 1, 1) | (0, 0, 1, 0, 1, 1, 2, 1, 1, 3, 1) | 27  | $x_2^2 x_4^2 x_5^3 x_6^5 x_8^5 x_9^5 x_{11}^5$                                                                                                         | 2                                                             |
| (3, 5, 1, 2) | (0, 0, 1, 0, 1, 1, 3, 1, 3, 1, 2) | 23  | $x_2^2 x_3^2 x_4^2 x_5^3 x_6^4 x_7 x_8^4 x_9 x_{10}^4$                                                                                                 | 2                                                             |
| (3, 4, 1, 3) | (0, 0, 1, 0, 1, 1, 3, 1, 3, 3, 2) | 21  | $x_2^2 x_3^2 x_4^2 x_5^3 x_6^3 x_7^2 x_8^3 x_9^2 x_{10}^2$                                                                                             | 2                                                             |
| (3, 6, 2, 0) | (0, 0, 1, 1, 1, 0, 2, 1, 1, 2, 1) | 28  | $x_2^2 x_4^3 x_5^4 x_6^2 x_7 x_8^5 x_9^5 x_{10} x_{11}^5$                                                                                              | 2                                                             |
| (3, 5, 2, 1) | (0, 1, 0, 1, 1, 0, 2, 1, 1, 3, 2) | 22  | $x_1 x_3 x_4^4 x_5^4 x_6^2 x_7 x_8^4 x_9^4 x_{11}$                                                                                                     | $-1 \cdot 2^2$                                                |
| (3, 4, 2, 2) | (0, 0, 1, 0, 2, 3, 1, 2, 1, 1, 3) | 20  | $x_2^2 x_3^3 x_4^2 x_5 x_6 x_7^3 x_8 x_9^3 x_{10}^3 x_{11}$                                                                                            | $-1 \cdot 2^2 \cdot 3$                                        |
| (3, 3, 2, 3) | (0, 1, 0, 0, 2, 3, 1, 3, 1, 3, 2) | 18  | $x_1^2 x_2^2 x_3 x_4^2 x_6^2 x_7^2 x_8^2 x_9^2 x_{10} x_{11}$                                                                                          | $2 \cdot 3$                                                   |
| (3, 5, 3, 0) | (0, 0, 1, 1, 0, 1, 2, 1, 1, 2, 2) | 25  | $x_2^2 x_4^3 x_5^2 x_6^4 x_7^2 x_8^4 x_9^4 x_{10}^2 x_{11}^2$                                                                                          | $2^2$                                                         |
| (3, 4, 3, 1) | (0, 0, 1, 1, 0, 1, 2, 2, 3, 1, 2) | 21  | $x_2^2 x_3^2 x_4^3 x_5^2 x_6^3 x_7^2 x_8^2 x_{10}^3 x_{11}^2$                                                                                          | $-1 \cdot 3$                                                  |
| (3, 3, 3, 2) | (0, 0, 1, 1, 0, 3, 2, 3, 1, 2, 2) | 19  | $x_1 x_2^2 x_3^2 x_4^2 x_5^2 x_6 x_7^2 x_8 x_9^2 x_{10}^2 x_{11}^2$                                                                                    | 2                                                             |

$$S \subseteq \mathbb{Z}_p \times \mathbb{Z}_4 \setminus \{(0, 0)\}, |S| = 11$$

| $\lambda$    | $\mathbf{a}$                      | deg | monomial/s                                                                                                                                             | coefficient/s                                               |
|--------------|-----------------------------------|-----|--------------------------------------------------------------------------------------------------------------------------------------------------------|-------------------------------------------------------------|
| (3, 4, 4, 0) | (0, 1, 1, 0, 1, 0, 2, 2, 2, 1, 2) | 23  | $x_1 x_3 x_4 x_5^3 x_6^2 x_7^3 x_8^3 x_9^3 x_{10}^3 x_{11}^3$                                                                                          | 2                                                           |
| (3, 3, 4, 1) | (0, 0, 1, 2, 2, 1, 0, 1, 2, 2, 3) | 21  | $x_2^2 x_3^2 x_4^2 x_5^3 x_6^2 x_7^2 x_8^2 x_9^3 x_{10}^3$                                                                                             | $2 \cdot 3$                                                 |
| (3, 2, 4, 2) | (0, 1, 0, 2, 2, 2, 3, 0, 1, 3, 2) | 19  | $x_1^2 x_2 x_3^2 x_5^3 x_6^3 x_7 x_8^2 x_9 x_{10} x_{11}^3$                                                                                            | $-1 \cdot 2$                                                |
| (3, 3, 5, 0) | (0, 0, 2, 0, 1, 2, 1, 1, 2, 2, 2) | 25  | $x_2^2 x_4^2 x_5 x_6^4 x_7^2 x_8^2 x_9^4 x_{10}^4 x_{11}^4$                                                                                            | $-1 \cdot 2^2$                                              |
| (3, 2, 5, 1) | (0, 0, 2, 0, 1, 2, 1, 3, 2, 2, 2) | 23  | $x_2^2 x_3^2 x_4^2 x_5 x_6^3 x_7 x_8^4 x_{10}^4 x_{11}^4$                                                                                              | 1                                                           |
| (3, 2, 6, 0) | (0, 0, 2, 0, 1, 2, 2, 2, 2, 2, 1) | 28  | $x_2^2 x_3^2 x_4^2 x_6^2 x_7^4 x_8^5 x_9^5 x_{10}^5 x_{11}$                                                                                            | 1                                                           |
| (3, 1, 6, 1) | (0, 1, 2, 2, 2, 2, 2, 3, 0, 0, 2) | 26  | $x_1^2 x_4^2 x_5^4 x_6^5 x_7^5 x_9 x_{10}^2 x_{11}^5$                                                                                                  | 1                                                           |
| (3, 1, 7, 0) | (0, 2, 0, 0, 2, 1, 2, 2, 2, 2, 2) | 33  | $x_1 x_3 x_4^2 x_5^3 x_7^3 x_8^5 x_9^6 x_{10}^6 x_{11}^6$                                                                                              | -1                                                          |
| (3, 0, 8, 0) | (0, 2, 0, 0, 2, 2, 2, 2, 2, 2, 2) | 57  | $x_1^2 x_2^2 x_3^2 x_4^2 x_5^7 x_6^7 x_7^7 x_8^7 x_9^7 x_{10}^7 x_{11}^7$<br>$x_1^2 x_2^3 x_3^2 x_4^2 x_5^6 x_6^7 x_7^7 x_8^7 x_9^7 x_{10}^7 x_{11}^7$ | $2^4 \cdot 5^2 \cdot 7 \cdot 11$<br>$2^5 \cdot 3 \cdot 467$ |
| (2, 9, 0, 0) | (1, 1, 0, 1, 0, 1, 1, 1, 1, 1, 1) | 47  | $x_1^2 x_2^2 x_4^3 x_5 x_6^7 x_8^8 x_9^8 x_{10}^8 x_{11}^8$                                                                                            | 2                                                           |
| (2, 8, 0, 1) | (0, 1, 0, 1, 1, 1, 1, 1, 1, 3, 1) | 39  | $x_3 x_4 x_5^3 x_6^6 x_7^7 x_8^7 x_9^7 x_{11}^7$                                                                                                       | $-1 \cdot 3$                                                |
| (2, 7, 0, 2) | (0, 1, 0, 1, 1, 3, 1, 3, 1, 1, 1) | 33  | $x_2^2 x_3 x_4 x_5^3 x_6 x_7^6 x_8^6 x_9^6 x_{10}^6 x_{11}^6$                                                                                          | -1                                                          |
| (2, 6, 0, 3) | (0, 1, 0, 1, 1, 1, 3, 3, 3, 1, 1) | 29  | $x_3 x_4^2 x_5^5 x_6^5 x_7^2 x_8^2 x_9^5 x_{10}^5 x_{11}^5$                                                                                            | $-1 \cdot 2^3$                                              |
| (2, 5, 0, 4) | (0, 1, 0, 1, 1, 1, 3, 3, 1, 3, 3) | 27  | $x_2^2 x_3 x_4^2 x_5^3 x_6^4 x_7^2 x_8^3 x_9^4 x_{10}^3 x_{11}^3$                                                                                      | $-1 \cdot 2$                                                |
| (2, 8, 1, 0) | (0, 1, 1, 1, 0, 1, 1, 1, 1, 2, 1) | 39  | $x_3^2 x_4^2 x_5 x_6^6 x_7^7 x_8^7 x_9^7 x_{11}^7$                                                                                                     | $-1 \cdot 3$                                                |
| (2, 7, 1, 1) | (0, 1, 0, 1, 1, 2, 1, 1, 3, 1, 1) | 31  | $x_1 x_3 x_4 x_5^5 x_7^5 x_8^6 x_{10}^6 x_{11}^6$                                                                                                      | 1                                                           |
| (2, 6, 1, 2) | (0, 1, 0, 1, 1, 1, 1, 2, 3, 1, 3) | 27  | $x_3 x_4^4 x_5^5 x_6^5 x_7 x_9 x_{10}^5 x_{11}$                                                                                                        | $-1 \cdot 3$                                                |
| (2, 5, 1, 3) | (0, 1, 0, 1, 1, 3, 1, 3, 1, 2, 3) | 23  | $x_1 x_3 x_4^3 x_5^4 x_6^2 x_7^4 x_8^2 x_9^4 x_{11}^2$                                                                                                 | $-1 \cdot 2$                                                |
| (2, 4, 1, 4) | (0, 1, 0, 1, 1, 2, 3, 3, 3, 1, 3) | 23  | $x_2 x_3 x_4^3 x_5^3 x_7^3 x_8^3 x_9^3 x_{10}^3 x_{11}^3$                                                                                              | $2^2$                                                       |
| (2, 7, 2, 0) | (0, 1, 0, 1, 1, 1, 2, 1, 2, 1, 1) | 33  | $x_3 x_4 x_5^5 x_6^6 x_7 x_8^6 x_9 x_{10}^6 x_{11}^6$                                                                                                  | $-1 \cdot 2^3$                                              |
| (2, 6, 2, 1) | (0, 1, 0, 1, 1, 1, 2, 1, 3, 1, 2) | 27  | $x_2^2 x_3 x_4^2 x_5^5 x_6^5 x_7 x_8^5 x_{10}^5 x_{11}$                                                                                                | -1                                                          |
| (2, 5, 2, 2) | (0, 1, 0, 1, 1, 1, 2, 1, 3, 3, 2) | 23  | $x_2^2 x_3 x_4^4 x_5^4 x_6^4 x_7 x_8^4 x_9 x_{10} x_{11}$                                                                                              | $-1 \cdot 2$                                                |
| (2, 4, 2, 3) | (0, 1, 0, 1, 1, 3, 1, 3, 2, 3, 2) | 21  | $x_2^3 x_3 x_4^3 x_5^3 x_6^2 x_7^3 x_8^2 x_9 x_{10}^2 x_{11}$                                                                                          | $-1 \cdot 2 \cdot 3$                                        |
| (2, 6, 3, 0) | (0, 1, 1, 0, 1, 2, 1, 1, 2, 2, 1) | 28  | $x_1 x_3 x_4 x_5^4 x_6^2 x_7^5 x_8^5 x_9^2 x_{10}^2 x_{11}^5$                                                                                          | $-1 \cdot 3^2$                                              |
| (2, 5, 3, 1) | (0, 1, 0, 1, 1, 1, 2, 1, 2, 2, 3) | 24  | $x_1 x_2^4 x_3 x_4^4 x_5^3 x_6^4 x_7^2 x_8^3 x_9^2$                                                                                                    | 1                                                           |

$$S \subseteq \mathbb{Z}_p \times \mathbb{Z}_4 \setminus \{(0, 0)\}, |S| = 11$$

| $\lambda$     | $\mathbf{a}$                      | deg | monomial/s                                                                                                                         | coefficient/s                                                   |
|---------------|-----------------------------------|-----|------------------------------------------------------------------------------------------------------------------------------------|-----------------------------------------------------------------|
| (2, 4, 3, 2)  | (0, 1, 0, 1, 1, 2, 2, 3, 1, 3, 2) | 20  | $x_1 x_2 x_3 x_4^3 x_5^3 x_6^2 x_7^2 x_8 x_9^3 x_{10} x_{11}^2$                                                                    | $-1 \cdot 2$                                                    |
| (2, 3, 3, 3)  | (0, 1, 0, 1, 1, 3, 2, 3, 2, 2, 3) | 20  | $x_1 x_2^2 x_3 x_4^2 x_5^2 x_6^2 x_7^2 x_8^2 x_9^2 x_{10}^2 x_{11}^2$                                                              | $2^2$                                                           |
| (2, 5, 4, 0)  | (0, 1, 1, 0, 1, 1, 2, 1, 2, 2, 2) | 27  | $x_2 x_3 x_4 x_5^4 x_6^4 x_7^3 x_8^4 x_9^3 x_{10}^3 x_{11}^3$                                                                      | $-1 \cdot 2$                                                    |
| (2, 4, 4, 1)  | (0, 1, 0, 1, 1, 2, 2, 3, 2, 2, 1) | 23  | $x_1 x_3 x_4^3 x_5^3 x_6^3 x_7^3 x_8^3 x_{10}^3 x_{11}^3$                                                                          | $-1 \cdot 2^4$                                                  |
| (2, 3, 4, 2)  | (0, 1, 0, 2, 3, 1, 3, 2, 2, 1, 2) | 21  | $x_1 x_2^2 x_3 x_4^2 x_5 x_6^2 x_7 x_8^3 x_9^3 x_{10}^2 x_{11}^3$                                                                  | $-1 \cdot 2^2$                                                  |
| (2, 4, 5, 0)  | (0, 1, 1, 0, 1, 2, 2, 2, 2, 1, 2) | 27  | $x_3^3 x_4 x_5^2 x_6^2 x_7^4 x_8^4 x_9^4 x_{10}^3 x_{11}^4$                                                                        | $-1 \cdot 2$                                                    |
| (2, 3, 5, 1)  | (0, 1, 1, 0, 1, 2, 2, 2, 2, 3, 2) | 23  | $x_1 x_3 x_4 x_5^2 x_6^2 x_7^4 x_8^4 x_9^4 x_{11}^4$                                                                               | 2                                                               |
| (2, 2, 5, 2)  | (0, 1, 0, 2, 2, 2, 3, 2, 2, 1, 3) | 23  | $x_3 x_4^3 x_5^4 x_6^4 x_7 x_8^4 x_9^4 x_{10} x_{11}$                                                                              | $-1 \cdot 3$                                                    |
| (2, 3, 6, 0)  | (0, 1, 1, 0, 2, 2, 1, 2, 2, 2, 2) | 29  | $x_3 x_4 x_5^2 x_6^4 x_7^2 x_8^4 x_9^5 x_{10}^5 x_{11}^5$                                                                          | 1                                                               |
| (2, 2, 6, 1)  | (0, 1, 2, 2, 2, 3, 0, 2, 2, 1, 2) | 27  | $x_2 x_4^4 x_5^5 x_7 x_8^5 x_9^5 x_{10} x_{11}^5$                                                                                  | $2^2$                                                           |
| (2, 2, 7, 0)  | (0, 2, 0, 1, 2, 2, 2, 2, 2, 1, 2) | 32  | $x_1 x_3 x_5 x_6^4 x_7^6 x_8^6 x_9^6 x_{10} x_{11}^6$                                                                              | 2                                                               |
| (2, 1, 7, 1)  | (0, 1, 2, 2, 2, 2, 2, 3, 0, 2, 2) | 32  | $x_4^2 x_5^5 x_6^6 x_7^6 x_9 x_{10}^6 x_{11}^6$                                                                                    | 3                                                               |
| (2, 1, 8, 0)  | (0, 2, 0, 2, 2, 1, 2, 2, 2, 2, 2) | 39  | $x_3 x_4^3 x_5^4 x_7^4 x_8^6 x_9^7 x_{10}^7 x_{11}^7$                                                                              | 1                                                               |
| (2, 0, 9, 0)  | (0, 2, 0, 2, 2, 2, 2, 2, 2, 2, 2) | 65  | $x_2^2 x_3 x_4^6 x_5^8 x_6^8 x_7^8 x_8^8 x_9^8 x_{10}^8 x_{11}^8$<br>$x_3^3 x_4^5 x_5^8 x_6^8 x_7^8 x_8^8 x_9^8 x_{10}^8 x_{11}^8$ | $-1 \cdot 2^2 \cdot 8069$<br>$-1 \cdot 2^2 \cdot 11 \cdot 2089$ |
| (1, 10, 0, 0) | (1, 1, 1, 0, 1, 1, 1, 1, 1, 1, 1) | 56  | $x_1 x_2^3 x_3^3 x_5^5 x_6^8 x_8^9 x_9^9 x_{10}^9 x_{11}^9$                                                                        | $-1 \cdot 2$                                                    |
| (1, 9, 0, 1)  | (1, 0, 1, 1, 1, 1, 1, 1, 3, 1, 1) | 46  | $x_1 x_3^2 x_4^4 x_5^7 x_6^8 x_8^8 x_{10}^8 x_{11}^8$                                                                              | $-1 \cdot 3$                                                    |
| (1, 8, 0, 2)  | (1, 0, 1, 1, 1, 3, 1, 1, 1, 1, 3) | 40  | $x_3^2 x_4^2 x_5^6 x_6 x_7^7 x_8^7 x_9^7 x_{10}^7 x_{11}$                                                                          | $-1 \cdot 2$                                                    |
| (1, 7, 0, 3)  | (1, 0, 1, 1, 1, 3, 3, 3, 1, 1, 1) | 34  | $x_3 x_4^3 x_5^6 x_6^2 x_7^2 x_8^2 x_9^6 x_{10}^6 x_{11}^6$                                                                        | $2 \cdot 3$                                                     |
| (1, 6, 0, 4)  | (1, 0, 1, 1, 1, 1, 3, 3, 3, 1, 3) | 32  | $x_3^2 x_4^3 x_5^5 x_6^5 x_7^3 x_8^3 x_9^3 x_{10}^3 x_{11}^3$                                                                      | $-1 \cdot 2$                                                    |
| (1, 5, 0, 5)  | (1, 0, 1, 1, 1, 1, 3, 3, 1, 3, 3) | 30  | $x_3 x_4^3 x_5^4 x_6^2 x_7^4 x_8^4 x_9^4 x_{10}^4 x_{11}^4$                                                                        | $-1 \cdot 2$                                                    |
| (1, 9, 1, 0)  | (0, 1, 1, 1, 1, 1, 1, 1, 2, 1, 1) | 47  | $x_2 x_3^2 x_4^4 x_5^8 x_6^8 x_8^8 x_{10}^8 x_{11}^8$                                                                              | $2^2$                                                           |
| (1, 8, 1, 1)  | (0, 1, 1, 1, 1, 1, 1, 1, 3, 1, 2) | 39  | $x_2 x_3 x_4^3 x_5^6 x_6^7 x_7^7 x_8^7 x_{10}^7$                                                                                   | $-1 \cdot 3$                                                    |
| (1, 7, 1, 2)  | (0, 1, 1, 1, 1, 3, 2, 1, 3, 1, 1) | 33  | $x_3^2 x_4^5 x_5^6 x_6^6 x_8 x_9 x_{10}^6 x_{11}^6$                                                                                | $-1 \cdot 2^2 \cdot 3$                                          |
| (1, 6, 1, 3)  | (0, 1, 1, 1, 1, 1, 2, 3, 1, 3, 3) | 29  | $x_2 x_3^2 x_4^5 x_5^5 x_6^5 x_8^2 x_9^5 x_{10}^2 x_{11}^2$                                                                        | $-1 \cdot 5$                                                    |
| (1, 5, 1, 4)  | (0, 1, 1, 1, 1, 3, 3, 3, 1, 3, 2) | 27  | $x_2 x_3^2 x_4^4 x_5^4 x_6^3 x_7^3 x_8^3 x_9^4 x_{10}^3$                                                                           | $-1 \cdot 2$                                                    |

$$S \subseteq \mathbb{Z}_p \times \mathbb{Z}_4 \setminus \{(0, 0)\}, |S| = 11$$

| $\lambda$     | $\mathbf{a}$                      | deg | monomial/s                                                                                                     | coefficient/s                                    |
|---------------|-----------------------------------|-----|----------------------------------------------------------------------------------------------------------------|--------------------------------------------------|
| (1, 8, 2, 0)  | (1, 0, 1, 1, 1, 2, 1, 2, 1, 1, 1) | 39  | $x_3x_4^2x_5^6x_6x_7^7x_8x_9^7x_{10}^7x_{11}^7$                                                                | -1                                               |
| (1, 7, 2, 1)  | (0, 1, 1, 1, 1, 1, 2, 3, 1, 2, 1) | 33  | $x_3^2x_4^5x_5^6x_6^6x_7x_9^6x_{10}x_{11}^6$                                                                   | $2^3$                                            |
| (1, 6, 2, 2)  | (1, 0, 1, 1, 1, 1, 2, 3, 1, 3, 2) | 27  | $x_3^3x_4^5x_5^5x_6^5x_7x_8x_9^5x_{10}x_{11}$                                                                  | $-1 \cdot 2 \cdot 3$                             |
| (1, 5, 2, 3)  | (0, 1, 1, 1, 1, 1, 2, 3, 3, 2, 3) | 25  | $x_2x_3^4x_4^4x_5^4x_6^4x_7x_8^2x_9^2x_{10}x_{11}^2$                                                           | 2                                                |
| (1, 4, 2, 4)  | (1, 0, 1, 1, 2, 3, 3, 3, 1, 3, 2) | 23  | $x_3^3x_4^3x_5x_6^3x_7^3x_8^3x_9^3x_{10}x_{11}$                                                                | $2^2 \cdot 3$                                    |
| (1, 7, 3, 0)  | (0, 1, 1, 1, 1, 2, 1, 2, 1, 1, 2) | 35  | $x_2x_3x_4^3x_5^6x_6^2x_7^6x_8^2x_9^6x_{10}^6x_{11}^2$                                                         | $-1 \cdot 2$                                     |
| (1, 6, 3, 1)  | (0, 1, 1, 1, 1, 2, 1, 2, 1, 3, 2) | 29  | $x_3^3x_4^5x_5^5x_6^2x_7^5x_8^2x_9^5x_{11}^2$                                                                  | $-1 \cdot 2 \cdot 3$                             |
| (1, 5, 3, 2)  | (0, 1, 1, 1, 1, 2, 1, 2, 2, 3, 3) | 25  | $x_2x_3^4x_4^4x_5^4x_6^2x_7^4x_8^2x_9^2x_{10}x_{11}$                                                           | $-1 \cdot 2$                                     |
| (1, 4, 3, 3)  | (0, 1, 1, 1, 2, 1, 2, 3, 3, 3, 2) | 23  | $x_2^2x_3^3x_4^3x_5^2x_6^3x_7^2x_8^2x_9^2x_{10}^2x_{11}^2$                                                     | $2^2$                                            |
| (1, 6, 4, 0)  | (0, 1, 1, 1, 1, 2, 1, 2, 2, 2, 1) | 32  | $x_2^2x_3^3x_4^5x_6^3x_7^5x_8^3x_9^3x_{10}^3x_{11}^5$                                                          | $-1 \cdot 2^3$                                   |
| (1, 5, 4, 1)  | (1, 0, 1, 1, 1, 2, 1, 2, 2, 3, 2) | 26  | $x_2^2x_3^4x_4^4x_5^3x_6^4x_7^4x_8^3x_9^3x_{11}^3$                                                             | $2 \cdot 3$                                      |
| (1, 4, 4, 2)  | (0, 1, 1, 1, 2, 1, 2, 3, 2, 2, 3) | 24  | $x_2x_3^3x_4^3x_5^3x_6^3x_7^3x_8^3x_9^3x_{10}x_{11}$                                                           | $2^3$                                            |
| (1, 3, 4, 3)  | (1, 0, 1, 1, 2, 2, 3, 2, 3, 3, 2) | 22  | $x_2^2x_3^2x_4^3x_5^3x_6^3x_7^2x_8^3x_9^2x_{10}^3x_{11}^3$                                                     | $-1 \cdot 2 \cdot 3^2$                           |
| (1, 5, 5, 0)  | (0, 1, 1, 1, 2, 1, 2, 2, 1, 2, 2) | 31  | $x_3x_4^3x_5^3x_6^4x_7^4x_8^4x_9^4x_{10}^4x_{11}^4$                                                            | 3                                                |
| (1, 4, 5, 1)  | (0, 1, 1, 1, 2, 2, 3, 2, 2, 1, 2) | 27  | $x_2x_3x_4^2x_5^4x_6^4x_7^4x_8^4x_9^3x_{10}^3x_{11}^4$                                                         | $-1 \cdot 2$                                     |
| (1, 3, 5, 2)  | (0, 1, 1, 2, 2, 1, 2, 2, 3, 3, 2) | 25  | $x_3x_4^4x_5^4x_6^2x_7^4x_8^4x_9x_{10}x_{11}^4$                                                                | $2 \cdot 3$                                      |
| (1, 4, 6, 0)  | (1, 1, 0, 1, 2, 2, 2, 2, 1, 2, 2) | 31  | $x_2x_4^2x_5x_6^4x_7^5x_8^3x_9^5x_{10}^5x_{11}^5$                                                              | $-1 \cdot 3$                                     |
| (1, 3, 6, 1)  | (0, 1, 1, 1, 2, 2, 2, 2, 3, 2, 2) | 29  | $x_3^2x_4^2x_5x_6^4x_7^5x_8^5x_{10}^5x_{11}^5$                                                                 | 3                                                |
| (1, 2, 6, 2)  | (1, 0, 2, 2, 2, 3, 2, 2, 1, 3, 2) | 27  | $x_4^4x_5^5x_6x_7^5x_8^5x_9x_{10}x_{11}^5$                                                                     | $2^2$                                            |
| (1, 3, 7, 0)  | (0, 2, 1, 2, 1, 2, 2, 1, 2, 2, 2) | 35  | $x_4^2x_5^2x_6^5x_7^6x_8^2x_9^6x_{10}^6x_{11}^6$                                                               | 3                                                |
| (1, 2, 7, 1)  | (0, 2, 1, 2, 1, 2, 2, 3, 2, 2, 2) | 33  | $x_3x_4^2x_5x_6^5x_7^6x_9^6x_{10}^6x_{11}^6$                                                                   | 3                                                |
| (1, 2, 8, 0)  | (0, 2, 1, 2, 2, 2, 2, 2, 1, 2, 2) | 40  | $x_2x_4x_5^3x_6^6x_7^7x_8^7x_9x_{10}^7x_{11}^7$                                                                | 3                                                |
| (1, 1, 8, 1)  | (1, 2, 2, 2, 2, 2, 3, 0, 2, 2, 2) | 38  | $x_2^2x_3^3x_4^6x_5^7x_6^6x_7^6x_{10}^7x_{11}^7$                                                               | 5                                                |
| (1, 1, 9, 0)  | (2, 0, 2, 2, 2, 1, 2, 2, 2, 2, 2) | 47  | $x_1x_3^3x_4^5x_5^7x_6^8x_7^8x_9^8x_{10}^8x_{11}^8$                                                            | 1                                                |
| (1, 0, 10, 0) | (2, 0, 2, 2, 2, 2, 2, 2, 2, 2, 2) | 73  | $x_1^8x_3^8x_4^8x_5^9x_7^8x_8^5x_9^9x_{10}^9x_{11}^9$<br>$x_1^8x_3^8x_4^9x_5^8x_7^8x_8^9x_9^9x_{10}^9x_{11}^9$ | $-1 \cdot 3 \cdot 5 \cdot 11$<br>$5 \cdot 77863$ |

$$S \subseteq \mathbb{Z}_p \times \mathbb{Z}_4 \setminus \{(0, 0)\}, |S| = 11$$

| $\lambda$     | $\mathbf{a}$                         | deg | monomial/s                                                                    | coefficient/s  |
|---------------|--------------------------------------|-----|-------------------------------------------------------------------------------|----------------|
| (0, 11, 0, 0) | (1, 1, 1, 1, 1, 1, 1, 1, 1, 1, 1)    | 67  | $x_1 x_2^3 x_3^4 x_4^5 x_5^8 x_6^9 x_7^9 x_8^9 x_9^9 x_{10}^{10} x_{11}^{10}$ | 7              |
| (0, 10, 0, 1) | (1, 1, 1, 1, 1, 1, 1, 3, 1, 1, 1)    | 57  | $x_1^2 x_2^2 x_3^3 x_4^8 x_5^8 x_6^8 x_7^8 x_8^9 x_9^9 x_{10}^9 x_{11}^9$     | -1             |
| (0, 9, 0, 2)  | (1, 1, 1, 1, 3, 1, 1, 1, 3, 1, 1)    | 49  | $x_1 x_2^3 x_3^4 x_4^8 x_5^8 x_6^8 x_7^8 x_8^8 x_9^8 x_{10}^8 x_{11}^8$       | 2              |
| (0, 8, 0, 3)  | (1, 1, 1, 1, 3, 1, 1, 1, 1, 3, 3)    | 43  | $x_1^2 x_2^2 x_3^5 x_4^7 x_5^2 x_6^7 x_7^7 x_8^7 x_9^7 x_{10}^2 x_{11}^2$     | $2^5$          |
| (0, 7, 0, 4)  | (1, 1, 1, 3, 3, 1, 1, 1, 1, 3, 3, 3) | 39  | $x_2 x_3^4 x_4^2 x_5^5 x_6^6 x_7^6 x_8^6 x_9^3 x_{10}^3 x_{11}^3$             | 2              |
| (0, 6, 0, 5)  | (1, 1, 1, 1, 1, 3, 3, 3, 1, 3, 3)    | 37  | $x_1 x_2 x_3^3 x_4^5 x_5^5 x_6^2 x_7^3 x_8^4 x_9^5 x_{10}^4 x_{11}^4$         | -1             |
| (0, 10, 1, 0) | (1, 1, 1, 1, 1, 1, 1, 2, 1, 1, 1)    | 56  | $x_1 x_2^2 x_3^4 x_4^6 x_5^7 x_6^9 x_7^9 x_8^9 x_9^9 x_{10}^9 x_{11}^9$       | 2              |
| (0, 9, 1, 1)  | (1, 1, 1, 1, 1, 1, 1, 1, 1, 2, 3)    | 48  | $x_1^2 x_2^3 x_3^4 x_4^7 x_5^8 x_6^8 x_7^8 x_8^8 x_9^8$                       | 3              |
| (0, 8, 1, 2)  | (1, 1, 1, 1, 1, 1, 1, 3, 1, 2, 3)    | 40  | $x_2 x_3^3 x_4^6 x_5^7 x_6^7 x_7^7 x_8^7 x_9^7 x_{10}^7 x_{11}^7$             | $-1 \cdot 3$   |
| (0, 7, 1, 3)  | (1, 1, 1, 1, 1, 1, 1, 2, 3, 3, 3)    | 36  | $x_1 x_2^2 x_3^3 x_4^6 x_5^6 x_6^6 x_7^6 x_8^2 x_9^2 x_{10}^2 x_{11}^2$       | 2              |
| (0, 6, 1, 4)  | (1, 1, 1, 1, 1, 2, 3, 1, 3, 3, 3)    | 32  | $x_2 x_3^4 x_4^5 x_5^5 x_7^3 x_8^3 x_9^3 x_{10}^3 x_{11}^3$                   | -1             |
| (0, 5, 1, 5)  | (1, 1, 1, 1, 1, 2, 3, 3, 3, 3, 3)    | 32  | $x_1 x_2^2 x_3^3 x_4^4 x_5^4 x_7^2 x_8^4 x_9^4 x_{10}^4 x_{11}^4$             | 2              |
| (0, 9, 2, 0)  | (1, 1, 1, 1, 1, 1, 1, 1, 2, 1, 2)    | 49  | $x_1^2 x_2^2 x_3^3 x_4^8 x_5^8 x_6^8 x_7^8 x_8^8 x_9^8 x_{10}^8 x_{11}^8$     | $-1 \cdot 2$   |
| (0, 8, 2, 1)  | (1, 1, 1, 1, 1, 1, 1, 2, 3, 2, 1)    | 41  | $x_2 x_3^3 x_4^7 x_5^7 x_6^7 x_7^7 x_8^7 x_{10}^7 x_{11}^7$                   | $-1 \cdot 2^2$ |
| (0, 7, 2, 2)  | (1, 1, 1, 1, 1, 1, 1, 3, 2, 3, 2)    | 35  | $x_1 x_2^2 x_3^4 x_4^6 x_5^6 x_6^6 x_7^6 x_8^6 x_9^6 x_{10}^6 x_{11}^6$       | $-1 \cdot 2$   |
| (0, 6, 2, 3)  | (1, 1, 1, 1, 1, 1, 2, 3, 3, 3, 2)    | 31  | $x_1 x_2^2 x_3^5 x_4^5 x_5^5 x_6^5 x_7^2 x_8^2 x_9^2 x_{10}^2 x_{11}^2$       | $-1 \cdot 2$   |
| (0, 5, 2, 4)  | (1, 1, 1, 1, 2, 3, 2, 1, 3, 3, 3)    | 29  | $x_1^4 x_2^4 x_3^4 x_4^4 x_5^3 x_6^3 x_7^3 x_8^3 x_9^2 x_{10}^2$              | 2              |
| (0, 8, 3, 0)  | (1, 1, 1, 1, 1, 1, 1, 2, 2, 1, 2)    | 43  | $x_2^2 x_3^2 x_4^6 x_5^6 x_6^7 x_7^7 x_8^2 x_9^2 x_{10}^2 x_{11}^2$           | $-1 \cdot 2$   |
| (0, 7, 3, 1)  | (1, 1, 1, 1, 1, 1, 1, 2, 2, 3, 2)    | 35  | $x_2 x_3^4 x_4^6 x_5^6 x_6^6 x_7^2 x_8^2 x_9^2 x_{10}^2 x_{11}^2$             | $-1 \cdot 2$   |
| (0, 6, 3, 2)  | (1, 1, 1, 1, 1, 2, 1, 2, 3, 2, 3)    | 31  | $x_2^3 x_3^5 x_4^5 x_5^5 x_6^2 x_7^2 x_8^2 x_9^2 x_{10}^2 x_{11}^2$           | $-1 \cdot 2^3$ |
| (0, 5, 3, 3)  | (1, 1, 1, 1, 1, 2, 3, 3, 2, 3, 2)    | 27  | $x_1^4 x_2^4 x_3^3 x_4^4 x_5^3 x_6^2 x_7^2 x_8^2 x_9^2 x_{10}^2$              | -1             |
| (0, 4, 3, 4)  | (1, 1, 1, 2, 1, 2, 3, 2, 3, 3, 3)    | 27  | $x_2^3 x_3^3 x_4^2 x_5^3 x_6^3 x_7^3 x_8^3 x_9^3 x_{10}^3 x_{11}^3$           | 2              |
| (0, 7, 4, 0)  | (1, 1, 1, 1, 1, 1, 2, 2, 1, 2, 2)    | 39  | $x_2 x_3^3 x_4^5 x_5^6 x_6^6 x_7^3 x_8^3 x_9^3 x_{10}^3 x_{11}^3$             | $-1 \cdot 2^3$ |
| (0, 6, 4, 1)  | (1, 1, 1, 1, 1, 2, 3, 2, 2, 1, 2)    | 33  | $x_1^5 x_2^5 x_3^4 x_4^5 x_5^4 x_6^3 x_7^3 x_8^3 x_9^3 x_{10}^3$              | -1             |
| (0, 5, 4, 2)  | (1, 1, 1, 1, 1, 2, 3, 2, 2, 3, 2)    | 29  | $x_1 x_2^2 x_3^4 x_4^4 x_5^4 x_6^3 x_7^3 x_8^3 x_9^3 x_{10}^3 x_{11}^3$       | $2 \cdot 3$    |
| (0, 4, 4, 3)  | (1, 1, 1, 2, 1, 2, 3, 3, 2, 3, 2)    | 27  | $x_1 x_2^2 x_3^3 x_4^3 x_5^3 x_6^2 x_7^2 x_8^2 x_9^2 x_{10}^2 x_{11}^2$       | $2^4$          |

$$S \subseteq \mathbb{Z}_p \times \mathbb{Z}_4 \setminus \{(0, 0)\}, |S| = 11$$

| $\lambda$     | $\mathbf{a}$                      | deg | monomial/s                                                                                                                                                         | coefficient/s                                  |
|---------------|-----------------------------------|-----|--------------------------------------------------------------------------------------------------------------------------------------------------------------------|------------------------------------------------|
| (0, 6, 5, 0)  | (1, 1, 1, 1, 2, 1, 2, 2, 2, 1, 2) | 36  | $x_2x_3^2x_4^5x_5^2x_6^5x_7^4x_8^4x_9^4x_{10}^5x_{11}^4$                                                                                                           | $2^2$                                          |
| (0, 5, 5, 1)  | (1, 1, 1, 1, 1, 2, 2, 2, 3, 2, 2) | 32  | $x_1x_2^2x_3^2x_4^4x_5^4x_6^3x_7^4x_8^4x_{10}^4x_{11}^4$                                                                                                           | $-1 \cdot 3$                                   |
| (0, 4, 5, 2)  | (1, 1, 1, 2, 1, 2, 3, 2, 2, 3, 2) | 28  | $x_2x_3^2x_4^4x_5^3x_6^4x_7x_8^4x_9^4x_{10}x_{11}^4$                                                                                                               | $2^2 \cdot 3$                                  |
| (0, 3, 5, 3)  | (1, 1, 1, 2, 2, 2, 3, 2, 2, 3, 3) | 28  | $x_2^2x_3^2x_4^2x_5^4x_6^4x_7^2x_8^4x_9^4x_{10}^2x_{11}^2$                                                                                                         | $2^2 \cdot 3$                                  |
| (0, 5, 6, 0)  | (1, 1, 1, 1, 2, 2, 2, 1, 2, 2, 2) | 37  | $x_1x_2x_3^2x_4^4x_5x_6^4x_7^5x_8^4x_9^5x_{10}^5x_{11}^5$                                                                                                          | 3                                              |
| (0, 4, 6, 1)  | (1, 1, 1, 2, 1, 2, 2, 2, 3, 2, 2) | 33  | $x_2x_3^3x_4^2x_5^3x_6^4x_7^5x_8^5x_{10}^5x_{11}^5$                                                                                                                | 3                                              |
| (0, 3, 6, 2)  | (1, 1, 1, 2, 2, 3, 2, 2, 2, 3, 2) | 31  | $x_1x_2x_3^2x_4^2x_5^3x_6^5x_7^5x_8^5x_9^5x_{10}x_{11}^5$                                                                                                          | $-1 \cdot 2^2$                                 |
| (0, 4, 7, 0)  | (1, 1, 1, 2, 2, 2, 2, 1, 2, 2, 2) | 39  | $x_2^2x_3^2x_4x_5^2x_6^5x_7^6x_8^3x_9^6x_{10}^6x_{11}^6$                                                                                                           | 3                                              |
| (0, 3, 7, 1)  | (1, 1, 1, 2, 2, 2, 2, 3, 2, 2, 2) | 35  | $x_2x_3^2x_4x_5^2x_6^5x_7^6x_8^6x_{10}^6x_{11}^6$                                                                                                                  | $-1 \cdot 3$                                   |
| (0, 2, 7, 2)  | (1, 2, 1, 2, 2, 2, 3, 2, 2, 2, 3) | 35  | $x_2x_3x_4^2x_5^5x_6^6x_7x_8^6x_9^6x_{10}^6x_{11}^6$                                                                                                               | $-1 \cdot 3$                                   |
| (0, 3, 8, 0)  | (1, 1, 2, 2, 2, 2, 1, 2, 2, 2, 2) | 43  | $x_2x_3x_4^2x_5^4x_6^6x_7^2x_8^6x_9^7x_{10}^7x_{11}^7$                                                                                                             | 1                                              |
| (0, 2, 8, 1)  | (1, 2, 2, 2, 3, 2, 2, 2, 2, 1, 2) | 41  | $x_1x_3^3x_4^3x_5^5x_6^7x_7^7x_8^7x_{10}x_{11}^7$                                                                                                                  | $-1 \cdot 2$                                   |
| (0, 2, 9, 0)  | (2, 1, 2, 2, 2, 2, 2, 1, 2, 2, 2) | 48  | $x_1x_3^2x_4^5x_5^7x_6^8x_8x_9^8x_{10}^8x_{11}^8$                                                                                                                  | 3                                              |
| (0, 1, 9, 1)  | (1, 2, 2, 2, 2, 2, 3, 2, 2, 2, 2) | 48  | $x_3^2x_4^3x_5^5x_6^7x_8^7x_9^8x_{10}^8x_{11}^8$                                                                                                                   | 1                                              |
| (0, 1, 10, 0) | (2, 2, 2, 2, 2, 1, 2, 2, 2, 2, 2) | 57  | $x_1x_2^3x_3^4x_4^6x_5^8x_8^8x_9^9x_{10}^9x_{11}^9$                                                                                                                | -1                                             |
| (0, 0, 11, 0) | (2, 2, 2, 2, 2, 2, 2, 2, 2, 2, 2) | 85  | $x_1^3x_2^4x_3^8x_4^{10}x_5^{10}x_6^{10}x_8^{10}x_9^{10}x_{10}^{10}x_{11}^{10}$<br>$x_1^3x_2^4x_3^9x_4^{10}x_5^{10}x_6^{10}x_8^{10}x_9^{10}x_{10}^{10}x_{11}^{10}$ | $-1 \cdot 2^2 \cdot 74257$<br>$-1 \cdot 90997$ |

$$S \subseteq \mathbb{Z}_p \times \mathbb{Z}_5 \setminus \{(0, 0)\}, |S| = 11$$

| $\lambda$        | $\mathbf{a}$                      | deg | monomial/s                                                                                                                                                                                     | coefficient/s                                                                                                  |
|------------------|-----------------------------------|-----|------------------------------------------------------------------------------------------------------------------------------------------------------------------------------------------------|----------------------------------------------------------------------------------------------------------------|
| (11, 0, 0, 0, 0) | (0, 0, 0, 0, 0, 0, 0, 0, 0, 0, 0) | 109 | $x_1^9x_2^{10}x_3^{10}x_4^{10}x_5^{10}x_6^{10}x_7^{10}x_8^{10}x_9^{10}x_{10}^{10}x_{11}^{10}$<br>$x_1^{10}x_2^9x_3^{10}x_4^{10}x_5^{10}x_6^{10}x_7^{10}x_8^{10}x_9^{10}x_{10}^{10}x_{11}^{10}$ | $-1 \cdot 2^3 \cdot 5 \cdot 11 \cdot 3019 \cdot 13647452681$<br>$-1 \cdot 2^3 \cdot 3^2 \cdot 644208651072689$ |
| (10, 1, 0, 0, 0) | (0, 0, 0, 0, 0, 1, 0, 0, 0, 0, 0) | 65  | $x_1x_2^3x_3^7x_4^9x_5^9x_8^9x_9^9x_{10}^9x_{11}^9$<br>$x_1x_2^4x_3^6x_4^9x_5^9x_8^9x_9^9x_{10}^9x_{11}^9$                                                                                     | $-1 \cdot 2^2 \cdot 3 \cdot 7 \cdot 11$<br>$-1 \cdot 2^2 \cdot 5^2 \cdot 23$                                   |
| (9, 2, 0, 0, 0)  | (0, 0, 0, 1, 0, 0, 0, 1, 0, 0, 0) | 46  | $x_1x_2^3x_3^5x_5^5x_6^8x_8x_9^7x_{10}^8x_{11}^8$                                                                                                                                              | $-1 \cdot 2$                                                                                                   |
| (9, 1, 1, 0, 0)  | (0, 0, 0, 1, 0, 0, 0, 2, 0, 0, 0) | 45  | $x_1x_2^3x_3^5x_5^5x_6^8x_9^7x_{10}^8x_{11}^8$                                                                                                                                                 | $-1 \cdot 2$                                                                                                   |
| (9, 1, 0, 0, 1)  | (0, 1, 0, 0, 0, 0, 0, 4, 0, 0, 0) | 56  | $x_1^2x_3^6x_4^8x_5^8x_6^8x_8^8x_{10}^8x_{11}^8$<br>$x_1^3x_3^5x_4^8x_5^8x_6^8x_9^8x_{10}^8x_{11}^8$                                                                                           | $2 \cdot 227$<br>$-1 \cdot 2 \cdot 5 \cdot 17$                                                                 |
| (8, 3, 0, 0, 0)  | (0, 0, 1, 0, 0, 1, 0, 0, 1, 0, 0) | 35  | $x_1x_2^3x_3^3x_4^5x_5x_6x_8^7x_9^2x_{10}^6x_{11}^7$                                                                                                                                           | -1                                                                                                             |

$$S \subseteq \mathbb{Z}_p \times \mathbb{Z}_5 \setminus \{(0, 0)\}, |S| = 11$$

| $\lambda$       | $\mathbf{a}$                      | deg | monomial/s                                                    | coefficient/s |
|-----------------|-----------------------------------|-----|---------------------------------------------------------------|---------------|
| (8, 2, 1, 0, 0) | (0, 0, 1, 0, 0, 1, 0, 0, 2, 0, 0) | 33  | $x_1 x_2^3 x_4^3 x_5^5 x_6^7 x_8^6 x_{10}^7 x_{11}^7$         | -1            |
| (8, 2, 0, 1, 0) | (0, 0, 3, 0, 0, 0, 1, 0, 0, 0, 1) | 38  | $x_1 x_2^3 x_4^2 x_5^4 x_6^7 x_8^6 x_9^7 x_{10}^7 x_{11}$     | 1             |
| (8, 2, 0, 0, 1) | (0, 0, 0, 1, 0, 0, 1, 0, 0, 0, 4) | 39  | $x_2^2 x_3^5 x_4 x_5^4 x_6^7 x_8^6 x_9^7 x_{10}^7$            | 1             |
| (8, 1, 1, 1, 0) | (0, 0, 3, 0, 0, 1, 0, 0, 2, 0, 0) | 32  | $x_1 x_2^3 x_4^3 x_5^5 x_8^7 x_{10}^6 x_{11}^7$               | -1            |
| (7, 4, 0, 0, 0) | (0, 0, 1, 0, 1, 0, 0, 1, 0, 1, 0) | 29  | $x_1 x_2^3 x_4^3 x_5 x_6^5 x_8^2 x_9^5 x_{10}^3 x_{11}^6$     | 1             |
| (7, 3, 1, 0, 0) | (2, 0, 0, 1, 0, 0, 1, 0, 0, 1, 0) | 28  | $x_3^2 x_4 x_5^2 x_6^4 x_8^5 x_9^6 x_{10}^2 x_{11}^6$         | -1            |
| (7, 3, 0, 1, 0) | (0, 0, 1, 1, 0, 0, 1, 0, 0, 3, 0) | 29  | $x_2^2 x_3^2 x_4^2 x_5^2 x_6^4 x_8^5 x_9^6 x_{11}^6$          | -1            |
| (7, 3, 0, 0, 1) | (0, 0, 1, 0, 0, 1, 1, 0, 0, 4, 0) | 29  | $x_2^2 x_3 x_4^2 x_5^5 x_6^2 x_8^5 x_9^6 x_{11}^6$            | -1            |
| (7, 2, 2, 0, 0) | (0, 2, 0, 0, 1, 0, 0, 1, 0, 2, 0) | 25  | $x_1 x_2^3 x_4^4 x_6^5 x_8^5 x_{10} x_{11}^6$                 | 1             |
| (7, 2, 1, 1, 0) | (0, 1, 0, 0, 2, 0, 1, 0, 0, 3, 0) | 24  | $x_2 x_3 x_4^3 x_6^3 x_8^4 x_9^6 x_{11}^6$                    | -1            |
| (7, 2, 1, 0, 1) | (0, 1, 0, 1, 0, 0, 2, 0, 0, 4, 0) | 24  | $x_3 x_4 x_5^2 x_6^4 x_8^4 x_9^6 x_{11}^6$                    | 1             |
| (7, 2, 0, 1, 1) | (0, 1, 0, 0, 1, 0, 0, 3, 4, 0, 0) | 27  | $x_1 x_3^3 x_4^5 x_5 x_6^6 x_{10}^5 x_{11}^6$                 | -1            |
| (7, 2, 0, 0, 2) | (0, 0, 1, 0, 0, 1, 0, 0, 0, 4, 4) | 33  | $x_1 x_2^3 x_4^3 x_5^6 x_6^5 x_7^6 x_8^6 x_9^6 x_{10} x_{11}$ | 1             |
| (7, 1, 1, 1, 1) | (0, 4, 0, 0, 3, 0, 0, 1, 0, 0, 2) | 25  | $x_1^2 x_3^2 x_4^4 x_6^6 x_9^5 x_{10}^6$                      | 1             |
| (6, 5, 0, 0, 0) | (0, 1, 0, 0, 1, 0, 1, 0, 1, 0, 1) | 27  | $x_1 x_2 x_3 x_4^3 x_5^2 x_6^3 x_8^4 x_9^3 x_{10}^5 x_{11}^4$ | -1            |
| (6, 4, 1, 0, 0) | (0, 1, 0, 1, 0, 1, 0, 0, 1, 0, 2) | 24  | $x_1 x_2 x_3^3 x_4 x_5^3 x_6^2 x_8^5 x_9^3 x_{10}^5$          | -1            |
| (6, 4, 0, 1, 0) | (0, 1, 0, 0, 1, 1, 0, 1, 0, 3, 0) | 24  | $x_1 x_3^2 x_4^4 x_5^2 x_6^2 x_8^3 x_9^5 x_{11}^5$            | 1             |
| (6, 4, 0, 0, 1) | (4, 0, 1, 0, 1, 0, 1, 0, 1, 0, 0) | 24  | $x_3^2 x_4^2 x_5^2 x_6^4 x_8^3 x_9^4 x_{10} x_{11}^5$         | -1            |
| (6, 3, 2, 0, 0) | (0, 1, 0, 2, 0, 0, 1, 0, 1, 2, 0) | 22  | $x_2 x_3 x_5^2 x_6^5 x_8^5 x_9^2 x_{10} x_{11}^5$             | -1            |
| (6, 3, 1, 1, 0) | (0, 1, 0, 0, 1, 2, 0, 0, 3, 1, 0) | 21  | $x_3 x_4^3 x_5 x_7^4 x_8^5 x_{10}^2 x_{11}^5$                 | 1             |
| (6, 3, 1, 0, 1) | (0, 0, 1, 0, 0, 1, 0, 2, 4, 0, 1) | 21  | $x_2^2 x_4^2 x_5^4 x_6 x_7^5 x_{10}^5 x_{11}^2$               | -1            |
| (6, 3, 0, 2, 0) | (0, 1, 0, 1, 0, 1, 0, 0, 3, 3, 0) | 22  | $x_1 x_3^3 x_4 x_5^3 x_6^2 x_8^5 x_9 x_{10} x_{11}^5$         | 1             |
| (6, 3, 0, 1, 1) | (1, 0, 0, 3, 0, 4, 0, 0, 1, 1, 0) | 23  | $x_3^2 x_5^3 x_7^4 x_8^5 x_9^2 x_{10}^5 x_{11}^5$             | -1            |
| (6, 3, 0, 0, 2) | (0, 4, 0, 0, 1, 1, 1, 0, 0, 4, 0) | 25  | $x_3 x_4^3 x_5^2 x_6^2 x_7^4 x_8^5 x_9^5 x_{10} x_{11}^5$     | -1            |
| (6, 2, 2, 1, 0) | (0, 2, 0, 1, 3, 0, 2, 0, 1, 0, 0) | 20  | $x_3 x_6^3 x_7 x_8^5 x_9 x_{10}^4 x_{11}^5$                   | -1            |

$$S \subseteq \mathbb{Z}_p \times \mathbb{Z}_5 \setminus \{(0, 0)\}, |S| = 11$$

| $\lambda$       | $\mathbf{a}$                      | deg | monomial/s                                                      | coefficient/s |
|-----------------|-----------------------------------|-----|-----------------------------------------------------------------|---------------|
| (6, 2, 2, 0, 1) | (0, 1, 0, 2, 0, 4, 0, 2, 0, 0, 1) | 19  | $x_1 x_3 x_5^2 x_7^4 x_8 x_9^4 x_{10}^5 x_{11}$                 | 1             |
| (6, 2, 1, 1, 1) | (0, 0, 3, 4, 0, 0, 1, 1, 0, 2, 0) | 19  | $x_2^2 x_3^2 x_6^4 x_7 x_8 x_9^4 x_{11}^5$                      | 1             |
| (6, 2, 1, 0, 2) | (0, 0, 4, 4, 0, 1, 2, 0, 1, 0, 0) | 20  | $x_2^2 x_4 x_5^2 x_6 x_8^4 x_9 x_{10}^4 x_{11}^5$               | -1            |
| (5, 6, 0, 0, 0) | (0, 1, 0, 1, 0, 1, 0, 1, 0, 1, 1) | 29  | $x_1 x_2 x_3^3 x_4 x_5^3 x_6^2 x_8^4 x_9^4 x_{10}^5 x_{11}^5$   | -1            |
| (5, 5, 1, 0, 0) | (0, 1, 1, 0, 1, 0, 0, 1, 0, 2, 1) | 24  | $x_1 x_3^2 x_4^3 x_5^2 x_6^4 x_8^4 x_9^4 x_{11}^4$              | -1            |
| (5, 5, 0, 1, 0) | (0, 0, 1, 0, 1, 1, 0, 1, 0, 3, 1) | 24  | $x_1 x_2^3 x_4^3 x_5 x_6^4 x_8^4 x_9^4 x_{11}^4$                | -1            |
| (5, 5, 0, 0, 1) | (1, 4, 1, 0, 1, 0, 1, 0, 1, 0, 0) | 24  | $x_1^2 x_3^3 x_4 x_5^3 x_6 x_8^3 x_9^4 x_{10}^3 x_{11}^4$       | 1             |
| (5, 4, 2, 0, 0) | (0, 1, 0, 2, 0, 1, 0, 1, 2, 0, 1) | 21  | $x_3 x_4 x_5^3 x_6 x_7^4 x_8^3 x_9 x_{10}^4 x_{11}^3$           | 2             |
| (5, 4, 1, 1, 0) | (0, 3, 1, 2, 0, 1, 0, 1, 0, 1, 0) | 20  | $x_3 x_5 x_6 x_7^3 x_8^3 x_9^4 x_{10}^3 x_{11}^4$               | -1 · 2        |
| (5, 4, 1, 0, 1) | (0, 1, 0, 0, 2, 4, 0, 1, 1, 0, 1) | 19  | $x_1 x_3 x_4^3 x_7^3 x_8^2 x_9^4 x_{10}^3 x_{11}^3$             | -1            |
| (5, 4, 0, 2, 0) | (3, 3, 0, 1, 0, 1, 0, 1, 0, 1, 0) | 20  | $x_2 x_5 x_6^2 x_7^3 x_8^2 x_9^4 x_{10}^3 x_{11}^4$             | 1             |
| (5, 4, 0, 1, 1) | (0, 0, 1, 0, 1, 0, 1, 1, 0, 4, 3) | 20  | $x_2^2 x_3 x_4^3 x_5 x_6^3 x_7^3 x_8^3 x_9^4$                   | -1            |
| (5, 4, 0, 0, 2) | (0, 0, 1, 0, 0, 1, 1, 1, 0, 4, 4) | 21  | $x_2^2 x_4^2 x_5^4 x_6^2 x_7^3 x_8^4 x_9^4 x_{10} x_{11}$       | -1            |
| (5, 3, 3, 0, 0) | (0, 1, 1, 0, 2, 2, 0, 2, 0, 1, 0) | 20  | $x_3 x_4 x_5 x_6^2 x_7^3 x_8^4 x_9^2 x_{10}^2 x_{11}^4$         | -1            |
| (5, 3, 2, 1, 0) | (0, 1, 0, 0, 2, 0, 1, 3, 0, 2, 1) | 17  | $x_1 x_3 x_4^3 x_6^4 x_7 x_9^4 x_{10} x_{11}^2$                 | 1             |
| (5, 3, 2, 0, 1) | (0, 2, 0, 4, 2, 0, 1, 0, 1, 1, 0) | 18  | $x_3^2 x_5 x_6^2 x_7 x_8^4 x_9^2 x_{10}^2 x_{11}^4$             | -1            |
| (5, 3, 1, 2, 0) | (0, 2, 1, 0, 0, 1, 0, 3, 3, 1, 0) | 18  | $x_4 x_5^3 x_6^2 x_7^4 x_8 x_9 x_{10}^2 x_{11}^4$               | 2             |
| (5, 3, 1, 1, 1) | (0, 0, 2, 1, 1, 0, 4, 0, 3, 0, 1) | 17  | $x_2^3 x_5 x_6^3 x_8^4 x_{10}^4 x_{11}^2$                       | -1            |
| (5, 3, 1, 0, 2) | (0, 0, 1, 1, 4, 1, 0, 2, 0, 4, 0) | 18  | $x_2^2 x_3 x_4 x_5 x_6^2 x_7^3 x_9^3 x_{10} x_{11}^4$           | -1            |
| (5, 3, 0, 2, 1) | (0, 1, 0, 3, 0, 4, 3, 1, 0, 0, 1) | 18  | $x_3^2 x_4 x_5^4 x_7 x_8 x_9^3 x_{10}^4 x_{11}^2$               | 1             |
| (5, 3, 0, 1, 2) | (0, 1, 0, 3, 4, 0, 4, 0, 0, 1, 1) | 18  | $x_3^2 x_6^4 x_7 x_8^3 x_9^4 x_{10}^2 x_{11}^2$                 | -1            |
| (5, 3, 0, 0, 3) | (0, 1, 0, 1, 1, 0, 0, 4, 0, 4, 4) | 22  | $x_1 x_3 x_4 x_5^2 x_6^3 x_7^4 x_8^2 x_9^4 x_{10}^2 x_{11}^2$   | -1            |
| (5, 2, 2, 2, 0) | (0, 0, 3, 3, 2, 1, 0, 0, 2, 1, 0) | 17  | $x_2^2 x_4 x_5 x_7^3 x_8^4 x_9 x_{10} x_{11}^4$                 | 1             |
| (5, 2, 2, 1, 1) | (0, 0, 1, 0, 2, 0, 4, 2, 0, 3, 1) | 16  | $x_2^2 x_4^3 x_5 x_6^4 x_8 x_9^4 x_{11}$                        | -1 · 3        |
| (5, 2, 1, 1, 2) | (0, 0, 1, 0, 3, 0, 4, 4, 0, 1, 2) | 16  | $x_1 x_2^3 x_4^2 x_6^3 x_7 x_8 x_9^4 x_{10}$                    | -1            |
| (4, 7, 0, 0, 0) | (1, 1, 0, 1, 0, 0, 1, 0, 1, 1, 1) | 32  | $x_1 x_2^3 x_3^3 x_4^3 x_5 x_6^3 x_8^3 x_9^5 x_{10}^6 x_{11}^6$ | -1            |

$$S \subseteq \mathbb{Z}_p \times \mathbb{Z}_5 \setminus \{(0, 0)\}, |S| = 11$$

| $\lambda$       | $\mathbf{a}$                      | deg | monomial/s                                                      | coefficient/s |
|-----------------|-----------------------------------|-----|-----------------------------------------------------------------|---------------|
| (4, 6, 1, 0, 0) | (2, 0, 1, 1, 0, 0, 1, 1, 0, 1, 1) | 26  | $x_3^2 x_4^2 x_5^2 x_6^3 x_8^4 x_9^3 x_{10}^5 x_{11}^5$         | -1            |
| (4, 6, 0, 1, 0) | (1, 1, 0, 1, 0, 0, 1, 0, 1, 1, 3) | 26  | $x_1^2 x_2^2 x_4^4 x_5^2 x_6^3 x_8^3 x_9^5 x_{10}^5$            | 1             |
| (4, 6, 0, 0, 1) | (1, 0, 0, 1, 1, 4, 0, 1, 1, 0, 1) | 25  | $x_2 x_3^3 x_4 x_5^4 x_8^4 x_9^3 x_{10}^3 x_{11}^5$             | 1             |
| (4, 5, 2, 0, 0) | (0, 1, 1, 0, 2, 0, 2, 1, 1, 0, 1) | 22  | $x_3 x_4^2 x_5 x_6^3 x_7 x_8^4 x_9^3 x_{10}^3 x_{11}^4$         | 2             |
| (4, 5, 1, 1, 0) | (1, 1, 0, 1, 0, 2, 1, 0, 3, 0, 1) | 20  | $x_2 x_4^2 x_5^3 x_7^4 x_8^3 x_{10}^3 x_{11}^4$                 | -1            |
| (4, 5, 1, 0, 1) | (0, 4, 1, 1, 1, 0, 1, 0, 1, 0, 2) | 21  | $x_1 x_3^2 x_4^2 x_5^2 x_6 x_7^3 x_8^3 x_9^4 x_{10}^3$          | 1             |
| (4, 5, 0, 2, 0) | (3, 0, 1, 0, 1, 1, 1, 0, 0, 3, 1) | 22  | $x_4^2 x_5^2 x_6^4 x_7^4 x_8^2 x_9^3 x_{10} x_{11}^4$           | 1             |
| (4, 5, 0, 1, 1) | (0, 1, 0, 1, 1, 1, 0, 1, 3, 4, 0) | 21  | $x_3^2 x_4^3 x_5^3 x_6^3 x_7^3 x_8^4 x_{11}^3$                  | -1            |
| (4, 5, 0, 0, 2) | (4, 0, 4, 0, 1, 1, 1, 0, 1, 0, 1) | 22  | $x_2 x_3 x_4^2 x_5^2 x_6^2 x_7^2 x_8^3 x_9^3 x_{10}^4 x_{11}^4$ | 1             |
| (4, 4, 3, 0, 0) | (0, 1, 1, 0, 1, 1, 0, 2, 2, 0, 2) | 19  | $x_1 x_3 x_4 x_5^2 x_6^3 x_7^2 x_8^2 x_9^2 x_{10}^3 x_{11}^2$   | -1            |
| (4, 4, 2, 1, 0) | (0, 2, 0, 0, 1, 1, 1, 3, 1, 2, 0) | 18  | $x_3^2 x_4^3 x_6^3 x_7^3 x_9^3 x_{10} x_{11}^3$                 | -1 · 2        |
| (4, 4, 2, 0, 1) | (0, 0, 4, 2, 1, 1, 0, 1, 0, 2, 1) | 18  | $x_2^2 x_5 x_6^2 x_7^3 x_8^3 x_9^3 x_{10} x_{11}^3$             | -1            |
| (4, 4, 1, 2, 0) | (0, 0, 1, 0, 3, 3, 1, 0, 1, 2, 1) | 18  | $x_2^2 x_4^3 x_5 x_6 x_7^2 x_8^3 x_9^3 x_{11}^3$                | 1             |
| (4, 4, 1, 1, 1) | (0, 0, 1, 3, 0, 4, 1, 2, 1, 0, 1) | 17  | $x_2^2 x_3 x_5^3 x_7^3 x_9^2 x_{10}^3 x_{11}^3$                 | -1            |
| (4, 4, 1, 0, 2) | (0, 1, 0, 2, 4, 0, 1, 1, 0, 4, 1) | 18  | $x_3 x_5 x_6^3 x_7^3 x_8^3 x_9^3 x_{10} x_{11}^3$               | -1 · 2 · 3    |
| (4, 4, 0, 3, 0) | (0, 1, 3, 0, 3, 1, 3, 1, 0, 1, 0) | 20  | $x_4 x_5^2 x_6^3 x_7^2 x_8^3 x_9^3 x_{10}^3 x_{11}^3$           | 3             |
| (4, 4, 0, 2, 1) | (0, 1, 0, 1, 1, 0, 3, 1, 3, 4, 0) | 18  | $x_3^2 x_4^2 x_5^3 x_6^3 x_7 x_8^3 x_9 x_{11}^3$                | -1            |
| (4, 4, 0, 1, 2) | (0, 1, 0, 3, 4, 4, 0, 1, 0, 1, 1) | 17  | $x_1 x_3 x_6 x_7^2 x_8^3 x_9^3 x_{10}^3 x_{11}^3$               | -1            |
| (4, 4, 0, 0, 3) | (0, 4, 0, 1, 1, 1, 1, 0, 4, 4, 0) | 20  | $x_3 x_4^2 x_5^2 x_6^2 x_7^3 x_8^3 x_9^2 x_{10}^2 x_{11}^3$     | -1            |
| (4, 3, 3, 1, 0) | (0, 1, 0, 2, 0, 0, 1, 1, 2, 2, 3) | 17  | $x_3^2 x_4^2 x_5^2 x_6^3 x_7^2 x_8^2 x_9^2 x_{10}^2$            | -1            |
| (4, 3, 3, 0, 1) | (0, 1, 0, 2, 0, 4, 2, 0, 2, 1, 1) | 17  | $x_1 x_3^2 x_4 x_5^3 x_7 x_8^3 x_9^2 x_{10}^2 x_{11}^2$         | 1             |
| (4, 3, 2, 2, 0) | (0, 1, 0, 3, 3, 0, 1, 1, 0, 2, 2) | 16  | $x_3^2 x_4 x_5 x_6^3 x_7^2 x_8^2 x_9^3 x_{10} x_{11}$           | -1            |
| (4, 3, 2, 1, 1) | (0, 0, 2, 1, 0, 3, 0, 1, 2, 4, 1) | 15  | $x_2^2 x_4^2 x_5^3 x_7^3 x_8^2 x_9 x_{11}^2$                    | -1            |
| (4, 3, 2, 0, 2) | (0, 1, 0, 1, 1, 4, 2, 0, 4, 0, 2) | 15  | $x_1 x_3 x_4 x_5^2 x_6 x_7 x_8^3 x_9 x_{10}^3 x_{11}$           | -1            |
| (4, 3, 1, 2, 1) | (0, 0, 1, 2, 1, 0, 4, 3, 1, 0, 3) | 15  | $x_1 x_2^3 x_5 x_6^3 x_8 x_9^2 x_{10}^3 x_{11}$                 | 1             |

$$S \subseteq \mathbb{Z}_p \times \mathbb{Z}_5 \setminus \{(0, 0)\}, |S| = 11$$

| $\lambda$       | $\mathbf{a}$                      | deg | monomial/s                                                      | coefficient/s |
|-----------------|-----------------------------------|-----|-----------------------------------------------------------------|---------------|
| (4, 3, 1, 1, 2) | (0, 0, 1, 1, 2, 0, 3, 1, 0, 4, 4) | 15  | $x_2^2 x_3 x_4^2 x_6^3 x_8^2 x_9^3 x_{10} x_{11}$               | 2             |
| (4, 3, 1, 0, 3) | (0, 0, 1, 0, 1, 2, 0, 4, 4, 1, 4) | 17  | $x_2^2 x_4^2 x_5^2 x_7^3 x_8^2 x_9^2 x_{10}^2 x_{11}^2$         | -1            |
| (4, 3, 0, 2, 2) | (0, 1, 0, 3, 4, 1, 0, 3, 0, 1, 4) | 16  | $x_2^2 x_3 x_4 x_6^2 x_7^3 x_8 x_9^3 x_{10}^2 x_{11}$           | 2             |
| (4, 2, 2, 2, 1) | (0, 0, 1, 3, 2, 1, 0, 2, 4, 0, 3) | 14  | $x_2^2 x_3 x_4 x_5 x_6 x_7^3 x_8 x_{10}^3 x_{11}$               | 2             |
| (3, 8, 0, 0, 0) | (1, 0, 1, 1, 1, 0, 1, 0, 1, 1, 1) | 37  | $x_1 x_3^2 x_4^4 x_5^5 x_6^2 x_8^2 x_9^7 x_{10}^7 x_{11}^7$     | -1            |
| (3, 7, 1, 0, 0) | (1, 1, 0, 1, 0, 1, 0, 1, 1, 1, 2) | 30  | $x_2^2 x_3^2 x_4^2 x_5^2 x_6^5 x_8^5 x_9^6 x_{10}^6$            | 1             |
| (3, 7, 0, 1, 0) | (1, 1, 1, 3, 0, 1, 0, 1, 1, 0, 1) | 29  | $x_2 x_3^3 x_5^2 x_6^5 x_8^5 x_9^5 x_{10}^2 x_{11}^6$           | -1            |
| (3, 7, 0, 0, 1) | (1, 1, 0, 1, 4, 1, 1, 0, 0, 1, 1) | 30  | $x_1^2 x_2^2 x_3 x_4^5 x_5^5 x_8 x_9^2 x_{10}^6 x_{11}^6$       | 1             |
| (3, 6, 2, 0, 0) | (1, 1, 0, 1, 0, 1, 0, 2, 1, 1, 2) | 24  | $x_2 x_4^2 x_5^2 x_6^5 x_7^2 x_8 x_9^5 x_{10}^5 x_{11}$         | -1            |
| (3, 6, 1, 1, 0) | (2, 0, 1, 0, 1, 0, 1, 1, 1, 3, 1) | 24  | $x_4 x_5 x_6^2 x_7^5 x_8^5 x_9^5 x_{11}^5$                      | 1             |
| (3, 6, 1, 0, 1) | (0, 1, 1, 1, 0, 1, 1, 4, 2, 1, 0) | 24  | $x_3^2 x_4^3 x_5^2 x_6^5 x_7^5 x_{10}^5 x_{11}^2$               | 1             |
| (3, 6, 0, 2, 0) | (1, 1, 1, 0, 1, 1, 1, 0, 3, 3, 0) | 25  | $x_2^2 x_3^2 x_4^2 x_5^3 x_6^5 x_7^5 x_8^2 x_9 x_{10} x_{11}^2$ | -1            |
| (3, 6, 0, 1, 1) | (1, 3, 1, 4, 0, 1, 1, 1, 0, 1, 0) | 24  | $x_3^3 x_5 x_6^4 x_7^4 x_8^4 x_9 x_{10}^5 x_{11}^2$             | 1             |
| (3, 6, 0, 0, 2) | (4, 1, 1, 0, 1, 1, 4, 0, 1, 0, 1) | 25  | $x_1 x_2 x_3 x_5^3 x_6^4 x_7 x_8^2 x_9^5 x_{10}^2 x_{11}^5$     | 1             |
| (3, 5, 3, 0, 0) | (2, 0, 0, 1, 1, 0, 1, 1, 2, 1, 2) | 22  | $x_3^2 x_5^2 x_6^2 x_7^4 x_8^4 x_9^2 x_{10}^4 x_{11}^2$         | 2             |
| (3, 5, 2, 1, 0) | (0, 1, 2, 0, 1, 2, 1, 0, 1, 1, 3) | 20  | $x_4 x_5^4 x_6 x_7^4 x_8^2 x_9^4 x_{10}^4$                      | -1 \cdot 2    |
| (3, 5, 2, 0, 1) | (1, 0, 1, 1, 1, 1, 0, 2, 2, 0, 4) | 20  | $x_2 x_3 x_4^4 x_5^4 x_6^4 x_7^2 x_8 x_9 x_{10}^2$              | -1            |
| (3, 5, 1, 2, 0) | (1, 0, 1, 1, 0, 1, 0, 2, 1, 3, 3) | 20  | $x_3^2 x_4^4 x_5^2 x_6^4 x_7^2 x_8^4 x_{10} x_{11}$             | -1            |
| (3, 5, 1, 1, 1) | (0, 1, 1, 0, 1, 0, 1, 4, 3, 1, 2) | 19  | $x_3^3 x_4^2 x_5^4 x_6^2 x_7^4 x_{10}^4$                        | -1            |
| (3, 5, 1, 0, 2) | (0, 1, 1, 1, 4, 1, 0, 1, 0, 2, 4) | 19  | $x_1 x_3 x_4^3 x_5 x_6^4 x_7^2 x_8^4 x_9^2 x_{11}$              | -1            |
| (3, 5, 0, 3, 0) | (0, 0, 1, 3, 3, 1, 3, 1, 0, 1, 1) | 22  | $x_2^2 x_4 x_5 x_6^2 x_7^2 x_8^4 x_9^2 x_{10}^4 x_{11}^4$       | -1            |
| (3, 5, 0, 2, 1) | (0, 1, 1, 1, 1, 0, 3, 1, 0, 3, 4) | 19  | $x_1 x_2 x_3 x_4^2 x_5^4 x_6^2 x_7 x_8^4 x_9^2 x_{10}$          | 1             |
| (3, 5, 0, 1, 2) | (0, 4, 0, 1, 1, 1, 1, 0, 1, 3, 4) | 20  | $x_1 x_3^2 x_4^2 x_5^2 x_6^3 x_7^3 x_8^2 x_9^4 x_{11}$          | 1             |
| (3, 5, 0, 0, 3) | (0, 4, 4, 1, 1, 1, 0, 1, 1, 0, 4) | 22  | $x_1 x_3 x_4 x_5^3 x_6^2 x_7^2 x_8^4 x_9^4 x_{10}^2 x_{11}^2$   | 1             |
| (3, 4, 4, 0, 0) | (1, 0, 0, 2, 0, 1, 1, 2, 2, 1, 2) | 21  | $x_3^2 x_5^2 x_6^2 x_7^3 x_8^3 x_9^3 x_{10}^3 x_{11}^3$         | 1             |
| (3, 4, 3, 1, 0) | (0, 2, 1, 0, 1, 3, 2, 1, 1, 0, 2) | 18  | $x_3 x_4^2 x_5^3 x_7^2 x_8^3 x_9^3 x_{10}^2 x_{11}^2$           | 1             |

$$S \subseteq \mathbb{Z}_p \times \mathbb{Z}_5 \setminus \{(0, 0)\}, |S| = 11$$

| $\lambda$       | $\mathbf{a}$                      | deg | monomial/s                                                  | coefficient/s        |
|-----------------|-----------------------------------|-----|-------------------------------------------------------------|----------------------|
| (3, 4, 3, 0, 1) | (0, 1, 1, 2, 4, 0, 0, 2, 1, 1, 2) | 18  | $x_1 x_3^2 x_4^2 x_6 x_7^2 x_8^2 x_9^3 x_{10}^3 x_{11}^2$   | 1                    |
| (3, 4, 2, 2, 0) | (0, 0, 3, 1, 2, 1, 0, 1, 3, 2, 1) | 17  | $x_2^2 x_3 x_4 x_5 x_6^2 x_7^2 x_8^3 x_9 x_{10} x_{11}^3$   | -1                   |
| (3, 4, 2, 1, 1) | (0, 1, 0, 0, 1, 1, 1, 3, 2, 4, 2) | 15  | $x_1^2 x_3 x_4^2 x_5^2 x_6^3 x_7^3 x_9 x_{11}$              | 1                    |
| (3, 4, 2, 0, 2) | (0, 1, 1, 0, 2, 4, 0, 1, 4, 2, 1) | 17  | $x_2 x_3^3 x_4^2 x_6 x_7^2 x_8^3 x_9 x_{10} x_{11}^3$       | 2                    |
| (3, 4, 1, 3, 0) | (0, 1, 3, 3, 1, 0, 1, 2, 1, 0, 3) | 17  | $x_1 x_2 x_4 x_5^2 x_6^2 x_7^3 x_9^3 x_{10}^2 x_{11}^2$     | 1                    |
| (3, 4, 1, 2, 1) | (0, 0, 4, 3, 1, 0, 3, 1, 1, 1, 2) | 16  | $x_1 x_2^2 x_5 x_6^2 x_7 x_8^3 x_9^3 x_{10}^3$              | 1                    |
| (3, 4, 1, 1, 2) | (0, 0, 1, 3, 0, 2, 1, 1, 4, 1, 4) | 16  | $x_1 x_2^2 x_5^2 x_7^3 x_8^3 x_9 x_{10}^3 x_{11}$           | 1                    |
| (3, 4, 1, 0, 3) | (0, 1, 1, 4, 1, 2, 0, 4, 1, 4, 0) | 18  | $x_3^2 x_4^2 x_5^3 x_7^2 x_8^2 x_9^3 x_{10}^2 x_{11}^2$     | $-1 \cdot 2 \cdot 3$ |
| (3, 4, 0, 3, 1) | (0, 1, 0, 0, 3, 1, 3, 1, 3, 1, 4) | 18  | $x_1 x_3 x_4^2 x_5 x_6^3 x_7^2 x_8^3 x_9^2 x_{10}^3$        | $-1 \cdot 2^2$       |
| (3, 4, 0, 2, 2) | (0, 1, 3, 1, 4, 3, 4, 1, 1, 0, 0) | 17  | $x_1 x_3 x_4^3 x_5 x_6 x_7 x_8^3 x_9^3 x_{10} x_{11}^2$     | $-1 \cdot 2$         |
| (3, 4, 0, 1, 3) | (0, 1, 3, 0, 4, 0, 4, 4, 1, 1, 1) | 18  | $x_1 x_2 x_4^2 x_6^2 x_7 x_8^3 x_9^3 x_{10}^3 x_{11}^3$     | -1                   |
| (3, 4, 0, 0, 4) | (1, 1, 0, 1, 0, 1, 0, 4, 4, 4, 4) | 20  | $x_2 x_4^2 x_5 x_6^3 x_7^2 x_8^3 x_9^3 x_{10}^3 x_{11}^3$   | 1                    |
| (3, 3, 3, 2, 0) | (0, 1, 2, 0, 1, 3, 0, 2, 2, 3, 1) | 15  | $x_1 x_4^2 x_5^2 x_6 x_7^2 x_8^2 x_9^2 x_{10} x_{11}^2$     | $-1 \cdot 2$         |
| (3, 3, 3, 1, 1) | (0, 0, 2, 2, 2, 1, 1, 0, 1, 3, 4) | 15  | $x_1 x_2^2 x_3 x_4^2 x_5^2 x_6^2 x_7 x_8^2 x_9^2$           | 1                    |
| (3, 3, 3, 0, 2) | (0, 1, 0, 1, 2, 4, 0, 1, 2, 2, 4) | 16  | $x_3^2 x_4^2 x_5^2 x_6 x_7^2 x_8^2 x_9^2 x_{10}^2 x_{11}$   | 2                    |
| (3, 3, 2, 2, 1) | (0, 0, 2, 1, 1, 3, 2, 4, 3, 0, 1) | 14  | $x_2^2 x_3 x_4^2 x_5^2 x_6 x_7 x_9 x_{10}^2 x_{11}^2$       | -1                   |
| (3, 3, 2, 1, 2) | (0, 0, 1, 0, 2, 4, 1, 1, 3, 2, 4) | 14  | $x_2^2 x_3^2 x_4^2 x_5 x_6 x_7^2 x_8^2 x_{10} x_{11}$       | 2                    |
| (3, 3, 2, 0, 3) | (0, 1, 2, 4, 0, 4, 2, 1, 0, 1, 4) | 16  | $x_1 x_2 x_4 x_5^2 x_6^2 x_7 x_8^2 x_9^2 x_{10}^2 x_{11}^2$ | $-1 \cdot 3$         |
| (3, 3, 1, 2, 2) | (0, 0, 3, 1, 0, 2, 1, 1, 4, 4, 3) | 14  | $x_1 x_2^2 x_3 x_4^2 x_5^2 x_7 x_8^2 x_9 x_{10} x_{11}$     | 2                    |
| (3, 3, 1, 1, 3) | (0, 0, 4, 4, 3, 1, 0, 4, 2, 1, 1) | 15  | $x_1^2 x_2^2 x_4 x_6^2 x_7^2 x_8^2 x_{10}^2 x_{11}^2$       | 1                    |
| (3, 2, 2, 2, 2) | (0, 0, 2, 1, 3, 2, 1, 0, 3, 4, 4) | 13  | $x_1^2 x_2^2 x_3 x_5 x_6 x_7 x_8^2 x_9 x_{10} x_{11}$       | -1                   |
| (2, 9, 0, 0, 0) | (0, 1, 0, 1, 1, 1, 1, 1, 1, 1, 1) | 44  | $x_2 x_3 x_4^2 x_5^3 x_6^7 x_8^7 x_9^7 x_{10}^8 x_{11}^8$   | -1                   |
| (2, 8, 1, 0, 0) | (1, 1, 1, 2, 1, 0, 1, 1, 1, 0, 1) | 35  | $x_1 x_2^2 x_3^5 x_5^6 x_6 x_8^6 x_9^6 x_{10} x_{11}^7$     | $-1 \cdot 2$         |
| (2, 8, 0, 1, 0) | (1, 1, 1, 0, 1, 0, 1, 1, 1, 3, 1) | 36  | $x_7^2 x_2^2 x_3^3 x_5^7 x_6 x_8^7 x_9^7 x_{11}^7$          | -1                   |
| (2, 8, 0, 0, 1) | (4, 1, 1, 0, 1, 1, 0, 1, 1, 1, 1) | 36  | $x_2 x_3 x_4 x_5^3 x_6^3 x_8^6 x_9^7 x_{10}^7 x_{11}^7$     | 2                    |

$$S \subseteq \mathbb{Z}_p \times \mathbb{Z}_5 \setminus \{(0, 0)\}, |S| = 11$$

| $\lambda$       | $\mathbf{a}$                      | deg | monomial/s                                                  | coefficient/s       |
|-----------------|-----------------------------------|-----|-------------------------------------------------------------|---------------------|
| (2, 7, 2, 0, 0) | (2, 1, 1, 0, 1, 2, 1, 1, 1, 1, 0) | 30  | $x_2 x_3^3 x_5^6 x_6 x_8^6 x_9^6 x_{10} x_{11}$             | -1                  |
| (2, 7, 1, 1, 0) | (0, 3, 1, 1, 1, 0, 1, 1, 1, 2, 1) | 29  | $x_4^3 x_5^2 x_6 x_7^5 x_8^6 x_9^6 x_{11}^6$                | -1                  |
| (2, 7, 1, 0, 1) | (2, 4, 0, 1, 1, 1, 0, 1, 1, 1, 1) | 29  | $x_4 x_5^2 x_6^2 x_7 x_8^5 x_9^6 x_{10} x_{11}^6$           | -1 · 2              |
| (2, 7, 0, 2, 0) | (1, 3, 0, 1, 3, 1, 1, 1, 1, 0, 1) | 30  | $x_1 x_4^5 x_5 x_6^6 x_8^5 x_9^5 x_{10} x_{11}^6$           | 2                   |
| (2, 7, 0, 1, 1) | (3, 0, 1, 1, 0, 1, 1, 4, 1, 1, 1) | 29  | $x_3 x_4^3 x_5 x_6^2 x_7^4 x_8^6 x_9^6 x_{10} x_{11}^6$     | -1                  |
| (2, 7, 0, 0, 2) | (1, 1, 4, 1, 1, 0, 4, 1, 1, 0, 1) | 29  | $x_2^2 x_3 x_4^3 x_5^4 x_6 x_8^6 x_9^5 x_{10} x_{11}^6$     | -1 · 2              |
| (2, 6, 3, 0, 0) | (1, 0, 1, 1, 0, 1, 1, 2, 2, 1, 2) | 26  | $x_3^2 x_4^2 x_5 x_6^5 x_7^5 x_8^2 x_9^2 x_{10}^5 x_{11}^2$ | -1                  |
| (2, 6, 2, 1, 0) | (1, 0, 3, 1, 2, 1, 1, 0, 2, 1, 1) | 24  | $x_4^2 x_6^5 x_7^5 x_8 x_9 x_{10}^5 x_{11}^5$               | -1 · 2              |
| (2, 6, 2, 0, 1) | (1, 0, 1, 1, 2, 2, 1, 1, 1, 4, 0) | 24  | $x_2 x_3 x_4^4 x_5 x_6 x_7^5 x_8^5 x_9^5 x_{11}$            | -1 · 2              |
| (2, 6, 1, 2, 0) | (0, 1, 1, 3, 1, 2, 0, 1, 3, 1, 1) | 24  | $x_3^3 x_4 x_5^3 x_7 x_8^5 x_9 x_{10}^5 x_{11}^5$           | 3                   |
| (2, 6, 1, 1, 1) | (0, 1, 1, 1, 1, 0, 4, 1, 2, 1, 3) | 22  | $x_1 x_2 x_3^2 x_4^2 x_5^5 x_6 x_8^5 x_{10}^5$              | 1                   |
| (2, 6, 1, 0, 2) | (1, 1, 0, 1, 1, 4, 1, 1, 0, 2, 4) | 24  | $x_1 x_2^3 x_3 x_4^2 x_5^4 x_6 x_7^5 x_8^5 x_9 x_{11}$      | -1                  |
| (2, 6, 0, 3, 0) | (1, 1, 1, 0, 1, 3, 1, 3, 3, 0, 1) | 25  | $x_2 x_3^2 x_5^5 x_6^2 x_7^5 x_8^2 x_9^2 x_{10} x_{11}^5$   | -1 · 3              |
| (2, 6, 0, 2, 1) | (0, 4, 1, 1, 1, 1, 1, 3, 0, 1, 3) | 24  | $x_3^2 x_4^2 x_5^2 x_6^5 x_7^5 x_8 x_9 x_{10}^5 x_{11}$     | 2                   |
| (2, 6, 0, 1, 2) | (0, 1, 1, 4, 1, 1, 1, 0, 4, 3, 1) | 24  | $x_3^2 x_4 x_5^4 x_6^5 x_7^5 x_8 x_9 x_{11}^5$              | -1                  |
| (2, 6, 0, 0, 3) | (1, 4, 4, 0, 1, 1, 1, 1, 0, 4, 1) | 26  | $x_2 x_3 x_5^3 x_6^3 x_7^5 x_8^5 x_9 x_{10}^2 x_{11}^5$     | -1                  |
| (2, 5, 4, 0, 0) | (2, 0, 1, 1, 0, 2, 1, 1, 2, 1, 2) | 24  | $x_3 x_4^2 x_5 x_6^2 x_7^4 x_8^4 x_9^3 x_{10}^4 x_{11}^3$   | 2                   |
| (2, 5, 3, 1, 0) | (0, 2, 1, 3, 1, 2, 2, 1, 1, 0, 1) | 21  | $x_5^4 x_6^2 x_7^2 x_8^4 x_9^4 x_{10} x_{11}^4$             | -1                  |
| (2, 5, 3, 0, 1) | (1, 0, 2, 1, 0, 2, 1, 1, 4, 2, 1) | 20  | $x_4^3 x_5 x_6^2 x_7^4 x_8^4 x_{10}^2 x_{11}^4$             | 1                   |
| (2, 5, 2, 2, 0) | (0, 2, 1, 1, 3, 1, 1, 2, 0, 3, 1) | 19  | $x_1 x_4^2 x_5 x_6^4 x_7^4 x_8 x_9 x_{10} x_{11}^4$         | 1                   |
| (2, 5, 2, 1, 1) | (0, 1, 2, 1, 3, 1, 4, 1, 1, 2, 0) | 19  | $x_2^3 x_4^2 x_6^4 x_8^4 x_9^4 x_{10} x_{11}$               | 1                   |
| (2, 5, 2, 0, 2) | (0, 4, 1, 1, 1, 2, 2, 1, 1, 0, 4) | 20  | $x_2 x_3^2 x_4 x_5^4 x_6 x_7 x_8^4 x_9^4 x_{10} x_{11}$     | 1                   |
| (2, 5, 1, 3, 0) | (0, 1, 3, 3, 1, 0, 1, 2, 1, 3, 1) | 21  | $x_2 x_4^2 x_5^3 x_6 x_7^4 x_8^4 x_{10}^2 x_{11}^4$         | 3                   |
| (2, 5, 1, 2, 1) | (0, 1, 1, 1, 1, 3, 2, 4, 3, 0, 1) | 19  | $x_3^4 x_4^4 x_5^4 x_6 x_9 x_{10} x_{11}^4$                 | 1                   |
| (2, 5, 1, 1, 2) | (0, 1, 1, 1, 3, 1, 4, 1, 2, 0, 4) | 19  | $x_3^4 x_4^4 x_6^4 x_7 x_8^4 x_{10} x_{11}$                 | 2                   |
| (2, 5, 1, 0, 3) | (0, 1, 4, 1, 1, 2, 4, 4, 1, 0, 1) | 21  | $x_2 x_3^2 x_4^2 x_5^3 x_7^2 x_8^2 x_9^4 x_{10} x_{11}^4$   | -1 · 2 <sup>2</sup> |

$$S \subseteq \mathbb{Z}_p \times \mathbb{Z}_5 \setminus \{(0, 0)\}, |S| = 11$$

| $\lambda$       | $\mathbf{a}$                      | deg | monomial/s                                                                                                                       | coefficient/s       |
|-----------------|-----------------------------------|-----|----------------------------------------------------------------------------------------------------------------------------------|---------------------|
| (2, 5, 0, 4, 0) | (3, 1, 0, 1, 3, 3, 1, 3, 1, 1, 0) | 24  | $x_4^2 x_5^3 x_6^3 x_7^4 x_8^3 x_9^4 x_{10}^4 x_{11}$                                                                            | 1                   |
| (2, 5, 0, 3, 1) | (0, 1, 1, 4, 3, 3, 1, 0, 1, 3, 1) | 21  | $x_3^2 x_5^2 x_6^2 x_7^4 x_8^4 x_9^4 x_{10}^2 x_{11}^4$                                                                          | -1                  |
| (2, 5, 0, 2, 2) | (0, 1, 1, 0, 4, 3, 4, 3, 1, 1, 1) | 20  | $x_3^3 x_4 x_5 x_6 x_7 x_8 x_9^4 x_{10}^4 x_{11}^4$                                                                              | 1                   |
| (2, 5, 0, 1, 3) | (0, 1, 1, 0, 1, 1, 4, 1, 3, 4, 4) | 20  | $x_1 x_3 x_4 x_5^4 x_6^3 x_7^2 x_8^4 x_{10}^2 x_{11}^2$                                                                          | -1                  |
| (2, 5, 0, 0, 4) | (4, 1, 4, 0, 1, 1, 1, 1, 0, 4, 4) | 24  | $x_2 x_3^2 x_4 x_5^3 x_6^3 x_7^3 x_8^4 x_9 x_{10}^3 x_{11}^3$                                                                    | -1                  |
| (2, 4, 4, 1, 0) | (1, 0, 2, 2, 2, 1, 1, 3, 2, 0, 1) | 19  | $x_3 x_4^3 x_5^3 x_6^2 x_7^3 x_9^3 x_{10} x_{11}^3$                                                                              | -1 · 2              |
| (2, 4, 4, 0, 1) | (0, 2, 1, 1, 4, 2, 1, 1, 2, 2, 0) | 20  | $x_3 x_4^3 x_6^3 x_7^3 x_8^3 x_9^3 x_{10}^3 x_{11}$                                                                              | 2 <sup>2</sup>      |
| (2, 4, 3, 2, 0) | (0, 1, 2, 1, 3, 2, 3, 1, 2, 1, 0) | 18  | $x_1 x_2^2 x_3 x_4^2 x_6^2 x_7 x_8^3 x_9^2 x_{10}^3 x_{11}$                                                                      | -1                  |
| (2, 4, 3, 1, 1) | (0, 1, 1, 4, 2, 0, 1, 3, 2, 1, 2) | 17  | $x_1 x_3^3 x_5^2 x_6 x_7^3 x_9^2 x_{10}^3 x_{11}^2$                                                                              | 1                   |
| (2, 4, 3, 0, 2) | (0, 1, 0, 2, 4, 2, 2, 1, 1, 1, 4) | 18  | $x_1 x_3 x_4 x_5 x_6^2 x_7^3 x_8^3 x_9^3 x_{10} x_{11}$                                                                          | 1                   |
| (2, 4, 2, 3, 0) | (0, 1, 1, 1, 0, 1, 2, 2, 3, 3, 3) | 18  | $x_3^3 x_4^3 x_5 x_6^3 x_7 x_8 x_9^2 x_{10}^2 x_{11}^2$                                                                          | -1                  |
| (2, 4, 2, 2, 1) | (0, 1, 1, 3, 4, 0, 2, 2, 1, 3, 1) | 16  | $x_2^2 x_3^3 x_4 x_6 x_7 x_8 x_9^3 x_{10} x_{11}^3$                                                                              | -1 · 3              |
| (2, 4, 2, 1, 2) | (0, 1, 0, 1, 1, 2, 4, 3, 1, 4, 2) | 16  | $x_1 x_2 x_3 x_4^3 x_5^3 x_6 x_7 x_9^3 x_{10} x_{11}$                                                                            | -1 · 2 <sup>2</sup> |
| (2, 4, 2, 0, 3) | (0, 2, 1, 1, 4, 4, 1, 1, 2, 0, 4) | 17  | $x_1 x_4^2 x_5^2 x_6^2 x_7^3 x_8^3 x_9 x_{10} x_{11}^2$                                                                          | 1                   |
| (2, 4, 1, 3, 1) | (0, 1, 2, 1, 4, 1, 3, 0, 3, 1, 3) | 17  | $x_1 x_2 x_4^3 x_6^3 x_7 x_8 x_9^2 x_{10}^3 x_{11}^2$                                                                            | -1                  |
| (2, 4, 1, 2, 2) | (0, 1, 1, 4, 1, 2, 4, 0, 1, 3, 3) | 15  | $x_1 x_3^3 x_4 x_5^3 x_7 x_8 x_9^3 x_{10} x_{11}$                                                                                | -1 · 2              |
| (2, 4, 1, 1, 3) | (0, 1, 1, 0, 4, 3, 4, 1, 4, 2, 1) | 17  | $x_2^2 x_3^3 x_4 x_5^2 x_7 x_8^3 x_9^2 x_{11}^3$                                                                                 | 2                   |
| (2, 4, 1, 0, 4) | (1, 0, 4, 4, 0, 1, 2, 1, 4, 1, 4) | 20  | $x_3 x_4^3 x_5 x_6^3 x_8^3 x_9^3 x_{10}^3 x_{11}^3$                                                                              | -1 · 2 · 3          |
| (2, 4, 0, 3, 2) | (0, 1, 1, 1, 1, 3, 0, 3, 4, 4, 3) | 18  | $x_2 x_3^2 x_4^3 x_5^3 x_6^2 x_7 x_8^2 x_9 x_{10} x_{11}^2$                                                                      | -1 · 2              |
| (2, 4, 0, 2, 3) | (0, 1, 3, 1, 4, 3, 1, 0, 4, 4, 1) | 18  | $x_3 x_4^3 x_5^2 x_6 x_7^3 x_8 x_9^2 x_{10}^2 x_{11}^3$                                                                          | 2                   |
| (2, 3, 3, 3, 0) | (0, 2, 1, 1, 0, 2, 3, 3, 1, 3, 2) | 17  | $x_2 x_3 x_4^2 x_5 x_6^2 x_7^2 x_8^2 x_9^2 x_{10}^2 x_{11}^2$<br>$x_1 x_3 x_4^2 x_5^2 x_6^2 x_7^2 x_8^2 x_9^2 x_{10}^2 x_{11}^2$ | 5<br>11             |
| (2, 3, 3, 2, 1) | (0, 1, 1, 2, 2, 2, 0, 4, 1, 3, 3) | 15  | $x_1 x_2 x_3^2 x_4^2 x_5^2 x_6^2 x_7 x_9^2 x_{10} x_{11}$                                                                        | -1                  |
| (2, 3, 3, 1, 2) | (0, 1, 0, 2, 1, 3, 4, 1, 2, 4, 2) | 14  | $x_1 x_3 x_4^2 x_5^2 x_7 x_8^2 x_9^2 x_{10} x_{11}^2$                                                                            | 2                   |
| (2, 3, 2, 2, 2) | (0, 1, 0, 4, 2, 2, 4, 1, 3, 1, 3) | 14  | $x_1 x_2^2 x_3 x_4 x_5 x_6 x_7 x_8^2 x_9^2 x_{10} x_{11}$                                                                        | -1                  |
| (2, 3, 2, 1, 3) | (0, 1, 1, 0, 2, 4, 2, 4, 4, 3, 1) | 15  | $x_2^2 x_3^2 x_4 x_5 x_6^2 x_7 x_8^2 x_9^2 x_{11}^2$                                                                             | 1                   |

$$S \subseteq \mathbb{Z}_p \times \mathbb{Z}_5 \setminus \{(0, 0)\}, |S| = 11$$

| $\lambda$        | $\mathbf{a}$                         | deg | monomial/s                                                        | coefficient/s |
|------------------|--------------------------------------|-----|-------------------------------------------------------------------|---------------|
| (1, 10, 0, 0, 0) | (1, 0, 1, 1, 1, 1, 1, 1, 1, 1)       | 52  | $x_1 x_3^2 x_4^3 x_5^4 x_6^9 x_7^8 x_8^9 x_9^8 x_{10}^9 x_{11}^9$ | 1             |
| (1, 9, 1, 0, 0)  | (1, 1, 1, 1, 2, 1, 1, 1, 1, 0, 1)    | 44  | $x_1^2 x_2^2 x_3^3 x_4^6 x_5^7 x_6^8 x_7^8 x_8^8 x_{11}^8$        | -1            |
| (1, 9, 0, 1, 0)  | (1, 1, 1, 3, 1, 1, 1, 0, 1, 1, 1)    | 44  | $x_1 x_2^3 x_3^4 x_5^6 x_6^6 x_7^8 x_8^8 x_{10}^8 x_{11}^8$       | -1            |
| (1, 9, 0, 0, 1)  | (4, 1, 1, 1, 0, 1, 1, 1, 1, 1, 1)    | 44  | $x_2^2 x_3^2 x_4^3 x_6^6 x_7^8 x_8^8 x_9^8 x_{10}^8 x_{11}^8$     | -1            |
| (1, 8, 2, 0, 0)  | (2, 1, 0, 1, 1, 1, 1, 1, 1, 2, 1)    | 37  | $x_1 x_2 x_4^2 x_5^4 x_6^7 x_7^8 x_8^7 x_9^7 x_{10}^7 x_{11}^7$   | 1             |
| (1, 8, 1, 1, 0)  | (1, 3, 1, 2, 1, 1, 1, 1, 1, 1, 0)    | 36  | $x_1 x_3^3 x_5^5 x_6^7 x_8^6 x_9^7 x_{10}^7$                      | 1             |
| (1, 8, 1, 0, 1)  | (1, 1, 4, 1, 1, 2, 1, 1, 1, 1, 0)    | 36  | $x_1 x_2^3 x_4^4 x_5^7 x_8^7 x_9^7 x_{10}^7$                      | 1             |
| (1, 8, 0, 2, 0)  | (1, 0, 1, 3, 1, 1, 1, 1, 1, 3, 1, 1) | 37  | $x_1 x_3^2 x_4 x_5^5 x_6^6 x_7^8 x_8^7 x_9 x_{10}^7 x_{11}^7$     | -1            |
| (1, 8, 0, 1, 1)  | (1, 1, 1, 3, 0, 1, 1, 1, 4, 1, 1)    | 35  | $x_1 x_2^2 x_3^5 x_6^6 x_7^8 x_{10}^7 x_{11}^7$                   | 1             |
| (1, 8, 0, 0, 2)  | (1, 4, 1, 1, 0, 1, 1, 4, 1, 1, 1)    | 37  | $x_1^3 x_2 x_3^4 x_4^3 x_6^4 x_8 x_9^7 x_{10}^7 x_{11}^7$         | -1            |
| (1, 7, 3, 0, 0)  | (1, 1, 2, 1, 1, 1, 2, 1, 1, 2, 0)    | 32  | $x_2 x_3^2 x_4^3 x_5^6 x_6^6 x_8^6 x_9^6 x_{10}^2$                | 2             |
| (1, 7, 2, 1, 0)  | (3, 1, 2, 1, 1, 1, 1, 0, 1, 1, 2)    | 30  | $x_2 x_4^2 x_5^3 x_6^5 x_7^6 x_8^6 x_9^6 x_{10} x_{11}$           | -1            |
| (1, 7, 2, 0, 1)  | (1, 1, 0, 1, 1, 2, 2, 1, 1, 4, 1)    | 29  | $x_2 x_4^6 x_5^3 x_6 x_7 x_8^5 x_9^6 x_{11}^6$                    | 1             |
| (1, 7, 1, 2, 0)  | (1, 1, 1, 1, 1, 3, 0, 1, 2, 1, 3)    | 29  | $x_2 x_3^2 x_4^6 x_5^6 x_6 x_8^6 x_{10}^6 x_{11}$                 | 2             |
| (1, 7, 1, 1, 1)  | (1, 2, 4, 0, 1, 1, 3, 1, 1, 1, 1)    | 29  | $x_1 x_5^2 x_6^4 x_8^5 x_9^5 x_{10}^6 x_{11}^6$                   | -1            |
| (1, 7, 1, 0, 2)  | (1, 0, 1, 1, 1, 4, 1, 1, 2, 4, 1)    | 30  | $x_3^2 x_4^3 x_5^5 x_6 x_7^6 x_8^6 x_{10} x_{11}^6$               | 3             |
| (1, 7, 0, 3, 0)  | (1, 1, 1, 1, 3, 1, 3, 3, 0, 1, 1)    | 32  | $x_1 x_2 x_3^3 x_4^5 x_5^2 x_6^6 x_8^2 x_{10}^6 x_{11}^6$         | 3             |
| (1, 7, 0, 2, 1)  | (4, 1, 1, 3, 1, 1, 1, 1, 0, 1, 3)    | 30  | $x_2 x_3^3 x_4 x_5^4 x_6^4 x_7^5 x_8^5 x_{10}^6 x_{11}$           | 1             |
| (1, 7, 0, 1, 2)  | (1, 0, 3, 1, 1, 1, 1, 1, 4, 4, 1)    | 30  | $x_4^2 x_5^4 x_6^4 x_7^6 x_8^6 x_9 x_{10} x_{11}^6$               | -1            |
| (1, 7, 0, 0, 3)  | (1, 4, 1, 1, 0, 1, 1, 4, 1, 4, 1)    | 32  | $x_1 x_2 x_3^3 x_4^5 x_6^6 x_8^2 x_9^6 x_{10}^2 x_{11}^6$         | 1             |
| (1, 6, 4, 0, 0)  | (1, 2, 0, 2, 1, 1, 1, 1, 1, 2, 2)    | 29  | $x_1 x_4^3 x_5^2 x_6^2 x_7^5 x_8^5 x_9^5 x_{10}^3 x_{11}^3$       | 1             |
| (1, 6, 3, 1, 0)  | (2, 1, 1, 1, 2, 1, 1, 2, 0, 1, 3)    | 25  | $x_1 x_3 x_4^5 x_5^2 x_6^4 x_7^5 x_8^5 x_{10}^5$                  | -1 · 2        |
| (1, 6, 3, 0, 1)  | (1, 1, 2, 1, 1, 1, 1, 0, 2, 4, 2)    | 26  | $x_1 x_2^2 x_4^4 x_5^5 x_6^5 x_7^5 x_9^2 x_{11}^2$                | 1             |
| (1, 6, 2, 2, 0)  | (2, 1, 0, 1, 1, 1, 3, 2, 1, 1, 3)    | 25  | $x_2^2 x_4 x_5^4 x_6^5 x_7 x_8 x_9^5 x_{10}^5 x_{11}$             | 2             |
| (1, 6, 2, 1, 1)  | (1, 1, 1, 1, 1, 1, 3, 0, 2, 2, 4)    | 24  | $x_1^2 x_2^2 x_3^3 x_4^5 x_5^5 x_6^5 x_9 x_{10}$                  | 1             |
| (1, 6, 2, 0, 2)  | (1, 4, 4, 1, 1, 2, 1, 2, 1, 0, 1)    | 25  | $x_2 x_3 x_4^3 x_5^4 x_6^5 x_7^5 x_8 x_9^4 x_{11}^5$              | -1 · 2        |

$$S \subseteq \mathbb{Z}_p \times \mathbb{Z}_5 \setminus \{(0, 0)\}, |S| = 11$$

| $\lambda$       | $\mathbf{a}$                      | deg | monomial/s                                                      | coefficient/s  |
|-----------------|-----------------------------------|-----|-----------------------------------------------------------------|----------------|
| (1, 6, 1, 3, 0) | (3, 1, 0, 1, 3, 1, 2, 1, 1, 3, 1) | 26  | $x_4^3 x_5^2 x_6^4 x_8^5 x_9^5 x_{10}^2 x_{11}^5$               | 1              |
| (1, 6, 1, 2, 1) | (1, 1, 1, 1, 2, 1, 3, 0, 1, 3, 4) | 24  | $x_2^2 x_3^5 x_4^5 x_6^5 x_7 x_9^5 x_{10}$                      | -1             |
| (1, 6, 1, 1, 2) | (0, 4, 3, 4, 1, 1, 1, 1, 1, 2, 1) | 24  | $x_2 x_4 x_5 x_6 x_7^5 x_8^5 x_9^5 x_{11}^5$                    | 2              |
| (1, 6, 1, 0, 3) | (2, 4, 1, 1, 4, 1, 1, 0, 1, 1, 4) | 25  | $x_3 x_4^3 x_5^2 x_6^3 x_7^4 x_9^5 x_{10}^2 x_{11}^2$           | -1             |
| (1, 6, 0, 4, 0) | (3, 3, 3, 0, 1, 1, 1, 3, 1, 1, 1) | 29  | $x_1 x_2 x_3^2 x_5 x_6^2 x_7^4 x_8^3 x_9^5 x_{10}^5 x_{11}^5$   | -1             |
| (1, 6, 0, 3, 1) | (1, 1, 1, 3, 0, 1, 3, 4, 1, 3, 1) | 26  | $x_2^2 x_3^3 x_4^2 x_6^5 x_7^2 x_9^5 x_{10}^2 x_{11}^5$         | $2^2 \cdot 3$  |
| (1, 6, 0, 2, 2) | (1, 1, 0, 1, 1, 4, 4, 1, 3, 3, 1) | 24  | $x_2 x_4^4 x_5^5 x_6 x_7 x_8^5 x_9 x_{10} x_{11}^5$             | 2              |
| (1, 6, 0, 1, 3) | (4, 0, 3, 4, 1, 1, 4, 1, 1, 1, 1) | 26  | $x_7^2 x_5 x_6^3 x_7^2 x_8^3 x_9^5 x_{10}^5 x_{11}^5$           | -1             |
| (1, 6, 0, 0, 4) | (4, 1, 1, 0, 1, 1, 1, 1, 4, 4, 4) | 29  | $x_1 x_2^2 x_3 x_5^3 x_6^5 x_7^5 x_8^5 x_9^3 x_{10}^3 x_{11}^3$ | 1              |
| (1, 5, 5, 0, 0) | (2, 1, 2, 1, 2, 1, 2, 0, 1, 2, 1) | 27  | $x_3^3 x_4 x_5^3 x_6^4 x_7^4 x_9^4 x_{10}^4 x_{11}^4$           | -1             |
| (1, 5, 4, 1, 0) | (1, 2, 2, 1, 1, 0, 2, 1, 3, 1, 2) | 24  | $x_1 x_3^2 x_4^3 x_5^4 x_7^3 x_8^4 x_{10}^4 x_{11}^3$           | $-1 \cdot 3$   |
| (1, 5, 4, 0, 1) | (2, 1, 1, 2, 2, 1, 1, 1, 4, 2, 0) | 24  | $x_1^2 x_3 x_4^3 x_5^3 x_6^4 x_7^4 x_8^4 x_{10}^3$              | 1              |
| (1, 5, 3, 2, 0) | (1, 1, 2, 1, 3, 3, 0, 2, 1, 1, 2) | 22  | $x_2^2 x_3^2 x_4^4 x_5 x_6 x_8^2 x_9^4 x_{10}^4 x_{11}^2$       | $-1 \cdot 3$   |
| (1, 5, 3, 1, 1) | (0, 4, 2, 1, 1, 1, 3, 1, 2, 1, 2) | 21  | $x_4 x_5^4 x_6^4 x_8^4 x_9^2 x_{10}^4 x_{11}^2$                 | $-1 \cdot 2$   |
| (1, 5, 3, 0, 2) | (1, 1, 0, 1, 2, 4, 2, 4, 1, 2, 1) | 22  | $x_1 x_2 x_4^4 x_5^2 x_6 x_7^2 x_8 x_9^4 x_{10}^2 x_{11}^4$     | 2              |
| (1, 5, 2, 3, 0) | (1, 1, 2, 1, 0, 3, 1, 2, 3, 3, 1) | 22  | $x_2^2 x_3 x_4^4 x_6^2 x_7^4 x_8 x_9^2 x_{10}^2 x_{11}^4$       | $2^2 \cdot 3$  |
| (1, 5, 2, 2, 1) | (1, 0, 1, 1, 2, 3, 1, 3, 1, 4, 2) | 20  | $x_3^4 x_4^4 x_5 x_6 x_7^4 x_8 x_9^4 x_{11}$                    | $-1 \cdot 3$   |
| (1, 5, 2, 1, 2) | (1, 0, 1, 1, 1, 3, 4, 1, 2, 4, 2) | 19  | $x_3^3 x_4^4 x_5^4 x_7 x_8^4 x_9 x_{10} x_{11}$                 | -1             |
| (1, 5, 2, 0, 3) | (1, 1, 0, 1, 2, 4, 4, 1, 1, 2, 4) | 22  | $x_1 x_2^2 x_4^4 x_5 x_6 x_7^2 x_8^4 x_9^4 x_{10} x_{11}^2$     | $-1 \cdot 2^2$ |
| (1, 5, 1, 4, 0) | (1, 1, 1, 3, 1, 3, 2, 3, 3, 1, 0) | 24  | $x_2 x_3^4 x_4^2 x_5^4 x_6^3 x_8^3 x_9^3 x_{10}^4$              | $-1 \cdot 3$   |
| (1, 5, 1, 3, 1) | (1, 0, 1, 2, 3, 1, 1, 4, 3, 3, 1) | 20  | $x_3^2 x_5^2 x_6^4 x_7^4 x_9^2 x_{10}^2 x_{11}^4$               | $-1 \cdot 2$   |
| (1, 5, 1, 2, 2) | (1, 0, 1, 3, 4, 1, 3, 4, 1, 1, 2) | 20  | $x_1^2 x_3^3 x_5 x_6^4 x_7 x_8 x_9^4 x_{10}^4$                  | $-1 \cdot 2$   |
| (1, 5, 1, 1, 3) | (1, 0, 1, 4, 2, 4, 1, 1, 1, 4, 3) | 21  | $x_3^4 x_4^2 x_6^2 x_7^3 x_8^4 x_9^4 x_{10}^2$                  | $-1 \cdot 2$   |
| (1, 5, 1, 0, 4) | (1, 1, 0, 4, 1, 1, 1, 2, 4, 4, 4) | 24  | $x_2^2 x_4^2 x_5^4 x_6^4 x_7^2 x_9^3 x_{10}^3 x_{11}^3$         | 1              |
| (1, 5, 0, 4, 1) | (1, 1, 3, 1, 1, 3, 3, 1, 0, 4, 3) | 24  | $x_1 x_2 x_3^2 x_4^4 x_5^4 x_6^3 x_7^2 x_8^4 x_{11}^3$          | $-1 \cdot 3$   |

$$S \subseteq \mathbb{Z}_p \times \mathbb{Z}_5 \setminus \{(0, 0)\}, |S| = 11$$

| $\lambda$        | $\mathbf{a}$                      | deg | monomial/s                                                                   | coefficient/s        |
|------------------|-----------------------------------|-----|------------------------------------------------------------------------------|----------------------|
| (1, 5, 0, 3, 2)  | (1, 1, 1, 0, 3, 3, 1, 4, 1, 3, 4) | 22  | $x_2^3 x_3^4 x_5 x_6^2 x_7^4 x_8 x_9^4 x_{10}^2 x_{11}$                      | $2^2$                |
| (1, 5, 0, 2, 3)  | (1, 1, 1, 4, 4, 3, 1, 3, 1, 0, 4) | 22  | $x_1 x_2 x_3^4 x_4^2 x_5^2 x_6 x_7^4 x_8 x_9^4 x_{11}^2$                     | $-1 \cdot 2 \cdot 3$ |
| (1, 5, 0, 1, 4)  | (4, 1, 1, 1, 1, 4, 0, 1, 3, 4, 4) | 24  | $x_1 x_2 x_3 x_4^4 x_5^4 x_6^3 x_8^4 x_{10}^3 x_{11}^3$                      | -1                   |
| (1, 5, 0, 0, 5)  | (4, 4, 0, 4, 4, 1, 4, 1, 1, 1, 1) | 27  | $x_2 x_4^2 x_5^3 x_6^2 x_7^4 x_8^3 x_9^4 x_{10}^4 x_{11}^4$                  | 1                    |
| (1, 4, 4, 2, 0)  | (1, 0, 1, 2, 3, 1, 2, 3, 1, 2, 2) | 21  | $x_3 x_4^3 x_5 x_6^3 x_7^3 x_8 x_9^3 x_{10}^3 x_{11}^3$                      | $-1 \cdot 3^2$       |
| (1, 4, 4, 1, 1)  | (1, 1, 0, 1, 2, 1, 2, 2, 4, 3, 2) | 20  | $x_2^2 x_4^3 x_5^3 x_6^3 x_7^3 x_8^3 x_{11}^3$                               | $-1 \cdot 2^2$       |
| (1, 4, 4, 0, 2)  | (1, 0, 2, 4, 2, 1, 1, 2, 4, 2, 1) | 20  | $x_4 x_3^3 x_6^3 x_7^3 x_8^3 x_9 x_{10}^3 x_{11}^3$                          | $2^4$                |
| (1, 4, 3, 3, 0)  | (1, 1, 1, 2, 1, 2, 3, 3, 3, 2, 0) | 20  | $x_2^2 x_3^3 x_4^2 x_5^3 x_6^2 x_7^2 x_8^2 x_9^2 x_{10}^2$                   | $-1 \cdot 2$         |
| (1, 4, 3, 2, 1)  | (1, 0, 1, 1, 3, 2, 1, 3, 2, 2, 4) | 18  | $x_1^2 x_3^2 x_4^3 x_5 x_6^2 x_7^3 x_8 x_9^2 x_{10}^2$                       | $-1 \cdot 3$         |
| (1, 4, 3, 1, 2)  | (0, 2, 1, 3, 2, 1, 4, 1, 1, 2, 4) | 18  | $x_2^2 x_3 x_5^2 x_6^3 x_7 x_8^3 x_9^3 x_{10}^2 x_{11}$                      | 1                    |
| (1, 4, 3, 0, 3)  | (1, 0, 2, 4, 1, 1, 1, 4, 2, 2, 4) | 20  | $x_3 x_4^2 x_5^3 x_6^3 x_7^2 x_8^2 x_9^2 x_{10}^2 x_{11}^2$                  | $-1 \cdot 3$         |
| (1, 4, 2, 3, 1)  | (0, 3, 1, 2, 3, 1, 2, 1, 3, 1, 4) | 18  | $x_3^3 x_4 x_5^2 x_6^3 x_7 x_8^2 x_9^2 x_{10}^3$                             | $3^2$                |
| (1, 4, 2, 2, 2)  | (0, 1, 3, 2, 1, 3, 2, 1, 1, 4, 4) | 17  | $x_2^3 x_3 x_4 x_5^3 x_6 x_7 x_8^2 x_9^3 x_{10} x_{11}$                      | $2^2$                |
| (1, 4, 2, 1, 3)  | (0, 1, 2, 4, 4, 1, 2, 1, 4, 3, 1) | 18  | $x_2 x_3 x_4^2 x_5^2 x_6^3 x_7 x_8^3 x_9^2 x_{11}^3$                         | $2^3$                |
| (1, 4, 2, 0, 4)  | (1, 1, 1, 4, 1, 4, 2, 2, 4, 4, 0) | 21  | $x_2 x_3^3 x_4^3 x_5^3 x_6^3 x_7 x_8 x_9^3 x_{10}^3$                         | $-1 \cdot 2^2$       |
| (1, 4, 1, 3, 2)  | (0, 1, 3, 2, 4, 1, 3, 3, 1, 4, 1) | 18  | $x_2^2 x_3^2 x_5 x_6^3 x_7^2 x_8^2 x_9^2 x_{10} x_{11}^3$                    | 2                    |
| (1, 4, 1, 2, 3)  | (0, 3, 4, 1, 4, 2, 1, 1, 1, 4, 3) | 18  | $x_2 x_4^3 x_5^2 x_7^3 x_8^3 x_9^3 x_{10}^2 x_{11}$                          | -1                   |
| (1, 4, 1, 1, 4)  | (1, 0, 1, 4, 2, 1, 4, 1, 4, 4, 3) | 19  | $x_3^2 x_4^2 x_6^3 x_7^3 x_8^3 x_9^3 x_{10}^3$                               | 1                    |
| (1, 4, 0, 3, 3)  | (1, 1, 4, 0, 3, 1, 3, 1, 4, 4, 3) | 19  | $x_2^2 x_3^2 x_5 x_6^3 x_7^2 x_8^3 x_9^2 x_{10}^2 x_{11}^2$                  | $2^2$                |
| (1, 3, 3, 3, 1)  | (0, 1, 1, 2, 2, 2, 3, 4, 3, 1, 3) | 17  | $x_2 x_3^2 x_4^2 x_5^2 x_6^2 x_7^2 x_9^2 x_{10}^2 x_{11}^2$                  | $-1 \cdot 2$         |
| (1, 3, 3, 2, 2)  | (0, 1, 1, 2, 2, 4, 3, 1, 3, 4, 2) | 16  | $x_2^2 x_3^2 x_4^2 x_5^2 x_6 x_7 x_8^2 x_9 x_{10} x_{11}^2$                  | $2^2$                |
| (1, 3, 2, 2, 3)  | (1, 1, 2, 4, 4, 4, 2, 1, 0, 3, 3) | 15  | $x_1 x_2^2 x_3 x_4^2 x_5^2 x_6^2 x_7 x_8^2 x_{10} x_{11}$                    | 1                    |
| (0, 11, 0, 0, 0) | (1, 1, 1, 1, 1, 1, 1, 1, 1, 1, 1) | 64  | $x_1^2 x_2^2 x_3^3 x_4^4 x_5^6 x_6^9 x_8^8 x_9^{10} x_{10}^{10} x_{11}^{10}$ | 1                    |
| (0, 10, 1, 0, 0) | (1, 1, 1, 1, 1, 1, 1, 2, 1, 1, 1) | 55  | $x_1 x_2^3 x_3^3 x_4^5 x_5^7 x_6^9 x_9^9 x_{10}^9 x_{11}^9$                  | 3                    |
| (0, 10, 0, 1, 0) | (1, 1, 1, 1, 1, 1, 1, 3, 1, 1, 1) | 55  | $x_1 x_2^3 x_3^4 x_4^4 x_5^7 x_6^9 x_9^9 x_{10}^9 x_{11}^9$                  | 2                    |
| (0, 10, 0, 0, 1) | (1, 1, 1, 1, 1, 1, 1, 4, 1, 1, 1) | 54  | $x_1 x_2^2 x_3^3 x_4^5 x_5^7 x_6^9 x_9^9 x_{10}^9 x_{11}^9$                  | 1                    |

$$S \subseteq \mathbb{Z}_p \times \mathbb{Z}_5 \setminus \{(0, 0)\}, |S| = 11$$

| $\lambda$       | $\mathbf{a}$                      | deg | monomial/s                                                        | coefficient/s  |
|-----------------|-----------------------------------|-----|-------------------------------------------------------------------|----------------|
| (0, 9, 2, 0, 0) | (2, 1, 1, 2, 1, 1, 1, 1, 1, 1, 1) | 46  | $x_2^2 x_3^2 x_4 x_5^4 x_6^7 x_8^6 x_9^8 x_{10}^8 x_{11}^8$       | 1              |
| (0, 9, 1, 1, 0) | (1, 1, 3, 1, 1, 1, 1, 1, 2, 1, 1) | 45  | $x_1 x_2^3 x_4^4 x_5^5 x_6^8 x_8^8 x_{10}^8 x_{11}^8$             | 2              |
| (0, 9, 1, 0, 1) | (1, 1, 1, 1, 1, 1, 1, 1, 1, 4, 2) | 44  | $x_1 x_2^2 x_3^4 x_4^5 x_5^8 x_6^8 x_8^8 x_9^8$                   | 2              |
| (0, 9, 0, 2, 0) | (1, 1, 1, 3, 1, 1, 1, 1, 3, 1, 1) | 45  | $x_1 x_2^2 x_3^3 x_4 x_5^5 x_6^8 x_8 x_9^8 x_{10}^8 x_{11}^8$     | -1             |
| (0, 9, 0, 1, 1) | (1, 1, 1, 1, 4, 1, 1, 1, 1, 1, 3) | 45  | $x_1^2 x_2^2 x_3^4 x_4^6 x_5^7 x_8^8 x_9^8 x_{10}^8$              | -1             |
| (0, 9, 0, 0, 2) | (4, 4, 1, 1, 1, 1, 1, 1, 1, 1, 1) | 46  | $x_2 x_3^2 x_4^3 x_5^3 x_6^7 x_8^8 x_9^8 x_{10}^8 x_{11}^8$       | -1             |
| (0, 8, 3, 0, 0) | (1, 2, 2, 1, 1, 1, 1, 2, 1, 1, 1) | 40  | $x_1 x_3^2 x_4^3 x_5^4 x_6^7 x_8^2 x_9^7 x_{10}^7 x_{11}^7$       | -1 · 3         |
| (0, 8, 2, 1, 0) | (2, 1, 3, 1, 1, 1, 1, 1, 1, 2, 1) | 37  | $x_2 x_4^4 x_5^4 x_6^6 x_7^8 x_9^7 x_{10}^7 x_{11}^7$             | 1              |
| (0, 8, 2, 0, 1) | (2, 1, 1, 2, 1, 1, 4, 1, 1, 1, 1) | 38  | $x_2^2 x_4 x_5^3 x_6^6 x_8^6 x_9^6 x_{10}^7 x_{11}^7$             | -1             |
| (0, 8, 1, 2, 0) | (1, 1, 2, 1, 3, 3, 1, 1, 1, 1, 1) | 38  | $x_1^2 x_2^2 x_4^7 x_6 x_8^5 x_9^7 x_{10}^7 x_{11}^7$             | -1             |
| (0, 8, 1, 1, 1) | (3, 1, 1, 1, 4, 1, 1, 1, 1, 2, 1) | 37  | $x_2 x_3^3 x_4^6 x_6^6 x_8^7 x_9^7 x_{11}^7$                      | 1              |
| (0, 8, 1, 0, 2) | (1, 1, 1, 1, 1, 4, 4, 1, 2, 1, 1) | 38  | $x_1 x_2 x_3^3 x_4^4 x_5^7 x_6 x_8^7 x_{10}^7 x_{11}^7$           | 2              |
| (0, 8, 0, 3, 0) | (3, 1, 3, 1, 1, 1, 1, 1, 3, 1, 1) | 40  | $x_2 x_3^2 x_4^3 x_5^5 x_6^6 x_8^7 x_9^2 x_{10}^7 x_{11}^7$       | 1              |
| (0, 8, 0, 2, 1) | (4, 1, 1, 3, 1, 1, 1, 1, 1, 3, 1) | 38  | $x_2^2 x_3^3 x_4 x_5^5 x_6^5 x_8^7 x_9^7 x_{10}^7 x_{11}^7$       | 1              |
| (0, 8, 0, 1, 2) | (4, 1, 1, 1, 3, 1, 1, 1, 1, 4, 1) | 38  | $x_1 x_2^2 x_3^2 x_4^5 x_6^6 x_8^7 x_9^7 x_{10}^7 x_{11}^7$       | -1             |
| (0, 8, 0, 0, 3) | (1, 1, 1, 1, 4, 4, 1, 1, 1, 1, 4) | 39  | $x_1 x_2^2 x_3^3 x_4^6 x_5^2 x_6^2 x_8^7 x_9^7 x_{10}^7 x_{11}^2$ | 2              |
| (0, 7, 4, 0, 0) | (1, 1, 1, 1, 2, 1, 2, 2, 2, 1, 1) | 35  | $x_2 x_3^2 x_4^5 x_5^3 x_6^6 x_8^3 x_9^3 x_{10}^6 x_{11}^6$       | 3 <sup>2</sup> |
| (0, 7, 3, 1, 0) | (3, 1, 1, 1, 1, 1, 2, 1, 1, 2, 2) | 33  | $x_3^2 x_4^3 x_5^4 x_6^6 x_7^2 x_8^6 x_9^6 x_{10}^2 x_{11}^2$     | 3              |
| (0, 7, 3, 0, 1) | (4, 2, 1, 1, 2, 1, 2, 1, 1, 1, 1) | 33  | $x_3 x_4 x_5^2 x_6^4 x_7^2 x_8^5 x_9^6 x_{10}^6 x_{11}^6$         | -1 · 2         |
| (0, 7, 2, 2, 0) | (1, 1, 1, 1, 1, 1, 2, 1, 3, 3, 2) | 32  | $x_2^3 x_3^2 x_4^5 x_5^6 x_6^6 x_7 x_8^6 x_9 x_{10} x_{11}$       | -1 · 2         |
| (0, 7, 2, 1, 1) | (1, 3, 2, 4, 2, 1, 1, 1, 1, 1, 1) | 31  | $x_1 x_3 x_5 x_6^2 x_7^3 x_8^5 x_9^6 x_{10}^6 x_{11}^6$           | -1             |
| (0, 7, 2, 0, 2) | (1, 1, 4, 1, 1, 1, 2, 2, 1, 1, 4) | 32  | $x_2^2 x_3 x_4^3 x_5^6 x_6^6 x_7 x_8 x_9^5 x_{10}^6 x_{11}$       | 2              |
| (0, 7, 1, 3, 0) | (1, 1, 1, 2, 3, 1, 1, 1, 3, 3, 1) | 33  | $x_2 x_3^4 x_5^2 x_6^4 x_7^6 x_8^6 x_9^2 x_{10}^2 x_{11}^6$       | 2              |
| (0, 7, 1, 2, 1) | (3, 1, 1, 1, 1, 3, 2, 4, 1, 1, 1) | 31  | $x_1 x_2 x_3^2 x_4^2 x_5^6 x_6^6 x_9^6 x_{10}^6 x_{11}^6$         | 1              |
| (0, 7, 1, 1, 2) | (1, 1, 1, 1, 3, 4, 1, 2, 4, 1, 1) | 30  | $x_2 x_3^3 x_4^6 x_6^6 x_7 x_9 x_{10}^6 x_{11}^6$                 | 1              |

$$S \subseteq \mathbb{Z}_p \times \mathbb{Z}_5 \setminus \{(0, 0)\}, |S| = 11$$

| $\lambda$       | $\mathbf{a}$                         | deg | monomial/s                                             | coefficient/s          |
|-----------------|--------------------------------------|-----|--------------------------------------------------------|------------------------|
| (0, 7, 1, 0, 3) | (4, 1, 2, 1, 4, 4, 1, 1, 1, 1, 1)    | 33  | $x_2x_4^2x_5^2x_6^2x_7^4x_8^4x_9^6x_{10}^6x_{11}^6$    | -1                     |
| (0, 7, 0, 4, 0) | (1, 1, 3, 1, 3, 3, 1, 1, 1, 1, 3, 1) | 36  | $x_1x_2^2x_3x_4^5x_5^3x_6^3x_8^6x_9^6x_{10}^3x_{11}^6$ | 2                      |
| (0, 7, 0, 3, 1) | (1, 3, 3, 1, 1, 3, 4, 1, 1, 1, 1, 1) | 32  | $x_3x_4x_5^5x_6^2x_8^5x_9^6x_{10}^6x_{11}^6$           | 1                      |
| (0, 7, 0, 2, 2) | (1, 3, 4, 4, 1, 3, 1, 1, 1, 1, 1, 1) | 32  | $x_1x_4x_5^4x_6x_7^3x_8^5x_9^5x_{10}^6x_{11}^6$        | 1                      |
| (0, 7, 0, 1, 3) | (4, 1, 4, 4, 1, 1, 1, 1, 4, 1, 3, 1) | 33  | $x_2x_3^2x_4^3x_5^3x_6^4x_7^6x_8^2x_9^6x_{11}^6$       | -1                     |
| (0, 7, 0, 0, 4) | (4, 4, 1, 1, 1, 1, 4, 4, 1, 1, 1, 1) | 36  | $x_1x_2^3x_3x_4^2x_5^6x_6^3x_8^6x_9^6x_{10}^6x_{11}^6$ | -1                     |
| (0, 6, 5, 0, 0) | (2, 2, 1, 1, 2, 1, 1, 2, 1, 1, 2)    | 34  | $x_2x_3^3x_4^3x_5^4x_6^5x_8^4x_9^5x_{10}^5x_{11}^4$    | $-1 \cdot 2 \cdot 5$   |
| (0, 6, 4, 1, 0) | (2, 1, 1, 2, 2, 3, 1, 2, 1, 1, 1)    | 30  | $x_1x_3^2x_4x_5^3x_7^5x_8^3x_9^5x_{10}^5x_{11}^5$      | 1                      |
| (0, 6, 4, 0, 1) | (2, 1, 2, 4, 1, 1, 1, 2, 2, 1, 1)    | 30  | $x_2x_3^3x_5^3x_6^2x_7^5x_8^3x_9^3x_{10}^5x_{11}^5$    | 1                      |
| (0, 6, 3, 2, 0) | (2, 1, 1, 2, 1, 3, 1, 3, 1, 2, 1)    | 28  | $x_2x_3x_4^2x_5^5x_6x_7^5x_8x_9^5x_{10}^2x_{11}^5$     | 2                      |
| (0, 6, 3, 1, 1) | (1, 3, 1, 2, 1, 4, 1, 2, 1, 2, 1)    | 27  | $x_1x_3^2x_5^5x_7^2x_8^5x_9^5x_{10}^2x_{11}^5$         | 1                      |
| (0, 6, 3, 0, 2) | (1, 1, 2, 4, 2, 1, 1, 1, 1, 2, 4)    | 27  | $x_2x_3^2x_4x_5^2x_6^4x_7^4x_8^5x_9^5x_{10}^2x_{11}$   | -1                     |
| (0, 6, 2, 3, 0) | (1, 3, 3, 1, 3, 1, 1, 2, 2, 1, 1)    | 28  | $x_2x_3x_4^3x_5^2x_6^4x_7^5x_8x_9x_{10}^5x_{11}^5$     | 1                      |
| (0, 6, 2, 2, 1) | (1, 1, 2, 3, 1, 1, 4, 3, 1, 1, 2)    | 25  | $x_2x_3x_4x_5^5x_6^5x_8x_9^5x_{10}^5x_{11}$            | $-1 \cdot 2$           |
| (0, 6, 2, 1, 2) | (1, 1, 2, 1, 3, 1, 4, 1, 2, 1, 4)    | 26  | $x_1x_2x_3x_4^5x_5^5x_7x_8^5x_9x_{10}^5x_{11}$         | 1                      |
| (0, 6, 2, 0, 3) | (2, 1, 1, 4, 1, 2, 1, 4, 4, 1, 1)    | 28  | $x_1x_3x_4x_5^5x_6x_7^5x_8^2x_9^2x_{10}^5x_{11}^5$     | $-1 \cdot 2$           |
| (0, 6, 1, 4, 0) | (2, 1, 3, 3, 1, 1, 1, 1, 1, 3, 3)    | 29  | $x_2x_4x_5^3x_6^3x_7^5x_8^5x_9^5x_{10}^3x_{11}^3$      | -1                     |
| (0, 6, 1, 3, 1) | (4, 3, 1, 1, 1, 3, 2, 1, 1, 1, 3)    | 27  | $x_3x_4^3x_5^5x_6^2x_8^4x_9^5x_{10}^2x_{11}^2$         | $-1 \cdot 3$           |
| (0, 6, 1, 2, 2) | (1, 3, 4, 1, 1, 2, 1, 4, 1, 3, 1)    | 26  | $x_4^4x_5^5x_7^5x_8x_9^5x_{10}x_{11}^5$                | 1                      |
| (0, 6, 1, 1, 3) | (1, 1, 1, 3, 1, 2, 4, 1, 1, 4, 4)    | 27  | $x_2x_3^5x_5^5x_7^2x_8^5x_9^5x_{10}^2x_{11}^2$         | $-1 \cdot 2^2$         |
| (0, 6, 1, 0, 4) | (1, 4, 1, 2, 4, 4, 1, 1, 1, 4, 1)    | 30  | $x_2x_3^2x_5^2x_6^3x_7^4x_8^5x_9^5x_{10}^3x_{11}^5$    | 1                      |
| (0, 6, 0, 5, 0) | (3, 1, 1, 3, 3, 1, 1, 1, 3, 3, 1)    | 34  | $x_2x_3^3x_4^3x_5^4x_6^5x_8^4x_9^4x_{10}^4x_{11}^5$    | 3                      |
| (0, 6, 0, 4, 1) | (3, 1, 1, 1, 1, 1, 3, 4, 3, 1, 3)    | 30  | $x_3^2x_4^4x_5^5x_6^5x_7^3x_9^3x_{10}^3x_{11}^3$       | 2                      |
| (0, 6, 0, 3, 2) | (1, 1, 1, 1, 3, 4, 3, 1, 1, 4, 3)    | 28  | $x_2x_3^4x_4^5x_5^2x_6x_7^2x_8^5x_9^5x_{10}x_{11}^2$   | $-1 \cdot 2^2 \cdot 3$ |
| (0, 6, 0, 2, 3) | (1, 4, 3, 4, 4, 1, 1, 1, 3, 1, 1)    | 28  | $x_2x_3x_4^2x_5^2x_6^2x_7^4x_8^5x_9x_{10}^5x_{11}^5$   | 1                      |
| (0, 6, 0, 1, 4) | (1, 1, 4, 1, 1, 1, 4, 1, 4, 3, 4)    | 29  | $x_2x_3x_4^3x_5^5x_6^5x_7^3x_8^5x_9^3x_{11}^3$         | -1                     |

$$S \subseteq \mathbb{Z}_p \times \mathbb{Z}_5 \setminus \{(0, 0)\}, |S| = 11$$

| $\lambda$       | $\mathbf{a}$                      | deg | monomial/s                                                                                                             | coefficient/s            |
|-----------------|-----------------------------------|-----|------------------------------------------------------------------------------------------------------------------------|--------------------------|
| (0, 6, 0, 0, 5) | (4, 4, 4, 4, 1, 1, 1, 1, 4, 1, 1) | 34  | $x_2 x_3^3 x_4^4 x_5^2 x_6^5 x_8^5 x_9^4 x_{10}^5 x_{11}^5$                                                            | 1                        |
| (0, 5, 5, 1, 0) | (1, 1, 2, 3, 2, 2, 2, 2, 1, 1, 1) | 29  | $x_2^2 x_3 x_5^2 x_6^4 x_7^4 x_8^4 x_9^4 x_{10}^4 x_{11}^4$                                                            | 1                        |
| (0, 5, 5, 0, 1) | (1, 2, 4, 1, 2, 1, 2, 1, 2, 1, 2) | 29  | $x_4^2 x_5^3 x_6^4 x_7^4 x_8^4 x_9^4 x_{10}^4 x_{11}^4$<br>$x_4^3 x_5^2 x_6^4 x_7^4 x_8^4 x_9^4 x_{10}^4 x_{11}^4$     | -1 · 2 · 5<br>-1 · 2 · 7 |
| (0, 5, 4, 2, 0) | (3, 1, 2, 1, 3, 2, 2, 1, 1, 2, 1) | 26  | $x_2 x_3 x_4^2 x_5 x_6^3 x_7^3 x_8^4 x_9^4 x_{10}^3 x_{11}^4$                                                          | 2 <sup>3</sup>           |
| (0, 5, 4, 1, 1) | (2, 1, 1, 1, 1, 3, 2, 2, 4, 2, 1) | 24  | $x_1^2 x_3 x_4^4 x_5^4 x_7^3 x_8^3 x_{10}^3 x_{11}^4$                                                                  | 1                        |
| (0, 5, 4, 0, 2) | (1, 1, 4, 2, 1, 1, 2, 2, 4, 2, 1) | 26  | $x_1 x_2^2 x_3 x_4 x_5^3 x_6^4 x_7^3 x_8^3 x_9 x_{10}^3 x_{11}^4$                                                      | -1 · 2                   |
| (0, 5, 3, 3, 0) | (1, 2, 2, 1, 3, 3, 1, 3, 1, 2, 1) | 24  | $x_2 x_3^2 x_4^2 x_5 x_6^2 x_7^2 x_8^4 x_9^2 x_{10}^4 x_{11}^4$                                                        | 2                        |
| (0, 5, 3, 2, 1) | (1, 2, 2, 4, 3, 1, 1, 3, 1, 2, 1) | 23  | $x_1 x_3^2 x_5 x_6^4 x_7^4 x_8 x_9^4 x_{10}^2 x_{11}^4$                                                                | 2                        |
| (0, 5, 3, 1, 2) | (1, 1, 2, 4, 1, 4, 2, 2, 3, 1, 1) | 23  | $x_1 x_2^4 x_3 x_5^4 x_6 x_7^2 x_8^2 x_{10}^4 x_{11}^4$                                                                | 1                        |
| (0, 5, 3, 0, 3) | (2, 4, 1, 2, 4, 2, 4, 1, 1, 1, 1) | 25  | $x_3^2 x_4^2 x_5^2 x_6^2 x_7^2 x_8^3 x_9^4 x_{10}^4 x_{11}^4$                                                          | 2                        |
| (0, 5, 2, 4, 0) | (1, 1, 1, 2, 3, 3, 3, 3, 2, 1, 1) | 26  | $x_1 x_2 x_3^4 x_4 x_5 x_6^3 x_7^3 x_8^3 x_9 x_{10}^4 x_{11}^4$                                                        | 1                        |
| (0, 5, 2, 3, 1) | (1, 1, 4, 2, 3, 3, 1, 2, 1, 1, 3) | 23  | $x_2^3 x_4 x_5^2 x_6^2 x_7^4 x_8 x_9^4 x_{10}^4 x_{11}^2$                                                              | -1 · 3                   |
| (0, 5, 2, 2, 2) | (1, 1, 3, 4, 2, 1, 2, 4, 1, 3, 1) | 22  | $x_2^4 x_3 x_4 x_5 x_6^4 x_7 x_8 x_9^4 x_{10} x_{11}^4$<br>$x_1 x_2^3 x_3 x_4 x_5 x_6^4 x_7 x_8 x_9^4 x_{10} x_{11}^4$ | 5 · 7<br>47              |
| (0, 5, 2, 1, 3) | (1, 1, 1, 4, 2, 4, 4, 2, 1, 1, 3) | 23  | $x_1 x_2^2 x_3^4 x_4^2 x_5 x_6^2 x_7^2 x_8 x_9^4 x_{10}^4$                                                             | -1                       |
| (0, 5, 2, 0, 4) | (1, 1, 4, 2, 4, 2, 1, 4, 4, 1, 1) | 25  | $x_2 x_3^2 x_5^3 x_6 x_7^4 x_8^3 x_9^3 x_{10}^4 x_{11}^4$                                                              | 3                        |
| (0, 5, 1, 4, 1) | (2, 3, 1, 3, 4, 3, 1, 1, 1, 3, 1) | 25  | $x_2 x_4^2 x_6^3 x_7^4 x_8^4 x_9^3 x_{10}^4 x_{11}^4$                                                                  | -1                       |
| (0, 5, 1, 3, 2) | (1, 1, 1, 3, 2, 4, 1, 1, 3, 3, 4) | 23  | $x_2^3 x_3^4 x_4^2 x_6 x_7^4 x_8^4 x_9^2 x_{10}^2 x_{11}$                                                              | -1                       |
| (0, 5, 1, 2, 3) | (1, 3, 1, 2, 1, 1, 4, 3, 1, 4, 4) | 22  | $x_3^3 x_5^4 x_6^4 x_7 x_8 x_9^4 x_{10}^2 x_{11}^2$                                                                    | -1                       |
| (0, 5, 1, 1, 4) | (2, 1, 1, 4, 1, 4, 3, 1, 4, 4, 1) | 25  | $x_3 x_4^3 x_5^4 x_6^3 x_8^4 x_9^3 x_{10}^4 x_{11}^4$                                                                  | 3                        |
| (0, 5, 1, 0, 5) | (1, 1, 2, 1, 4, 4, 1, 4, 4, 4, 1) | 29  | $x_2^2 x_4^3 x_5 x_6^3 x_7^4 x_8^4 x_9^4 x_{10}^4 x_{11}^4$                                                            | 1                        |
| (0, 5, 0, 4, 2) | (4, 3, 1, 3, 4, 1, 1, 1, 1, 3, 3) | 25  | $x_3 x_4^3 x_5 x_6^2 x_7^4 x_8^4 x_9^3 x_{10}^3 x_{11}^3$                                                              | 2                        |
| (0, 5, 0, 3, 3) | (3, 1, 4, 1, 3, 4, 1, 1, 4, 3, 1) | 25  | $x_3 x_4^4 x_5^2 x_6^2 x_7^4 x_8^4 x_9^2 x_{10}^2 x_{11}^4$                                                            | -1 · 2                   |
| (0, 5, 0, 2, 4) | (1, 4, 3, 4, 1, 1, 1, 4, 4, 3, 1) | 26  | $x_2 x_4^3 x_5^4 x_6^3 x_7^4 x_8^3 x_9^3 x_{10}^4 x_{11}^4$                                                            | 2                        |
| (0, 4, 4, 3, 0) | (3, 1, 2, 1, 3, 1, 2, 1, 3, 2, 2) | 24  | $x_2 x_3 x_4^3 x_5^2 x_6^3 x_7^3 x_8^3 x_9^2 x_{10}^3 x_{11}^3$                                                        | 1                        |

$$S \subseteq \mathbb{Z}_p \times \mathbb{Z}_5 \setminus \{(0, 0)\}, |S| = 11$$

| $\lambda$       | $\mathbf{a}$                      | deg | monomial/s                                                                                                                            | coefficient/s                  |
|-----------------|-----------------------------------|-----|---------------------------------------------------------------------------------------------------------------------------------------|--------------------------------|
| (0, 4, 4, 2, 1) | (1, 1, 1, 1, 2, 2, 2, 3, 4, 2, 3) | 22  | $x_2^2 x_3^3 x_4^4 x_5^3 x_6^3 x_7^3 x_8 x_9 x_{10} x_{11}$                                                                           | 1                              |
| (0, 4, 4, 1, 2) | (1, 2, 4, 2, 4, 1, 2, 1, 3, 1, 2) | 22  | $x_2^2 x_3 x_4^3 x_5 x_6^3 x_7^3 x_8^3 x_9^3 x_{10}^3 x_{11}^3$                                                                       | 3                              |
| (0, 4, 4, 0, 3) | (2, 1, 2, 1, 4, 4, 2, 1, 2, 4, 1) | 24  | $\frac{x_3^3 x_4^3 x_5^2 x_6^2 x_7^3 x_8^3 x_9^2 x_{10}^3 x_{11}^3}{x_2 x_3^2 x_4^3 x_5^2 x_6^2 x_7^3 x_8^3 x_9^2 x_{10}^3 x_{11}^3}$ | $-1 \cdot 19$<br>$-1 \cdot 29$ |
| (0, 4, 3, 3, 1) | (1, 1, 2, 4, 1, 2, 1, 2, 3, 3, 3) | 21  | $x_2^3 x_3^2 x_5^3 x_6^2 x_7^3 x_8^2 x_9^2 x_{10}^2 x_{11}^2$                                                                         | 2                              |
| (0, 4, 3, 2, 2) | (1, 1, 1, 3, 1, 2, 3, 2, 4, 2, 4) | 20  | $x_1 x_2^3 x_3^3 x_4 x_5^3 x_6^2 x_7 x_8^2 x_9 x_{10}^2 x_{11}$                                                                       | 1                              |
| (0, 4, 3, 1, 3) | (1, 2, 4, 2, 1, 4, 3, 1, 1, 2, 4) | 20  | $x_2 x_3^2 x_4^2 x_5^3 x_6^2 x_8^3 x_9^2 x_{10}^2 x_{11}^2$                                                                           | $-1 \cdot 2$                   |
| (0, 4, 3, 0, 4) | (4, 1, 1, 4, 2, 2, 4, 4, 1, 1, 2) | 24  | $x_2 x_3^3 x_4^3 x_5^2 x_6^2 x_7^3 x_8^3 x_9^3 x_{10}^3 x_{11}^2$                                                                     | $-1 \cdot 3$                   |
| (0, 4, 2, 3, 2) | (1, 1, 2, 3, 1, 3, 3, 4, 2, 1, 4) | 19  | $x_2^3 x_3 x_4^2 x_5^3 x_6^2 x_7^2 x_8 x_9 x_{10}^3 x_{11}$                                                                           | 3                              |
| (0, 4, 2, 2, 3) | (1, 1, 3, 4, 2, 2, 1, 1, 3, 4, 4) | 20  | $x_1 x_2^3 x_3 x_4^2 x_5 x_6^3 x_7^3 x_8^3 x_9 x_{10}^2 x_{11}^2$                                                                     | $-1 \cdot 2^2$                 |
| (0, 4, 2, 1, 4) | (1, 2, 1, 4, 2, 1, 1, 4, 3, 4, 4) | 22  | $x_3^3 x_4^3 x_5 x_6^3 x_7^3 x_8^3 x_{10}^3 x_{11}^3$                                                                                 | -1                             |
| (0, 4, 1, 3, 3) | (1, 3, 1, 1, 3, 4, 4, 3, 1, 2, 4) | 21  | $x_2^2 x_3^3 x_4^3 x_5^2 x_6^2 x_7^2 x_8^3 x_9^3 x_{11}^2$                                                                            | $2 \cdot 3$                    |
| (0, 3, 3, 3, 2) | (1, 1, 3, 3, 2, 3, 4, 2, 4, 1, 2) | 19  | $x_1 x_2^2 x_3^2 x_4^2 x_5^2 x_6^2 x_7 x_8^2 x_9 x_{10}^2 x_{11}^2$                                                                   | 1                              |

$$S \subseteq \mathbb{Z}_p \times \mathbb{Z}_2 \setminus \{(0, 0)\}, |S| = 12$$

| $\lambda$ | $\mathbf{a}$                         | deg | monomial/s                                                                                                                                                                                                                                          | coefficient/s                                                                                                 |
|-----------|--------------------------------------|-----|-----------------------------------------------------------------------------------------------------------------------------------------------------------------------------------------------------------------------------------------------------|---------------------------------------------------------------------------------------------------------------|
| (12, 0)   | (0, 0, 0, 0, 0, 0, 0, 0, 0, 0, 0, 0) | 131 | $\frac{x_1^{10} x_2^{11} x_3^{11} x_4^{11} x_5^{11} x_6^{11} x_7^{11} x_8^{11} x_9^{11} x_{10}^{11} x_{11}^{11} x_{12}^{11}}{x_1^{11} x_2^{10} x_3^{11} x_4^{11} x_5^{11} x_6^{11} x_7^{11} x_8^{11} x_9^{11} x_{10}^{11} x_{11}^{11} x_{12}^{11}}$ | $2^4 \cdot 3 \cdot 29 \cdot 12953077208391719881$<br>$2^3 \cdot 3 \cdot 277 \cdot 1901 \cdot 786640832519761$ |
| (11, 1)   | (0, 0, 0, 0, 0, 0, 1, 0, 0, 0, 0, 0) | 80  | $\frac{x_1 x_2^3 x_3^7 x_4^{10} x_6^{10} x_8^9 x_9^{10} x_{10}^{10} x_{11}^{10} x_{12}^{10}}{x_1 x_2^4 x_3^6 x_4^{10} x_6^{10} x_8^9 x_9^{10} x_{10}^{10} x_{11}^{10} x_{12}^{10}}$                                                                 | $-1 \cdot 2^2 \cdot 3 \cdot 17$<br>$-1 \cdot 2^3 \cdot 3 \cdot 19$                                            |
| (10, 2)   | (0, 0, 0, 0, 0, 1, 0, 0, 0, 0, 0, 1) | 71  | $\frac{x_1^2 x_2^5 x_3^9 x_4^9 x_5^9 x_6^8 x_8^9 x_9^9 x_{10}^9 x_{11}^9}{x_1^3 x_2^4 x_3^9 x_4^9 x_5^9 x_6^8 x_8^9 x_9^9 x_{10}^9 x_{11}^9}$                                                                                                       | $-1 \cdot 2^4 \cdot 3 \cdot 293$<br>$-1 \cdot 2^{11} \cdot 11$                                                |
| (9, 3)    | (0, 0, 0, 0, 0, 1, 0, 0, 0, 0, 1, 1) | 66  | $\frac{x_2^4 x_3^8 x_4^8 x_5^8 x_6^2 x_7^8 x_8^8 x_9^8 x_{10}^2 x_{11}^2 x_{12}^2}{x_1 x_2^3 x_3^8 x_4^8 x_5^8 x_6^2 x_7^8 x_8^8 x_9^8 x_{10}^2 x_{11}^2 x_{12}^2}$                                                                                 | $-1 \cdot 2^4 \cdot 3 \cdot 293$<br>$-1 \cdot 2^5 \cdot 3^3 \cdot 43$                                         |
| (8, 4)    | (0, 0, 0, 0, 1, 0, 0, 0, 0, 1, 1, 1) | 61  | $\frac{x_1^3 x_2^7 x_3^7 x_4^3 x_5^7 x_6^7 x_7^7 x_8^3 x_9^3 x_{11}^3 x_{12}^3}{x_1^4 x_2^6 x_3^7 x_4^3 x_5^7 x_6^7 x_7^7 x_8^3 x_9^3 x_{11}^3 x_{12}^3}$                                                                                           | $-1 \cdot 2^4 \cdot 3 \cdot 293$<br>$-1 \cdot 2^2 \cdot 11 \cdot 691$                                         |
| (7, 5)    | (0, 0, 0, 0, 1, 0, 0, 0, 1, 1, 1, 1) | 60  | $\frac{x_1^4 x_2^6 x_3^6 x_4^6 x_5^4 x_6^6 x_7^6 x_8^4 x_9^4 x_{10}^4 x_{11}^4 x_{12}^4}{x_1^5 x_2^5 x_3^6 x_4^6 x_5^4 x_6^6 x_7^6 x_8^4 x_9^4 x_{10}^4 x_{11}^4 x_{12}^4}$                                                                         | $-1 \cdot 2 \cdot 34613$<br>$-1 \cdot 2^5 \cdot 3 \cdot 547$                                                  |
| (6, 6)    | (0, 0, 0, 1, 0, 0, 0, 1, 1, 1, 1, 1) | 59  | $\frac{x_1^4 x_2^5 x_3^5 x_4^5 x_5^5 x_6^5 x_7^5 x_8^5 x_9^5 x_{10}^5 x_{11}^5 x_{12}^5}{x_1^5 x_2^4 x_3^5 x_4^5 x_5^5 x_6^5 x_7^5 x_8^5 x_9^5 x_{10}^5 x_{11}^5 x_{12}^5}$                                                                         | $-1 \cdot 2^2 \cdot 7 \cdot 11^2$<br>$2^4 \cdot 31 \cdot 491$                                                 |
| (5, 7)    | (0, 0, 0, 1, 0, 0, 1, 1, 1, 1, 1, 1) | 62  | $x_1^4 x_2^4 x_3^4 x_4^6 x_5^4 x_6^6 x_7^6 x_8^6 x_9^6 x_{10}^6 x_{11}^6 x_{12}^6$                                                                                                                                                                  | $-1 \cdot 2 \cdot 3 \cdot 255259$                                                                             |
|           | (1, 1, 1, 1, 0, 0, 1, 1, 1, 0, 0, 0) | 62  | $x_1^6 x_2^6 x_3^6 x_4^4 x_5^4 x_6^6 x_7^6 x_8^4 x_9^4 x_{10}^4 x_{11}^4 x_{12}^4$                                                                                                                                                                  | $2^2 \cdot 7 \cdot 53 \cdot 11443$                                                                            |

$$S \subseteq \mathbb{Z}_p \times \mathbb{Z}_2 \setminus \{(0, 0)\}, |S| = 12$$

| $\lambda$ | $\mathbf{a}$                         | deg | monomial/s                                                                                                                                                                                                                        | coefficient/s                                                                        |
|-----------|--------------------------------------|-----|-----------------------------------------------------------------------------------------------------------------------------------------------------------------------------------------------------------------------------------|--------------------------------------------------------------------------------------|
| (4, 8)    | (0, 0, 1, 0, 0, 1, 1, 1, 1, 1, 1, 1) | 65  | $\frac{x_1^2 x_2^3 x_3^5 x_4^3 x_5^3 x_6^7 x_7^7 x_8^7 x_9^7 x_{10}^7 x_{11}^7 x_{12}^7}{x_1^3 x_2^3 x_3^4 x_4^3 x_5^3 x_6^7 x_7^7 x_8^7 x_9^7 x_{10}^7 x_{11}^7 x_{12}^7}$                                                       | $2^8 \cdot 3203$<br>$-1 \cdot 2^5 \cdot 31 \cdot 293$                                |
| (3, 9)    | (0, 0, 1, 0, 1, 1, 1, 1, 1, 1, 1, 1) | 72  | $\frac{x_2^2 x_3^4 x_4^2 x_5^8 x_6^8 x_7^8 x_8^8 x_9^8 x_{10}^8 x_{11}^8 x_{12}^8}{x_2^2 x_3^5 x_4^2 x_5^7 x_6^8 x_7^8 x_8^8 x_9^8 x_{10}^8 x_{11}^8 x_{12}^8}$                                                                   | $2 \cdot 7 \cdot 17 \cdot 29 \cdot 179$<br>$2^3 \cdot 23 \cdot 7177$                 |
| (2, 10)   | (0, 1, 0, 1, 1, 1, 1, 1, 1, 1, 1, 1) | 79  | $\frac{x_1 x_2^5 x_3 x_4^8 x_5^9 x_6^9 x_7^9 x_8^9 x_9^9 x_{10}^9 x_{11}^9 x_{12}^9}{x_1 x_2^5 x_3 x_4^9 x_5^9 x_6^9 x_7^9 x_8^9 x_9^9 x_{10}^9 x_{11}^9 x_{12}^9}$                                                               | $-1 \cdot 197 \cdot 78623$<br>$5 \cdot 61 \cdot 18223$                               |
| (1, 11)   | (0, 1, 1, 1, 1, 1, 1, 1, 1, 1, 1, 1) | 90  | $\frac{x_1^5 x_2^6 x_3^9 x_4^{10} x_5^{10} x_6^{10} x_7^{10} x_8^{10} x_9^{10} x_{10}^{10} x_{11}^{10} x_{12}^{10}}{x_2^4 x_3^7 x_4^9 x_5^{10} x_6^{10} x_7^{10} x_8^{10} x_9^{10} x_{10}^{10} x_{11}^{10} x_{12}^{10}}$          | $-1 \cdot 2^3 \cdot 3^2 \cdot 281627$<br>$-1 \cdot 2^2 \cdot 7 \cdot 13 \cdot 73583$ |
| (0, 12)   | (1, 1, 1, 1, 1, 1, 1, 1, 1, 1, 1, 1) | 101 | $\frac{x_1^3 x_2^4 x_3^6 x_4^{11} x_5^{11} x_6^{11} x_7^{11} x_8^{11} x_9^{11} x_{10}^{11} x_{11}^{11} x_{12}^{11}}{x_1^3 x_2^4 x_3^7 x_4^{10} x_5^{11} x_6^{11} x_7^{11} x_8^{11} x_9^{11} x_{10}^{11} x_{11}^{11} x_{12}^{11}}$ | $30062393$<br>$3^2 \cdot 431 \cdot 11489$                                            |

$$S \subseteq \mathbb{Z}_p \times \mathbb{Z}_3 \setminus \{(0, 0)\}, |S| = 12$$

| $\lambda$  | $\mathbf{a}$                         | deg | monomial/s                                                                                                                                                                                                                                          | coefficient/s                                                                                                 |
|------------|--------------------------------------|-----|-----------------------------------------------------------------------------------------------------------------------------------------------------------------------------------------------------------------------------------------------------|---------------------------------------------------------------------------------------------------------------|
| (12, 0, 0) | (0, 0, 0, 0, 0, 0, 0, 0, 0, 0, 0, 0) | 131 | $\frac{x_1^{10} x_2^{11} x_3^{11} x_4^{11} x_5^{11} x_6^{11} x_7^{11} x_8^{11} x_9^{11} x_{10}^{11} x_{11}^{11} x_{12}^{11}}{x_1^{11} x_2^{10} x_3^{11} x_4^{11} x_5^{11} x_6^{11} x_7^{11} x_8^{11} x_9^{11} x_{10}^{11} x_{11}^{11} x_{12}^{11}}$ | $2^4 \cdot 3 \cdot 29 \cdot 12953077208391719881$<br>$2^3 \cdot 3 \cdot 277 \cdot 1901 \cdot 786640832519761$ |
| (11, 1, 0) | (0, 0, 0, 0, 0, 0, 1, 0, 0, 0, 0, 0) | 80  | $\frac{x_1 x_2^3 x_3^6 x_4^{10} x_5^{10} x_6^{10} x_7^{10} x_8^{10} x_9^{10} x_{10}^{10} x_{11}^{10} x_{12}^{10}}{x_1 x_2^4 x_3^3 x_4^{10} x_5^{10} x_6^{10} x_7^{10} x_8^{10} x_9^{10} x_{10}^{10} x_{11}^{10} x_{12}^{10}}$                       | $-1 \cdot 5^2 \cdot 349$<br>$-1 \cdot 2 \cdot 3 \cdot 5 \cdot 467$                                            |
| (10, 2, 0) | (0, 0, 0, 0, 1, 0, 0, 0, 1, 0, 0, 0) | 58  | $x_1 x_2^3 x_3^5 x_4^7 x_5^6 x_6^9 x_7^8 x_8^9 x_9^8 x_{10}^9 x_{11}^9 x_{12}^9$                                                                                                                                                                    | -1                                                                                                            |
| (10, 1, 1) | (0, 0, 0, 0, 0, 1, 0, 0, 0, 0, 0, 2) | 70  | $x_1^8 x_2^9 x_3^9 x_4^9 x_5^9 x_6^8 x_7^9 x_8^9 x_9 x_{10} x_{11}$                                                                                                                                                                                 | $2 \cdot 3^2 \cdot 7$                                                                                         |
| (9, 3, 0)  | (0, 0, 0, 1, 0, 0, 0, 1, 0, 0, 0, 1) | 51  | $x_1^2 x_2^4 x_3^6 x_4 x_5^5 x_6^8 x_7^8 x_8^7 x_9^8 x_{10}^8 x_{11}^8$                                                                                                                                                                             | -1                                                                                                            |
| (9, 2, 1)  | (0, 0, 0, 0, 1, 0, 0, 1, 0, 0, 0, 2) | 50  | $x_1 x_2^3 x_3^5 x_4^8 x_5^8 x_6^8 x_7^8 x_8^7 x_9^8 x_{10}^8 x_{11}^8$                                                                                                                                                                             | -2                                                                                                            |
| (8, 4, 0)  | (0, 0, 0, 1, 0, 0, 1, 0, 0, 0, 1, 1) | 48  | $x_1 x_2^3 x_3^6 x_4^3 x_5^7 x_6^2 x_7^6 x_8^7 x_9^7 x_{10}^3 x_{11}^3 x_{12}^3$                                                                                                                                                                    | 2                                                                                                             |
| (8, 3, 1)  | (0, 0, 0, 0, 1, 0, 0, 1, 0, 0, 2, 1) | 45  | $x_1 x_2^3 x_3^7 x_4^7 x_5^2 x_6^7 x_7^8 x_8^7 x_9^7 x_{10}^2 x_{11}^2$                                                                                                                                                                             | $-1 \cdot 3$                                                                                                  |
| (8, 2, 2)  | (0, 0, 0, 1, 0, 0, 1, 0, 0, 0, 2, 2) | 43  | $x_1^2 x_2^4 x_3^7 x_4 x_5^7 x_6^6 x_7^8 x_8^7 x_9^7 x_{10} x_{11}$                                                                                                                                                                                 | $-1 \cdot 2^2$                                                                                                |
| (7, 5, 0)  | (0, 0, 0, 1, 0, 0, 1, 0, 0, 1, 1, 1) | 46  | $x_1 x_2^3 x_3^5 x_4^3 x_5^6 x_6^4 x_7^6 x_8^6 x_9^4 x_{10}^4 x_{11}^4 x_{12}^4$                                                                                                                                                                    | $-1 \cdot 2 \cdot 3$                                                                                          |
| (7, 4, 1)  | (0, 0, 0, 1, 0, 0, 1, 0, 0, 2, 1, 1) | 41  | $x_1^2 x_2^4 x_3^6 x_4^2 x_5^6 x_6^3 x_7^6 x_8^6 x_9^3 x_{10}^3 x_{11}^3$                                                                                                                                                                           | -1                                                                                                            |
| (7, 3, 2)  | (0, 0, 0, 0, 1, 0, 1, 0, 0, 2, 1, 2) | 40  | $x_1 x_2^2 x_3^6 x_4^6 x_5^6 x_6^2 x_7^6 x_8^6 x_9^6 x_{10} x_{11}^2$                                                                                                                                                                               | $2^2 \cdot 5^2$                                                                                               |
| (6, 6, 0)  | (0, 0, 1, 0, 0, 1, 0, 0, 1, 1, 1, 1) | 45  | $x_1 x_2^3 x_3 x_4^5 x_5^5 x_6^5 x_7^5 x_8^5 x_9^5 x_{10}^5 x_{11}^5$                                                                                                                                                                               | $2^2$                                                                                                         |
| (6, 5, 1)  | (0, 0, 0, 1, 0, 1, 0, 0, 1, 1, 1, 2) | 41  | $x_2^2 x_3^4 x_4^4 x_5^5 x_6^4 x_7^5 x_8^4 x_9^4 x_{10}^4 x_{11}^4$                                                                                                                                                                                 | $2 \cdot 3^2$                                                                                                 |
| (6, 4, 2)  | (0, 0, 0, 0, 1, 0, 1, 0, 2, 1, 2, 1) | 38  | $x_1^5 x_2^5 x_3^5 x_4^4 x_5^3 x_6^4 x_7^2 x_8^4 x_9^2 x_{10} x_{11} x_{12}^2$                                                                                                                                                                      | 1                                                                                                             |

$$S \subseteq \mathbb{Z}_p \times \mathbb{Z}_3 \setminus \{(0, 0)\}, |S| = 12$$

| $\lambda$  | $\mathbf{a}$                                                                 | deg      | monomial/s                                                                                                                                                               | coefficient/s                                                      |
|------------|------------------------------------------------------------------------------|----------|--------------------------------------------------------------------------------------------------------------------------------------------------------------------------|--------------------------------------------------------------------|
| (6, 3, 3)  | (0, 0, 0, 1, 0, 1, 0, 0, 2, 1, 2, 2)                                         | 36       | $x_1 x_2^3 x_3^5 x_4^2 x_5^5 x_6^2 x_7^5 x_8^5 x_9^2 x_{10}^2 x_{11}^2 x_{12}^2$                                                                                         | $-1 \cdot 2^2 \cdot 3$                                             |
| (5, 7, 0)  | (0, 0, 1, 0, 1, 0, 0, 1, 1, 1, 1, 1)                                         | 48       | $x_1 x_2^2 x_3^3 x_4^4 x_5^6 x_6^4 x_7^4 x_8^6 x_9^6 x_{10}^6 x_{11}^6 x_{12}^6$                                                                                         | $-1 \cdot 2 \cdot 3^3$                                             |
| (5, 6, 1)  | (0, 0, 0, 1, 0, 1, 0, 1, 1, 1, 2, 1)                                         | 42       | $x_1^4 x_2^4 x_3^4 x_4^5 x_5^4 x_6^5 x_7^4 x_8^4 x_9^4 x_{10}^3 x_{11} x_{12}$                                                                                           | $-1 \cdot 2^4$                                                     |
| (5, 5, 2)  | (0, 0, 0, 1, 0, 1, 0, 2, 1, 2, 1, 1)                                         | 37       | $x_1^3 x_2^3 x_3^4 x_4^2 x_5^4 x_6^4 x_7^4 x_8^4 x_9^4 x_{11}^4 x_{12}^4$                                                                                                | $-1 \cdot 2$                                                       |
| (5, 4, 3)  | (0, 0, 0, 0, 1, 1, 0, 2, 1, 2, 1, 2)                                         | 36       | $x_1^2 x_2^4 x_3^4 x_4^4 x_5^3 x_6^3 x_7^4 x_8^2 x_9^3 x_{10}^2 x_{11}^3 x_{12}^2$<br>$x_1^4 x_2^4 x_3^4 x_4^3 x_5^3 x_6^3 x_7^4 x_8^2 x_9^3 x_{10}^2 x_{11}^3 x_{12}^2$ | $2^2 \cdot 13$<br>$2 \cdot 7$                                      |
| (4, 8, 0)  | (0, 0, 1, 0, 1, 0, 1, 1, 1, 1, 1, 1)                                         | 52       | $x_1^3 x_2^3 x_3^7 x_4^3 x_5^6 x_6^3 x_7^7 x_8^7 x_9^7 x_{10}^5 x_{11} x_{12}$                                                                                           | $-1 \cdot 2^2 \cdot 7$                                             |
| (4, 7, 1)  | (0, 0, 1, 0, 1, 0, 1, 1, 1, 2, 1, 1)                                         | 44       | $x_1 x_2^3 x_3 x_4^3 x_5^4 x_6^3 x_7^5 x_8^6 x_9^6 x_{11}^6 x_{12}^6$                                                                                                    | $-1 \cdot 2^2 \cdot 3$                                             |
| (4, 6, 2)  | (0, 0, 0, 1, 1, 0, 1, 1, 1, 2, 1, 2)                                         | 40       | $x_2^3 x_3^3 x_4^4 x_5^5 x_6^3 x_7^5 x_8^5 x_9^5 x_{10}^5 x_{11} x_{12}$                                                                                                 | $2^4 \cdot 3^2$                                                    |
| (4, 5, 3)  | (0, 0, 2, 0, 1, 1, 0, 1, 2, 1, 2, 1)                                         | 37       | $x_1^3 x_2^3 x_3^2 x_4^3 x_5^4 x_6^3 x_7^3 x_8^4 x_9^2 x_{10}^4 x_{11}^2 x_{12}^4$<br>$x_1^3 x_2^2 x_3^3 x_4^3 x_5^4 x_6^3 x_7^3 x_8^4 x_9^2 x_{10}^4 x_{11}^2 x_{12}^4$ | $2^2 \cdot 11$<br>$-1 \cdot 3833$                                  |
| (4, 4, 4)  | (0, 0, 0, 1, 1, 0, 2, 1, 2, 1, 2, 2)                                         | 35       | $x_1^3 x_2^3 x_3^3 x_4^2 x_5^3 x_6^3 x_7^3 x_8^3 x_9^3 x_{10}^3 x_{11}^3 x_{12}^3$                                                                                       | $-1 \cdot 2^4$                                                     |
| (3, 9, 0)  | (0, 1, 0, 1, 0, 1, 1, 1, 1, 1, 1, 1)                                         | 57       | $x_1 x_2 x_3 x_4^4 x_5^2 x_6^8 x_8^8 x_9^8 x_{10}^8 x_{11}^8 x_{12}^8$                                                                                                   | $-1 \cdot 2^4 \cdot 3^3$                                           |
| (3, 8, 1)  | (0, 0, 1, 1, 0, 1, 1, 1, 1, 1, 1, 2)                                         | 50       | $x_2^2 x_3 x_4^3 x_5^2 x_6^7 x_7^7 x_8^7 x_9^7 x_{10}^7 x_{11}^7$                                                                                                        | $-1 \cdot 2^2 \cdot 3 \cdot 5$                                     |
| (3, 7, 2)  | (0, 0, 1, 0, 1, 1, 1, 1, 2, 1, 2, 1)                                         | 44       | $x_2^2 x_3^2 x_4^2 x_5^6 x_6^6 x_7^6 x_8^6 x_9^6 x_{10}^6 x_{11}^6 x_{12}^6$<br>$x_1 x_2^2 x_3 x_4^2 x_5^6 x_6^6 x_7^6 x_8^6 x_9^6 x_{10}^6 x_{11}^6 x_{12}^6$           | $3 \cdot 31$<br>$-1 \cdot 3 \cdot 173$                             |
| (3, 6, 3)  | (0, 0, 1, 0, 1, 2, 1, 2, 1, 2, 1, 1)                                         | 39       | $x_1^2 x_2^3 x_3^3 x_4^2 x_5^4 x_6^2 x_7^5 x_8^2 x_9^5 x_{10}^2 x_{11}^5 x_{12}^5$<br>$x_1^2 x_2^2 x_3^4 x_4^2 x_5^3 x_6^5 x_7^2 x_8^5 x_9^2 x_{10}^5 x_{11}^5 x_{12}^5$ | $3 \cdot 5 \cdot 11$<br>$3 \cdot 47$                               |
| (3, 5, 4)  | (0, 0, 1, 0, 1, 1, 2, 2, 1, 2, 1, 2)<br>(0, 0, 1, 2, 1, 1, 0, 2, 1, 2, 1, 2) | 38<br>38 | $x_1^2 x_2^2 x_3^4 x_4^2 x_5^4 x_6^4 x_7^3 x_8^4 x_9^3 x_{10}^4 x_{11}^3 x_{12}^3$<br>$x_1^2 x_2^2 x_3^4 x_4^3 x_5^4 x_6^4 x_7^3 x_8^4 x_9^3 x_{10}^4 x_{11}^3 x_{12}^3$ | $-1 \cdot 2^2 \cdot 3 \cdot 5 \cdot 17$<br>$-1 \cdot 2 \cdot 3329$ |
| (2, 10, 0) | (0, 1, 1, 0, 1, 1, 1, 1, 1, 1, 1, 1)                                         | 66       | $x_2^2 x_3^2 x_4 x_5^7 x_6^9 x_8^9 x_9^9 x_{10}^9 x_{11}^9 x_{12}^9$<br>$x_2^2 x_3^3 x_4 x_5^6 x_6^9 x_8^9 x_9^9 x_{10}^9 x_{11}^9 x_{12}^9$                             | $2^4 \cdot 17$<br>401                                              |
| (2, 9, 1)  | (0, 1, 0, 1, 1, 1, 1, 1, 1, 1, 2, 1)                                         | 57       | $x_2 x_3 x_4^7 x_5^8 x_6^8 x_8^8 x_9^8 x_{10}^8 x_{12}^8$                                                                                                                | $-1 \cdot 3^2 \cdot 7$                                             |
| (2, 8, 2)  | (2, 0, 1, 1, 1, 1, 1, 0, 1, 2, 1, 1)                                         | 49       | $x_3^2 x_4^3 x_5^7 x_6^7 x_7^7 x_8^7 x_9^7 x_{10}^7 x_{11}^7 x_{12}^7$<br>$x_3^2 x_4^4 x_5^6 x_6^7 x_7^7 x_8^7 x_9^7 x_{10}^7 x_{11}^7 x_{12}^7$                         | $2 \cdot 3 \cdot 11$<br>47                                         |
| (2, 7, 3)  | (0, 1, 0, 1, 1, 1, 1, 1, 2, 2, 1, 2)                                         | 45       | $x_2^2 x_3 x_4^6 x_5^6 x_6^6 x_7^6 x_8^2 x_9^2 x_{10}^6 x_{11}^2 x_{12}^2$<br>$x_3^3 x_3 x_4^5 x_5^6 x_6^6 x_7^6 x_8^2 x_9^2 x_{10}^6 x_{11}^2 x_{12}^2$                 | $3^2 \cdot 11$<br>$2^2 \cdot 53$                                   |
| (2, 6, 4)  | (0, 1, 0, 1, 1, 1, 1, 2, 1, 2, 2, 2)                                         | 42       | $x_2^4 x_3 x_4^5 x_5^5 x_6^5 x_7^3 x_8^5 x_9^3 x_{10}^3 x_{11}^3 x_{12}^3$                                                                                               | $-1 \cdot 5$                                                       |
| (2, 5, 5)  | (0, 1, 0, 1, 1, 2, 2, 1, 2, 1, 2, 2)                                         | 40       | $x_1 x_2^2 x_3 x_4^4 x_5^4 x_6^4 x_7^4 x_8^4 x_9^4 x_{10}^4 x_{11}^4 x_{12}^4$<br>$x_1 x_2^3 x_3 x_4^3 x_5^4 x_6^4 x_7^4 x_8^4 x_9^4 x_{10}^4 x_{11}^4 x_{12}^4$         | $2^3 \cdot 3 \cdot 53$<br>$2^2 \cdot 229$                          |

$$S \subseteq \mathbb{Z}_p \times \mathbb{Z}_3 \setminus \{(0, 0)\}, |S| = 12$$

| $\lambda$  | $\mathbf{a}$                         | deg | monomial/s                                                                                                                                                                                                     | coefficient/s                                                                           |
|------------|--------------------------------------|-----|----------------------------------------------------------------------------------------------------------------------------------------------------------------------------------------------------------------|-----------------------------------------------------------------------------------------|
| (1, 11, 0) | (0, 1, 1, 1, 1, 1, 1, 1, 1, 1, 1, 1) | 76  | $x_2^2 x_3^4 x_4^5 x_5^5 x_6^{10} x_7^{10} x_8^{10} x_9^{10} x_{10}^{10} x_{11}^{10} x_{12}^{10}$                                                                                                              | $-1 \cdot 2^2 \cdot 3^5$                                                                |
| (1, 10, 1) | (1, 0, 1, 1, 1, 1, 1, 1, 1, 2, 1, 1) | 65  | $x_1 x_2^2 x_3^8 x_4^9 x_5^9 x_6^9 x_7^9 x_8^9 x_9^9 x_{11}^9 x_{12}^9$<br>$x_1 x_3^3 x_4^7 x_5^9 x_6^9 x_7^9 x_8^9 x_9^9 x_{11}^9 x_{12}^9$                                                                   | $-1 \cdot 2^3 \cdot 17$<br>$-1 \cdot 503$                                               |
| (1, 9, 2)  | (0, 1, 1, 2, 2, 1, 1, 1, 1, 1, 1, 1) | 59  | $x_2^3 x_3^4 x_4 x_5 x_6^5 x_7^5 x_8^8 x_9^8 x_{10}^8 x_{11}^8 x_{12}^8$<br>$x_2^4 x_3^3 x_4 x_5 x_6^5 x_7^5 x_8^8 x_9^8 x_{10}^8 x_{11}^8 x_{12}^8$                                                           | $2 \cdot 443$<br>$-1 \cdot 2 \cdot 3 \cdot 109$                                         |
| (1, 8, 3)  | (0, 1, 1, 2, 2, 1, 1, 2, 1, 1, 1, 1) | 52  | $x_2^4 x_3^4 x_4^2 x_5^2 x_6^5 x_7^5 x_8^2 x_9^7 x_{10}^7 x_{11}^7 x_{12}^7$<br>$x_2^3 x_3^5 x_4^2 x_5^2 x_6^5 x_7^5 x_8^2 x_9^7 x_{10}^7 x_{11}^7 x_{12}^7$                                                   | $-1 \cdot 2^2 \cdot 3^2 \cdot 5 \cdot 11$<br>$3 \cdot 1823$                             |
| (1, 7, 4)  | (2, 1, 1, 1, 1, 1, 1, 0, 1, 2, 2, 2) | 48  | $x_1^2 x_2^5 x_3^4 x_4^5 x_5^5 x_6^6 x_7^6 x_8^3 x_9^3 x_{10}^3 x_{11}^3 x_{12}^3$                                                                                                                             | $3 \cdot 5^2$                                                                           |
| (1, 6, 5)  | (0, 1, 1, 2, 2, 1, 1, 2, 2, 1, 1, 2) | 48  | $x_2^3 x_3^5 x_4^4 x_5^4 x_6^5 x_7^4 x_8^4 x_9^5 x_{10}^5 x_{11}^4 x_{12}^4$<br>$x_2^4 x_3^4 x_4^4 x_5^4 x_6^5 x_7^4 x_8^4 x_9^5 x_{10}^5 x_{11}^4 x_{12}^4$                                                   | $-1 \cdot 3 \cdot 7 \cdot 89 \cdot 359$<br>$-332317$                                    |
| (0, 12, 0) | (1, 1, 1, 1, 1, 1, 1, 1, 1, 1, 1, 1) | 87  | $x_1 x_2^3 x_3^4 x_4^5 x_5^8 x_6^{11} x_7^{11} x_8^{11} x_9^{11} x_{10}^{11} x_{11}^{11} x_{12}^{11}$<br>$x_1 x_2^3 x_3^4 x_4^6 x_5^7 x_6^{11} x_7^{11} x_8^{11} x_9^{11} x_{10}^{11} x_{11}^{11} x_{12}^{11}$ | $2^2 \cdot 3 \cdot 43$<br>$3^3 \cdot 31$                                                |
| (0, 11, 1) | (1, 1, 1, 1, 1, 1, 1, 1, 1, 1, 1, 2) | 77  | $x_1^2 x_2^5 x_3^5 x_4^5 x_5^{10} x_6^{10} x_8^{10} x_9^{10} x_{10}^{10} x_{11}^{10}$                                                                                                                          | $-1 \cdot 2^3 \cdot 3$                                                                  |
| (0, 10, 2) | (1, 1, 1, 1, 1, 1, 1, 1, 1, 1, 2, 2) | 68  | $x_1^3 x_2^6 x_3^6 x_4^6 x_5^9 x_6^9 x_7^9 x_8^9 x_9^9 x_{10}^{11} x_{11}^{12}$<br>$x_1^4 x_2^5 x_3^6 x_4^6 x_5^9 x_6^9 x_7^9 x_8^9 x_9^9 x_{10}^{11} x_{11}^{12}$                                             | $109$<br>$97$                                                                           |
| (0, 9, 3)  | (1, 1, 2, 2, 1, 1, 2, 1, 1, 1, 1, 1) | 60  | $x_1^2 x_2^5 x_3^2 x_4^2 x_5^7 x_6^8 x_7^8 x_8^8 x_9^8 x_{10}^8 x_{11}^8 x_{12}^8$<br>$x_1^3 x_2^4 x_3^2 x_4^2 x_5^7 x_6^8 x_7^8 x_8^8 x_9^8 x_{10}^8 x_{11}^8 x_{12}^8$                                       | $2 \cdot 11 \cdot 13$<br>$-1 \cdot 1487$                                                |
| (0, 8, 4)  | (1, 1, 2, 2, 1, 1, 2, 2, 1, 1, 1, 1) | 58  | $x_1^5 x_2^6 x_3^3 x_4^3 x_5^7 x_6^3 x_7^3 x_8^7 x_9^7 x_{10}^7 x_{11}^7 x_{12}^7$<br>$x_1^6 x_2^5 x_3^3 x_4^3 x_5^7 x_6^3 x_7^3 x_8^7 x_9^7 x_{10}^7 x_{11}^7 x_{12}^7$                                       | $-1 \cdot 3^2 \cdot 751$<br>$5167$                                                      |
| (0, 7, 5)  | (1, 1, 2, 2, 1, 1, 2, 2, 1, 1, 2, 1) | 55  | $x_1^5 x_2^6 x_3^4 x_4^4 x_5^6 x_7^4 x_8^6 x_9^6 x_{10}^4 x_{11}^6 x_{12}^6$<br>$x_1^6 x_2^5 x_3^4 x_4^4 x_5^6 x_7^4 x_8^6 x_9^6 x_{10}^4 x_{11}^6 x_{12}^6$                                                   | $-1 \cdot 2 \cdot 3^5 \cdot 11 \cdot 43$<br>$-1 \cdot 3 \cdot 30047$                    |
| (0, 6, 6)  | (1, 1, 2, 2, 1, 1, 2, 2, 1, 1, 2, 2) | 53  | $x_2^3 x_3^5 x_4^5 x_5^5 x_6^5 x_7^5 x_8^5 x_9^5 x_{10}^5 x_{11}^5 x_{12}^5$<br>$x_1 x_2^2 x_3^5 x_4^5 x_5^5 x_6^5 x_7^5 x_8^5 x_9^5 x_{10}^5 x_{11}^5 x_{12}^5$                                               | $-1 \cdot 2^2 \cdot 3 \cdot 5 \cdot 3847$<br>$-1 \cdot 2^3 \cdot 3 \cdot 13^2 \cdot 47$ |

$$S \subseteq \mathbb{Z}_p \times \mathbb{Z}_4 \setminus \{(0, 0)\}, |S| = 12$$

| $\lambda$     | $\mathbf{a}$                         | deg | monomial/s                                                                                                                                                                                                                                       | coefficient/s                                                                                                 |
|---------------|--------------------------------------|-----|--------------------------------------------------------------------------------------------------------------------------------------------------------------------------------------------------------------------------------------------------|---------------------------------------------------------------------------------------------------------------|
| (12, 0, 0, 0) | (0, 0, 0, 0, 0, 0, 0, 0, 0, 0, 0, 0) | 131 | $x_1^{10} x_2^{11} x_3^{11} x_4^{11} x_5^{11} x_6^{11} x_7^{11} x_8^{11} x_9^{11} x_{10}^{11} x_{11}^{11} x_{12}^{11}$<br>$x_1^{11} x_2^{10} x_3^{11} x_4^{11} x_5^{11} x_6^{11} x_7^{11} x_8^{11} x_9^{11} x_{10}^{11} x_{11}^{11} x_{12}^{11}$ | $2^4 \cdot 3 \cdot 29 \cdot 12953077208391719881$<br>$2^3 \cdot 3 \cdot 277 \cdot 1901 \cdot 786640832519761$ |
| (11, 1, 0, 0) | (0, 0, 0, 0, 0, 0, 1, 0, 0, 0, 0, 0) | 80  | $x_1 x_2^3 x_3^7 x_4^{10} x_6^{10} x_8^9 x_9^{10} x_{10}^{10} x_{11}^{10} x_{12}^{10}$<br>$x_1 x_2^4 x_3^6 x_4^{10} x_6^{10} x_8^9 x_9^{10} x_{10}^{10} x_{11}^{10} x_{12}^{10}$                                                                 | $-1 \cdot 2^2 \cdot 3 \cdot 17$<br>$-1 \cdot 2^3 \cdot 19$                                                    |
| (11, 0, 1, 0) | (0, 0, 0, 0, 0, 0, 2, 0, 0, 0, 0, 0) | 80  | $x_1 x_2^3 x_3^7 x_4^{10} x_6^{10} x_8^9 x_9^{10} x_{10}^{10} x_{11}^{10} x_{12}^{10}$<br>$x_1 x_2^4 x_3^6 x_4^{10} x_6^{10} x_8^9 x_9^{10} x_{10}^{10} x_{11}^{10} x_{12}^{10}$                                                                 | $-1 \cdot 2^2 \cdot 3 \cdot 17$<br>$-1 \cdot 2^3 \cdot 19$                                                    |
| (10, 2, 0, 0) | (0, 0, 0, 0, 1, 0, 0, 0, 1, 0, 0, 0) | 58  | $x_1 x_2^3 x_3^5 x_4^7 x_6^6 x_8^9 x_9^8 x_{10}^9 x_{11}^9 x_{12}^9$                                                                                                                                                                             | $-1$                                                                                                          |

$$S \subseteq \mathbb{Z}_p \times \mathbb{Z}_4 \setminus \{(0, 0)\}, |S| = 12$$

| $\lambda$     | $\mathbf{a}$                         | deg | monomial/s                                                                                                                                                       | coefficient/s                                                         |
|---------------|--------------------------------------|-----|------------------------------------------------------------------------------------------------------------------------------------------------------------------|-----------------------------------------------------------------------|
| (10, 1, 0, 1) | (0, 0, 0, 0, 0, 1, 0, 0, 0, 0, 0, 3) | 70  | $x_1^3 x_2^4 x_3^9 x_4^9 x_5^9 x_8^9 x_9^9 x_{10}^9 x_{11}^9$<br>$x_1^3 x_2^5 x_3^8 x_4^9 x_5^9 x_8^9 x_9^9 x_{10}^9 x_{11}^9$                                   | $2^{11} \cdot 11$<br>$2^5 \cdot 5 \cdot 433$                          |
| (10, 1, 1, 0) | (0, 0, 0, 0, 1, 0, 0, 0, 2, 0, 0, 0) | 57  | $x_1 x_2^3 x_3^5 x_4^7 x_6^6 x_8^9 x_{10}^8 x_{11}^9 x_{12}^9$                                                                                                   | -1                                                                    |
| (10, 0, 2, 0) | (0, 0, 0, 0, 0, 2, 0, 0, 0, 0, 0, 2) | 71  | $x_1^2 x_2^5 x_3^9 x_4^9 x_5^9 x_6^9 x_8^9 x_9^9 x_{10}^9 x_{11}^9$<br>$x_1^3 x_2^4 x_3^9 x_4^9 x_5^9 x_8^9 x_9^9 x_{10}^9 x_{11}^9 x_{12}^9$                    | $-1 \cdot 2^4 \cdot 3 \cdot 293$<br>$2^{11} \cdot 11$                 |
| (9, 3, 0, 0)  | (0, 0, 0, 1, 0, 0, 1, 0, 0, 1, 0, 0) | 45  | $x_2^2 x_3^4 x_4 x_3^3 x_5^5 x_8^5 x_9^8 x_{10}^2 x_{11}^7 x_{12}^8$                                                                                             | 1                                                                     |
| (9, 2, 0, 1)  | (0, 0, 0, 0, 1, 0, 0, 1, 0, 0, 0, 3) | 50  | $x_1 x_2^3 x_3^5 x_4^8 x_5^8 x_6^8 x_8 x_7 x_{10}^8 x_{11}^8$                                                                                                    | $2^2$                                                                 |
| (9, 2, 1, 0)  | (0, 0, 0, 1, 0, 0, 0, 1, 0, 0, 0, 2) | 49  | $x_1^2 x_2^4 x_3^6 x_5^5 x_6^8 x_8 x_7 x_{10}^8 x_{11}^8$                                                                                                        | 2                                                                     |
| (9, 1, 1, 1)  | (0, 0, 0, 1, 0, 0, 2, 0, 0, 3, 0, 0) | 42  | $x_2^2 x_3^4 x_5^3 x_6^5 x_8^5 x_9^8 x_{11}^7 x_{12}^8$                                                                                                          | -1                                                                    |
| (9, 1, 2, 0)  | (0, 0, 0, 2, 0, 0, 1, 0, 0, 2, 0, 0) | 43  | $x_2^2 x_3^4 x_5^3 x_6^5 x_8^8 x_9 x_{10} x_{11}^7 x_{12}^8$                                                                                                     | -1                                                                    |
| (9, 0, 3, 0)  | (0, 0, 0, 0, 0, 2, 0, 0, 0, 0, 2, 2) | 66  | $x_2^4 x_3^8 x_4^8 x_5^8 x_6^8 x_7^8 x_8^8 x_9^8 x_{10}^2 x_{11}^2 x_{12}^2$<br>$x_1 x_2^3 x_3^8 x_4^8 x_5^2 x_6^2 x_7^2 x_8^8 x_9^8 x_{10}^2 x_{11}^2 x_{12}^2$ | $-1 \cdot 2^4 \cdot 3 \cdot 293$<br>$-1 \cdot 2^5 \cdot 3^3 \cdot 43$ |
| (8, 4, 0, 0)  | (0, 0, 1, 0, 0, 1, 0, 0, 1, 0, 0, 1) | 40  | $x_1^2 x_2^4 x_3^3 x_5^5 x_6 x_7 x_8^2 x_9^6 x_{10} x_{11}^7 x_{12}^3$                                                                                           | -1                                                                    |
| (8, 3, 0, 1)  | (0, 0, 0, 1, 0, 0, 1, 0, 1, 0, 0, 3) | 38  | $x_2^2 x_3^4 x_4 x_3^3 x_6^6 x_7 x_8^2 x_9^6 x_{10} x_{11}^7$                                                                                                    | 1                                                                     |
| (8, 2, 0, 2)  | (0, 0, 0, 1, 0, 0, 1, 0, 0, 0, 3, 3) | 43  | $x_1^2 x_2^4 x_3^7 x_4 x_7 x_5^6 x_7 x_8^7 x_9^7 x_{10} x_{11}$                                                                                                  | $-1 \cdot 2^2$                                                        |
| (8, 3, 1, 0)  | (0, 0, 0, 1, 0, 1, 0, 0, 1, 0, 0, 2) | 38  | $x_1 x_2^3 x_3^5 x_4 x_5^5 x_6 x_7 x_8^2 x_9^6 x_{10} x_{11}^7$                                                                                                  | -1                                                                    |
| (8, 2, 1, 1)  | (0, 0, 0, 1, 0, 0, 2, 0, 3, 0, 0, 1) | 36  | $x_2^2 x_3^4 x_5^3 x_6^6 x_7 x_8^6 x_{10} x_{11}^7 x_{12}$                                                                                                       | -1                                                                    |
| (8, 2, 2, 0)  | (0, 0, 0, 1, 0, 2, 0, 0, 2, 1, 0, 0) | 37  | $x_1 x_2^3 x_3^5 x_6^6 x_7 x_8^7 x_9 x_{10} x_{11}^6 x_{12}^7$                                                                                                   | 1                                                                     |
| (8, 1, 2, 1)  | (0, 0, 1, 0, 0, 2, 0, 0, 3, 0, 0, 2) | 35  | $x_1^2 x_2^4 x_3^3 x_5^5 x_7 x_8^6 x_{10} x_{11}^7 x_{12}$                                                                                                       | -1                                                                    |
| (8, 1, 3, 0)  | (0, 0, 0, 2, 0, 0, 1, 0, 2, 0, 0, 2) | 38  | $x_2^2 x_3^4 x_5^3 x_6^6 x_7 x_8^6 x_9 x_{10} x_{11}^7 x_{12}^2$                                                                                                 | -1                                                                    |
| (8, 0, 4, 0)  | (0, 0, 0, 0, 2, 0, 0, 0, 0, 2, 2, 2) | 61  | $x_1^3 x_2^7 x_3^7 x_4^3 x_5^7 x_6^7 x_7^7 x_8^7 x_9^7 x_{11}^3 x_{12}^3$<br>$x_1^4 x_2^6 x_3^7 x_4^3 x_5^3 x_6^7 x_7^7 x_8^7 x_9^7 x_{11}^3 x_{12}^3$           | $-1 \cdot 2^4 \cdot 3 \cdot 293$<br>$-1 \cdot 2^2 \cdot 11 \cdot 691$ |
| (7, 5, 0, 0)  | (0, 0, 1, 0, 1, 0, 0, 1, 0, 0, 1, 1) | 39  | $x_1 x_2^3 x_3 x_4^4 x_5^2 x_6^6 x_8^3 x_9^5 x_{10}^6 x_{11}^4 x_{12}^4$                                                                                         | -1                                                                    |
| (7, 4, 0, 1)  | (0, 0, 0, 1, 0, 0, 1, 0, 1, 0, 3, 1) | 35  | $x_2^2 x_3^4 x_5^3 x_6^6 x_7 x_8^6 x_9^3 x_{10}^6 x_{12}^3$                                                                                                      | 1                                                                     |
| (7, 3, 0, 2)  | (0, 0, 0, 1, 0, 1, 0, 1, 0, 0, 3, 3) | 33  | $x_2^2 x_3^4 x_4 x_5^4 x_6 x_7 x_8^2 x_9^5 x_{10}^6 x_{11} x_{12}$                                                                                               | 1                                                                     |
| (7, 4, 1, 0)  | (0, 0, 0, 1, 0, 1, 0, 1, 0, 0, 2, 1) | 35  | $x_2^2 x_3^4 x_5^3 x_6^6 x_7 x_8^3 x_9^5 x_{10}^6 x_{12}^3$                                                                                                      | -1                                                                    |
| (7, 3, 1, 1)  | (0, 0, 1, 0, 0, 1, 0, 1, 0, 0, 3, 2) | 31  | $x_1 x_2^3 x_4^2 x_5^4 x_6^2 x_7 x_8^2 x_9^5 x_{10}^6$                                                                                                           | -1                                                                    |
| (7, 2, 1, 2)  | (0, 0, 0, 1, 0, 0, 2, 0, 3, 0, 1, 3) | 31  | $x_2^2 x_3^4 x_5^4 x_6^6 x_8^6 x_9 x_{10}^6 x_{11} x_{12}$                                                                                                       | 2                                                                     |

$$S \subseteq \mathbb{Z}_p \times \mathbb{Z}_4 \setminus \{(0, 0)\}, |S| = 12$$

| $\lambda$    | $\mathbf{a}$                         | deg | monomial/s                                                                                                                                                               | coefficient/s                                                           |
|--------------|--------------------------------------|-----|--------------------------------------------------------------------------------------------------------------------------------------------------------------------------|-------------------------------------------------------------------------|
| (7, 3, 2, 0) | (0, 0, 0, 1, 0, 2, 0, 2, 1, 0, 0, 1) | 33  | $x_2^2 x_3^4 x_5^5 x_6^6 x_7^8 x_9 x_{10}^5 x_{11}^6 x_{12}^2$                                                                                                           | -1                                                                      |
| (7, 2, 2, 1) | (0, 0, 0, 1, 0, 2, 0, 3, 0, 0, 1, 2) | 31  | $x_2^2 x_3^4 x_4 x_5^5 x_7^6 x_9^5 x_{10}^6 x_{11} x_{12}$                                                                                                               | -1                                                                      |
| (7, 2, 3, 0) | (0, 0, 1, 0, 2, 0, 0, 2, 1, 0, 0, 2) | 32  | $x_1 x_2^3 x_4^2 x_6^4 x_7^6 x_8^2 x_9 x_{10}^5 x_{11}^6 x_{12}^2$                                                                                                       | $-1 \cdot 2^2$                                                          |
| (7, 1, 3, 1) | (0, 0, 0, 1, 0, 2, 0, 2, 2, 3, 0, 0) | 32  | $x_2^2 x_3^4 x_5^3 x_6^2 x_7^6 x_8^2 x_9^2 x_{11}^5 x_{12}^6$                                                                                                            | -1                                                                      |
| (7, 1, 4, 0) | (0, 0, 0, 2, 0, 0, 1, 0, 2, 0, 2, 2) | 35  | $x_2^2 x_3^4 x_5^3 x_6^5 x_8^3 x_9^6 x_{10}^3 x_{11}^3 x_{12}^3$                                                                                                         | -1                                                                      |
| (7, 0, 5, 0) | (0, 0, 0, 0, 2, 0, 0, 0, 2, 2, 2, 2) | 60  | $x_1^4 x_2^6 x_3^6 x_4^6 x_5^4 x_6^6 x_7^6 x_8^6 x_9^4 x_{10}^4 x_{11}^4 x_{12}^4$<br>$x_1^5 x_2^5 x_3^6 x_4^6 x_5^6 x_6^6 x_7^6 x_8^6 x_9^4 x_{10}^4 x_{11}^4 x_{12}^4$ | $-1 \cdot 2 \cdot 34613$<br>$-1 \cdot 2^5 \cdot 3 \cdot 547$            |
| (6, 6, 0, 0) | (0, 0, 1, 0, 1, 0, 1, 0, 0, 1, 1, 1) | 39  | $x_2^2 x_3 x_4^2 x_5^5 x_6^5 x_8^4 x_9^5 x_{10}^5 x_{11}^5 x_{12}^5$                                                                                                     | $-1 \cdot 2$                                                            |
| (6, 5, 0, 1) | (0, 0, 1, 0, 0, 1, 0, 1, 0, 3, 1, 1) | 33  | $x_1 x_2^3 x_4^2 x_5^5 x_6 x_7^4 x_8^4 x_9^5 x_{11}^4 x_{12}^4$                                                                                                          | 1                                                                       |
| (6, 4, 0, 2) | (0, 0, 0, 1, 0, 0, 1, 1, 0, 3, 1, 3) | 31  | $x_2^2 x_3^4 x_5^4 x_6^5 x_7^3 x_8^5 x_9 x_{10}^3 x_{11}^3 x_{12}$                                                                                                       | 3                                                                       |
| (6, 3, 0, 3) | (0, 0, 1, 0, 1, 0, 1, 0, 0, 3, 3, 3) | 29  | $x_1 x_2^3 x_4^2 x_5^5 x_6^2 x_7^4 x_8^5 x_9^2 x_{10}^2 x_{11}^2 x_{12}^2$                                                                                               | 1                                                                       |
| (6, 5, 1, 0) | (0, 0, 0, 1, 0, 1, 0, 1, 0, 2, 1, 1) | 34  | $x_2^2 x_3^4 x_5^3 x_6^5 x_7^4 x_8^5 x_9^4 x_{11}^4 x_{12}^4$                                                                                                            | $-1 \cdot 2^2$                                                          |
| (6, 4, 1, 1) | (0, 0, 0, 1, 0, 1, 0, 1, 0, 3, 1, 2) | 30  | $x_2^2 x_3^4 x_4 x_5^5 x_6^2 x_7^5 x_8^3 x_9^5 x_{11}^3$                                                                                                                 | 1                                                                       |
| (6, 3, 1, 2) | (0, 0, 0, 1, 0, 0, 2, 3, 0, 1, 3, 1) | 28  | $x_2^2 x_3^4 x_4^2 x_5^4 x_6^5 x_8 x_9^5 x_{10}^2 x_{11} x_{12}^2$                                                                                                       | 3                                                                       |
| (6, 4, 2, 0) | (0, 0, 1, 0, 1, 0, 1, 0, 0, 2, 1, 2) | 30  | $x_1 x_2^3 x_4^2 x_5^5 x_6^3 x_7^4 x_8^5 x_9 x_{10}^3 x_{11}^3 x_{12}$                                                                                                   | -1                                                                      |
| (6, 3, 2, 1) | (0, 0, 0, 1, 0, 2, 0, 2, 1, 0, 1, 3) | 28  | $x_2^2 x_3^4 x_4 x_5^5 x_6^5 x_7^8 x_9^2 x_{10}^5 x_{11}^2$                                                                                                              | $-1 \cdot 3$                                                            |
| (6, 2, 2, 2) | (0, 0, 1, 0, 0, 2, 0, 3, 0, 1, 3, 2) | 26  | $x_1 x_2^3 x_4^3 x_5^5 x_7^5 x_8 x_9^5 x_{10} x_{11} x_{12}$                                                                                                             | 2                                                                       |
| (6, 3, 3, 0) | (0, 0, 0, 1, 1, 0, 0, 1, 0, 2, 2, 2) | 30  | $x_2^2 x_3^4 x_4 x_5 x_6^4 x_7^5 x_8^2 x_9^5 x_{10}^2 x_{11}^2 x_{12}^2$                                                                                                 | -1                                                                      |
| (6, 2, 3, 1) | (0, 0, 0, 1, 0, 2, 2, 2, 3, 0, 0, 1) | 28  | $x_2^2 x_3^4 x_4 x_5^5 x_6^2 x_7^2 x_8^2 x_{10}^5 x_{11}^5 x_{12}$                                                                                                       | 3                                                                       |
| (6, 2, 4, 0) | (0, 0, 0, 1, 2, 0, 2, 2, 2, 1, 0, 0) | 31  | $x_2^3 x_3^5 x_6^4 x_7^3 x_8^3 x_9 x_{10}^4 x_{11}^5 x_{12}^5$                                                                                                           | $-1 \cdot 2^2$                                                          |
| (6, 1, 4, 1) | (0, 0, 1, 0, 2, 0, 2, 2, 3, 0, 0, 2) | 29  | $x_1 x_2^3 x_4^2 x_6^5 x_7^3 x_8^4 x_{10}^5 x_{11}^3 x_{12}^3$                                                                                                           | $-1 \cdot 3$                                                            |
| (6, 1, 5, 0) | (0, 0, 0, 2, 0, 0, 1, 2, 0, 2, 2, 2) | 34  | $x_2^2 x_3^4 x_4 x_5^5 x_6^5 x_8 x_9^5 x_{10}^4 x_{11}^4 x_{12}^4$                                                                                                       | $-1 \cdot 3$                                                            |
| (6, 0, 6, 0) | (0, 0, 0, 2, 0, 0, 0, 2, 2, 2, 2, 2) | 59  | $x_1^4 x_2^5 x_3^5 x_4^5 x_5^5 x_6^5 x_7^5 x_8^5 x_9^5 x_{10}^5 x_{11}^5 x_{12}^5$<br>$x_1^5 x_2^4 x_3^5 x_4^5 x_5^5 x_6^5 x_7^5 x_8^5 x_9^5 x_{10}^5 x_{11}^5 x_{12}^5$ | $-1 \cdot 2^2 \cdot 7 \cdot 11^2 \cdot 397$<br>$2^4 \cdot 31 \cdot 491$ |
| (5, 7, 0, 0) | (0, 0, 1, 0, 1, 0, 1, 0, 1, 1, 1, 1) | 41  | $x_2^2 x_3 x_4^2 x_5^4 x_6^4 x_8^6 x_9^6 x_{10}^6 x_{11}^6 x_{12}^6$                                                                                                     | 3                                                                       |
| (5, 6, 0, 1) | (0, 0, 1, 0, 1, 0, 1, 0, 3, 1, 1, 1) | 35  | $x_2^2 x_3 x_4 x_5 x_6^3 x_7^5 x_8^4 x_{10}^5 x_{11}^5 x_{12}^5$                                                                                                         | 1                                                                       |
| (5, 5, 0, 2) | (0, 0, 0, 1, 0, 0, 1, 1, 3, 1, 3, 1) | 31  | $x_2^3 x_3^4 x_5^3 x_6^4 x_7^3 x_8^4 x_9 x_{10}^4 x_{11} x_{12}^4$                                                                                                       | $-1 \cdot 2^2$                                                          |

$$S \subseteq \mathbb{Z}_p \times \mathbb{Z}_4 \setminus \{(0, 0)\}, |S| = 12$$

| $\lambda$    | $\mathbf{a}$                         | deg | monomial/s                                                                         | coefficient/s                      |
|--------------|--------------------------------------|-----|------------------------------------------------------------------------------------|------------------------------------|
| (5, 4, 0, 3) | (0, 0, 0, 1, 0, 1, 1, 0, 3, 1, 3, 3) | 29  | $x_2^2 x_3^4 x_4 x_5^4 x_6^2 x_7^3 x_8^4 x_9^2 x_{10}^3 x_{11}^2 x_{12}^2$         | 3                                  |
| (5, 6, 1, 0) | (0, 0, 1, 0, 1, 0, 1, 0, 2, 1, 1, 1) | 34  | $x_1 x_2^3 x_4^2 x_5 x_6^4 x_7^4 x_8^4 x_{10}^5 x_{11}^5 x_{12}^5$                 | $-1 \cdot 2$                       |
| (5, 5, 1, 1) | (0, 0, 0, 1, 0, 1, 1, 0, 2, 1, 1, 3) | 30  | $x_2^2 x_3^4 x_5^4 x_6^4 x_7^4 x_8^4 x_{10}^4 x_{11}^4$                            | $-1 \cdot 2^2$                     |
| (5, 4, 1, 2) | (0, 0, 1, 0, 0, 1, 1, 0, 3, 1, 3, 2) | 26  | $x_1 x_2^3 x_4^3 x_5^4 x_6^3 x_7^3 x_8^4 x_9 x_{10}^3 x_{11}$                      | 3                                  |
| (5, 3, 1, 3) | (0, 0, 0, 1, 0, 0, 2, 3, 1, 3, 1, 3) | 26  | $x_2^3 x_3^4 x_4^2 x_5^3 x_6^4 x_8^2 x_9^2 x_{10}^2 x_{11}^2 x_{12}^2$             | $-1 \cdot 2^2 \cdot 3$             |
| (5, 5, 2, 0) | (0, 0, 0, 1, 1, 0, 1, 0, 2, 1, 1, 2) | 31  | $x_2^2 x_3^4 x_4 x_5^2 x_6^4 x_7^4 x_8^4 x_9 x_{10}^4 x_{11}^4 x_{12}$             | $2^2$                              |
| (5, 4, 2, 1) | (0, 0, 0, 1, 0, 2, 3, 0, 1, 2, 1, 1) | 27  | $x_1^3 x_2^4 x_3^4 x_4^3 x_5^3 x_6^4 x_8^3 x_9^3 x_{10} x_{11}$                    | 1                                  |
| (5, 3, 2, 2) | (0, 0, 0, 1, 0, 2, 3, 0, 1, 3, 1, 2) | 25  | $x_2^4 x_3^4 x_4^2 x_5^4 x_7 x_8^4 x_9^2 x_{10} x_{11}^2 x_{12}$                   | $2^2 \cdot 3$                      |
| (5, 4, 3, 0) | (0, 0, 0, 1, 1, 0, 1, 0, 2, 2, 2, 1) | 29  | $x_2^2 x_3^4 x_4 x_5^2 x_6^4 x_7^3 x_8^4 x_9^2 x_{10}^2 x_{11}^3 x_{12}^3$         | 2                                  |
| (5, 3, 3, 1) | (0, 0, 1, 0, 1, 0, 1, 0, 2, 2, 3, 2) | 25  | $x_1 x_2^3 x_4^3 x_5^2 x_6^4 x_7^2 x_8^4 x_9^2 x_{10}^2 x_{12}^2$                  | $-1 \cdot 5$                       |
| (5, 2, 3, 2) | (0, 0, 0, 1, 0, 2, 2, 2, 3, 0, 1, 3) | 25  | $x_2^3 x_3^4 x_4 x_5^4 x_6^2 x_7^2 x_8^2 x_9 x_{10}^4 x_{11} x_{12}$               | $-1 \cdot 2^2$                     |
| (5, 3, 4, 0) | (0, 0, 0, 1, 2, 2, 1, 0, 0, 1, 2, 2) | 29  | $x_2^3 x_3^4 x_4 x_5^2 x_6^3 x_7 x_8^3 x_9^4 x_{10}^2 x_{11}^3 x_{12}^3$           | $2^2$                              |
| (5, 2, 4, 1) | (0, 0, 0, 1, 2, 2, 2, 3, 0, 0, 1, 2) | 27  | $x_2^4 x_3^4 x_4 x_5^2 x_6^2 x_7^3 x_9^3 x_{10}^4 x_{11} x_{12}^3$                 | $-1 \cdot 2^3$                     |
| (5, 2, 5, 0) | (0, 0, 1, 2, 0, 2, 2, 2, 1, 0, 0, 2) | 30  | $x_1 x_2^3 x_5^3 x_6^3 x_7^4 x_8^4 x_9 x_{10}^3 x_{11}^4 x_{12}^4$                 | -1                                 |
| (5, 1, 5, 1) | (0, 0, 0, 1, 2, 2, 2, 2, 2, 3, 0, 0) | 30  | $x_2^3 x_3^4 x_5 x_6^3 x_7^4 x_8^4 x_9^4 x_{11}^3 x_{12}^4$                        | $-1 \cdot 2$                       |
| (5, 1, 6, 0) | (0, 0, 0, 2, 0, 0, 1, 2, 2, 2, 2, 2) | 35  | $x_2^3 x_3^4 x_5^3 x_6^4 x_8^4 x_9^4 x_{10}^5 x_{11}^5 x_{12}^5$                   | $-1 \cdot 2$                       |
| (5, 0, 7, 0) | (0, 0, 0, 2, 0, 0, 2, 2, 2, 2, 2, 2) | 62  | $x_1^4 x_2^4 x_3^4 x_4^6 x_5^4 x_6^4 x_7^6 x_8^6 x_9^6 x_{10}^6 x_{11}^6 x_{12}^6$ | $-1 \cdot 2 \cdot 3 \cdot 255259$  |
|              | (2, 2, 2, 2, 0, 0, 2, 2, 2, 0, 0, 0) | 62  | $x_1^6 x_2^6 x_3^6 x_4^6 x_5^4 x_6^4 x_7^6 x_8^6 x_9^6 x_{10}^4 x_{11}^4 x_{12}^4$ | $2^2 \cdot 7 \cdot 53 \cdot 11443$ |
| (4, 8, 0, 0) | (0, 1, 0, 1, 0, 1, 0, 1, 1, 1, 1, 1) | 44  | $x_1^2 x_3^2 x_4 x_5^3 x_6^2 x_8^6 x_9^7 x_{10}^7 x_{11}^7 x_{12}^7$               | $-1 \cdot 2$                       |
| (4, 7, 0, 1) | (0, 0, 1, 0, 1, 1, 0, 1, 1, 1, 1, 3) | 38  | $x_2^2 x_4^2 x_5^2 x_6^5 x_7^3 x_8^6 x_9^6 x_{10}^6 x_{11}^6$                      | $2 \cdot 3$                        |
| (4, 6, 0, 2) | (0, 0, 1, 0, 0, 1, 1, 3, 1, 3, 1, 1) | 32  | $x_1^2 x_2^3 x_4^2 x_5^3 x_6^3 x_7^3 x_8^5 x_{10} x_{11}^5 x_{12}^5$               | $-1 \cdot 2^2$                     |
| (4, 5, 0, 3) | (0, 0, 1, 0, 0, 1, 1, 1, 3, 3, 1, 3) | 30  | $x_2^3 x_4^2 x_5^3 x_6^4 x_7^4 x_8^2 x_9^2 x_{10}^4 x_{11}^2 x_{12}^2$             | 2                                  |
| (4, 4, 0, 4) | (0, 0, 1, 0, 1, 1, 0, 3, 1, 3, 3, 3) | 28  | $x_1 x_2^3 x_4^2 x_5 x_6^3 x_7^3 x_8^3 x_9^3 x_{10}^3 x_{11}^3 x_{12}^3$           | $-1 \cdot 2$                       |
| (4, 7, 1, 0) | (0, 0, 1, 1, 0, 1, 0, 1, 1, 1, 1, 2) | 38  | $x_2^2 x_3 x_4 x_5^2 x_6^5 x_7^3 x_8^6 x_9^6 x_{10}^6 x_{11}^6$                    | $2 \cdot 3$                        |
| (4, 6, 1, 1) | (0, 0, 0, 1, 0, 1, 1, 2, 1, 1, 3, 1) | 32  | $x_2^3 x_3^3 x_5^3 x_6^3 x_7^5 x_9^5 x_{10}^5 x_{12}^5$                            | 2                                  |
| (4, 5, 1, 2) | (0, 0, 0, 1, 0, 1, 1, 3, 1, 3, 1, 2) | 28  | $x_2^3 x_3^3 x_4^2 x_5^3 x_6^3 x_7^4 x_8 x_9^4 x_{10} x_{11}^4$                    | 2                                  |

$$S \subseteq \mathbb{Z}_p \times \mathbb{Z}_4 \setminus \{(0, 0)\}, |S| = 12$$

| $\lambda$    | $\mathbf{a}$                         | deg | monomial/s                                                                                                                                                               | coefficient/s                                         |
|--------------|--------------------------------------|-----|--------------------------------------------------------------------------------------------------------------------------------------------------------------------------|-------------------------------------------------------|
| (4, 4, 1, 3) | (0, 0, 0, 1, 0, 1, 1, 3, 1, 3, 3, 2) | 26  | $x_2^3 x_3^3 x_4^2 x_5^3 x_6^3 x_7^3 x_8^2 x_9^3 x_{10}^2 x_{11}^2$                                                                                                      | 2                                                     |
| (4, 6, 2, 0) | (0, 0, 0, 1, 1, 1, 0, 2, 1, 1, 2, 1) | 33  | $x_2^3 x_3^3 x_5^3 x_6^4 x_7^3 x_8 x_9^5 x_{10}^5 x_{11} x_{12}^5$                                                                                                       | 2                                                     |
| (4, 5, 2, 1) | (0, 0, 1, 0, 1, 1, 0, 2, 1, 1, 3, 2) | 27  | $x_1 x_2^3 x_4^2 x_5^4 x_6^3 x_7^3 x_8 x_9^4 x_{10}^4 x_{12}$                                                                                                            | $2^2$                                                 |
| (4, 4, 2, 2) | (0, 0, 0, 1, 0, 2, 3, 1, 2, 1, 1, 3) | 25  | $x_2^3 x_3^3 x_4^3 x_5^3 x_6 x_7^3 x_8^3 x_9 x_{10}^3 x_{11}^3 x_{12}$                                                                                                   | $-1 \cdot 2^2 \cdot 3$                                |
| (4, 3, 2, 3) | (0, 0, 1, 0, 0, 2, 3, 1, 3, 1, 3, 2) | 23  | $x_1^2 x_2^3 x_3^2 x_4^2 x_5^3 x_7^2 x_8^2 x_9^2 x_{10}^2 x_{11}^2 x_{12}$                                                                                               | $-1 \cdot 2^2 \cdot 3$                                |
| (4, 5, 3, 0) | (0, 0, 0, 1, 1, 0, 1, 2, 1, 1, 2, 2) | 30  | $x_2^3 x_3^3 x_5^3 x_6^4 x_7^2 x_8^4 x_9^4 x_{10}^2 x_{11}^2 x_{12}^2$                                                                                                   | $2^2$                                                 |
| (4, 4, 3, 1) | (0, 0, 0, 1, 1, 0, 1, 2, 2, 3, 1, 2) | 26  | $x_2^3 x_3^3 x_4^2 x_5^3 x_6^3 x_7^3 x_8^2 x_9^2 x_{11}^3 x_{12}^2$                                                                                                      | $-1 \cdot 3$                                          |
| (4, 3, 3, 2) | (0, 0, 0, 1, 1, 0, 3, 2, 3, 1, 2, 2) | 24  | $x_1^2 x_2^2 x_3^3 x_4^2 x_5^2 x_6^3 x_7 x_8^2 x_9 x_{10}^2 x_{11}^2 x_{12}^2$                                                                                           | $-1 \cdot 2$                                          |
| (4, 4, 4, 0) | (0, 0, 1, 1, 0, 1, 0, 2, 2, 2, 1, 2) | 28  | $x_1 x_2^3 x_4 x_5^2 x_6^3 x_7^3 x_8^3 x_9^3 x_{10}^3 x_{11}^3 x_{12}^3$                                                                                                 | $-1 \cdot 2$                                          |
| (4, 3, 4, 1) | (0, 0, 0, 1, 2, 2, 1, 0, 1, 2, 2, 3) | 26  | $x_2^3 x_3^3 x_4^2 x_5^2 x_6^3 x_7^2 x_8^3 x_9^2 x_{10}^3 x_{11}^3$                                                                                                      | $2 \cdot 3$                                           |
| (4, 2, 4, 2) | (0, 0, 1, 0, 2, 2, 2, 3, 0, 1, 3, 2) | 24  | $x_1^2 x_2^3 x_3 x_4^3 x_5^3 x_6^3 x_7^3 x_8 x_9^3 x_{10} x_{11} x_{12}^3$                                                                                               | $2^2$                                                 |
| (4, 3, 5, 0) | (0, 0, 0, 2, 0, 1, 2, 1, 1, 2, 2, 2) | 30  | $x_2^3 x_3^3 x_5^3 x_6^4 x_7^2 x_8^2 x_9^4 x_{10}^4 x_{11}^4 x_{12}^4$                                                                                                   | $-1 \cdot 2^2$                                        |
| (4, 2, 5, 1) | (0, 0, 0, 2, 0, 1, 2, 1, 3, 2, 2, 2) | 28  | $x_2^3 x_3^3 x_4^2 x_5^3 x_6^3 x_7^3 x_8 x_{10}^4 x_{11}^4 x_{12}^4$                                                                                                     | 1                                                     |
| (4, 2, 6, 0) | (0, 0, 0, 2, 0, 1, 2, 2, 2, 2, 2, 1) | 33  | $x_2^3 x_3^3 x_4^2 x_5^3 x_7^2 x_8^4 x_9^5 x_{10}^5 x_{11}^5 x_{12}$                                                                                                     | 1                                                     |
| (4, 1, 6, 1) | (0, 0, 1, 2, 2, 2, 2, 2, 3, 0, 0, 2) | 31  | $x_1^2 x_2^3 x_5^2 x_6^4 x_7^5 x_8^5 x_{10}^2 x_{11}^3 x_{12}^5$                                                                                                         | $-1 \cdot 2$                                          |
| (4, 1, 7, 0) | (0, 0, 2, 0, 0, 1, 2, 2, 2, 2, 2, 2) | 38  | $x_2^3 x_3 x_4^2 x_5^3 x_7^2 x_8^4 x_9^5 x_{10}^6 x_{11}^6 x_{12}^6$                                                                                                     | $-1 \cdot 2$                                          |
| (4, 0, 8, 0) | (0, 0, 2, 0, 0, 2, 2, 2, 2, 2, 2, 2) | 65  | $x_1^2 x_2^3 x_3^5 x_4^3 x_5^3 x_6^7 x_7^7 x_8^7 x_9^7 x_{10}^7 x_{11}^7 x_{12}^7$<br>$x_1^3 x_2^3 x_3^4 x_4^3 x_5^3 x_6^7 x_7^7 x_8^7 x_9^7 x_{10}^7 x_{11}^7 x_{12}^7$ | $2^8 \cdot 3203$<br>$-1 \cdot 2^5 \cdot 31 \cdot 293$ |
| (3, 9, 0, 0) | (0, 1, 1, 0, 1, 0, 1, 1, 1, 1, 1, 1) | 51  | $x_2^2 x_3^2 x_4 x_5^5 x_6^2 x_7^8 x_8^8 x_9^8 x_{10}^8 x_{11}^8 x_{12}^8$                                                                                               | $-1 \cdot 2^2$                                        |
| (3, 8, 0, 1) | (0, 0, 1, 0, 1, 1, 1, 1, 1, 1, 3, 1) | 43  | $x_2^2 x_4^2 x_5 x_6^3 x_7^7 x_8^7 x_9^7 x_{10}^7 x_{12}^7$                                                                                                              | $-1 \cdot 3$                                          |
| (3, 7, 0, 2) | (0, 0, 1, 0, 1, 1, 3, 1, 3, 1, 1, 1) | 37  | $x_2^2 x_3^2 x_4^2 x_5^4 x_6^4 x_7^6 x_8^6 x_9^6 x_{10}^6 x_{11}^6 x_{12}^6$                                                                                             | $-1 \cdot 2$                                          |
| (3, 6, 0, 3) | (0, 0, 1, 0, 1, 1, 1, 3, 3, 3, 1, 1) | 33  | $x_2^2 x_4^2 x_5^3 x_6^5 x_7^5 x_8^2 x_9^2 x_{10}^5 x_{11}^5 x_{12}^5$                                                                                                   | $-1 \cdot 5$                                          |
| (3, 5, 0, 4) | (0, 0, 1, 0, 1, 1, 1, 3, 3, 1, 3, 3) | 31  | $x_2^2 x_3^2 x_4^2 x_5^3 x_6^3 x_7^4 x_8^2 x_9^3 x_{10}^4 x_{11}^3 x_{12}^3$                                                                                             | -1                                                    |
| (3, 8, 1, 0) | (0, 0, 1, 1, 1, 0, 1, 1, 1, 1, 2, 1) | 43  | $x_2^2 x_4^2 x_5^2 x_6^2 x_7^7 x_8^7 x_9^7 x_{10}^7 x_{12}^7$                                                                                                            | $-1 \cdot 3$                                          |
| (3, 7, 1, 1) | (0, 0, 1, 0, 1, 1, 2, 1, 1, 3, 1, 1) | 35  | $x_1^2 x_2^2 x_4^2 x_5^5 x_6^5 x_8^6 x_9^6 x_{11}^6 x_{12}^6$                                                                                                            | -1                                                    |
| (3, 6, 1, 2) | (0, 0, 1, 0, 1, 1, 1, 1, 2, 3, 1, 3) | 31  | $x_2^2 x_4^2 x_5^5 x_6^5 x_7^5 x_8^5 x_{10}^5 x_{11}^5 x_{12}$                                                                                                           | $-1 \cdot 2$                                          |

$$S \subseteq \mathbb{Z}_p \times \mathbb{Z}_4 \setminus \{(0, 0)\}, |S| = 12$$

| $\lambda$     | $\mathbf{a}$                         | deg | monomial/s                                                                                                                                                       | coefficient/s                                                                |
|---------------|--------------------------------------|-----|------------------------------------------------------------------------------------------------------------------------------------------------------------------|------------------------------------------------------------------------------|
| (3, 5, 1, 3)  | (0, 0, 1, 0, 1, 1, 3, 1, 3, 1, 2, 3) | 27  | $x_1^2 x_2^2 x_4^2 x_5^3 x_6^4 x_7^2 x_8^4 x_9^2 x_{10}^4 x_{12}^2$                                                                                              | 2                                                                            |
| (3, 4, 1, 4)  | (0, 0, 1, 0, 1, 1, 2, 3, 3, 3, 1, 3) | 27  | $x_2^2 x_3^2 x_4^2 x_5^3 x_6^3 x_8^3 x_9^3 x_{10}^3 x_{11}^3 x_{12}^3$                                                                                           | 2                                                                            |
| (3, 7, 2, 0)  | (0, 0, 1, 0, 1, 1, 1, 2, 1, 2, 1, 1) | 37  | $x_2^2 x_3 x_4^2 x_5^5 x_6^6 x_7^6 x_8^6 x_{10}^6 x_{11}^6 x_{12}^6$                                                                                             | 2                                                                            |
| (3, 6, 2, 1)  | (0, 0, 1, 0, 1, 1, 1, 2, 1, 3, 1, 2) | 31  | $x_2^2 x_3^2 x_4^2 x_5^3 x_6^5 x_7^5 x_8^5 x_9^5 x_{11}^5 x_{12}^5$                                                                                              | $2^2$                                                                        |
| (3, 5, 2, 2)  | (0, 0, 1, 0, 1, 1, 1, 2, 1, 3, 3, 2) | 27  | $x_2^2 x_3^3 x_4^2 x_5^4 x_6^4 x_7^4 x_8^4 x_{10} x_{11} x_{12}$                                                                                                 | $-1 \cdot 2^2$                                                               |
| (3, 4, 2, 3)  | (0, 0, 1, 0, 1, 1, 3, 1, 3, 2, 3, 2) | 25  | $x_1^2 x_2^2 x_3^3 x_4^2 x_5^2 x_6^3 x_7^2 x_8^3 x_9^2 x_{10} x_{11}^2 x_{12}$                                                                                   | 1                                                                            |
| (3, 6, 3, 0)  | (0, 0, 1, 1, 0, 1, 2, 1, 1, 2, 2, 1) | 32  | $x_1^2 x_2^2 x_4 x_5^2 x_6^4 x_7^2 x_8^5 x_9^5 x_{10}^2 x_{11}^2 x_{12}^5$                                                                                       | $3^2$                                                                        |
| (3, 5, 3, 1)  | (0, 0, 1, 0, 1, 1, 1, 2, 1, 2, 2, 3) | 28  | $x_1^2 x_2^2 x_3^4 x_4^2 x_5^3 x_6^3 x_7^4 x_8^2 x_9^4 x_{10}^2$                                                                                                 | 1                                                                            |
| (3, 4, 3, 2)  | (0, 0, 1, 0, 1, 1, 2, 2, 3, 1, 3, 2) | 24  | $x_1^2 x_2^2 x_3 x_4^2 x_5^3 x_6^3 x_7^2 x_8^2 x_9 x_{10}^3 x_{11} x_{12}^2$                                                                                     | 2                                                                            |
| (3, 3, 3, 3)  | (0, 0, 1, 0, 1, 1, 3, 2, 3, 2, 2, 3) | 24  | $x_1^2 x_2^2 x_3^2 x_4^2 x_5^2 x_6^2 x_7^2 x_8^2 x_9^2 x_{10}^2 x_{11}^2 x_{12}^2$                                                                               | $-1 \cdot 2^2$                                                               |
| (3, 5, 4, 0)  | (0, 0, 1, 1, 0, 1, 1, 2, 1, 2, 2, 2) | 31  | $x_2^2 x_3 x_4^2 x_5^4 x_6^4 x_7^3 x_8^4 x_9^3 x_{10}^3 x_{11}^3 x_{12}^3$                                                                                       | $-1 \cdot 2$                                                                 |
| (3, 4, 4, 1)  | (0, 0, 1, 0, 1, 1, 2, 2, 3, 2, 2, 1) | 27  | $x_1^2 x_2^2 x_3^3 x_4^2 x_5^3 x_6^3 x_7^2 x_8^3 x_{10}^3 x_{11}^3 x_{12}^2$                                                                                     | 1                                                                            |
| (3, 3, 4, 2)  | (0, 0, 1, 0, 2, 3, 1, 3, 2, 2, 1, 2) | 25  | $x_1^2 x_2^2 x_3^2 x_4^2 x_5^2 x_6^2 x_7^2 x_8^3 x_9^3 x_{10}^2 x_{11}^3 x_{12}^3$                                                                               | $2^2$                                                                        |
| (3, 4, 5, 0)  | (0, 0, 1, 1, 0, 1, 2, 2, 2, 2, 1, 2) | 31  | $x_2^2 x_3^3 x_4^2 x_5^2 x_6^3 x_7^4 x_8^4 x_9^4 x_{10}^3 x_{11}^3 x_{12}^4$                                                                                     | -1                                                                           |
| (3, 3, 5, 1)  | (0, 0, 1, 1, 0, 1, 2, 2, 2, 2, 3, 2) | 27  | $x_1^2 x_2^2 x_4 x_5^2 x_6^2 x_7^2 x_8^4 x_9^4 x_{10}^4 x_{12}^4$                                                                                                | $-1 \cdot 2$                                                                 |
| (3, 2, 5, 2)  | (0, 0, 1, 0, 2, 2, 2, 3, 2, 2, 1, 3) | 27  | $x_2^2 x_4^2 x_5^4 x_6^4 x_7^4 x_8^4 x_9^4 x_{10}^4 x_{11} x_{12}$                                                                                               | 3                                                                            |
| (3, 3, 6, 0)  | (0, 0, 1, 1, 0, 2, 2, 1, 2, 2, 2, 2) | 33  | $x_2^2 x_4 x_5^2 x_6^3 x_7^4 x_8^4 x_9^5 x_{10}^5 x_{11}^5 x_{12}^5$                                                                                             | 1                                                                            |
| (3, 2, 6, 1)  | (0, 0, 1, 2, 2, 2, 3, 0, 2, 2, 1, 2) | 31  | $x_2^2 x_3 x_5^5 x_6^5 x_8^5 x_9^5 x_{10}^5 x_{11} x_{12}^5$                                                                                                     | $3^2$                                                                        |
| (3, 2, 7, 0)  | (0, 0, 2, 0, 1, 2, 2, 2, 2, 2, 1, 2) | 36  | $x_1^2 x_2^2 x_4^2 x_6 x_7^4 x_8^6 x_9^6 x_{10}^6 x_{11} x_{12}^6$                                                                                               | $-1 \cdot 2$                                                                 |
| (3, 1, 7, 1)  | (0, 0, 1, 2, 2, 2, 2, 2, 3, 0, 2, 2) | 36  | $x_2^2 x_5^2 x_6^6 x_7^6 x_8^2 x_{10}^6 x_{11}^6 x_{12}^6$                                                                                                       | $-1 \cdot 3$                                                                 |
| (3, 1, 8, 0)  | (0, 0, 2, 0, 2, 2, 1, 2, 2, 2, 2, 2) | 43  | $x_2^2 x_4^2 x_5^4 x_6^4 x_8^6 x_9^7 x_{10}^7 x_{11}^7 x_{12}^7$                                                                                                 | 1                                                                            |
| (3, 0, 9, 0)  | (0, 0, 2, 0, 2, 2, 2, 2, 2, 2, 2, 2) | 72  | $x_2^2 x_3^4 x_4^2 x_5^8 x_6^8 x_7^8 x_8^8 x_9^8 x_{10}^8 x_{11}^8 x_{12}^8$<br>$x_1 x_2^2 x_3^3 x_4^2 x_5^8 x_6^8 x_7^8 x_8^8 x_9^8 x_{10}^8 x_{11}^8 x_{12}^8$ | $2 \cdot 7 \cdot 17 \cdot 29 \cdot 179$<br>$-1 \cdot 2 \cdot 3 \cdot 263951$ |
| (2, 10, 0, 0) | (0, 1, 1, 1, 0, 1, 1, 1, 1, 1, 1, 1) | 59  | $x_2 x_3^3 x_4^3 x_5 x_6^7 x_8^8 x_9^9 x_{10}^9 x_{11}^9 x_{12}^9$                                                                                               | 7                                                                            |
| (2, 9, 0, 1)  | (0, 1, 0, 1, 1, 1, 1, 1, 1, 3, 1, 1) | 49  | $x_1 x_2 x_3 x_4^2 x_5^5 x_6^8 x_7^8 x_8^8 x_{11}^8 x_{12}^8$                                                                                                    | $-1 \cdot 2^2$                                                               |
| (2, 8, 0, 2)  | (0, 1, 0, 1, 1, 1, 1, 1, 1, 3, 1, 3) | 43  | $x_3 x_4^2 x_5^3 x_6^7 x_7^7 x_8^7 x_9^7 x_{10} x_{11}^7 x_{12}$                                                                                                 | $-1 \cdot 2$                                                                 |

$$S \subseteq \mathbb{Z}_p \times \mathbb{Z}_4 \setminus \{(0, 0)\}, |S| = 12$$

| $\lambda$    | $\mathbf{a}$                            | deg | monomial/s                                                                                                                       | coefficient/s        |
|--------------|-----------------------------------------|-----|----------------------------------------------------------------------------------------------------------------------------------|----------------------|
| (2, 7, 0, 3) | (0, 1, 0, 1, 1, 1, 3, 3, 3, 1, 1, 1)    | 37  | $x_1 x_3 x_4 x_5^4 x_6^6 x_7^2 x_8^2 x_9^6 x_{10}^6 x_{11}^6 x_{12}^6$                                                           | $-1 \cdot 2 \cdot 5$ |
| (2, 6, 0, 4) | (0, 1, 0, 1, 1, 1, 1, 3, 3, 3, 3, 1, 3) | 35  | $x_3 x_4^2 x_5^5 x_6^5 x_7^3 x_8^3 x_9^3 x_{10}^5 x_{11}^3 x_{12}^3$                                                             | $2^2$                |
| (2, 5, 0, 5) | (0, 1, 0, 1, 1, 1, 3, 3, 1, 3, 3, 3, 3) | 33  | $x_1 x_3 x_4^2 x_5^3 x_6^4 x_7^2 x_8^4 x_9^4 x_{10}^4 x_{11}^4 x_{12}^4$                                                         | 2                    |
| (2, 9, 1, 0) | (0, 1, 0, 1, 1, 1, 1, 1, 1, 1, 1, 2, 1) | 50  | $x_2 x_3 x_4^2 x_5^6 x_6^8 x_7^8 x_8^8 x_9^8 x_{10}^8 x_{12}^8$                                                                  | $2 \cdot 3$          |
| (2, 8, 1, 1) | (0, 1, 0, 1, 1, 1, 1, 1, 1, 3, 1, 2)    | 42  | $x_2^2 x_3 x_4 x_5^3 x_6^7 x_7^7 x_8^7 x_9^7 x_{11}^7$                                                                           | 5                    |
| (2, 7, 1, 2) | (0, 1, 0, 1, 1, 1, 1, 2, 3, 1, 3, 1)    | 36  | $x_3 x_4^3 x_5^6 x_6^6 x_7^6 x_9^6 x_{10}^6 x_{11}^6 x_{12}^6$<br>$x_3 x_4^4 x_5^5 x_6^6 x_7^6 x_9^6 x_{10}^6 x_{11}^6 x_{12}^6$ | $3 \cdot 7$<br>13    |
| (2, 6, 1, 3) | (0, 1, 0, 1, 1, 1, 1, 2, 3, 1, 3, 3)    | 32  | $x_2^2 x_3 x_4^4 x_5^4 x_6^5 x_7^2 x_9^5 x_{10}^2 x_{11}^2 x_{12}^2$                                                             | 5                    |
| (2, 5, 1, 4) | (0, 1, 0, 1, 1, 1, 3, 3, 1, 3, 3, 2)    | 30  | $x_2^2 x_3 x_4^3 x_5^4 x_6^4 x_7^3 x_8^3 x_9^4 x_{10}^3 x_{11}^3$                                                                | $-1 \cdot 2 \cdot 3$ |
| (2, 8, 2, 0) | (0, 1, 0, 1, 1, 1, 2, 1, 2, 1, 1, 1)    | 42  | $x_1 x_3 x_4 x_5^2 x_6^7 x_7^7 x_8^7 x_9^7 x_{10}^7 x_{11}^7 x_{12}^7$                                                           | 1                    |
| (2, 7, 2, 1) | (0, 1, 0, 1, 1, 1, 1, 2, 1, 2, 1, 3)    | 36  | $x_3 x_4^3 x_5^6 x_6^6 x_7^6 x_8^6 x_9^6 x_{10}^6 x_{11}^6$                                                                      | $2 \cdot 3^2$        |
| (2, 6, 2, 2) | (0, 1, 0, 1, 1, 1, 1, 2, 3, 1, 3, 2)    | 30  | $x_1 x_3 x_4^4 x_5^5 x_6^5 x_7^5 x_8 x_9 x_{10}^5 x_{11} x_{12}$                                                                 | 5                    |
| (2, 5, 2, 3) | (0, 1, 0, 1, 1, 1, 1, 2, 3, 2, 3, 3)    | 28  | $x_2^3 x_3 x_4^4 x_5^4 x_6^4 x_7^4 x_8 x_9^2 x_{10}^2 x_{11}^2 x_{12}^2$                                                         | $2^2$                |
| (2, 4, 2, 4) | (0, 1, 0, 1, 1, 2, 3, 3, 3, 1, 3, 2)    | 26  | $x_1 x_2 x_3 x_4^3 x_5^3 x_6^3 x_7^3 x_8^3 x_9^3 x_{10}^3 x_{11}^3 x_{12}^3$                                                     | $2^2 \cdot 3^2$      |
| (2, 7, 3, 0) | (0, 1, 0, 1, 1, 1, 2, 1, 1, 2, 1, 2)    | 38  | $x_2^2 x_3 x_4 x_5^4 x_6^6 x_7^6 x_8^6 x_9^6 x_{10}^6 x_{11}^6 x_{12}^6$                                                         | $2^4 \cdot 3$        |
| (2, 6, 3, 1) | (0, 1, 0, 1, 1, 1, 1, 2, 3, 2, 2, 1)    | 32  | $x_2 x_3 x_4^4 x_5^5 x_6^5 x_7^5 x_8^2 x_{10}^2 x_{11}^2 x_{12}^5$                                                               | $2 \cdot 3$          |
| (2, 5, 3, 2) | (0, 1, 0, 1, 1, 1, 2, 1, 2, 2, 3, 3)    | 28  | $x_2^3 x_3 x_4^4 x_5^4 x_6^4 x_7^4 x_8^2 x_9^2 x_{10}^2 x_{11} x_{12}$                                                           | $-1 \cdot 2^2$       |
| (2, 4, 3, 3) | (0, 1, 0, 1, 1, 2, 1, 2, 3, 3, 3, 2)    | 26  | $x_1 x_2^3 x_3 x_4^3 x_5^3 x_6^2 x_7^3 x_8^2 x_9^2 x_{10}^2 x_{11}^2 x_{12}^2$                                                   | $2^5$                |
| (2, 6, 4, 0) | (0, 1, 0, 1, 1, 1, 2, 1, 2, 2, 1, 2)    | 35  | $x_3 x_4^3 x_5^4 x_6^5 x_7^3 x_8^5 x_9^3 x_{10}^3 x_{11}^5 x_{12}^3$                                                             | $3 \cdot 5$          |
| (2, 5, 4, 1) | (0, 1, 0, 1, 1, 1, 2, 1, 2, 2, 3, 2)    | 29  | $x_1 x_3 x_4^3 x_5^4 x_6^4 x_7^3 x_8^4 x_9^3 x_{10}^3 x_{12}^3$                                                                  | $-1 \cdot 2 \cdot 3$ |
| (2, 4, 4, 2) | (0, 1, 0, 1, 1, 2, 1, 2, 3, 2, 2, 3)    | 27  | $x_2^3 x_3 x_4^3 x_5^3 x_6^3 x_7^3 x_8^3 x_9 x_{10}^3 x_{11}^3 x_{12}$                                                           | $-1 \cdot 2^3$       |
| (2, 3, 4, 3) | (0, 1, 0, 1, 1, 2, 2, 3, 2, 3, 3, 2)    | 25  | $x_1 x_2^2 x_3 x_4^2 x_5^2 x_6^3 x_7^3 x_8^2 x_9^3 x_{10}^2 x_{11} x_{12}^3$                                                     | 2                    |
| (2, 5, 5, 0) | (0, 1, 0, 1, 1, 1, 2, 2, 2, 1, 2, 2)    | 34  | $x_3 x_4 x_5^4 x_6^4 x_7^4 x_8^4 x_9^4 x_{10}^4 x_{11}^4 x_{12}^4$                                                               | $-1 \cdot 2$         |
| (2, 4, 5, 1) | (0, 1, 0, 1, 1, 2, 2, 3, 2, 2, 1, 2)    | 30  | $x_2^2 x_3 x_4 x_5^3 x_6^4 x_7^4 x_9^4 x_{10}^3 x_{11}^4 x_{12}^4$                                                               | $3^2$                |
| (2, 3, 5, 2) | (0, 1, 0, 1, 2, 2, 1, 2, 2, 3, 2, 3)    | 28  | $x_1 x_3 x_4^2 x_5^4 x_6^4 x_7^4 x_8^4 x_9^4 x_{10}^4 x_{11} x_{12}$                                                             | 1                    |
| (2, 4, 6, 0) | (0, 1, 1, 0, 1, 2, 2, 2, 2, 1, 2, 2)    | 34  | $x_1 x_3 x_4 x_5^2 x_6^5 x_7^5 x_8^5 x_9^3 x_{10}^5 x_{11}^5 x_{12}^5$                                                           | $-1 \cdot 5$         |

$$S \subseteq \mathbb{Z}_p \times \mathbb{Z}_4 \setminus \{(0, 0)\}, |S| = 12$$

| $\lambda$     | $\mathbf{a}$                         | deg | monomial/s                                                                                                                          | coefficient/s                                          |
|---------------|--------------------------------------|-----|-------------------------------------------------------------------------------------------------------------------------------------|--------------------------------------------------------|
| (2, 3, 6, 1)  | (0, 1, 0, 1, 1, 2, 2, 2, 2, 3, 2, 2) | 32  | $x_3x_4^2x_5^2x_6^2x_7^5x_8^5x_9^5x_{11}^5x_{12}^5$                                                                                 | $-1 \cdot 2$                                           |
| (2, 2, 6, 2)  | (0, 1, 0, 2, 2, 2, 3, 2, 2, 1, 3, 2) | 30  | $x_1x_3x_5^5x_6^5x_7x_8^5x_9^5x_{10}x_{11}x_{12}^5$                                                                                 | $-1 \cdot 3^2$                                         |
| (2, 3, 7, 0)  | (0, 1, 1, 0, 2, 2, 1, 2, 2, 2, 2, 2) | 38  | $x_2x_3x_4x_5^2x_6^4x_7^2x_8^4x_9^5x_{10}^6x_{11}^6x_{12}^6$                                                                        | 2                                                      |
| (2, 2, 7, 1)  | (0, 1, 0, 2, 2, 2, 3, 2, 2, 2, 2, 1) | 36  | $x_3x_4x_5^3x_6^6x_8^6x_9^6x_{10}^6x_{11}^6x_{12}$                                                                                  | $-1 \cdot 2$                                           |
| (2, 2, 8, 0)  | (0, 1, 2, 0, 2, 2, 2, 1, 2, 2, 2, 2) | 43  | $x_4x_5^2x_6^4x_7x_8x_9^7x_{10}^7x_{11}^7x_{12}^7$                                                                                  | $-1 \cdot 2$                                           |
| (2, 1, 8, 1)  | (0, 1, 2, 2, 2, 2, 2, 3, 0, 2, 2, 2) | 41  | $x_1x_4^2x_5^3x_6^6x_7^7x_9x_{10}^7x_{11}^7x_{12}^7$                                                                                | $-1 \cdot 5$                                           |
| (2, 1, 9, 0)  | (0, 2, 0, 2, 2, 1, 2, 2, 2, 2, 2, 2) | 50  | $x_2x_3x_4^4x_5^7x_6^6x_7x_8^8x_{10}^8x_{11}^8x_{12}^8$                                                                             | $-1 \cdot 3$                                           |
| (2, 0, 10, 0) | (0, 2, 0, 2, 2, 2, 2, 2, 2, 2, 2, 2) | 79  | $x_1x_2^5x_3x_4^8x_5^9x_6^9x_7x_8^9x_9^9x_{10}^9x_{11}^9x_{12}^9$<br>$x_1x_2^5x_3x_4^9x_5^9x_6^9x_8^9x_9^9x_{10}^9x_{11}^9x_{12}^9$ | $-1 \cdot 197 \cdot 78623$<br>$5 \cdot 61 \cdot 18223$ |
| (1, 11, 0, 0) | (0, 1, 1, 1, 1, 1, 1, 1, 1, 1, 1, 1) | 69  | $x_2x_3^2x_4^5x_5^5x_6^6x_7^{10}x_9^{10}x_{10}^{10}x_{11}^{10}x_{12}^{10}$                                                          | 5                                                      |
| (1, 10, 0, 1) | (0, 1, 1, 1, 1, 1, 1, 1, 3, 1, 1, 1) | 59  | $x_2^2x_3^2x_4^3x_5^7x_6^9x_8^9x_{10}^9x_{11}^9x_{12}^9$                                                                            | $-1 \cdot 3$                                           |
| (1, 9, 0, 2)  | (0, 1, 1, 1, 1, 1, 1, 1, 3, 3, 1, 1) | 51  | $x_2x_3^2x_4^6x_5^8x_6^8x_8^8x_9x_{10}x_{11}^8x_{12}^8$                                                                             | 5                                                      |
| (1, 8, 0, 3)  | (0, 1, 1, 1, 1, 1, 1, 1, 3, 1, 3, 3) | 45  | $x_2x_3x_4^2x_5^7x_6^7x_7^7x_8^2x_9^7x_{10}^2x_{11}^2x_{12}^2$                                                                      | $-1 \cdot 2^2$                                         |
| (1, 7, 0, 4)  | (0, 1, 1, 1, 1, 3, 3, 3, 1, 3, 1, 1) | 41  | $x_3x_4^4x_5^6x_6^3x_7^3x_8^3x_9^3x_{10}^6x_{11}^6x_{12}^6$<br>$x_3^2x_4^3x_5^6x_6^3x_7^3x_8^3x_9^3x_{10}^6x_{11}^6x_{12}^6$        | $-1 \cdot 3 \cdot 23$<br>$-1 \cdot 61$                 |
| (1, 6, 0, 5)  | (0, 1, 1, 1, 1, 1, 3, 3, 3, 1, 3, 3) | 39  | $x_2x_3x_4^4x_5^5x_6^3x_7^3x_8^4x_9^5x_{10}^4x_{11}^4x_{12}^4$                                                                      | -1                                                     |
| (1, 10, 1, 0) | (1, 0, 1, 1, 1, 1, 1, 1, 1, 2, 1, 1) | 58  | $x_1x_2^2x_3^3x_4^7x_5^9x_6^9x_8^9x_9^9x_{11}^9x_{12}^9$                                                                            | $2 \cdot 5$                                            |
| (1, 9, 1, 1)  | (0, 1, 1, 1, 1, 1, 1, 1, 1, 1, 2, 3) | 50  | $x_2^2x_3^3x_4^5x_5^8x_6^8x_8^8x_9^8x_{10}^8$                                                                                       | $2 \cdot 3$                                            |
| (1, 8, 1, 2)  | (1, 1, 1, 3, 2, 1, 0, 1, 1, 3, 1, 1) | 42  | $x_2x_3^5x_4x_6^6x_7^7x_8^7x_{10}x_{11}^7x_{12}^7$                                                                                  | $2^2$                                                  |
| (1, 7, 1, 3)  | (3, 1, 1, 1, 0, 3, 1, 1, 1, 3, 2, 1) | 38  | $x_2x_3^3x_4^6x_6^2x_7^6x_8^6x_9^6x_{10}^2x_{12}^6$                                                                                 | $-1 \cdot 2$                                           |
| (1, 6, 1, 4)  | (1, 3, 3, 3, 1, 2, 0, 1, 1, 3, 1, 1) | 34  | $x_2^2x_3x_4^3x_5^5x_8^5x_9^3x_{10}^3x_{11}^5x_{12}^5$                                                                              | $-1 \cdot 2 \cdot 3$                                   |
| (1, 5, 1, 5)  | (1, 3, 3, 0, 1, 1, 1, 3, 3, 2, 1, 3) | 34  | $x_2^2x_3^4x_5^4x_6^4x_7^4x_8^4x_9^4x_{11}^4x_{12}^4$<br>$x_1x_2x_3^4x_4^4x_5^4x_6^4x_7^4x_8^4x_9^4x_{11}^4x_{12}^4$                | $-1 \cdot 2^2 \cdot 19$<br>$-1 \cdot 2 \cdot 79$       |
| (1, 9, 2, 0)  | (1, 1, 1, 1, 0, 1, 1, 1, 2, 1, 1, 2) | 51  | $x_1^2x_2^3x_3^4x_4^8x_6^8x_8^8x_9x_{10}^8x_{11}^8x_{12}$                                                                           | $-1 \cdot 2 \cdot 3 \cdot 7$                           |
| (1, 8, 2, 1)  | (1, 0, 2, 3, 1, 1, 2, 1, 1, 1, 1, 1) | 43  | $x_3x_5^3x_6^4x_7x_8^6x_9^7x_{10}^7x_{11}^7x_{12}^7$                                                                                | $-1 \cdot 2$                                           |
| (1, 7, 2, 2)  | (1, 2, 1, 2, 1, 3, 1, 0, 1, 1, 1, 3) | 37  | $x_1x_3^3x_4x_5^6x_6^6x_7^6x_9^6x_{10}^6x_{11}^6x_{12}$                                                                             | $3 \cdot 5$                                            |
| (1, 6, 2, 3)  | (2, 3, 2, 3, 1, 1, 1, 3, 1, 0, 1, 1) | 33  | $x_2x_3x_4^2x_5^3x_6^4x_7^5x_8^2x_9^5x_{11}^5x_{12}^5$                                                                              | $-1 \cdot 2$                                           |

$$S \subseteq \mathbb{Z}_p \times \mathbb{Z}_4 \setminus \{(0, 0)\}, |S| = 12$$

| $\lambda$     | $\mathbf{a}$                         | deg | monomial/s                                                                                                                                                               | coefficient/s         |
|---------------|--------------------------------------|-----|--------------------------------------------------------------------------------------------------------------------------------------------------------------------------|-----------------------|
| (1, 5, 2, 4)  | (0, 1, 1, 1, 3, 3, 1, 2, 3, 3, 1, 2) | 31  | $x_2^4 x_3^3 x_4^4 x_5^3 x_6^3 x_7^3 x_8^3 x_9^3 x_{10}^3 x_{11}^4$                                                                                                      | 2                     |
| (1, 8, 3, 0)  | (2, 1, 2, 1, 1, 1, 1, 2, 0, 1, 1, 1) | 45  | $x_1 x_3 x_4^3 x_5^4 x_6^6 x_7^7 x_8^2 x_{10}^7 x_{11}^7 x_{12}^7$                                                                                                       | 1                     |
| (1, 7, 3, 1)  | (1, 1, 1, 3, 1, 2, 0, 1, 2, 2, 1, 1) | 37  | $x_2 x_3^6 x_5^6 x_6^2 x_8^6 x_9^2 x_{10}^2 x_{11}^6 x_{12}^6$                                                                                                           | $2 \cdot 3^2$         |
| (1, 6, 3, 2)  | (1, 0, 2, 3, 1, 3, 2, 2, 1, 1, 1, 1) | 33  | $x_3^2 x_4 x_5^5 x_6 x_7^2 x_8^2 x_9^5 x_{10}^5 x_{11}^5 x_{12}^5$                                                                                                       | $-1 \cdot 2$          |
| (1, 5, 3, 3)  | (3, 1, 2, 1, 2, 1, 1, 2, 1, 3, 0, 3) | 29  | $x_2^3 x_3^2 x_4^4 x_5^2 x_6^4 x_7^2 x_8^2 x_9^4 x_{10}^2 x_{12}^2$                                                                                                      | $2 \cdot 3$           |
| (1, 4, 3, 4)  | (0, 1, 3, 2, 3, 2, 2, 1, 1, 3, 1, 3) | 29  | $x_2^3 x_3^3 x_4 x_5^3 x_6^2 x_7^2 x_8^3 x_9^3 x_{10}^3 x_{11}^3 x_{12}^3$                                                                                               | $2^2$                 |
| (1, 7, 4, 0)  | (1, 0, 1, 1, 2, 2, 1, 2, 2, 1, 1, 1) | 41  | $x_1 x_3 x_4^3 x_5^3 x_6^3 x_7^6 x_8^3 x_9^3 x_{10}^6 x_{11}^6 x_{12}^6$                                                                                                 | $-1 \cdot 2^4$        |
| (1, 6, 4, 1)  | (1, 2, 3, 1, 1, 2, 2, 2, 1, 1, 1, 0) | 35  | $x_1^2 x_4^4 x_5^5 x_6^3 x_7^3 x_8^3 x_9^5 x_{10}^5 x_{11}^5$                                                                                                            | $2^2 \cdot 3$         |
| (1, 5, 4, 2)  | (2, 3, 0, 1, 2, 3, 1, 2, 1, 1, 1, 2) | 31  | $x_1^3 x_2 x_4^3 x_5^3 x_6 x_7^4 x_8^3 x_9^4 x_{10}^4 x_{11}^4 x_{12}$                                                                                                   | $3^2$                 |
| (1, 4, 4, 3)  | (3, 2, 3, 2, 3, 2, 1, 2, 0, 1, 1, 1) | 29  | $x_1^2 x_2^3 x_3^2 x_4^3 x_5^2 x_6^3 x_7^3 x_8^3 x_{10}^3 x_{11}^2 x_{12}^3$                                                                                             | 3                     |
| (1, 6, 5, 0)  | (1, 1, 2, 2, 1, 0, 2, 2, 2, 1, 1, 1) | 38  | $x_2 x_3^2 x_4^3 x_5^5 x_7^4 x_8^4 x_9^5 x_{10}^5 x_{11}^5 x_{12}^5$                                                                                                     | 2                     |
| (1, 5, 5, 1)  | (0, 1, 1, 1, 2, 2, 2, 1, 2, 1, 2, 3) | 34  | $x_3^3 x_4^3 x_5^4 x_6^4 x_7^4 x_8^4 x_9^4 x_{10}^4 x_{11}^4$                                                                                                            | $2^5$                 |
| (1, 4, 5, 2)  | (2, 1, 2, 2, 2, 1, 3, 0, 1, 2, 3, 1) | 30  | $x_2^3 x_3^4 x_4^4 x_5^4 x_6^3 x_7 x_9^3 x_{10}^4 x_{11} x_{12}^3$                                                                                                       | $2^3$                 |
| (1, 3, 5, 3)  | (2, 2, 0, 1, 2, 1, 3, 2, 2, 3, 3, 1) | 30  | $x_1^2 x_2^4 x_3^2 x_4^4 x_5^2 x_6^2 x_7^4 x_8^4 x_9^2 x_{10}^2 x_{11}^2 x_{12}^2$<br>$x_1^3 x_2^3 x_3^2 x_4^4 x_5^2 x_6^2 x_7^4 x_8^4 x_9^2 x_{10}^2 x_{11}^2 x_{12}^2$ | $83$<br>$2^3 \cdot 5$ |
| (1, 5, 6, 0)  | (2, 1, 1, 2, 2, 2, 1, 1, 1, 2, 2, 0) | 39  | $x_2^2 x_4^5 x_5^5 x_6^5 x_7^4 x_8^4 x_9^5 x_{10}^5 x_{11}^5$                                                                                                            | $2^3 \cdot 3$         |
| (1, 4, 6, 1)  | (1, 1, 2, 2, 1, 0, 2, 2, 2, 3, 2, 1) | 35  | $x_2 x_3^3 x_4^5 x_5^3 x_7^5 x_8^5 x_9^5 x_{11}^5 x_{12}^3$                                                                                                              | 5                     |
| (1, 3, 6, 2)  | (1, 1, 2, 1, 2, 0, 3, 2, 2, 3, 2, 2) | 33  | $x_1 x_2 x_3^3 x_4^2 x_5^4 x_7 x_8^5 x_9^5 x_{10} x_{11}^5 x_{12}^5$                                                                                                     | $2 \cdot 3 \cdot 5$   |
| (1, 4, 7, 0)  | (2, 1, 2, 0, 2, 1, 2, 2, 2, 1, 2, 1) | 41  | $x_1 x_3 x_5^6 x_6^3 x_7^6 x_8^6 x_9^3 x_{10}^6 x_{11}^6 x_{12}^3$                                                                                                       | $-1 \cdot 3$          |
| (1, 3, 7, 1)  | (2, 2, 3, 2, 0, 2, 2, 1, 1, 2, 1, 2) | 37  | $x_2^3 x_4^4 x_6^6 x_7^2 x_8^2 x_9^6 x_{10}^2 x_{11}^6 x_{12}^6$                                                                                                         | $2^2 \cdot 3$         |
| (1, 2, 7, 2)  | (0, 1, 2, 2, 2, 3, 2, 3, 2, 1, 2, 2) | 37  | $x_3 x_4^3 x_5^6 x_6 x_7^6 x_8^6 x_9 x_{10} x_{11}^6 x_{12}^6$<br>$x_3 x_4^4 x_5^5 x_6 x_7^6 x_8^6 x_9 x_{10} x_{11}^6 x_{12}^6$                                         | $3^2 \cdot 7$<br>47   |
| (1, 3, 8, 0)  | (2, 1, 2, 1, 2, 2, 2, 1, 2, 0, 2, 2) | 45  | $x_2 x_3 x_4^2 x_5^4 x_6^7 x_7^7 x_8^2 x_9^7 x_{11}^7 x_{12}^7$                                                                                                          | $2^2$                 |
| (1, 2, 8, 1)  | (1, 2, 2, 1, 2, 2, 2, 2, 2, 3, 0, 2) | 43  | $x_1 x_3^4 x_4 x_5^3 x_6^6 x_7^7 x_8^7 x_9^7 x_{12}^7$                                                                                                                   | 2                     |
| (1, 2, 9, 0)  | (2, 1, 2, 2, 2, 2, 0, 2, 1, 2, 2, 2) | 50  | $x_3 x_4^4 x_5^4 x_6^8 x_8^8 x_9 x_{10}^8 x_{11}^8 x_{12}^8$                                                                                                             | $-1 \cdot 5$          |
| (1, 1, 9, 1)  | (2, 2, 2, 1, 2, 0, 2, 2, 2, 2, 3, 2) | 50  | $x_1^2 x_2^3 x_3^5 x_5^8 x_8^8 x_9^8 x_{10}^8 x_{12}^8$                                                                                                                  | 1                     |
| (1, 1, 10, 0) | (2, 0, 2, 2, 2, 1, 2, 2, 2, 2, 2, 2) | 59  | $x_1 x_3^3 x_4^5 x_5^8 x_7^8 x_9^8 x_{10}^9 x_{11}^9 x_{12}^9$                                                                                                           | 3                     |

$$S \subseteq \mathbb{Z}_p \times \mathbb{Z}_4 \setminus \{(0, 0)\}, |S| = 12$$

| $\lambda$     | $\mathbf{a}$                            | deg | monomial/s                                                                                                                                                                                 | coefficient/s                                                                        |
|---------------|-----------------------------------------|-----|--------------------------------------------------------------------------------------------------------------------------------------------------------------------------------------------|--------------------------------------------------------------------------------------|
| (1, 0, 11, 0) | (0, 2, 2, 2, 2, 2, 2, 2, 2, 2, 2, 2)    | 90  | $x_2^5 x_3^6 x_4^9 x_5^{10} x_6^{10} x_8^{10} x_9^{10} x_{10}^{10} x_{11}^{10} x_{12}^{10}$<br>$x_2^4 x_3^7 x_4^9 x_5^{10} x_6^{10} x_8^{10} x_9^{10} x_{10}^{10} x_{11}^{10} x_{12}^{10}$ | $-1 \cdot 2^3 \cdot 3^2 \cdot 281627$<br>$-1 \cdot 2^2 \cdot 7 \cdot 13 \cdot 73583$ |
| (0, 12, 0, 0) | (1, 1, 1, 1, 1, 1, 1, 1, 1, 1, 1, 1)    | 80  | $x_1 x_2^2 x_3^4 x_4^5 x_5^6 x_8^{10} x_9^{11} x_{10}^{11} x_{11}^{11} x_{12}^{11}$                                                                                                        | 2                                                                                    |
| (0, 11, 0, 1) | (1, 1, 1, 1, 1, 1, 1, 1, 1, 1, 1, 3)    | 70  | $x_1 x_2^3 x_3^4 x_4^5 x_5^7 x_6^{10} x_8^{10} x_9^{10} x_{10}^{10} x_{11}^{10}$                                                                                                           | $-1 \cdot 7$                                                                         |
| (0, 10, 0, 2) | (1, 1, 3, 1, 1, 1, 1, 1, 1, 3, 1, 1)    | 60  | $x_1 x_2^2 x_3^4 x_4^6 x_5^9 x_6^9 x_8^9 x_{10}^9 x_{11}^9 x_{12}^9$                                                                                                                       | $-1 \cdot 3$                                                                         |
| (0, 9, 0, 3)  | (1, 1, 1, 1, 1, 3, 3, 3, 1, 1, 1, 1)    | 54  | $x_2^2 x_3^2 x_4^6 x_5^8 x_6^2 x_8^8 x_9^8 x_{10}^8 x_{11}^8 x_{12}^8$                                                                                                                     | $3 \cdot 7$                                                                          |
| (0, 8, 0, 4)  | (1, 1, 1, 1, 3, 3, 1, 1, 1, 1, 3, 3)    | 48  | $x_1 x_2^3 x_3^4 x_4^7 x_5^3 x_6^7 x_8^7 x_9^7 x_{10}^3 x_{11}^3 x_{12}^3$                                                                                                                 | $-1 \cdot 2 \cdot 3 \cdot 5$                                                         |
| (0, 7, 0, 5)  | (3, 3, 3, 1, 3, 1, 1, 1, 3, 1, 1, 1)    | 46  | $x_2^2 x_3^2 x_4^2 x_5^4 x_6^4 x_7^6 x_8^4 x_9^6 x_{10}^6 x_{11}^6 x_{12}^6$                                                                                                               | $-1 \cdot 2$                                                                         |
| (0, 6, 0, 6)  | (3, 1, 1, 1, 3, 3, 3, 3, 3, 1, 1, 1)    | 44  | $x_2^2 x_3^3 x_4^3 x_5^5 x_6^5 x_7^5 x_8^5 x_9^5 x_{10}^5 x_{11}^5 x_{12}^5$                                                                                                               | 2                                                                                    |
| (0, 11, 1, 0) | (1, 1, 1, 1, 1, 1, 1, 1, 1, 1, 1, 2)    | 70  | $x_1^2 x_2^2 x_3^4 x_4^5 x_5^7 x_6^{10} x_8^{10} x_9^{10} x_{10}^{10} x_{11}^{10}$                                                                                                         | $-1 \cdot 5$                                                                         |
| (0, 10, 1, 1) | (1, 1, 1, 1, 1, 1, 2, 1, 1, 1, 3, 1)    | 60  | $x_1 x_2^2 x_3^5 x_4^7 x_5^9 x_6^9 x_8^9 x_9^9 x_{10}^9 x_{12}^9$                                                                                                                          | $-1 \cdot 3^2$                                                                       |
| (0, 9, 1, 2)  | (1, 2, 1, 1, 1, 3, 1, 1, 3, 1, 1, 1)    | 52  | $x_1^2 x_3^3 x_4^5 x_5^8 x_6^8 x_8^8 x_9^8 x_{10}^8 x_{11}^8 x_{12}^8$                                                                                                                     | $-1$                                                                                 |
| (0, 8, 1, 3)  | (1, 3, 3, 3, 1, 1, 1, 1, 2, 1, 1, 1)    | 46  | $x_2 x_3^2 x_4^2 x_5^3 x_6^4 x_7^6 x_8^7 x_{10}^7 x_{11}^7 x_{12}^7$                                                                                                                       | 2                                                                                    |
| (0, 7, 1, 4)  | (1, 1, 1, 3, 2, 1, 1, 1, 1, 3, 3, 3)    | 42  | $x_1 x_2^2 x_3^3 x_4^6 x_5^6 x_6^6 x_7^6 x_8^6 x_9^3 x_{10}^3 x_{11}^3 x_{12}^3$<br>$x_1 x_2^3 x_3^2 x_4^3 x_5^6 x_6^6 x_7^6 x_8^6 x_9^3 x_{10}^3 x_{11}^3 x_{12}^3$                       | $-1 \cdot 3 \cdot 7$<br>29                                                           |
| (0, 6, 1, 5)  | (1, 3, 1, 3, 2, 3, 1, 1, 3, 1, 3, 1)    | 40  | $x_2 x_3^3 x_4^4 x_5^5 x_6^5 x_7^4 x_8^5 x_9^4 x_{10}^4 x_{11}^4 x_{12}^5$<br>$x_2^2 x_3^2 x_4^4 x_5^5 x_6^5 x_7^4 x_8^5 x_9^4 x_{10}^4 x_{11}^4 x_{12}^5$                                 | $-1 \cdot 2^2 \cdot 19$<br>$-1 \cdot 2 \cdot 3 \cdot 17$                             |
| (0, 10, 2, 0) | (1, 1, 1, 1, 1, 1, 1, 1, 1, 2, 1, 2)    | 61  | $x_1 x_2^3 x_3^4 x_4^9 x_5^9 x_6^9 x_8^9 x_9^9 x_{10}^9 x_{11}^9 x_{12}^9$                                                                                                                 | $5^2$                                                                                |
| (0, 9, 2, 1)  | (1, 1, 1, 2, 1, 1, 1, 1, 2, 3, 1, 1, 1) | 51  | $x_1 x_2^2 x_3^6 x_4^8 x_5^8 x_6^8 x_8^8 x_{10}^8 x_{11}^8 x_{12}^8$                                                                                                                       | $2 \cdot 3 \cdot 5$                                                                  |
| (0, 8, 2, 2)  | (1, 2, 3, 1, 1, 1, 3, 1, 1, 1, 2, 1)    | 45  | $x_3 x_4^2 x_5^5 x_6^7 x_7^8 x_8^7 x_9^7 x_{10}^7 x_{11}^7 x_{12}^7$                                                                                                                       | $2^2$                                                                                |
| (0, 7, 2, 3)  | (2, 1, 1, 1, 1, 3, 3, 1, 2, 3, 1, 1)    | 39  | $x_3^3 x_4^5 x_5^6 x_6^2 x_7^6 x_8^6 x_9 x_{10}^2 x_{11}^6 x_{12}^6$                                                                                                                       | 1                                                                                    |
| (0, 6, 2, 4)  | (1, 1, 1, 3, 3, 3, 1, 2, 3, 1, 1, 2)    | 37  | $x_2^3 x_3^5 x_4^3 x_5^3 x_6^5 x_7^8 x_8^3 x_{10}^5 x_{11}^5 x_{12}^5$<br>$x_2^4 x_3^4 x_4^3 x_5^3 x_6^5 x_7^8 x_8^3 x_{10}^5 x_{11}^5 x_{12}^5$                                           | $-1 \cdot 11 \cdot 13$<br>$-1 \cdot 41$                                              |
| (0, 5, 2, 5)  | (3, 1, 1, 1, 3, 2, 1, 3, 3, 3, 1, 2)    | 35  | $x_2^2 x_3^3 x_4^4 x_5^4 x_6^4 x_7^4 x_8^4 x_9^4 x_{10}^4 x_{11}^4 x_{12}^4$<br>$x_2^3 x_3^3 x_4^3 x_5^4 x_6^4 x_7^4 x_8^4 x_9^4 x_{10}^4 x_{11}^4 x_{12}^4$                               | $2 \cdot 5$<br>7                                                                     |
| (0, 9, 3, 0)  | (1, 2, 1, 1, 1, 1, 1, 2, 1, 2, 1, 1, 1) | 54  | $x_1 x_2 x_3^4 x_4^4 x_5^8 x_7^8 x_8^2 x_{10}^8 x_{11}^8 x_{12}^8$                                                                                                                         | $-1 \cdot 2^2 \cdot 3^2$                                                             |
| (0, 8, 3, 1)  | (1, 1, 1, 2, 1, 2, 3, 2, 1, 1, 1, 1)    | 46  | $x_1^2 x_2 x_3^4 x_4^2 x_5^5 x_6^2 x_8^7 x_9^7 x_{10}^7 x_{11}^7 x_{12}^7$                                                                                                                 | $-1 \cdot 2^3 \cdot 3$                                                               |
| (0, 7, 3, 2)  | (1, 2, 1, 3, 1, 2, 1, 2, 1, 3, 1, 1)    | 40  | $x_2 x_3^3 x_4 x_5^6 x_6^2 x_7^6 x_8^2 x_9 x_{10}^6 x_{11}^6 x_{12}^6$                                                                                                                     | $2 \cdot 5$                                                                          |

$$S \subseteq \mathbb{Z}_p \times \mathbb{Z}_4 \setminus \{(0, 0)\}, |S| = 12$$

| $\lambda$    | $\mathbf{a}$                         | deg | monomial/s                                                                                                                                                              | coefficient/s                                                      |
|--------------|--------------------------------------|-----|-------------------------------------------------------------------------------------------------------------------------------------------------------------------------|--------------------------------------------------------------------|
| (0, 6, 3, 3) | (1, 3, 3, 2, 1, 2, 2, 1, 3, 1, 1, 1) | 36  | $x_1 x_2 x_3^2 x_4^2 x_5^4 x_6^2 x_7 x_8^2 x_9^2 x_{10}^5 x_{11}^5 x_{12}^5$                                                                                            | $2 \cdot 3$                                                        |
| (0, 5, 3, 4) | (2, 1, 3, 3, 1, 3, 2, 1, 1, 2, 1, 3) | 34  | $\frac{x_2^2 x_3^3 x_4^3 x_5^4 x_6^3 x_7^2 x_8^4 x_9^2 x_{10}^4 x_{11}^3 x_{12}^3}{x_1 x_2 x_3^3 x_4^3 x_5^4 x_6^3 x_7^2 x_8^4 x_9^2 x_{10}^4 x_{11}^3 x_{12}^3}$       | $-1 \cdot 59$<br>$-1 \cdot 3 \cdot 5^2$                            |
| (0, 8, 4, 0) | (1, 1, 1, 1, 1, 2, 1, 2, 1, 2, 1, 2) | 48  | $\frac{x_1 x_2^2 x_3^5 x_4^7 x_5^3 x_6^3 x_7^3 x_8^3 x_9^3 x_{10}^7 x_{11}^3 x_{12}^3}{x_1 x_2^3 x_3^4 x_4^7 x_5^3 x_6^3 x_7^3 x_8^3 x_9^3 x_{10}^7 x_{11}^3 x_{12}^3}$ | $-1 \cdot 5 \cdot 19$<br>$-1 \cdot 5 \cdot 59$                     |
| (0, 7, 4, 1) | (1, 2, 2, 1, 1, 3, 1, 1, 2, 2, 1, 1) | 42  | $x_2 x_3^3 x_4^2 x_5^6 x_7^6 x_8^3 x_9^3 x_{10}^6 x_{11}^6 x_{12}^6$                                                                                                    | $2 \cdot 3^3$                                                      |
| (0, 6, 4, 2) | (1, 2, 1, 2, 3, 2, 3, 1, 2, 1, 1, 1) | 36  | $\frac{x_3^5 x_4^3 x_5^3 x_6^3 x_7 x_8^5 x_9^3 x_{10}^5 x_{11}^5 x_{12}^5}{x_1 x_3^4 x_4^3 x_5^3 x_6^3 x_7 x_8^5 x_9^3 x_{10}^5 x_{11}^5 x_{12}^5}$                     | $3 \cdot 11$<br>$59$                                               |
| (0, 5, 4, 3) | (1, 2, 1, 1, 3, 2, 1, 2, 1, 2, 3, 3) | 34  | $\frac{x_3^3 x_4^4 x_5^2 x_6^3 x_7^4 x_8^3 x_9^4 x_{10}^3 x_{11}^2 x_{12}^2}{x_1 x_2^3 x_3^3 x_4^4 x_5^2 x_6^3 x_7^4 x_8^3 x_9^4 x_{10}^3 x_{11}^2 x_{12}^2}$           | $2 \cdot 5 \cdot 11$<br>$17 \cdot 19$                              |
| (0, 4, 4, 4) | (1, 2, 1, 2, 3, 3, 2, 3, 2, 3, 1, 1) | 32  | $\frac{x_2^2 x_3^3 x_4^3 x_5^3 x_6^3 x_7^3 x_8^3 x_9^3 x_{10}^3 x_{11}^3 x_{12}^3}{x_1 x_2 x_3^3 x_4^3 x_5^3 x_6^3 x_7^3 x_8^3 x_9^3 x_{10}^3 x_{11}^3 x_{12}^3}$       | $2 \cdot 5 \cdot 43$<br>$2^2 \cdot 113$                            |
| (0, 7, 5, 0) | (1, 1, 1, 1, 1, 1, 2, 2, 1, 2, 2, 2) | 46  | $x_1^2 x_2^2 x_3^4 x_4^6 x_5^6 x_7^4 x_8^4 x_9^6 x_{10}^4 x_{11}^4 x_{12}^4$                                                                                            | $2$                                                                |
| (0, 6, 5, 1) | (1, 1, 1, 2, 2, 1, 3, 2, 1, 2, 2, 1) | 40  | $x_1 x_2 x_3^3 x_4^4 x_5^4 x_6^4 x_8^5 x_9^4 x_{10}^4 x_{11}^4 x_{12}^5$                                                                                                | $5^2$                                                              |
| (0, 5, 5, 2) | (1, 1, 2, 3, 1, 1, 2, 3, 2, 2, 1, 2) | 36  | $\frac{x_1 x_2 x_3^4 x_4^4 x_5^4 x_6^4 x_7^4 x_8^4 x_9^4 x_{10}^4 x_{11}^4 x_{12}^4}{x_1 x_2^2 x_3^3 x_4^4 x_5^4 x_6^4 x_7^4 x_8^4 x_9^4 x_{10}^4 x_{11}^4 x_{12}^4}$   | $2 \cdot 5 \cdot 23$<br>$2^3 \cdot 29$                             |
| (0, 4, 5, 3) | (1, 2, 3, 2, 1, 2, 3, 2, 1, 2, 3, 1) | 34  | $\frac{x_2^3 x_3^2 x_4^4 x_5^3 x_6^2 x_7^4 x_8^3 x_9^4 x_{10}^2 x_{11}^3 x_{12}^3}{x_1 x_2^2 x_3^2 x_4^4 x_5^3 x_6^2 x_7^4 x_8^3 x_9^4 x_{10}^2 x_{11}^3 x_{12}^3}$     | $-1 \cdot 2 \cdot 3 \cdot 797$<br>$-1 \cdot 2 \cdot 5^2 \cdot 223$ |
| (0, 6, 6, 0) | (1, 2, 2, 2, 1, 2, 1, 2, 1, 2, 1, 1) | 45  | $\frac{x_1 x_2^3 x_3^3 x_4^4 x_5^4 x_7^5 x_8^5 x_9^5 x_{10}^5 x_{11}^5 x_{12}^5}{x_1^2 x_2^2 x_3^3 x_4^4 x_5^4 x_7^5 x_8^5 x_9^5 x_{10}^5 x_{11}^5 x_{12}^5}$           | $3 \cdot 79$<br>$131$                                              |
| (0, 5, 6, 1) | (2, 1, 2, 1, 1, 2, 3, 1, 2, 2, 1, 2) | 39  | $\frac{x_3^3 x_4^4 x_5^4 x_6^5 x_8^5 x_9^5 x_{10}^4 x_{11}^5 x_{12}^5}{x_2 x_3^2 x_4^4 x_5^4 x_6^5 x_8^5 x_9^5 x_{10}^4 x_{11}^5 x_{12}^5}$                             | $2 \cdot 97$<br>$11 \cdot 13$                                      |
| (0, 4, 6, 2) | (1, 2, 2, 2, 3, 2, 1, 2, 1, 2, 3, 1) | 37  | $\frac{x_2 x_3^5 x_4^5 x_5^5 x_6^3 x_7^5 x_8^3 x_9^5 x_{10}^3 x_{11}^3 x_{12}^3}{x_1 x_3^5 x_4^5 x_5^5 x_6^3 x_7^5 x_8^3 x_9^5 x_{10}^3 x_{11}^3 x_{12}^3}$             | $2^2 \cdot 3 \cdot 13$<br>$2 \cdot 3^2 \cdot 17$                   |
| (0, 3, 6, 3) | (2, 3, 1, 1, 2, 2, 2, 3, 2, 1, 2, 3) | 35  | $x_3^2 x_4^2 x_5^5 x_6^5 x_7^2 x_8^5 x_9^2 x_{10}^5 x_{11}^5 x_{12}^2$                                                                                                  | $-1 \cdot 2^4$                                                     |
| (0, 5, 7, 0) | (2, 1, 2, 2, 1, 1, 1, 2, 2, 2, 1, 2) | 46  | $\frac{x_1^2 x_3^4 x_4^6 x_5^4 x_6^4 x_7^4 x_9^6 x_{10}^6 x_{11}^4 x_{12}^6}{x_1^2 x_2^2 x_3^4 x_5^4 x_6^4 x_7^4 x_9^6 x_{10}^6 x_{11}^4 x_{12}^6}$                     | $7 \cdot 13$<br>$-1 \cdot 47$                                      |
| (0, 4, 7, 1) | (1, 2, 1, 2, 2, 2, 1, 2, 1, 2, 3, 2) | 42  | $x_1 x_2^2 x_3^4 x_4^5 x_6^6 x_7^6 x_8^3 x_9^6 x_{10}^6 x_{12}^6$                                                                                                       | $-1 \cdot 3^2$                                                     |
| (0, 3, 7, 2) | (1, 2, 3, 1, 2, 2, 2, 3, 2, 2, 2, 1) | 40  | $x_2^2 x_3 x_4^2 x_5^2 x_6^6 x_7^6 x_8^6 x_9^6 x_{10}^6 x_{11}^6 x_{12}^2$                                                                                              | $-1 \cdot 2 \cdot 3$                                               |
| (0, 4, 8, 0) | (1, 2, 2, 2, 2, 1, 2, 2, 2, 2, 1, 1) | 48  | $x_2 x_3^3 x_4^7 x_5^7 x_6^3 x_7^7 x_8^7 x_9^7 x_{10}^3 x_{11}^3 x_{12}^3$                                                                                              | $-1 \cdot 2^3$                                                     |
| (0, 3, 8, 1) | (1, 1, 2, 3, 2, 2, 2, 2, 1, 2, 2, 2) | 46  | $x_2^2 x_3^2 x_5^5 x_6^7 x_8^7 x_9^7 x_{10}^7 x_{11}^7 x_{12}^7$                                                                                                        | $2^2$                                                              |

$$S \subseteq \mathbb{Z}_p \times \mathbb{Z}_4 \setminus \{(0, 0)\}, |S| = 12$$

| $\lambda$     | $\mathbf{a}$                         | deg | monomial/s                                                                                                                                                                                                   | coefficient/s                           |
|---------------|--------------------------------------|-----|--------------------------------------------------------------------------------------------------------------------------------------------------------------------------------------------------------------|-----------------------------------------|
| (0, 2, 8, 2)  | (2, 1, 2, 2, 2, 2, 3, 2, 1, 3, 2, 2) | 44  | $x_3 x_4^5 x_5^7 x_6^7 x_7 x_8^7 x_9 x_{10} x_{11}^7 x_{12}^7$                                                                                                                                               | $-1 \cdot 2 \cdot 3$                    |
| (0, 3, 9, 0)  | (2, 1, 2, 2, 1, 2, 2, 2, 2, 1, 2, 2) | 54  | $x_1 x_3^3 x_4^6 x_5^2 x_6^8 x_8^8 x_9^8 x_{10}^2 x_{11}^8 x_{12}^8$                                                                                                                                         | $-1 \cdot 2^3 \cdot 3$                  |
| (0, 2, 9, 1)  | (2, 1, 2, 2, 2, 1, 2, 2, 2, 3, 2, 2) | 52  | $x_1 x_2 x_3^2 x_4^7 x_5^8 x_6^8 x_8^8 x_{11}^8 x_{12}^8$<br>$x_1 x_2 x_3^3 x_4^6 x_5^8 x_6^8 x_8^8 x_{11}^8 x_{12}^8$                                                                                       | 19<br>$2 \cdot 23$                      |
| (0, 2, 10, 0) | (2, 2, 2, 2, 2, 1, 2, 2, 2, 2, 2, 1) | 61  | $x_1^2 x_2^3 x_3^5 x_4^6 x_5^9 x_8^9 x_9^9 x_{10}^9 x_{11}^9 x_{12}$                                                                                                                                         | 1                                       |
| (0, 1, 10, 1) | (2, 2, 2, 3, 2, 2, 2, 2, 2, 1, 2, 2) | 59  | $x_1 x_2^4 x_3^4 x_5^9 x_6^9 x_8^9 x_9^9 x_{11}^9 x_{12}^9$                                                                                                                                                  | 5                                       |
| (0, 1, 11, 0) | (2, 2, 2, 2, 2, 2, 1, 2, 2, 2, 2, 2) | 70  | $x_1 x_2^3 x_3^4 x_4^8 x_6^8 x_7 x_8^9 x_9^9 x_{10}^9 x_{11}^9 x_{12}^9$                                                                                                                                     | 1                                       |
| (0, 0, 12, 0) | (2, 2, 2, 2, 2, 2, 2, 2, 2, 2, 2, 2) | 101 | $x_1^3 x_2^4 x_3^6 x_4^{11} x_5^{11} x_6^{11} x_8^{11} x_9^{11} x_{10}^{11} x_{11}^{11} x_{12}^{11}$<br>$x_1^3 x_2^4 x_3^7 x_4^{10} x_5^{11} x_6^{11} x_8^{11} x_9^{11} x_{10}^{11} x_{11}^{11} x_{12}^{11}$ | 30062393<br>$3^2 \cdot 431 \cdot 11489$ |

$$S \subseteq \mathbb{Z}_p \times \mathbb{Z}_2 \setminus \{(0, 0)\}, |S| = 13$$

| $\lambda$ | $\mathbf{a}$                               | deg | monomial/s                                                                                                                                                                                              | coefficient/s                                                                                                 |
|-----------|--------------------------------------------|-----|---------------------------------------------------------------------------------------------------------------------------------------------------------------------------------------------------------|---------------------------------------------------------------------------------------------------------------|
| (13, 0)   | (0, 0, 0, 0, 0, 0, 0, 0, 0, 0, 0, 0, 0, 0) | 155 |                                                                                                                                                                                                         |                                                                                                               |
| (12, 1)   | (0, 0, 0, 0, 0, 0, 1, 0, 0, 0, 0, 0, 0, 0) | 96  | $x_1 x_2^4 x_3^4 x_4^{10} x_5^{11} x_6^{11} x_8^{11} x_9^{11} x_{11}^{11} x_{12}^{11} x_{13}^{11}$<br>$x_1^2 x_2^4 x_3^4 x_4^9 x_5^{11} x_6^{11} x_8^{11} x_9^{11} x_{11}^{11} x_{12}^{11} x_{13}^{11}$ | $2^2 \cdot 19 \cdot 443$<br>$-1 \cdot 2^3 \cdot 14821$                                                        |
| (11, 2)   | (0, 0, 0, 0, 0, 1, 0, 0, 0, 0, 0, 0, 0, 1) | 86  | $x_1^4 x_2^5 x_3^6 x_4^{10} x_5^{10} x_6 x_7^{10} x_9^{10} x_{10}^{10} x_{11}^{10} x_{12}^{10}$<br>$x_1^5 x_2^5 x_3^5 x_4^{10} x_5^{10} x_6 x_7^{10} x_9^{10} x_{10}^{10} x_{11}^{10} x_{12}^{10}$      | $-1 \cdot 2 \cdot 3 \cdot 7 \cdot 9767$<br>$2 \cdot 13 \cdot 13469$                                           |
| (10, 3)   | (0, 0, 0, 0, 0, 1, 0, 0, 0, 0, 0, 0, 1, 1) | 80  | $x_2^4 x_3^7 x_4^9 x_5^9 x_6^9 x_7^9 x_8^9 x_9^9 x_{10}^9 x_{11}^9 x_{12}^2 x_{13}^2$<br>$x_2^5 x_3^6 x_4^9 x_5^9 x_6^9 x_7^9 x_8^9 x_9^9 x_{10}^9 x_{11}^9 x_{12}^2 x_{13}^2$                          | $-1 \cdot 2^3 \cdot 13 \cdot 41 \cdot 53$<br>$-1 \cdot 2 \cdot 5^2 \cdot 6899$                                |
| (9, 4)    | (0, 0, 0, 0, 1, 0, 0, 0, 0, 0, 0, 1, 1, 1) | 74  | $x_1^4 x_2^5 x_3^8 x_4^8 x_5^3 x_6^8 x_7^8 x_8^8 x_9^8 x_{10}^3 x_{12}^3 x_{13}^3$<br>$x_1^4 x_2^6 x_3^7 x_4^8 x_5^3 x_6^8 x_7^8 x_8^8 x_9^8 x_{10}^3 x_{12}^3 x_{13}^3$                                | $2 \cdot 5^2 \cdot 6899$<br>$2 \cdot 3^3 \cdot 79 \cdot 109$                                                  |
| (8, 5)    | (0, 0, 0, 0, 1, 0, 0, 0, 0, 0, 1, 1, 1, 1) | 72  | $x_1^4 x_2^6 x_3^7 x_4^7 x_5^4 x_6^7 x_7^7 x_8^7 x_9^4 x_{10}^4 x_{11}^4 x_{12}^4 x_{13}^4$<br>$x_1^5 x_2^5 x_3^7 x_4^7 x_5^4 x_6^7 x_7^7 x_8^7 x_9^4 x_{10}^4 x_{11}^4 x_{12}^4 x_{13}^4$              | $-1 \cdot 2 \cdot 67 \cdot 73517$<br>$2^2 \cdot 3 \cdot 61 \cdot 2621$                                        |
| (7, 6)    | (0, 0, 0, 1, 0, 0, 0, 0, 0, 1, 1, 1, 1, 1) | 70  | $x_1^4 x_2^6 x_3^6 x_4^5 x_5^6 x_6^6 x_7^6 x_8^5 x_9^5 x_{10}^5 x_{11}^5 x_{12}^5 x_{13}^5$<br>$x_1^5 x_2^5 x_3^6 x_4^5 x_5^6 x_6^6 x_7^6 x_8^5 x_9^5 x_{10}^5 x_{11}^5 x_{12}^5 x_{13}^5$              | $-1 \cdot 2^3 \cdot 3 \cdot 401 \cdot 7307$<br>$-1 \cdot 2^4 \cdot 3 \cdot 103 \cdot 6997$                    |
| (6, 7)    | (0, 0, 0, 1, 0, 0, 0, 1, 1, 1, 1, 1, 1, 1) | 72  | $x_1^5 x_2^5 x_3^5 x_4^5 x_5^5 x_6^5 x_7^6 x_8^6 x_9^6 x_{10}^6 x_{11}^6 x_{12}^6 x_{13}^6$<br>$x_1^5 x_2^5 x_3^5 x_4^5 x_5^5 x_6^5 x_7^6 x_8^6 x_9^6 x_{10}^6 x_{11}^6 x_{12}^6 x_{13}^6$              | $2^3 \cdot 5 \cdot 7 \cdot 13 \cdot 43 \cdot 113$<br>$-1 \cdot 2^2 \cdot 5^3 \cdot 31 \cdot 5774149$          |
| (5, 8)    | (0, 0, 1, 0, 1, 1, 0, 1, 1, 0, 1, 1, 1, 1) | 74  | $x_1^2 x_2^4 x_3^7 x_4^7 x_5^7 x_6^7 x_7^4 x_8^7 x_9^4 x_{10}^7 x_{11}^7 x_{12}^7 x_{13}^7$<br>$x_1^3 x_2^3 x_3^7 x_4^7 x_5^7 x_6^7 x_7^4 x_8^7 x_9^4 x_{10}^7 x_{11}^7 x_{12}^7 x_{13}^7$              | $2^3 \cdot 5 \cdot 13 \cdot 17 \cdot 1637 \cdot 3011$<br>$2^3 \cdot 7 \cdot 79 \cdot 103 \cdot 107 \cdot 733$ |
| (4, 9)    | (0, 0, 1, 0, 0, 1, 1, 1, 1, 1, 1, 1, 1, 1) | 80  | $x_2^3 x_3^7 x_4^3 x_5^8 x_6^8 x_7^8 x_8^8 x_9^8 x_{10}^8 x_{11}^8 x_{12}^8 x_{13}^8$<br>$x_1 x_2^3 x_3^7 x_4^3 x_5^8 x_6^8 x_7^8 x_8^8 x_9^8 x_{10}^8 x_{11}^8 x_{12}^8 x_{13}^8$                      | $2^5 \cdot 11 \cdot 92179$<br>$2^4 \cdot 7 \cdot 1056323$                                                     |
| (3, 10)   | (0, 1, 0, 0, 1, 1, 1, 1, 1, 1, 1, 1, 1, 1) | 86  | $x_1^2 x_2^3 x_3^2 x_4^2 x_5^9 x_6^9 x_7^9 x_8^9 x_9^9 x_{10}^9 x_{11}^9 x_{12}^9 x_{13}^9$<br>$x_1^2 x_2^3 x_3^2 x_4^2 x_5^9 x_6^9 x_7^9 x_8^9 x_9^9 x_{10}^9 x_{11}^9 x_{12}^9 x_{13}^9$              | $-1 \cdot 2^4 \cdot 3^3 \cdot 5 \cdot 107 \cdot 1399$<br>$2^4 \cdot 3 \cdot 5^2 \cdot 31^2 \cdot 313$         |

$$S \subseteq \mathbb{Z}_p \times \mathbb{Z}_2 \setminus \{(0, 0)\}, |S| = 13$$

| $\lambda$ | $\mathbf{a}$                            | deg | monomial/s                                                                                                                                                                                                                                                | coefficient/s                                                                       |
|-----------|-----------------------------------------|-----|-----------------------------------------------------------------------------------------------------------------------------------------------------------------------------------------------------------------------------------------------------------|-------------------------------------------------------------------------------------|
| (2, 11)   | (0, 1, 0, 1, 1, 1, 1, 1, 1, 1, 1, 1, 1) | 96  | $x_1 x_2^4 x_3 x_4^{10} x_5^{10} x_6^{10} x_7^{10} x_8^{10} x_9^{10} x_{10}^{10} x_{11}^{10} x_{12}^{10} x_{13}^{10}$<br>$x_1 x_2^5 x_3 x_4^9 x_5^{10} x_6^{10} x_7^{10} x_8^{10} x_9^{10} x_{10}^{10} x_{11}^{10} x_{12}^{10} x_{13}^{10}$               | $2^3 \cdot 108955667$<br>$23 \cdot 227 \cdot 390161$                                |
| (1, 12)   | (1, 0, 1, 1, 1, 1, 1, 1, 1, 1, 1, 1, 1) | 106 | $x_1^3 x_2^4 x_3^{11} x_4^{11} x_5^{11} x_6^{11} x_7^{11} x_8^{11} x_9^{11} x_{10}^{11} x_{11}^{11} x_{12}^{11} x_{13}^{11}$<br>$x_1^4 x_2^4 x_3^4 x_4^{10} x_5^{11} x_6^{11} x_7^{11} x_8^{11} x_9^{11} x_{10}^{11} x_{11}^{11} x_{12}^{11} x_{13}^{11}$ | $2 \cdot 3^2 \cdot 5^2 \cdot 47 \cdot 101 \cdot 463$<br>$2 \cdot 3 \cdot 530259889$ |
| (0, 13)   | (1, 1, 1, 1, 1, 1, 1, 1, 1, 1, 1, 1, 1) | 120 | $x_1^2 x_2^4 x_3^6 x_4^{12} x_5^{12} x_6^{12} x_7^{12} x_8^{12} x_9^{12} x_{10}^{12} x_{11}^{12} x_{12}^{12} x_{13}^{12}$<br>$x_1^2 x_2^5 x_3^5 x_4^{12} x_5^{12} x_6^{12} x_7^{12} x_8^{12} x_9^{12} x_{10}^{12} x_{11}^{12} x_{12}^{12} x_{13}^{12}$    | $2^2 \cdot 5 \cdot 17^2 \cdot 89 \cdot 2689$<br>$2 \cdot 3 \cdot 1151 \cdot 159161$ |

$$S \subseteq \mathbb{Z}_p \times \mathbb{Z}_3 \setminus \{(0, 0)\}, |S| = 13$$

| $\lambda$  | $\mathbf{a}$                            | deg | monomial/s                                                                                                                                                                                                                                        | coefficient/s                                                              |
|------------|-----------------------------------------|-----|---------------------------------------------------------------------------------------------------------------------------------------------------------------------------------------------------------------------------------------------------|----------------------------------------------------------------------------|
| (13, 0, 0) | (0, 0, 0, 0, 0, 0, 0, 0, 0, 0, 0, 0, 0) | 155 |                                                                                                                                                                                                                                                   |                                                                            |
| (12, 1, 0) | (0, 0, 0, 0, 0, 0, 1, 0, 0, 0, 0, 0, 0) | 96  | $x_1 x_2^4 x_3^4 x_4^{10} x_5^{11} x_6^{11} x_7^{11} x_8^{11} x_9^{11} x_{10}^{11} x_{11}^{11} x_{12}^{11} x_{13}^{11}$<br>$x_1^2 x_2^4 x_3^4 x_4^9 x_5^{11} x_6^{11} x_7^{11} x_8^{11} x_9^{11} x_{10}^{11} x_{11}^{11} x_{12}^{11} x_{13}^{11}$ | $2^2 \cdot 19 \cdot 443$<br>$-1 \cdot 2^3 \cdot 14821$                     |
| (11, 2, 0) | (0, 0, 0, 0, 1, 0, 0, 0, 0, 1, 0, 0, 0) | 71  | $x_1^2 x_2^4 x_3^5 x_4^6 x_5^9 x_6^{10} x_7^{10} x_8^{10} x_9^{10} x_{10}^{10} x_{11}^{10} x_{12}^{10} x_{13}^{10}$                                                                                                                               | 3                                                                          |
| (11, 1, 1) | (1, 0, 0, 0, 0, 0, 0, 2, 0, 0, 0, 0, 0) | 85  | $x_2^4 x_3^5 x_4^6 x_5^{10} x_6^{10} x_7^{10} x_8^{10} x_9^{10} x_{10}^{10} x_{11}^{10} x_{12}^{10} x_{13}^{10}$<br>$x_2^5 x_3^5 x_4^6 x_5^{10} x_6^{10} x_7^{10} x_8^{10} x_9^{10} x_{10}^{10} x_{11}^{10} x_{12}^{10} x_{13}^{10}$              | $2^2 \cdot 13 \cdot 1061$<br>$-1 \cdot 2^5 \cdot 3 \cdot 7 \cdot 131$      |
| (10, 3, 0) | (1, 0, 0, 0, 1, 0, 0, 0, 0, 1, 0, 0, 0) | 63  | $x_1^2 x_2^4 x_3^4 x_4 x_5 x_6^6 x_7^9 x_8^9 x_9^9 x_{10}^9 x_{11}^9 x_{12}^9 x_{13}^9$                                                                                                                                                           | $-1 \cdot 3$                                                               |
| (10, 2, 1) | (0, 0, 0, 1, 1, 0, 0, 0, 0, 2, 0, 0, 0) | 62  | $x_1 x_2^4 x_3^4 x_4 x_5 x_6^6 x_7^9 x_8^9 x_9^9 x_{10}^9 x_{11}^9 x_{12}^9 x_{13}^9$                                                                                                                                                             | 3                                                                          |
| (9, 4, 0)  | (1, 0, 0, 0, 1, 0, 0, 0, 1, 0, 0, 0, 1) | 59  | $x_1 x_2^4 x_3^4 x_4 x_5 x_6^7 x_7^8 x_8^8 x_9^8 x_{10}^8 x_{11}^8 x_{12}^8 x_{13}^8$                                                                                                                                                             | 5                                                                          |
| (9, 3, 1)  | (0, 1, 0, 0, 0, 0, 0, 0, 1, 0, 0, 2, 1) | 65  | $x_1^4 x_2^7 x_3^8 x_4^8 x_5^8 x_6^8 x_7^8 x_8^8 x_9^8 x_{10}^8 x_{11}^8 x_{12}^8 x_{13}^8$<br>$x_1^5 x_2^6 x_3^8 x_4^8 x_5^8 x_6^8 x_7^8 x_8^8 x_9^8 x_{10}^8 x_{11}^8 x_{12}^8 x_{13}^8$                                                        | $-1 \cdot 2^4 \cdot 31 \cdot 71$<br>$-1 \cdot 2 \cdot 5 \cdot 7 \cdot 709$ |
| (9, 2, 2)  | (0, 0, 0, 0, 1, 0, 0, 1, 0, 0, 0, 2, 2) | 55  | $x_1^4 x_2^4 x_3^6 x_4^6 x_5 x_6^8 x_7^8 x_8^8 x_9^8 x_{10}^8 x_{11}^8 x_{12}^8$                                                                                                                                                                  | $-1 \cdot 2 \cdot 3$                                                       |
| (8, 5, 0)  | (0, 0, 0, 1, 0, 1, 0, 0, 0, 1, 1, 0, 1) | 56  | $x_1^2 x_2^5 x_3^4 x_4^7 x_5^4 x_6^7 x_7^7 x_8^7 x_9^7 x_{10}^7 x_{11}^7 x_{12}^7$                                                                                                                                                                | $-1 \cdot 2^2 \cdot 3^2 \cdot 7$                                           |
| (8, 4, 1)  | (0, 0, 0, 1, 0, 0, 1, 0, 0, 0, 1, 1, 2) | 52  | $x_1^4 x_2^5 x_3^3 x_4^7 x_5^2 x_6^6 x_7^7 x_8^7 x_9^7 x_{10}^3 x_{11}^3 x_{12}^3$                                                                                                                                                                | $-1 \cdot 2^5$                                                             |
| (8, 3, 2)  | (0, 0, 0, 0, 1, 1, 0, 2, 0, 0, 1, 0, 2) | 50  | $x_1^3 x_2^4 x_3^7 x_4^7 x_5^2 x_6^7 x_7^8 x_8^7 x_9^7 x_{10}^2 x_{11}^2 x_{12}^2 x_{13}^2$<br>$x_1^4 x_2^3 x_3^7 x_4^7 x_5^2 x_6^7 x_7^8 x_8^7 x_9^7 x_{10}^2 x_{11}^2 x_{12}^2 x_{13}^2$                                                        | 47<br>$-1 \cdot 3 \cdot 5 \cdot 103$                                       |
| (7, 6, 0)  | (0, 1, 1, 0, 1, 1, 0, 0, 0, 1, 0, 0, 1) | 54  | $x_1^2 x_2^6 x_3^5 x_4^5 x_5^6 x_6^6 x_7^5 x_8^6 x_9^6 x_{10}^6 x_{11}^6 x_{12}^6 x_{13}^6$                                                                                                                                                       | $-1 \cdot 2^5 \cdot 3 \cdot 5^2$                                           |
| (7, 5, 1)  | (1, 0, 1, 0, 1, 0, 0, 1, 0, 1, 0, 0, 2) | 50  | $x_1 x_2 x_3^4 x_4^4 x_5^6 x_6^6 x_7^4 x_8^6 x_9^4 x_{10}^6 x_{11}^6 x_{12}^6$                                                                                                                                                                    | $2^2 \cdot 3 \cdot 5^2$                                                    |
| (7, 4, 2)  | (1, 0, 0, 2, 0, 1, 0, 1, 0, 0, 1, 0, 2) | 47  | $x_3^6 x_4^6 x_5^3 x_6^6 x_7^3 x_8^6 x_9^6 x_{10}^3 x_{11}^6 x_{12}^6 x_{13}^6$<br>$x_2 x_3^5 x_4^6 x_5^6 x_6^6 x_7^3 x_8^6 x_9^6 x_{10}^3 x_{11}^6 x_{12}^6 x_{13}^6$                                                                            | $2^3 \cdot 13$<br>$2^2 \cdot 79$                                           |
| (7, 3, 3)  | (1, 0, 0, 1, 1, 2, 0, 0, 0, 2, 2, 0, 0) | 45  | $x_3^5 x_4^2 x_5^2 x_6^6 x_7^6 x_8^6 x_9^2 x_{10}^2 x_{11}^6 x_{12}^6 x_{13}^6$                                                                                                                                                                   | $-1 \cdot 2^3 \cdot 3^3$                                                   |
| (6, 7, 0)  | (0, 0, 1, 1, 0, 1, 1, 0, 0, 1, 0, 1, 1) | 56  | $x_1 x_2^2 x_3^4 x_4^6 x_5^6 x_6^6 x_7^5 x_8^5 x_9^5 x_{10}^5 x_{11}^6 x_{13}^6$<br>$x_1^2 x_2^3 x_3^3 x_4^5 x_5^6 x_6^6 x_7^5 x_8^5 x_9^5 x_{10}^5 x_{11}^6 x_{13}^6$                                                                            | $-1 \cdot 7 \cdot 17 \cdot 163$<br>$-1 \cdot 2 \cdot 28927$                |

$$S \subseteq \mathbb{Z}_p \times \mathbb{Z}_3 \setminus \{(0, 0)\}, |S| = 13$$

| $\lambda$  | $\mathbf{a}$                                                                       | deg      | monomial/s                                                                                                                                                                                 | coefficient/s                                               |
|------------|------------------------------------------------------------------------------------|----------|--------------------------------------------------------------------------------------------------------------------------------------------------------------------------------------------|-------------------------------------------------------------|
| (6, 6, 1)  | (0, 0, 0, 1, 0, 1, 1, 1, 1, 0, 2, 1, 0)                                            | 50       | $x_2^3 x_3^3 x_4^4 x_5^5 x_6^5 x_7^5 x_8^5 x_9^5 x_{10}^5 x_{12}^5 x_{13}^5$<br>$x_1 x_2^3 x_3^3 x_4^3 x_5^5 x_6^5 x_7^5 x_8^5 x_9^5 x_{10}^5 x_{12}^5 x_{13}^5$                           | $2 \cdot 13 \cdot 61$<br>$2 \cdot 3 \cdot 163$              |
| (6, 5, 2)  | (0, 0, 0, 1, 0, 1, 0, 0, 1, 1, 1, 2, 2)                                            | 46       | $x_1 x_2^3 x_3^5 x_4^4 x_5^5 x_6^4 x_7^5 x_8^5 x_9^4 x_{10}^4 x_{11}^4 x_{12} x_{13}$                                                                                                      | $-1 \cdot 2 \cdot 3 \cdot 5$                                |
| (6, 4, 3)  | (0, 0, 0, 0, 1, 0, 1, 0, 2, 1, 2, 1, 2)                                            | 44       | $x_1 x_2^5 x_3^5 x_4^5 x_5^3 x_6^5 x_7^3 x_8^5 x_9^2 x_{10}^2 x_{11}^3 x_{12}^2 x_{13}^2$<br>$x_1^2 x_2^4 x_3^5 x_4^3 x_5^5 x_6^3 x_7^3 x_8^5 x_9^2 x_{10}^2 x_{11}^3 x_{12}^2 x_{13}^2$   | $2^2 \cdot 3^2 \cdot 83$<br>$3 \cdot 1021$                  |
| (5, 8, 0)  | (0, 0, 1, 0, 1, 0, 0, 1, 1, 1, 1, 1, 1)                                            | 59       | $x_2^2 x_3^4 x_4^7 x_5^4 x_6^4 x_7^7 x_8^7 x_9^7 x_{10}^7 x_{11}^7 x_{12}^7 x_{13}^7$<br>$x_1 x_2^2 x_3^4 x_4^7 x_5^4 x_6^4 x_7^7 x_8^7 x_9^7 x_{10}^7 x_{11}^7 x_{12}^7 x_{13}^7$         | $-1 \cdot 2 \cdot 11 \cdot 17$<br>$2^5 \cdot 59$            |
| (5, 7, 1)  | (0, 0, 1, 0, 0, 1, 0, 1, 1, 1, 2, 1, 1)                                            | 51       | $x_1 x_2^4 x_4^4 x_5^6 x_6^4 x_7^6 x_8^6 x_9^6 x_{10}^6 x_{12}^6 x_{13}^6$                                                                                                                 | 3                                                           |
| (5, 6, 2)  | (0, 0, 0, 1, 0, 1, 0, 1, 1, 1, 2, 1, 2)                                            | 47       | $x_1^2 x_2 x_3^4 x_4^5 x_5^4 x_6^5 x_7^4 x_8^5 x_9^5 x_{10}^5 x_{11} x_{12}^5 x_{13}$<br>$x_1 x_2^4 x_3^3 x_4^5 x_5^4 x_6^5 x_7^4 x_8^5 x_9^5 x_{10}^5 x_{11} x_{12}^5$                    | $3 \cdot 7^4$<br>$2^4 \cdot 13^2$                           |
| (5, 5, 3)  | (0, 0, 0, 0, 1, 0, 1, 2, 1, 2, 1, 2, 1)                                            | 44       | $x_1^3 x_2^4 x_3^4 x_4^4 x_5^4 x_6^4 x_7^4 x_8^4 x_9^2 x_{10}^4 x_{11}^2 x_{12}^4 x_{13}^4$                                                                                                | $-1 \cdot 2^4$                                              |
| (5, 4, 4)  | (0, 0, 0, 0, 1, 1, 0, 2, 1, 2, 1, 2, 2)                                            | 43       | $x_1^4 x_2^4 x_3^4 x_4^2 x_5^3 x_6^4 x_7^3 x_8^3 x_9^3 x_{10}^3 x_{11}^3 x_{12}^3 x_{13}^3$                                                                                                | $-1 \cdot 2^6$                                              |
| (4, 9, 0)  | (0, 1, 0, 0, 1, 0, 1, 1, 1, 1, 1, 1, 1)                                            | 63       | $x_1^2 x_2^3 x_3^3 x_4^4 x_5^3 x_6^5 x_7^8 x_8^8 x_9^8 x_{10}^8 x_{11}^8 x_{12}^8 x_{13}^8$<br>$x_1^2 x_2^3 x_3^3 x_4^4 x_5^3 x_6^6 x_7^8 x_8^8 x_9^8 x_{10}^8 x_{11}^8 x_{12}^8 x_{13}^8$ | $-1 \cdot 2 \cdot 7^2 \cdot 19$<br>$-1 \cdot 2^3 \cdot 743$ |
| (4, 8, 1)  | (0, 0, 1, 0, 1, 0, 1, 1, 1, 1, 1, 1, 2)                                            | 56       | $x_2^3 x_3^5 x_4^3 x_6^7 x_7^7 x_8^7 x_9^7 x_{10}^7 x_{11}^7 x_{12}^7$<br>$x_1 x_2^3 x_3^3 x_4^3 x_6^7 x_7^7 x_8^7 x_9^7 x_{10}^7 x_{11}^7 x_{12}^7$                                       | $2^2 \cdot 3 \cdot 7 \cdot 29$<br>$2^3 \cdot 271$           |
| (4, 7, 2)  | (0, 0, 1, 0, 1, 0, 1, 1, 1, 2, 1, 1, 2)                                            | 50       | $x_1^3 x_2^3 x_3^6 x_4^3 x_5^6 x_6^3 x_8^6 x_9^6 x_{10}^6 x_{11}^6 x_{12}^6 x_{13}$<br>$x_1^3 x_2^3 x_3^6 x_4^3 x_5^6 x_6^3 x_7^6 x_8^6 x_9^6 x_{10}^6 x_{11}^6 x_{12}^6 x_{13}$           | $2^2 \cdot 7 \cdot 29$<br>$-1 \cdot 5 \cdot 383$            |
| (4, 6, 3)  | (0, 0, 0, 1, 1, 0, 1, 1, 1, 2, 1, 2, 2)                                            | 46       | $x_1^3 x_2^3 x_3^3 x_4^4 x_5^4 x_6^3 x_7^5 x_8^5 x_9^5 x_{10}^2 x_{11}^5 x_{12}^2 x_{13}^2$<br>$x_1^3 x_2^3 x_3^3 x_4^5 x_5^2 x_6^2 x_7^5 x_8^5 x_9^5 x_{11}^5 x_{12}^2 x_{13}^2$          | $-1 \cdot 5^2 \cdot 13$<br>$-1 \cdot 2^3 \cdot 11$          |
| (4, 5, 4)  | (0, 0, 2, 0, 1, 1, 0, 1, 2, 1, 2, 1, 2)<br>(0, 0, 2, 0, 1, 0, 1, 1, 2, 1, 2, 1, 2) | 44<br>44 | $x_1^3 x_2^3 x_3^3 x_4^4 x_5^4 x_6^3 x_7^4 x_8^3 x_9^4 x_{10}^3 x_{11}^4 x_{12}^3 x_{13}^3$<br>$x_1^3 x_2^3 x_3^3 x_4^4 x_5^4 x_6^3 x_7^4 x_8^3 x_9^4 x_{10}^3 x_{11}^4 x_{12}^3 x_{13}^3$ | $2 \cdot 3 \cdot 9833$<br>$2^3 \cdot 3 \cdot 13 \cdot 197$  |
| (3, 10, 0) | (0, 1, 0, 1, 0, 1, 1, 1, 1, 1, 1, 1, 1)                                            | 71       | $x_1^2 x_2^4 x_3^4 x_4^2 x_5^6 x_6^6 x_7^9 x_8^9 x_9^9 x_{10}^9 x_{11}^9 x_{12}^9 x_{13}^9$<br>$x_1^2 x_2^4 x_3^4 x_4^2 x_5^6 x_6^6 x_7^9 x_8^9 x_9^9 x_{10}^9 x_{11}^9 x_{12}^9 x_{13}^9$ | 9733<br>11 · 5189                                           |
| (3, 9, 1)  | (0, 0, 1, 0, 1, 1, 1, 1, 1, 1, 1, 2, 1)                                            | 62       | $x_1^2 x_2^4 x_3^4 x_4^2 x_5^8 x_6^8 x_7^8 x_8^8 x_{10}^8 x_{11}^8 x_{13}^8$<br>$x_1^2 x_2^4 x_3^4 x_5^8 x_6^8 x_7^8 x_8^8 x_{10}^8 x_{11}^8 x_{13}^8$                                     | $2 \cdot 3 \cdot 11^2 \cdot 13$<br>$-1 \cdot 3 \cdot 3331$  |
| (3, 8, 2)  | (0, 0, 1, 0, 1, 1, 1, 1, 2, 1, 2, 1, 1)                                            | 54       | $x_1^2 x_2^2 x_3^7 x_4^2 x_5^5 x_6^6 x_7^9 x_{10}^7 x_{11}^7 x_{12}^7 x_{13}^7$<br>$x_1^2 x_2^2 x_3^7 x_4^2 x_5^6 x_6^6 x_7^9 x_{10}^7 x_{11}^7 x_{12}^7 x_{13}^7$                         | $2 \cdot 337$<br>$-1 \cdot 2 \cdot 3 \cdot 17$              |
| (3, 7, 3)  | (0, 0, 1, 0, 1, 1, 1, 1, 2, 1, 2, 1, 2)                                            | 51       | $x_1^2 x_2^2 x_3^3 x_4^2 x_5^6 x_6^6 x_7^6 x_8^2 x_9^6 x_{10}^2 x_{11}^6 x_{12}^2 x_{13}^2$<br>$x_1^2 x_2^2 x_3^4 x_4^2 x_5^6 x_6^6 x_7^6 x_8^2 x_9^6 x_{10}^2 x_{11}^6 x_{12}^2 x_{13}^2$ | $2 \cdot 11 \cdot 17^2$<br>$2^3 \cdot 1301$                 |
| (3, 6, 4)  | (0, 0, 1, 0, 1, 2, 1, 2, 1, 2, 1, 1, 2)                                            | 47       | $x_1^2 x_2^2 x_3^4 x_4^2 x_5^5 x_6^3 x_7^5 x_8^3 x_9^5 x_{10}^3 x_{11}^5 x_{12}^3 x_{13}^3$<br>$x_1^2 x_2^2 x_3^5 x_4^2 x_5^5 x_6^3 x_7^5 x_8^3 x_9^5 x_{10}^3 x_{11}^5 x_{12}^3 x_{13}^3$ | $5 \cdot 17 \cdot 71$<br>$2 \cdot 6067$                     |

$$S \subseteq \mathbb{Z}_p \times \mathbb{Z}_3 \setminus \{(0, 0)\}, |S| = 13$$

| $\lambda$  | $\mathbf{a}$                            | deg | monomial/s                                                                                                                                                                                                               | coefficient/s                                                               |
|------------|-----------------------------------------|-----|--------------------------------------------------------------------------------------------------------------------------------------------------------------------------------------------------------------------------|-----------------------------------------------------------------------------|
| (3, 5, 5)  | (0, 0, 1, 0, 1, 1, 2, 2, 1, 2, 1, 2, 2) | 45  | $x_1^2 x_2^2 x_3^3 x_4^2 x_5^4 x_6^4 x_7^4 x_8^4 x_9^4 x_{10}^4 x_{11}^4 x_{12}^4 x_{13}^4$<br>$x_1^2 x_2^2 x_3^4 x_4^2 x_5^3 x_6^4 x_7^4 x_8^4 x_9^4 x_{10}^4 x_{11}^4 x_{12}^4 x_{13}^4$                               | $2 \cdot 7 \cdot 23$<br>$-1 \cdot 2 \cdot 3 \cdot 5 \cdot 29$               |
| (2, 11, 0) | (0, 1, 0, 1, 1, 1, 1, 1, 1, 1, 1, 1, 1) | 80  | $x_1 x_2^3 x_3 x_4^3 x_5^6 x_6^6 x_7^{10} x_8^{10} x_{10}^{10} x_{11}^{10} x_{12}^{10} x_{13}^{10}$<br>$x_1 x_2^3 x_3 x_4^3 x_5^6 x_6^7 x_7^9 x_8^{10} x_{10}^{10} x_{11}^{10} x_{12}^{10} x_{13}^{10}$                  | $-1 \cdot 2^6 \cdot 3 \cdot 173$<br>$-1 \cdot 3 \cdot 19 \cdot 31 \cdot 53$ |
| (2, 10, 1) | (0, 1, 0, 1, 1, 1, 1, 1, 1, 1, 2, 1, 1) | 69  | $x_1 x_2^4 x_3 x_4^6 x_5^6 x_6^6 x_7^9 x_8^9 x_{10}^9 x_{12}^9 x_{13}^9$<br>$x_1 x_2^4 x_3 x_4^5 x_5^6 x_6^6 x_7^9 x_8^9 x_{10}^9 x_{12}^9 x_{13}^9$                                                                     | $2^2 \cdot 5 \cdot 349$<br>$2^3 \cdot 3 \cdot 11 \cdot 47$                  |
| (2, 9, 2)  | (0, 1, 0, 1, 1, 1, 1, 1, 1, 1, 2, 1, 2) | 63  | $x_1 x_2^5 x_3 x_4^6 x_5^8 x_6^8 x_7^8 x_8^8 x_{10}^8 x_{11}^8 x_{12}^8 x_{13}^8$<br>$x_1 x_2^5 x_3 x_4^7 x_5^7 x_6^8 x_7^8 x_8^8 x_{10}^8 x_{11}^8 x_{12}^8 x_{13}^8$                                                   | $-1 \cdot 3 \cdot 43 \cdot 349$<br>$-1 \cdot 2^3 \cdot 3 \cdot 5 \cdot 251$ |
| (2, 8, 3)  | (2, 0, 1, 1, 1, 1, 1, 0, 1, 2, 1, 1, 2) | 57  | $x_1^2 x_2 x_3^3 x_4^4 x_5^7 x_6^7 x_7^7 x_8^7 x_{10}^2 x_{11}^7 x_{12}^7 x_{13}^2$<br>$x_1^2 x_2 x_3^3 x_4^5 x_5^6 x_6^7 x_7^8 x_8^7 x_{10}^2 x_{11}^7 x_{12}^7 x_{13}^2$                                               | $11 \cdot 269$<br>$2 \cdot 3 \cdot 307$                                     |
| (2, 7, 4)  | (0, 1, 0, 1, 1, 1, 1, 1, 2, 2, 1, 2, 2) | 51  | $x_1 x_2^3 x_3 x_4^4 x_5^6 x_6^6 x_7^6 x_8^6 x_{10}^3 x_{11}^3 x_{12}^3 x_{13}^3$<br>$x_1 x_2^3 x_3 x_4^5 x_5^5 x_6^6 x_7^6 x_8^6 x_{10}^3 x_{11}^3 x_{12}^3 x_{13}^3$                                                   | $2^3 \cdot 3^2 \cdot 43$<br>$-1 \cdot 1061$                                 |
| (2, 6, 5)  | (0, 1, 0, 1, 1, 1, 1, 2, 1, 2, 2, 2, 2) | 51  | $x_1^5 x_2 x_3^5 x_4^5 x_5^5 x_6^5 x_7^4 x_8^5 x_{10}^4 x_{11}^4 x_{12}^4 x_{13}^4$<br>$x_1 x_2^4 x_3 x_4^5 x_5^5 x_6^5 x_7^5 x_8^4 x_{10}^4 x_{11}^4 x_{12}^4 x_{13}^4$                                                 | $2 \cdot 3 \cdot 23 \cdot 101$<br>$19 \cdot 1033$                           |
| (1, 12, 0) | (1, 0, 1, 1, 1, 1, 1, 1, 1, 1, 1, 1, 1) | 90  | $x_1^3 x_2^4 x_3^6 x_4^6 x_5^7 x_6^9 x_7^{11} x_8^{11} x_{10}^{11} x_{11}^{11} x_{12}^{11} x_{13}^{11}$<br>$x_1^3 x_2^5 x_3^5 x_4^6 x_5^7 x_6^9 x_7^{11} x_8^{11} x_{10}^{11} x_{11}^{11} x_{12}^{11} x_{13}^{11}$       | $5 \cdot 11^2 \cdot 17$<br>$-1 \cdot 32057$                                 |
| (1, 11, 1) | (0, 1, 1, 1, 1, 1, 1, 1, 1, 2, 1, 1, 1) | 80  | $x_2^5 x_3^5 x_4^5 x_5^{10} x_6^{10} x_7^{10} x_8^{10} x_{10}^{10} x_{11}^{10} x_{12}^{10} x_{13}^{10}$<br>$x_2^4 x_3^5 x_4^5 x_5^6 x_6^{10} x_7^{10} x_8^{10} x_{10}^{10} x_{11}^{10} x_{12}^{10} x_{13}^{10}$          | $2 \cdot 673$<br>$-1 \cdot 2^2 \cdot 17 \cdot 59$                           |
| (1, 10, 2) | (0, 1, 1, 2, 2, 1, 1, 1, 1, 1, 1, 1, 1) | 71  | $x_2^4 x_3^4 x_4 x_5 x_6^7 x_7^9 x_8^9 x_{10}^9 x_{11}^9 x_{12}^9 x_{13}^9$<br>$x_2^4 x_3^5 x_4 x_5 x_6^6 x_7^9 x_8^9 x_{10}^9 x_{11}^9 x_{12}^9 x_{13}^9$                                                               | $2^2 \cdot 13 \cdot 37$<br>$2^4 \cdot 3^3 \cdot 29$                         |
| (1, 9, 3)  | (1, 1, 2, 2, 1, 1, 0, 1, 1, 2, 1, 1, 1) | 63  | $x_1^3 x_2^6 x_3^2 x_4^8 x_5^8 x_6^8 x_7^2 x_{10}^8 x_{11}^8 x_{12}^8 x_{13}^8$<br>$x_1^4 x_2^5 x_3^2 x_4^8 x_5^8 x_6^8 x_7^2 x_{10}^8 x_{11}^8 x_{12}^8 x_{13}^8$                                                       | $2^2 \cdot 3^4 \cdot 7 \cdot 43$<br>$-1 \cdot 2 \cdot 3^3 \cdot 139$        |
| (1, 8, 4)  | (1, 1, 2, 2, 1, 1, 0, 1, 1, 2, 2, 1, 1) | 59  | $x_1^5 x_2^7 x_3^3 x_4^7 x_5^7 x_6^7 x_7^3 x_{10}^3 x_{11}^7 x_{12}^7 x_{13}^7$                                                                                                                                          | $2^5 \cdot 3^3 \cdot 5^2 \cdot 7$                                           |
| (1, 7, 5)  | (1, 1, 2, 2, 1, 1, 0, 1, 1, 2, 2, 1, 2) | 56  | $x_1^3 x_2^3 x_3^4 x_4^4 x_5^6 x_6^6 x_7^6 x_8^4 x_{10}^4 x_{11}^6 x_{12}^4 x_{13}^4$<br>$x_1^2 x_2^4 x_3^4 x_4^6 x_5^6 x_6^6 x_7^6 x_8^4 x_{10}^4 x_{11}^6 x_{12}^4 x_{13}^4$                                           | $7 \cdot 11 \cdot 307$<br>$5 \cdot 101477$                                  |
| (1, 6, 6)  | (1, 1, 2, 2, 1, 1, 0, 2, 1, 2, 2, 1, 2) | 55  | $x_1^2 x_2^3 x_3^5 x_4^5 x_5^5 x_6^5 x_7^5 x_8^5 x_{10}^5 x_{11}^5 x_{12}^5 x_{13}^5$<br>$x_1^3 x_2^2 x_3^5 x_4^5 x_5^5 x_6^5 x_7^5 x_8^5 x_{10}^5 x_{11}^5 x_{12}^5 x_{13}^5$                                           | $-1 \cdot 3 \cdot 424493$<br>$-1 \cdot 965317$                              |
| (0, 13, 0) | (1, 1, 1, 1, 1, 1, 1, 1, 1, 1, 1, 1, 1) | 104 | $x_1^2 x_2^4 x_3^6 x_4^6 x_5^6 x_6^8 x_7^{12} x_8^{12} x_{10}^{12} x_{11}^{12} x_{12}^{12} x_{13}^{12}$<br>$x_1^2 x_2^5 x_3^6 x_4^6 x_5^6 x_6^8 x_7^{12} x_8^{12} x_{10}^{12} x_{11}^{12} x_{12}^{12} x_{13}^{12}$       | $2 \cdot 3 \cdot 5 \cdot 29^2$<br>$5 \cdot 1789$                            |
| (0, 12, 1) | (1, 1, 2, 1, 1, 1, 1, 1, 1, 1, 1, 1, 1) | 92  | $x_1^3 x_2^4 x_3^5 x_4^6 x_5^8 x_6^{11} x_7^{11} x_8^{11} x_{10}^{11} x_{11}^{11} x_{12}^{11} x_{13}^{11}$<br>$x_1^4 x_2^5 x_3^5 x_4^6 x_5^8 x_6^{11} x_7^{11} x_8^{11} x_{10}^{11} x_{11}^{11} x_{12}^{11} x_{13}^{11}$ | $2^2 \cdot 3167$<br>$-1 \cdot 3 \cdot 67 \cdot 181$                         |
| (0, 11, 2) | (1, 1, 2, 2, 1, 1, 1, 1, 1, 1, 1, 1, 1) | 81  | $x_1^4 x_2^5 x_3 x_4 x_5^5 x_6^{10} x_7^{10} x_8^{10} x_{10}^{10} x_{11}^{10} x_{12}^{10} x_{13}^{10}$<br>$x_1^5 x_2^3 x_3 x_4 x_5^5 x_6^{10} x_7^{10} x_8^{10} x_{10}^{10} x_{11}^{10} x_{12}^{10} x_{13}^{10}$         | $2^2 \cdot 8963$<br>$-1 \cdot 2 \cdot 18119$                                |
| (0, 10, 3) | (1, 1, 2, 2, 1, 1, 2, 1, 1, 1, 1, 1, 1) | 75  | $x_1^4 x_2^5 x_3^2 x_4^6 x_5^9 x_6^9 x_7^9 x_8^9 x_{10}^9 x_{11}^9 x_{12}^9 x_{13}^9$<br>$x_1^5 x_2^3 x_3^2 x_4^6 x_5^9 x_6^9 x_7^9 x_8^9 x_{10}^9 x_{11}^9 x_{12}^9 x_{13}^9$                                           | $3 \cdot 19037$<br>$-1 \cdot 2 \cdot 3^3 \cdot 29 \cdot 73$                 |

$$S \subseteq \mathbb{Z}_p \times \mathbb{Z}_3 \setminus \{(0, 0)\}, |S| = 13$$

| $\lambda$ | $\mathbf{a}$                            | deg | monomial/s                                                                                                                                                                     | coefficient/s                                              |
|-----------|-----------------------------------------|-----|--------------------------------------------------------------------------------------------------------------------------------------------------------------------------------|------------------------------------------------------------|
| (0, 9, 4) | (1, 1, 2, 2, 1, 1, 2, 2, 1, 1, 1, 1, 1) | 69  | $x_1^4 x_2^5 x_3^3 x_4^8 x_5^8 x_6^3 x_7^3 x_8^8 x_{10}^8 x_{11}^8 x_{12}^8 x_{13}^8$<br>$x_1^5 x_2^4 x_3^3 x_4^8 x_5^8 x_6^3 x_7^3 x_8^8 x_{10}^8 x_{11}^8 x_{12}^8 x_{13}^8$ | $-1 \cdot 2 \cdot 134153$<br>$2^3 \cdot 47629$             |
| (0, 8, 5) | (1, 1, 2, 2, 1, 1, 2, 2, 1, 1, 2, 1, 1) | 64  | $x_1^4 x_2^5 x_3^4 x_4^7 x_5^7 x_6^4 x_7^4 x_8^7 x_{10}^4 x_{11}^7 x_{12}^7 x_{13}^7$<br>$x_1^5 x_2^4 x_3^4 x_4^7 x_5^7 x_6^4 x_7^4 x_8^7 x_{10}^4 x_{11}^7 x_{12}^7 x_{13}^7$ | $2^4 \cdot 130021$<br>$-1 \cdot 3 \cdot 13 \cdot 8669$     |
| (0, 7, 6) | (1, 1, 2, 2, 1, 1, 2, 2, 1, 1, 2, 2, 1) | 66  | $x_1^3 x_2^3 x_3^5 x_4^6 x_5^6 x_6^5 x_7^5 x_8^6 x_{10}^6 x_{11}^5 x_{12}^6 x_{13}^6$<br>$x_1^2 x_2^5 x_3^5 x_4^6 x_5^6 x_6^5 x_7^5 x_8^6 x_{10}^6 x_{11}^5 x_{12}^6 x_{13}^6$ | $2 \cdot 3 \cdot 491 \cdot 35089$<br>$2^2 \cdot 106231523$ |

$$S \subseteq \mathbb{Z}_p \times \mathbb{Z}_2 \setminus \{(0, 0)\}, |S| = 14$$

| $\lambda$ | $\mathbf{a}$                                     | deg | monomial/s                                                                                                                                                                                                                                                               | coefficient/s                                                                                                                |
|-----------|--------------------------------------------------|-----|--------------------------------------------------------------------------------------------------------------------------------------------------------------------------------------------------------------------------------------------------------------------------|------------------------------------------------------------------------------------------------------------------------------|
| (14, 0)   | (0, 0, 0, 0, 0, 0, 0, 0, 0, 0, 0, 0, 0, 0)       | 181 |                                                                                                                                                                                                                                                                          |                                                                                                                              |
| (13, 1)   | (0, 0, 0, 0, 0, 0, 0, 1, 0, 0, 0, 0, 0, 0)       | 114 | $x_1 x_2^4 x_3^4 x_4^9 x_5^{12} x_6^{12} x_7^{12} x_8^{12} x_{10}^{12} x_{12}^{12} x_{13}^{12} x_{14}^{12}$<br>$x_1 x_2^4 x_3^5 x_4^8 x_5^2 x_6^{12} x_7^{12} x_8^{12} x_{10}^{12} x_{12}^{12} x_{13}^{12} x_{14}^{12}$                                                  | $-1 \cdot 2^2 \cdot 645329$<br>$-1 \cdot 2^5 \cdot 5^2 \cdot 23 \cdot 757$                                                   |
| (12, 2)   | (0, 0, 0, 0, 0, 0, 1, 0, 0, 0, 0, 0, 0, 1)       | 103 | $x_1^4 x_2^5 x_3^6 x_4^{10} x_5^{11} x_6^{11} x_7 x_8^{11} x_{10}^{11} x_{11}^{11} x_{12}^{11} x_{13}^{11}$<br>$x_1^4 x_2^6 x_3^5 x_4^{10} x_5^{11} x_6^{11} x_7 x_8^{11} x_{10}^{11} x_{11}^{11} x_{12}^{11} x_{13}^{11}$                                               | $-1 \cdot 2 \cdot 7 \cdot 974989$<br>$2^7 \cdot 3 \cdot 240893$                                                              |
| (11, 3)   | (0, 0, 0, 0, 0, 0, 1, 0, 0, 0, 0, 0, 0, 1, 1)    | 96  | $x_1^4 x_2^7 x_3^9 x_4^{10} x_5^{10} x_6^2 x_7^{10} x_8^{10} x_{10}^{10} x_{11}^{10} x_{12}^{10} x_{13}^2 x_{14}^2$<br>$x_1^4 x_2^8 x_3^8 x_4^{10} x_5^{10} x_6^2 x_7^{10} x_8^{10} x_{10}^{10} x_{11}^{10} x_{12}^{10} x_{13}^2 x_{14}^2$                               | $2 \cdot 47 \cdot 291887$<br>$2^5 \cdot 5 \cdot 7 \cdot 13 \cdot 1609$                                                       |
| (10, 4)   | (0, 0, 0, 0, 0, 1, 0, 0, 0, 0, 0, 0, 1, 1, 1)    | 89  | $x_1^4 x_2^4 x_3^6 x_4^9 x_5^9 x_6^3 x_7^9 x_8^9 x_9^9 x_{10}^9 x_{11}^3 x_{12}^3 x_{13}^3 x_{14}^3$<br>$x_1^3 x_2^5 x_3^6 x_4^9 x_5^9 x_6^3 x_7^9 x_8^9 x_9^9 x_{10}^9 x_{11}^3 x_{12}^3 x_{13}^3 x_{14}^3$                                                             | $2^5 \cdot 2155159$<br>$2^4 \cdot 683 \cdot 26921$                                                                           |
| (9, 5)    | (0, 0, 0, 0, 0, 1, 0, 0, 0, 0, 0, 1, 1, 1, 1)    | 86  | $x_1^4 x_2^6 x_3^8 x_4^8 x_5^4 x_6^8 x_7^8 x_8^8 x_9^8 x_{10}^4 x_{11}^4 x_{12}^4 x_{13}^4 x_{14}^4$<br>$x_1^5 x_2^5 x_3^8 x_4^8 x_5^4 x_6^8 x_7^8 x_8^8 x_9^8 x_{10}^4 x_{11}^4 x_{12}^4 x_{13}^4 x_{14}^4$                                                             | $2 \cdot 547 \cdot 978973$<br>$2 \cdot 124623043$                                                                            |
| (8, 6)    | (0, 0, 0, 0, 1, 1, 1, 0, 0, 0, 0, 1, 1, 1, 1)    | 83  | $x_1^4 x_2^7 x_3^7 x_4^5 x_5^5 x_6^5 x_7^7 x_8^7 x_9^7 x_{10}^7 x_{11}^5 x_{12}^5 x_{13}^5 x_{14}^5$<br>$x_1^5 x_2^6 x_3^7 x_4^5 x_5^5 x_6^5 x_7^7 x_8^7 x_9^7 x_{10}^7 x_{11}^5 x_{12}^5 x_{13}^5 x_{14}^5$                                                             | $2^3 \cdot 3^2 \cdot 23 \cdot 463 \cdot 32939$<br>$2^2 \cdot 3^3 \cdot 5 \cdot 13 \cdot 2501119$                             |
| (7, 7)    | (0, 0, 0, 0, 1, 0, 0, 0, 1, 1, 1, 1, 1, 1, 1)    | 84  | $x_1^6 x_2^6 x_3^6 x_4^6 x_5^6 x_6^6 x_7^6 x_8^6 x_9^6 x_{10}^6 x_{11}^6 x_{12}^6 x_{13}^6 x_{14}^6$<br>$x_1^6 x_2^6 x_3^6 x_4^6 x_5^6 x_6^6 x_7^6 x_8^6 x_9^6 x_{10}^6 x_{11}^6 x_{12}^6 x_{13}^6 x_{14}^6$                                                             | $2^4 \cdot 3 \cdot 7 \cdot 17 \cdot 53 \cdot 8387$<br>$2^3 \cdot 3 \cdot 7 \cdot 23 \cdot 24946279$                          |
| (6, 8)    | (0, 0, 0, 1, 1, 1, 0, 0, 0, 1, 1, 1, 1, 1, 1)    | 85  | $x_1^4 x_2^5 x_3^5 x_4^7 x_5^7 x_6^5 x_7^5 x_8^5 x_9^7 x_{10}^7 x_{11}^7 x_{12}^7 x_{13}^7 x_{14}^7$<br>$x_1^5 x_2^4 x_3^5 x_4^7 x_5^7 x_6^5 x_7^5 x_8^5 x_9^7 x_{10}^7 x_{11}^7 x_{12}^7 x_{13}^7 x_{14}^7$                                                             | $-1 \cdot 2^3 \cdot 11 \cdot 941 \cdot 1091681$<br>$2^4 \cdot 3^3 \cdot 9043 \cdot 21487$                                    |
| (5, 9)    | (0, 0, 0, 1, 1, 1, 1, 1, 0, 1, 1, 0, 1, 1, 1)    | 90  | $x_1^2 x_2^4 x_3^4 x_4^8 x_5^8 x_6^8 x_7^8 x_8^4 x_9^8 x_{10}^8 x_{11}^8 x_{12}^8 x_{13}^8 x_{14}^8$<br>$x_1^3 x_2^3 x_3^4 x_4^8 x_5^8 x_6^8 x_7^8 x_8^4 x_9^8 x_{10}^8 x_{11}^8 x_{12}^8 x_{13}^8 x_{14}^8$                                                             | $-1 \cdot 2 \cdot 7^2 \cdot 29868578809$<br>$-1 \cdot 2^2 \cdot 3 \cdot 421848565301$                                        |
| (4, 10)   | (0, 0, 1, 1, 1, 1, 1, 0, 1, 1, 0, 1, 1, 1, 1)    | 95  | $x_1^3 x_2^3 x_3^2 x_4^9 x_5^9 x_6^9 x_7^3 x_8^9 x_9^9 x_{10}^3 x_{11}^9 x_{12}^9 x_{13}^9 x_{14}^9$<br>$x_1^3 x_2^3 x_3^3 x_4^8 x_5^9 x_6^9 x_7^3 x_8^9 x_9^9 x_{10}^3 x_{11}^9 x_{12}^9 x_{13}^9 x_{14}^9$                                                             | $-1 \cdot 2^3 \cdot 5 \cdot 29 \cdot 463 \cdot 8167703$<br>$-1 \cdot 2^2 \cdot 5^3 \cdot 7 \cdot 17^2 \cdot 587 \cdot 10433$ |
| (3, 11)   | (0, 0, 1, 0, 1, 1, 1, 1, 1, 1, 1, 1, 1, 1, 1, 1) | 104 | $x_1^2 x_2^2 x_3^4 x_4^2 x_5^{10} x_6^{10} x_7^{10} x_8^{10} x_9^{10} x_{10}^{10} x_{11}^{10} x_{12}^{10} x_{13}^{10} x_{14}^{10}$<br>$x_1^2 x_2^3 x_3^4 x_4^2 x_5^{10} x_6^{10} x_7^{10} x_8^{10} x_9^{10} x_{10}^{10} x_{11}^{10} x_{12}^{10} x_{13}^{10} x_{14}^{10}$ | $-1 \cdot 2 \cdot 117284188253$<br>$-1 \cdot 3 \cdot 65260863697$                                                            |
| (2, 12)   | (0, 1, 0, 1, 1, 1, 1, 1, 1, 1, 1, 1, 1, 1, 1, 1) | 113 | $x_1 x_2^4 x_3 x_4^8 x_5^{11} x_6^{11} x_7^{11} x_8^{11} x_9^{11} x_{10}^{11} x_{11}^{11} x_{12}^{11} x_{13}^{11} x_{14}^{11}$<br>$x_1 x_2^4 x_3 x_4^9 x_5^{10} x_6^{11} x_7^{11} x_8^{11} x_9^{11} x_{10}^{11} x_{11}^{11} x_{12}^{11} x_{13}^{11} x_{14}^{11}$         | $3 \cdot 19 \cdot 79 \cdot 4111 \cdot 26723$<br>$41 \cdot 25343 \cdot 419303$                                                |

$$S \subseteq \mathbb{Z}_p \times \mathbb{Z}_2 \setminus \{(0, 0)\}, |S| = 14$$

| $\lambda$ | $\mathbf{a}$                               | deg | monomial/s                                                                                                                                                                                                                                                                           | coefficient/s                                                                           |
|-----------|--------------------------------------------|-----|--------------------------------------------------------------------------------------------------------------------------------------------------------------------------------------------------------------------------------------------------------------------------------------|-----------------------------------------------------------------------------------------|
| (1, 13)   | (1, 0, 1, 1, 1, 1, 1, 1, 1, 1, 1, 1, 1, 1) | 126 | $x_1^3 x_2^4 x_3^{11} x_4^{12} x_5^{12} x_6^{12} x_7^{12} x_8^{12} x_9^{12} x_{10}^{12} x_{11}^{12} x_{12}^{12} x_{13}^{12} x_{14}^{12}$<br>$x_1^4 x_2^4 x_3^{10} x_4^{12} x_5^{12} x_6^{12} x_7^{12} x_8^{12} x_9^{12} x_{10}^{12} x_{11}^{12} x_{12}^{12} x_{13}^{12} x_{14}^{12}$ | $3 \cdot 5 \cdot 13370603941$<br>$3^2 \cdot 13 \cdot 23 \cdot 313 \cdot 349 \cdot 1873$ |
| (0, 14)   | (1, 1, 1, 1, 1, 1, 1, 1, 1, 1, 1, 1, 1, 1) | 139 | $x_1^2 x_2^4 x_3^6 x_4^{10} x_5^{13} x_6^{13} x_7^{13} x_8^{13} x_9^{13} x_{10}^{13} x_{11}^{13} x_{12}^{13} x_{13}^{13} x_{14}^{13}$<br>$x_1^2 x_2^5 x_3^5 x_4^{10} x_5^{13} x_6^{13} x_7^{13} x_8^{13} x_9^{13} x_{10}^{13} x_{11}^{13} x_{12}^{13} x_{13}^{13} x_{14}^{13}$       | $7 \cdot 407951725837$<br>$2^2 \cdot 3 \cdot 5 \cdot 29 \cdot 43 \cdot 1105141$         |

$$S \subseteq \mathbb{Z}_p \times \mathbb{Z}_2 \setminus \{(0, 0)\}, |S| = 15$$

| $\lambda$ | $\mathbf{a}$                                     | deg | monomial/s                                                                                                                                                                                                                                                                                             | coefficient/s                                                                                               |
|-----------|--------------------------------------------------|-----|--------------------------------------------------------------------------------------------------------------------------------------------------------------------------------------------------------------------------------------------------------------------------------------------------------|-------------------------------------------------------------------------------------------------------------|
| (15, 0)   |                                                  |     |                                                                                                                                                                                                                                                                                                        |                                                                                                             |
| (14, 1)   | (0, 0, 0, 0, 0, 0, 0, 1, 0, 0, 0, 0, 0, 0, 0)    | 133 | $x_1 x_2^4 x_3^4 x_4^9 x_5^{12} x_6^{12} x_7^{13} x_8^{13} x_9^{13} x_{10}^{13} x_{11}^{13} x_{12}^{13} x_{13}^{13} x_{14}^{13} x_{15}^{13}$<br>$x_1 x_2^4 x_3^5 x_4^8 x_5^{12} x_6^{12} x_7^{13} x_8^{13} x_9^{13} x_{10}^{13} x_{11}^{13} x_{12}^{13} x_{13}^{13} x_{14}^{13} x_{15}^{13}$           | $3 \cdot 5 \cdot 449 \cdot 77699$<br>$2^3 \cdot 17 \cdot 431 \cdot 48781$                                   |
| (13, 2)   | (0, 0, 0, 0, 0, 0, 1, 0, 0, 0, 0, 0, 0, 0, 1)    | 121 | $x_1^4 x_2^5 x_3^6 x_4^{10} x_5^{11} x_6^{12} x_7 x_8^{12} x_9^{12} x_{10}^{12} x_{11}^{12} x_{12}^{12} x_{13}^{12} x_{14}^{12}$<br>$x_1^4 x_2^5 x_3^7 x_4^9 x_5^{11} x_6^{12} x_7 x_8^{12} x_9^{12} x_{10}^{12} x_{11}^{12} x_{12}^{12} x_{13}^{12} x_{14}^{12}$                                      | $43 \cdot 59031989$<br>$5 \cdot 7 \cdot 31 \cdot 61 \cdot 140863$                                           |
| (12, 3)   | (0, 0, 0, 0, 0, 0, 1, 0, 0, 0, 0, 0, 0, 1, 1)    | 113 | $x_1^4 x_2^7 x_3^9 x_4^{10} x_5^{11} x_6^2 x_7^{11} x_8^{11} x_9^{11} x_{10}^{11} x_{11}^{11} x_{12}^{11} x_{13}^{11} x_{14}^2 x_{15}^2$<br>$x_1^4 x_2^8 x_3^8 x_4^{10} x_5^{11} x_6^2 x_7^{11} x_8^{11} x_9^{11} x_{10}^{11} x_{11}^{11} x_{12}^{11} x_{13}^{11} x_{14}^2 x_{15}^2$                   | $3^2 \cdot 37 \cdot 97 \cdot 65789$<br>$3^5 \cdot 7 \cdot 43 \cdot 25189$                                   |
| (11, 4)   | (0, 0, 0, 0, 0, 1, 0, 0, 0, 0, 0, 0, 0, 1, 1, 1) | 105 | $x_1^4 x_2^4 x_3^6 x_4^9 x_5^{10} x_6^3 x_7^{10} x_8^{10} x_9^{10} x_{10}^{10} x_{11}^{10} x_{12}^{10} x_{13}^3 x_{14}^3 x_{15}^3$<br>$x_1^4 x_2^5 x_3^5 x_4^9 x_5^{10} x_6^3 x_7^{10} x_8^{10} x_9^{10} x_{10}^{10} x_{11}^{10} x_{12}^{10} x_{13}^3 x_{14}^3 x_{15}^3$                               | $2^2 \cdot 22697 \cdot 120607$<br>$-1 \cdot 2^2 \cdot 3 \cdot 11 \cdot 8386817$                             |
| (10, 5)   | (0, 0, 0, 0, 0, 1, 0, 0, 0, 0, 0, 0, 1, 1, 1, 1) | 101 | $x_1^5 x_2^6 x_3^8 x_4^8 x_5^9 x_6^4 x_7^9 x_8^9 x_9^9 x_{10}^9 x_{11}^4 x_{12}^4 x_{13}^4 x_{14}^4 x_{15}^4$<br>$x_1^5 x_2^6 x_3^7 x_4^9 x_5^9 x_6^4 x_7^9 x_8^9 x_9^9 x_{10}^9 x_{11}^4 x_{12}^4 x_{13}^4 x_{14}^4 x_{15}^4$                                                                         | $3 \cdot 170389 \cdot 794471$<br>$2^8 \cdot 3 \cdot 7 \cdot 11 \cdot 31 \cdot 129581$                       |
| (9, 6)    | (0, 0, 0, 0, 1, 0, 0, 0, 0, 0, 1, 1, 1, 1, 1, 1) | 97  | $x_1^5 x_2^6 x_3^8 x_4^8 x_5^5 x_6^8 x_7^8 x_8^8 x_9^8 x_{10}^5 x_{11}^5 x_{12}^5 x_{13}^5 x_{14}^5 x_{15}^5$<br>$x_1^6 x_2^5 x_3^8 x_4^8 x_5^5 x_6^8 x_7^8 x_8^8 x_9^8 x_{10}^5 x_{11}^5 x_{12}^5 x_{13}^5 x_{14}^5 x_{15}^5$                                                                         | $-1 \cdot 2^3 \cdot 7 \cdot 13 \cdot 41 \cdot 53 \cdot 3556601$<br>$2^3 \cdot 151 \cdot 681853993$          |
| (8, 7)    | (0, 0, 0, 0, 1, 0, 0, 0, 0, 1, 1, 1, 1, 1, 1, 1) | 97  | $x_1^6 x_2^7 x_3^7 x_4^6 x_5^6 x_6^7 x_7^7 x_8^7 x_9^6 x_{10}^6 x_{11}^6 x_{12}^6 x_{13}^6 x_{14}^6 x_{15}^6$<br>$x_1^7 x_2^6 x_3^7 x_4^6 x_5^6 x_6^7 x_7^7 x_8^7 x_9^6 x_{10}^6 x_{11}^6 x_{12}^6 x_{13}^6 x_{14}^6 x_{15}^6$                                                                         | $2^3 \cdot 3^2 \cdot 31119324101$<br>$-1 \cdot 2^4 \cdot 3^6 \cdot 8731 \cdot 16057$                        |
| (7, 8)    | (0, 0, 0, 1, 0, 0, 0, 0, 1, 1, 1, 1, 1, 1, 1, 1) | 97  | $x_1^5 x_2^6 x_3^6 x_4^7 x_5^6 x_6^6 x_7^6 x_8^6 x_9^7 x_{10}^7 x_{11}^7 x_{12}^7 x_{13}^7 x_{14}^7 x_{15}^7$<br>$x_1^6 x_2^5 x_3^6 x_4^7 x_5^6 x_6^6 x_7^6 x_8^6 x_9^7 x_{10}^7 x_{11}^7 x_{12}^7 x_{13}^7 x_{14}^7 x_{15}^7$                                                                         | $2^5 \cdot 3^2 \cdot 31 \cdot 27059 \cdot 35291$<br>$-1 \cdot 2^4 \cdot 3 \cdot 863 \cdot 5237 \cdot 10939$ |
| (6, 9)    | (0, 0, 0, 1, 0, 0, 0, 1, 1, 1, 1, 1, 1, 1, 1, 1) | 101 | $x_1^4 x_2^5 x_3^5 x_4^8 x_5^5 x_6^5 x_7^8 x_8^8 x_9^8 x_{10}^8 x_{11}^8 x_{12}^8 x_{13}^8 x_{14}^8 x_{15}^8$<br>$x_1^5 x_2^4 x_3^5 x_4^8 x_5^5 x_6^5 x_7^8 x_8^8 x_9^8 x_{10}^8 x_{11}^8 x_{12}^8 x_{13}^8 x_{14}^8 x_{15}^8$                                                                         | $-1 \cdot 2 \cdot 3 \cdot 886287349231$<br>$2^2 \cdot 3^2 \cdot 7 \cdot 49439843113$                        |
| (5, 10)   | (0, 0, 0, 1, 1, 1, 1, 1, 0, 1, 1, 0, 1, 1, 1, 1) | 106 | $x_1^2 x_2^4 x_3^4 x_4^7 x_5^9 x_6^9 x_7^9 x_8^4 x_9^9 x_{10}^9 x_{11}^4 x_{12}^9 x_{13}^9 x_{14}^9 x_{15}^9$<br>$x_1^2 x_2^4 x_3^4 x_4^8 x_5^8 x_6^9 x_7^9 x_8^4 x_9^9 x_{10}^9 x_{11}^4 x_{12}^9 x_{13}^9 x_{14}^9 x_{15}^9$                                                                         | $2 \cdot 139 \cdot 181 \cdot 293 \cdot 997 \cdot 5501$<br>$2^3 \cdot 3 \cdot 41 \cdot 1511 \cdot 167856823$ |
| (4, 11)   | (0, 0, 1, 0, 0, 1, 1, 1, 1, 1, 1, 1, 1, 1, 1, 1) | 113 | $x_1^3 x_2^3 x_3^4 x_4^3 x_5^7 x_6^{10} x_7^{10} x_8^{10} x_9^{10} x_{10}^{10} x_{11}^{10} x_{12}^{10} x_{13}^{10} x_{14}^{10} x_{15}^{10}$<br>$x_1^3 x_2^3 x_3^4 x_4^3 x_5^8 x_6^9 x_7^8 x_8^9 x_9^{10} x_{10}^{10} x_{11}^{10} x_{12}^{10} x_{13}^{10} x_{14}^{10} x_{15}^{10}$                      | $-1 \cdot 1489 \cdot 153071 \cdot 1290593$<br>$-1 \cdot 3 \cdot 11 \cdot 14869 \cdot 688228531$             |
| (3, 12)   | (0, 1, 0, 0, 1, 1, 1, 1, 1, 1, 1, 1, 1, 1, 1, 1) | 121 | $x_1^2 x_2^5 x_3^2 x_4^{11} x_5^{11} x_6^{11} x_7^{11} x_8^{11} x_9^{11} x_{10}^{11} x_{11}^{11} x_{12}^{11} x_{13}^{11} x_{14}^{11} x_{15}^{11}$<br>$x_1^2 x_2^6 x_3^2 x_4^{10} x_5^{11} x_6^{11} x_7^{11} x_8^{11} x_9^{11} x_{10}^{11} x_{11}^{11} x_{12}^{11} x_{13}^{11} x_{14}^{11} x_{15}^{11}$ | $3 \cdot 33102802861319$<br>$7 \cdot 13 \cdot 944337461087$                                                 |
| (2, 13)   | (0, 1, 0, 1, 1, 1, 1, 1, 1, 1, 1, 1, 1, 1, 1, 1) | 133 |                                                                                                                                                                                                                                                                                                        |                                                                                                             |
| (1, 14)   | (1, 0, 1, 1, 1, 1, 1, 1, 1, 1, 1, 1, 1, 1, 1, 1) | 145 |                                                                                                                                                                                                                                                                                                        |                                                                                                             |

$$S \subseteq \mathbb{Z}_p \times \mathbb{Z}_2 \setminus \{(0,0)\}, |S| = 15$$

| $\lambda$ | $\mathbf{a}$                                  | deg | monomial/s | coefficient/s |
|-----------|-----------------------------------------------|-----|------------|---------------|
| (0, 15)   | (1, 1, 1, 1, 1, 1, 1, 1, 1, 1, 1, 1, 1, 1, 1) | 161 |            |               |
